# Supplementary material for: Jeans Model for the Shapes of Self-interacting Dark Matter Halos
Source: arXiv:2511.10765 ancillary file (2025-11-13)
Supplement: Supplementary file 1 [file Ancillary1.pdf]

# Ancillary material 1: SIDM1 and CDM halos in the Eagle-50 simulations set. This material is associated to the submission, Jeans Model for the Shapes of Self-interacting Dark Matter Halo Shapes

Yilber Fabian Bautista, Andrew Robertson, Laura Sagunski, Adam Smith-Orlik, and Sean Tulin

The figures in this ancillary file correspond to relaxed halos from the EAGLE-50 simulations presented in Ref. [1], for two models: self-interacting dark matter with  $\sigma/m = 1 \text{ cm}^2/\text{g}$  (SIDM1) and collisionless dark matter with  $\sigma/m = 0$  (CDM). The left panels show the spherically averaged density profiles, the central panels display the azimuthally averaged iso-density contours, and the right panels present the halo shape profiles for a given halo. Further details are provided in Section IV-A of the main text.

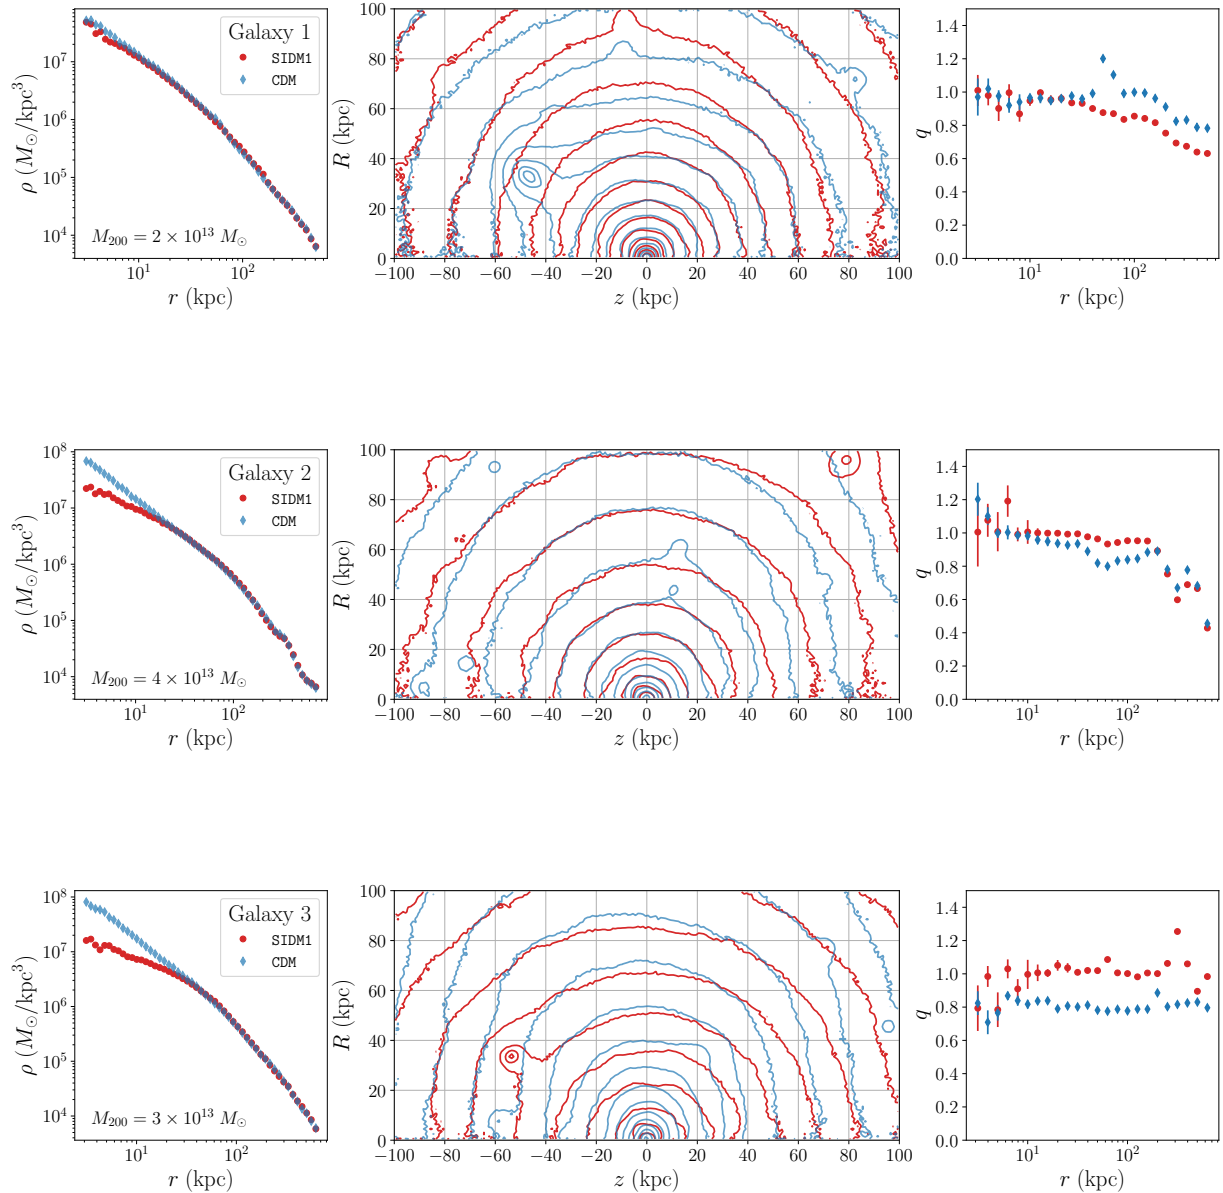

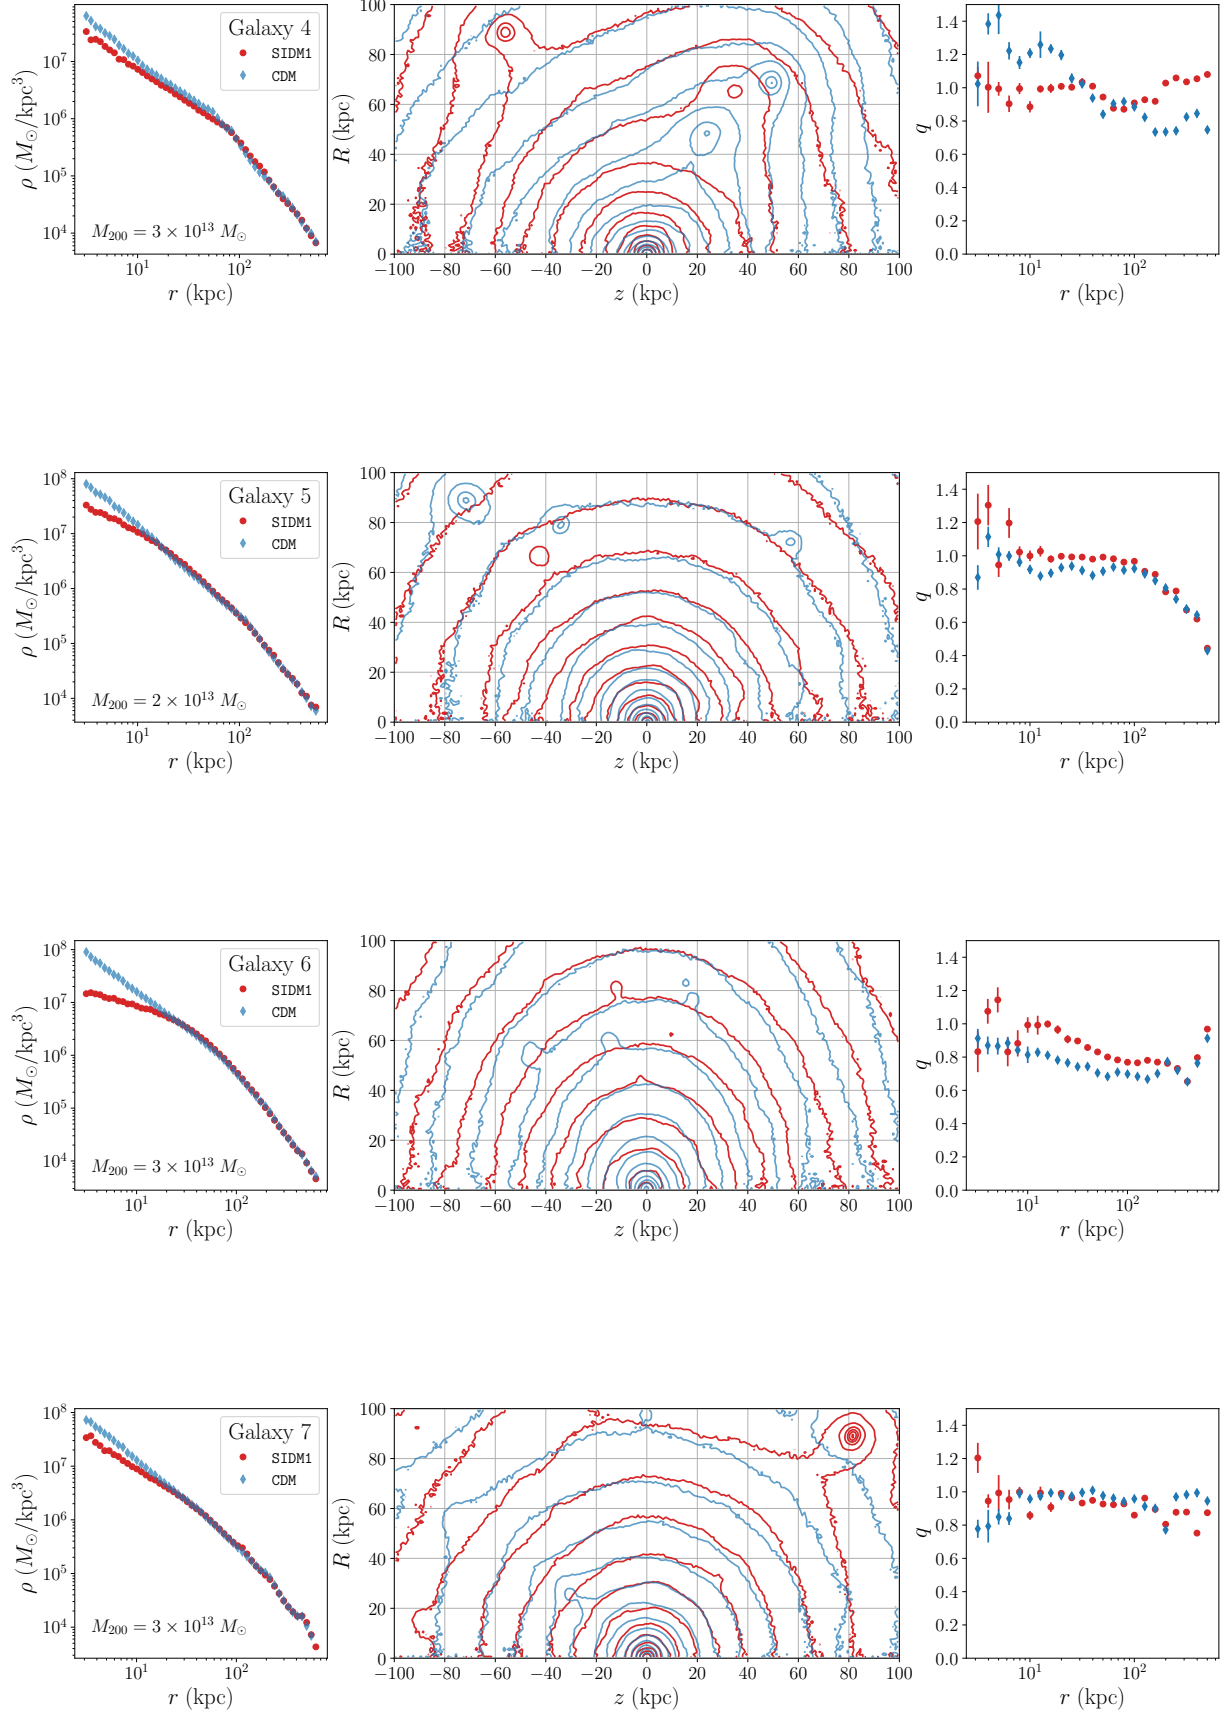

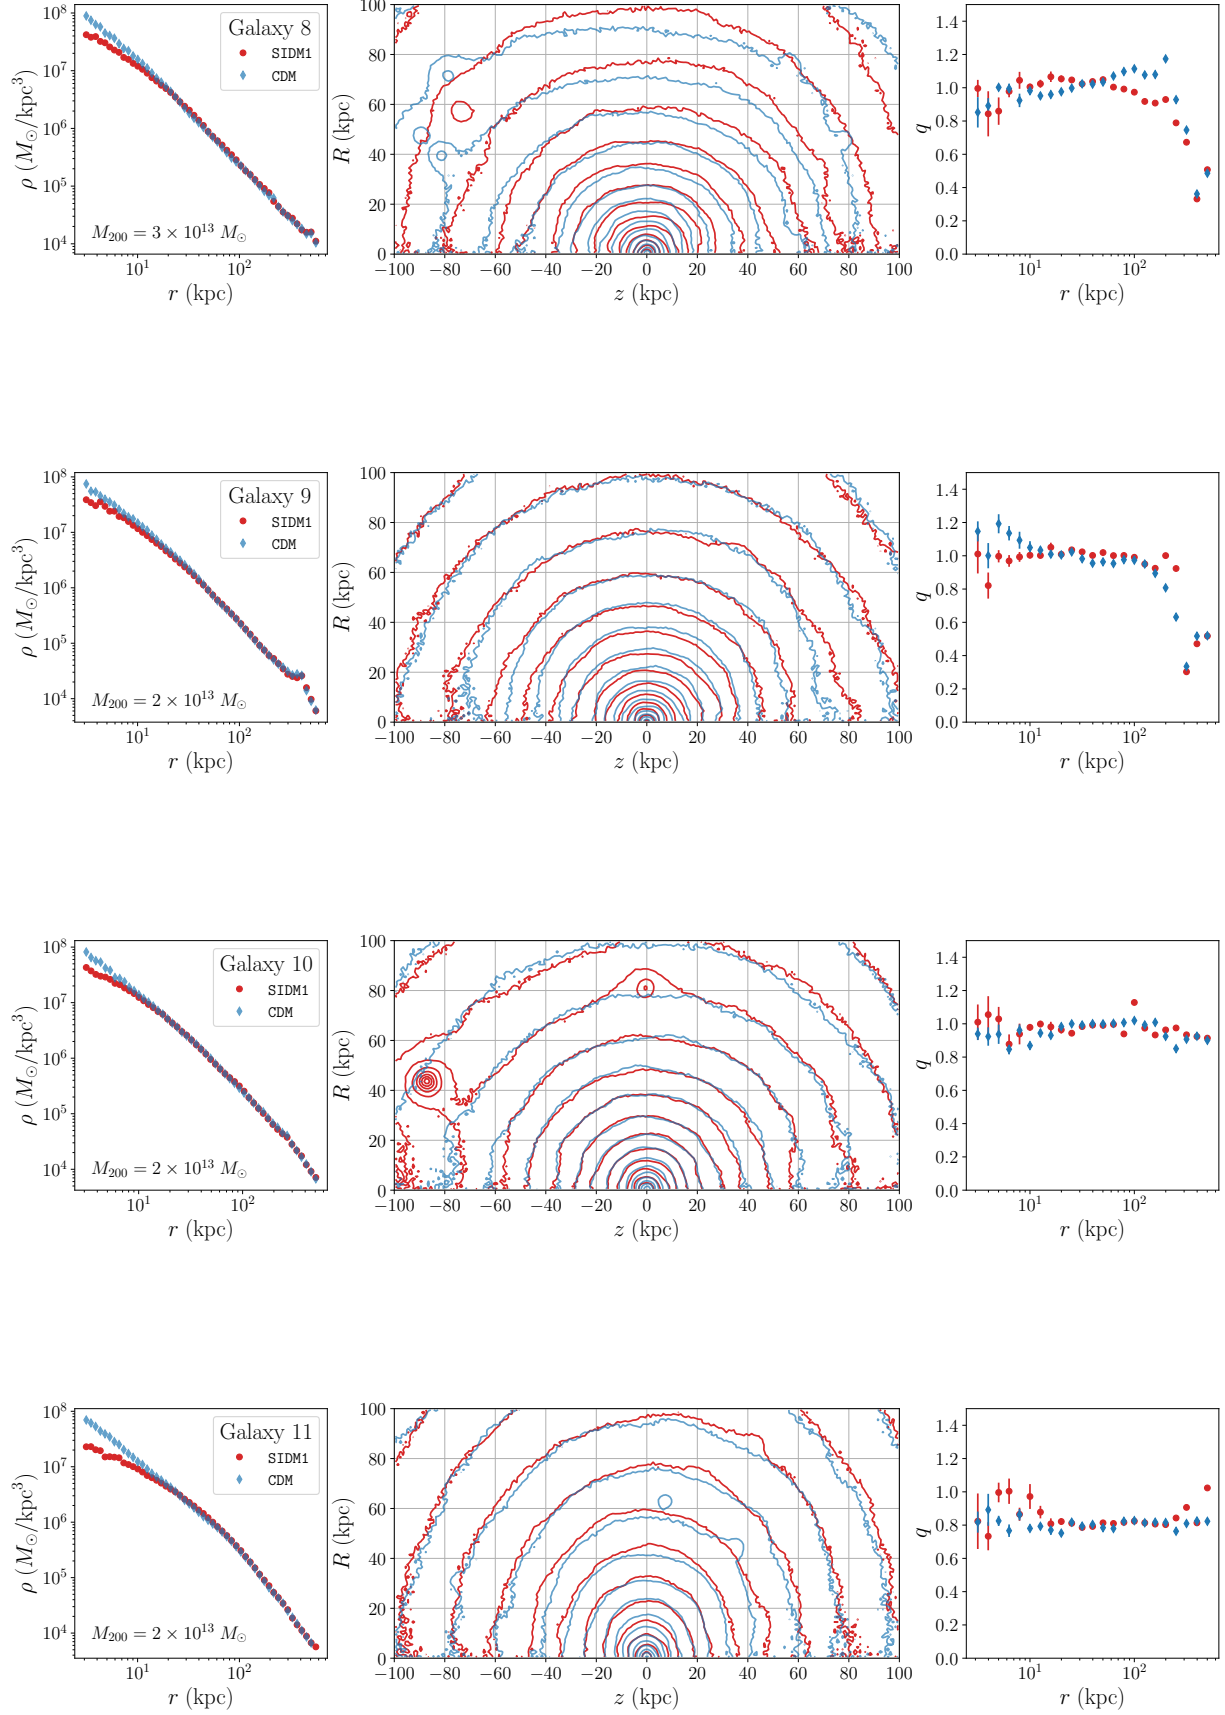

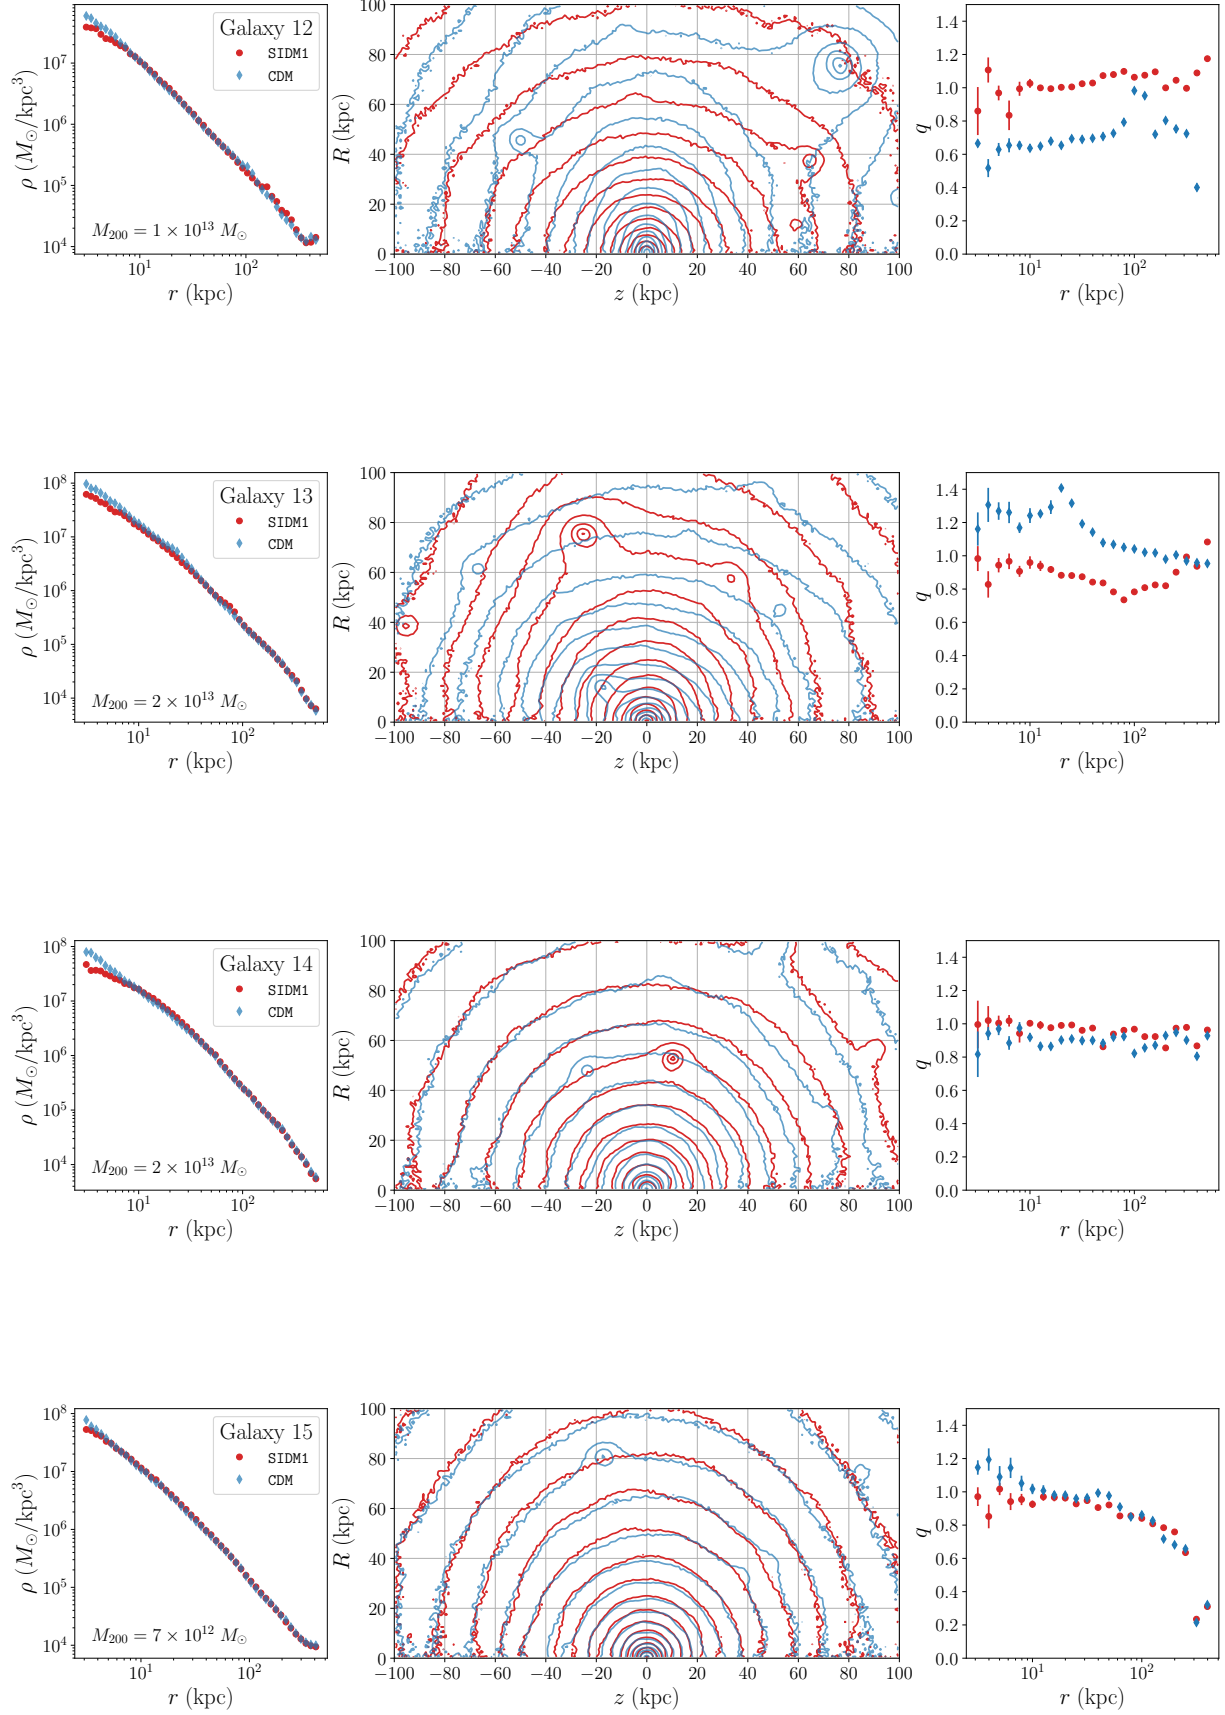



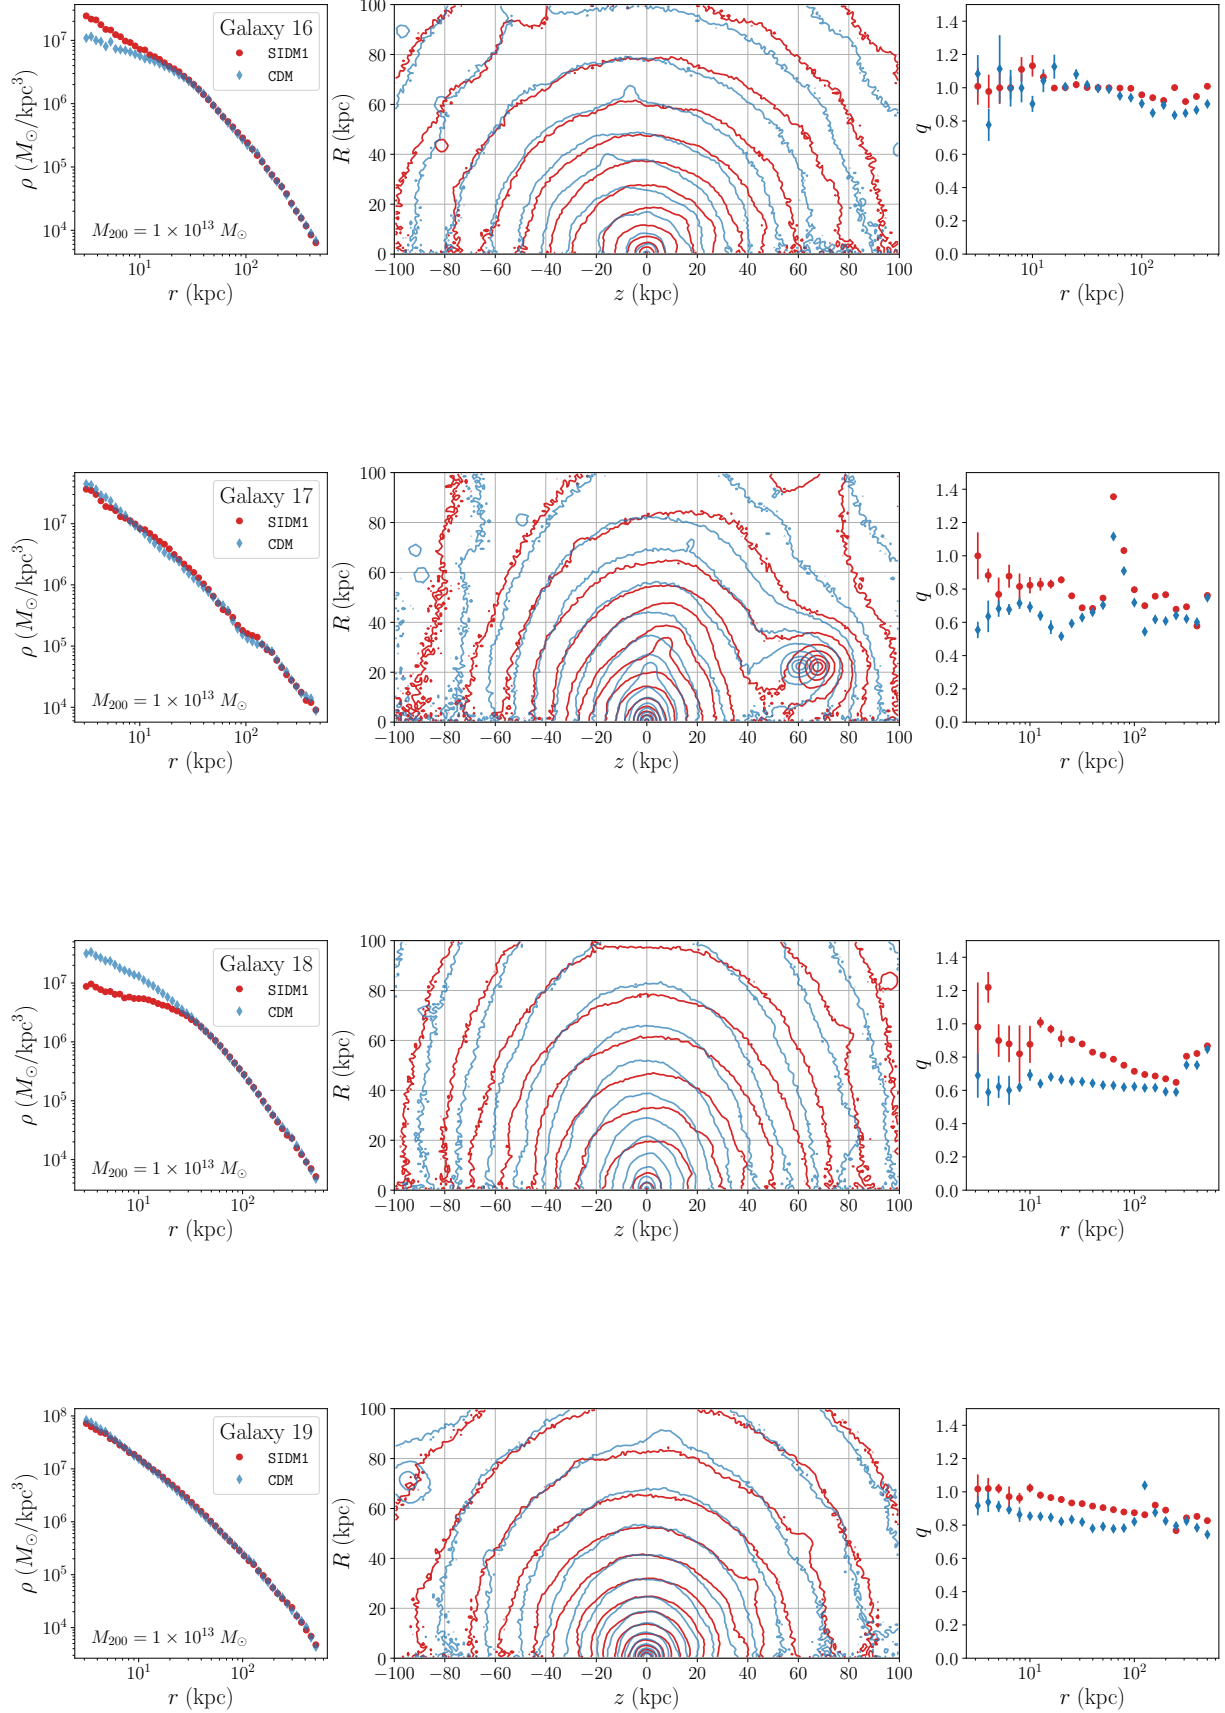

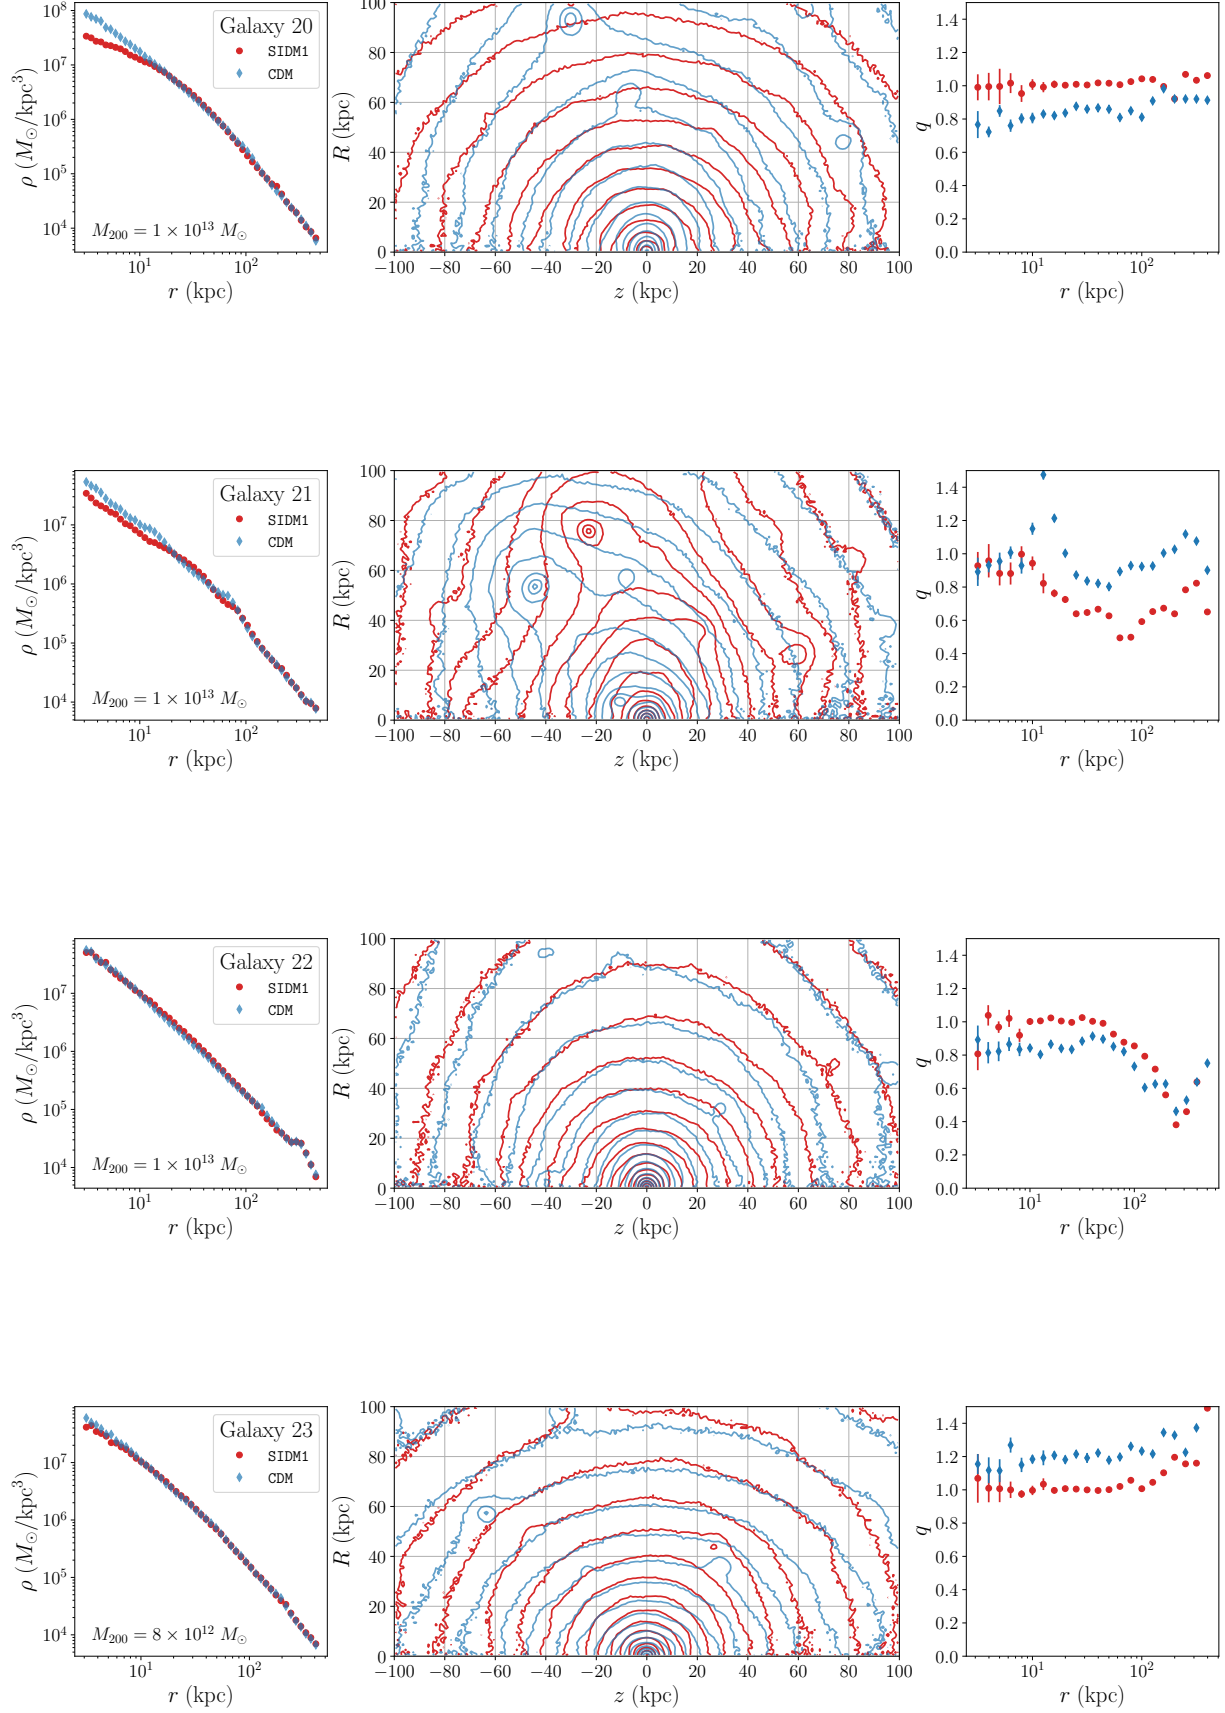

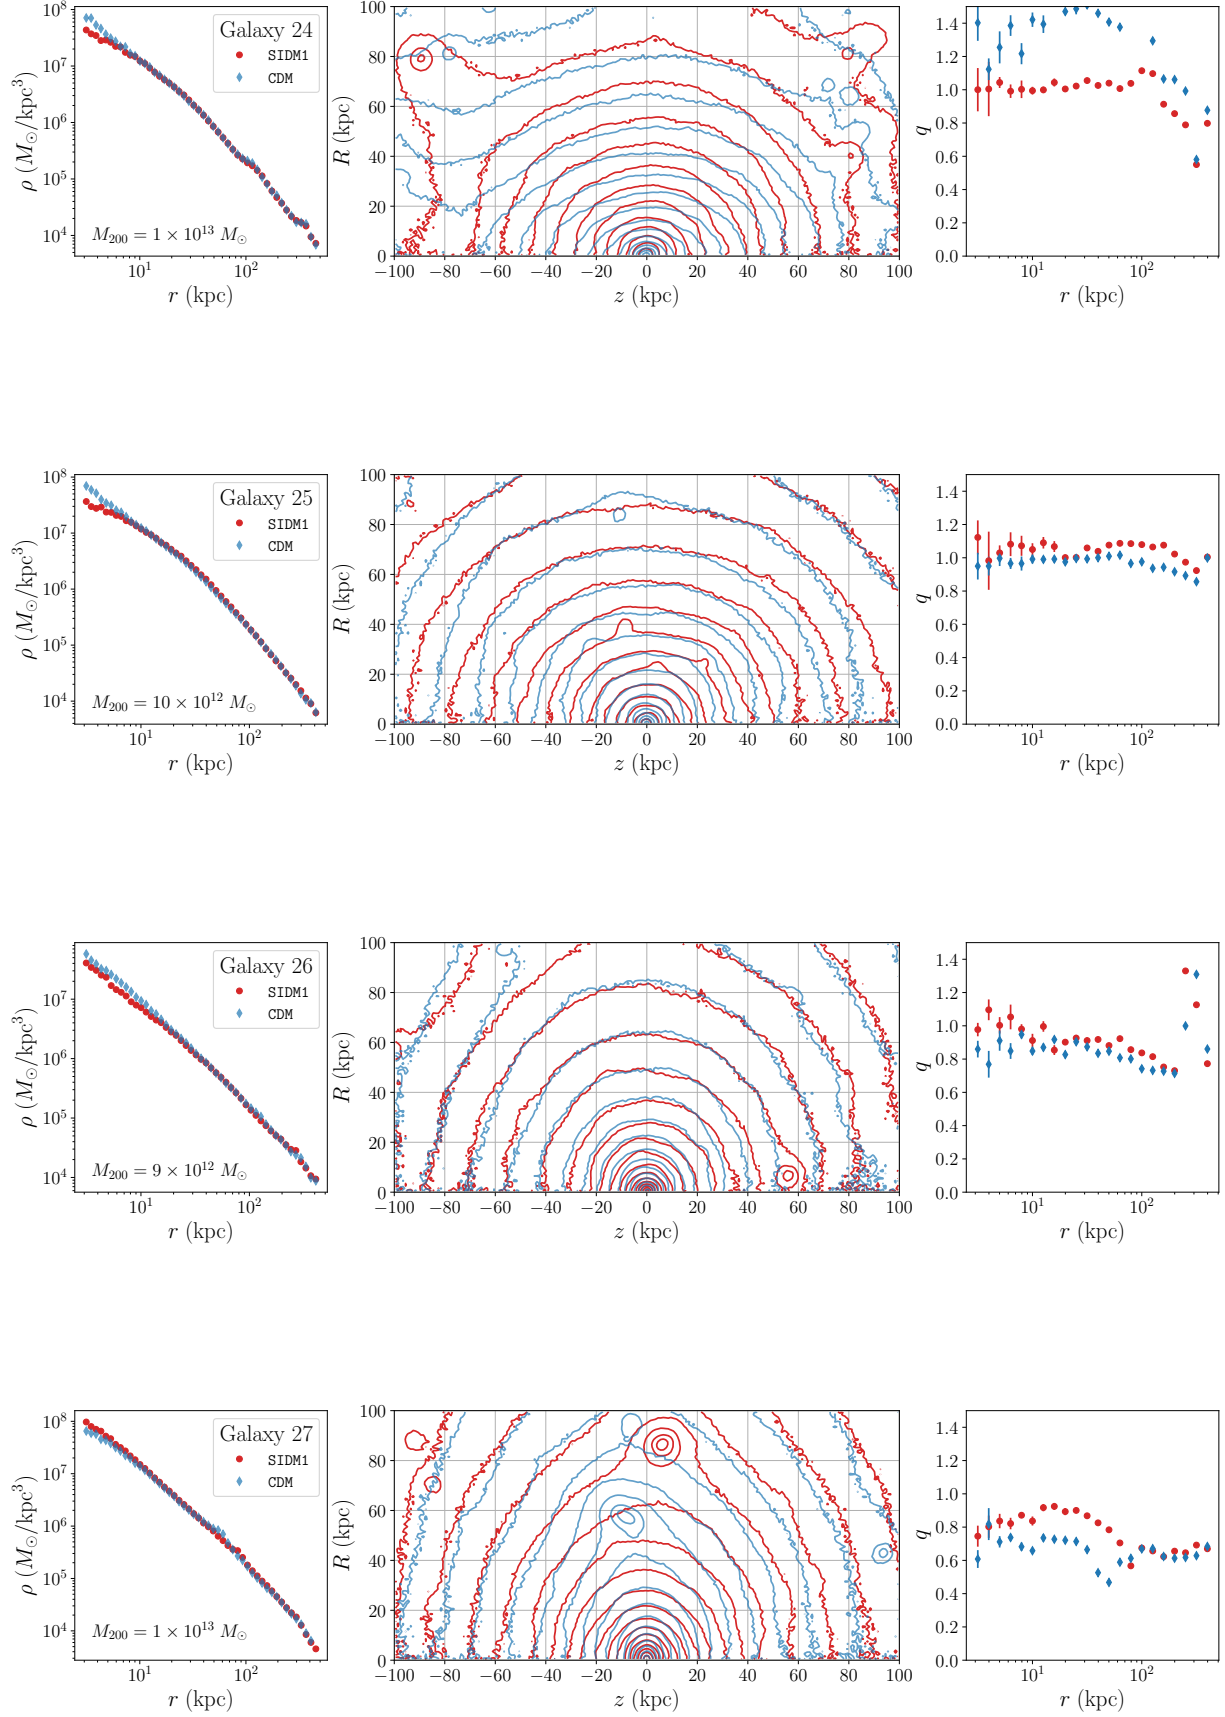

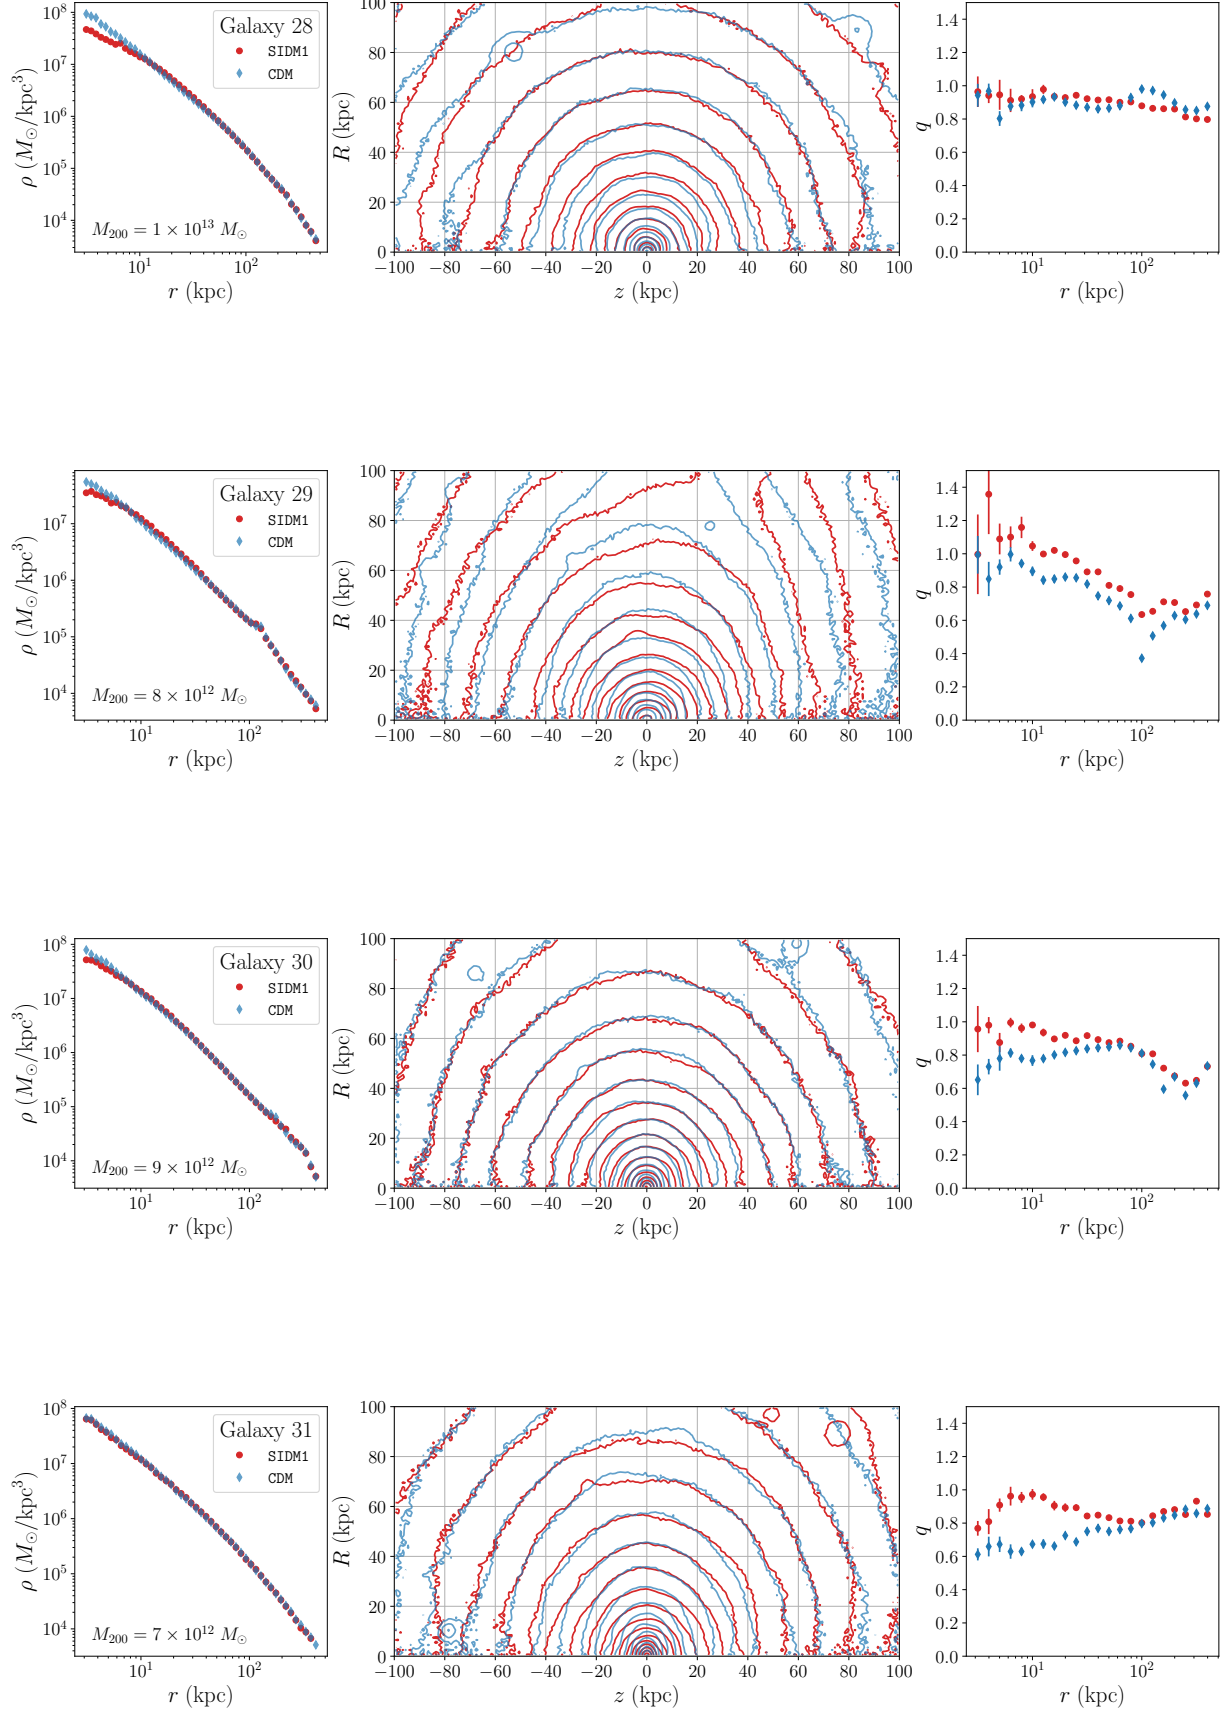

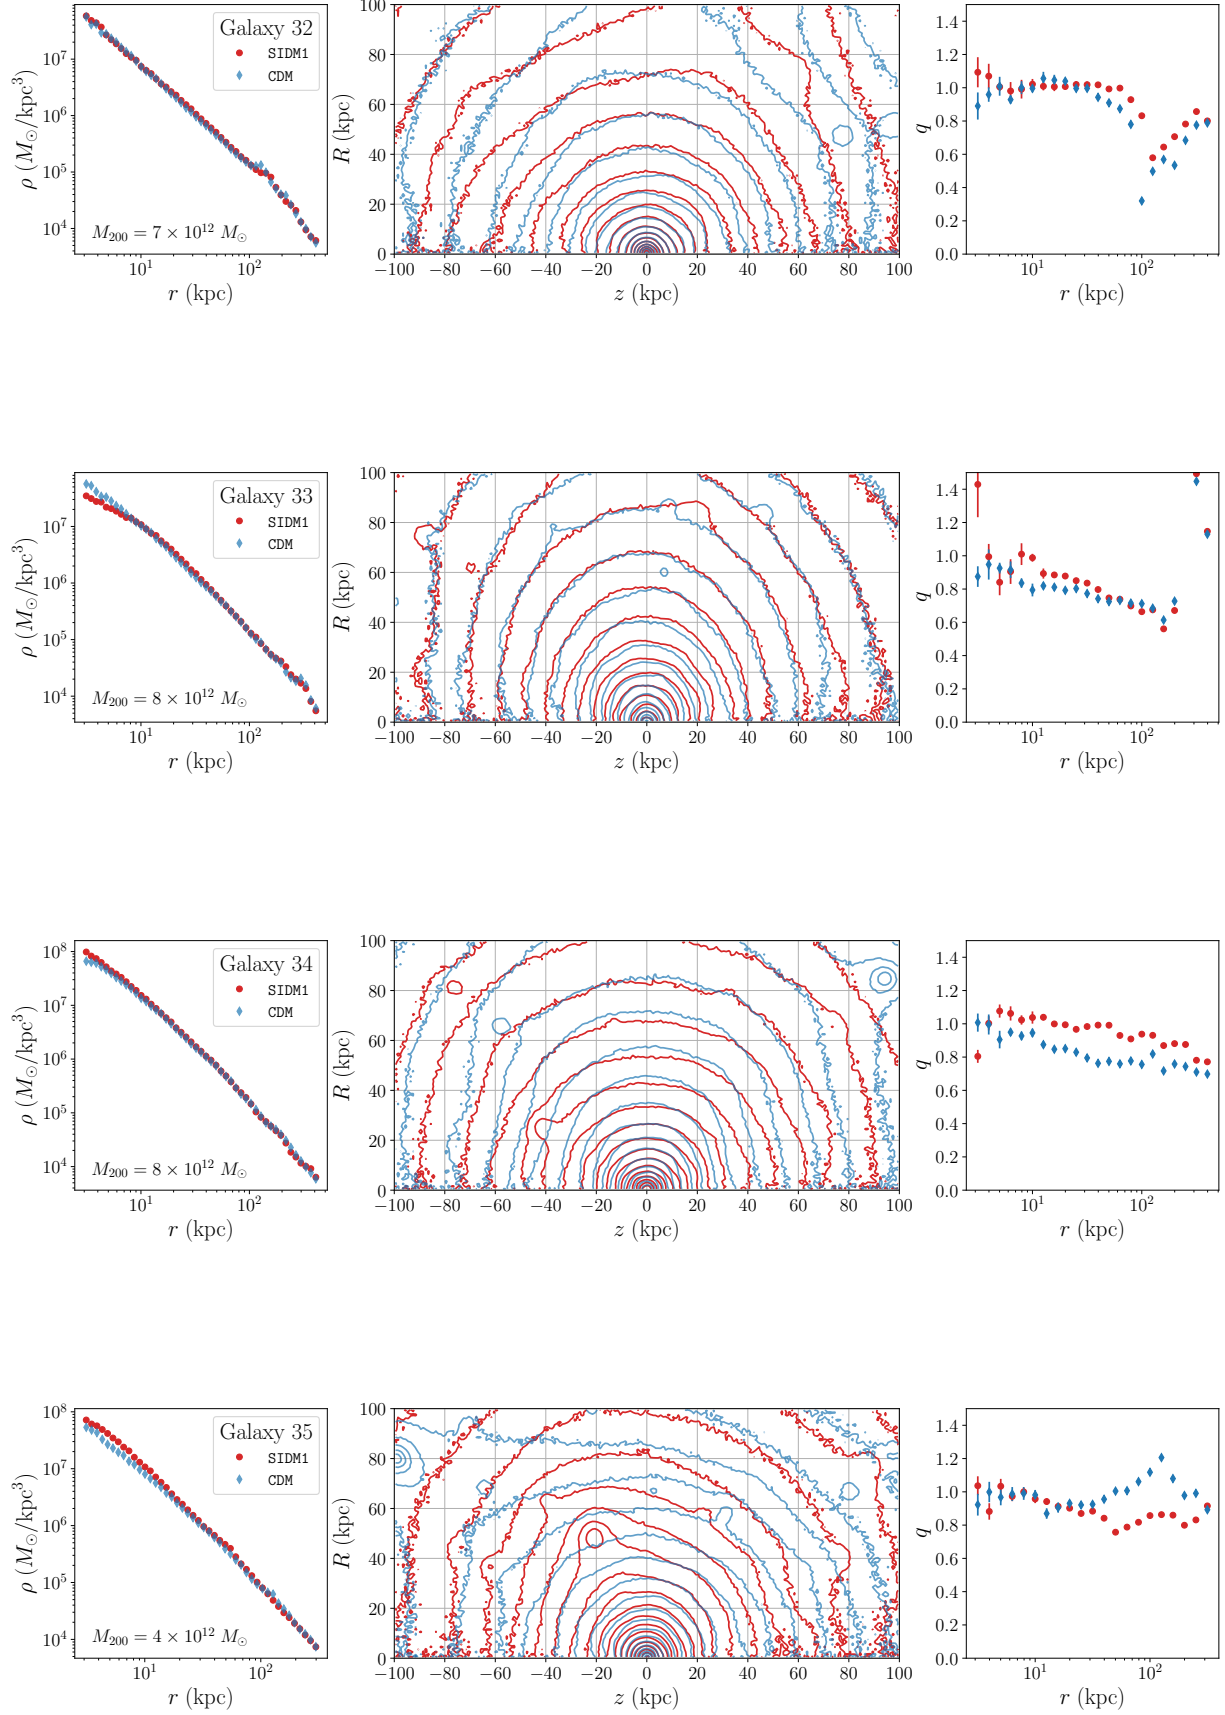

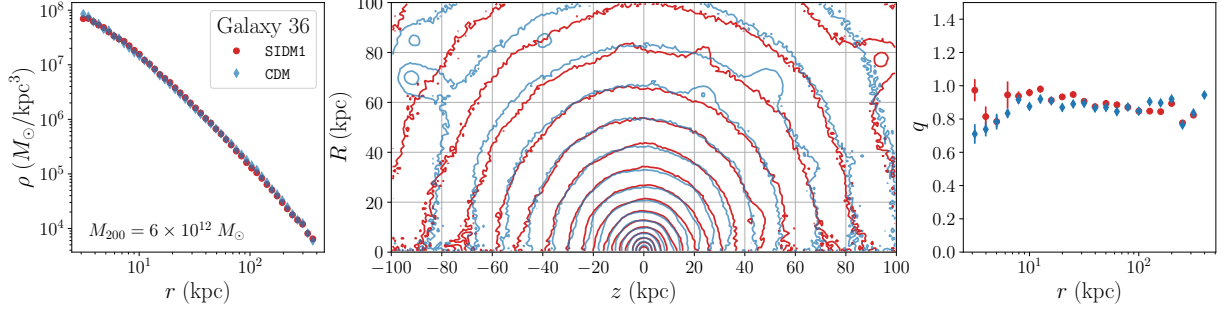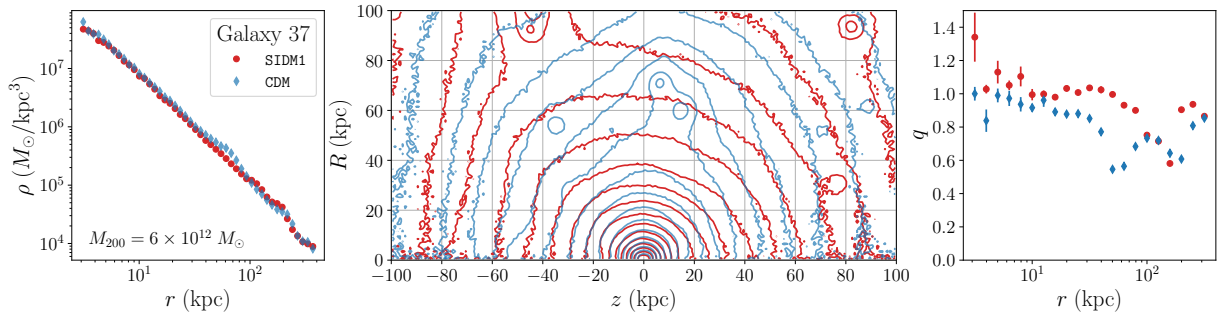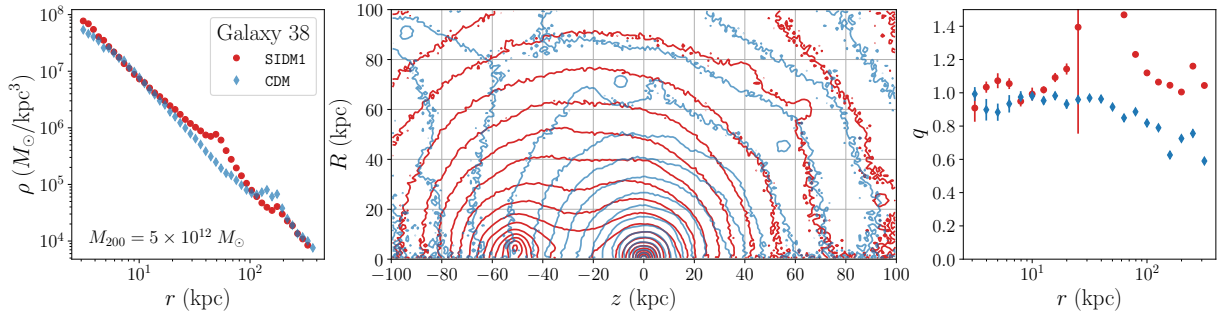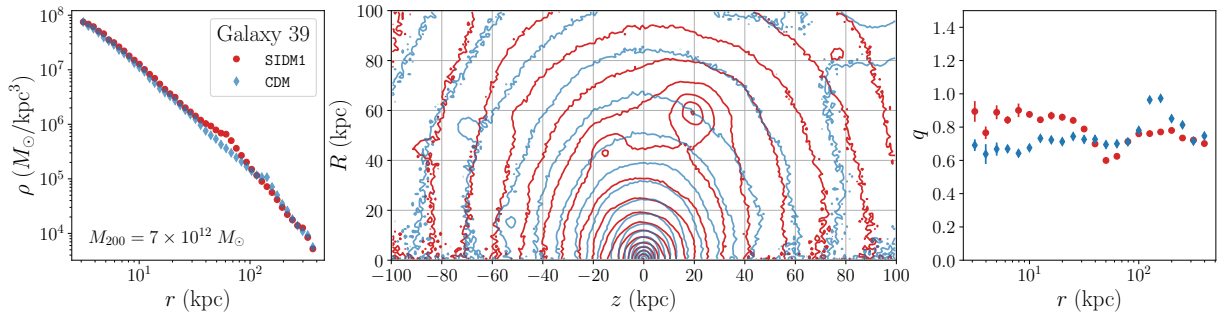



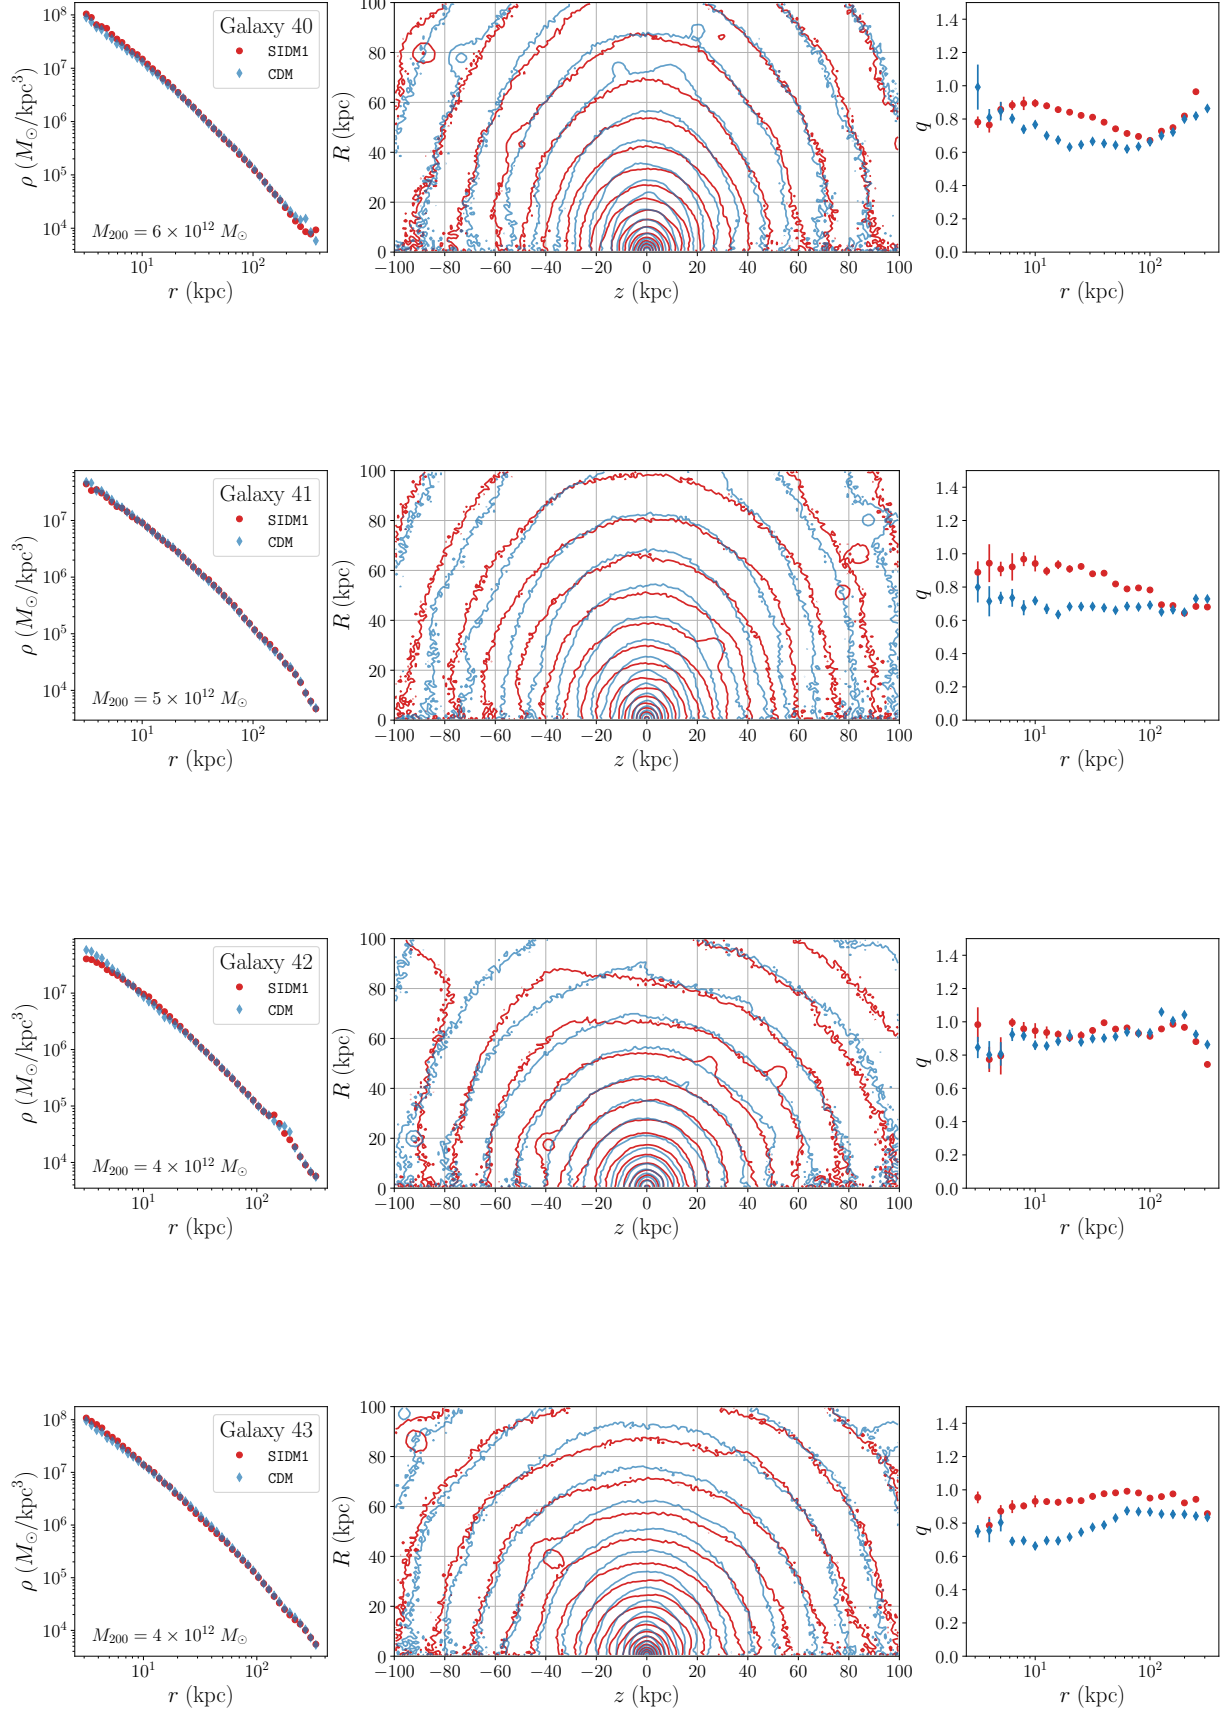

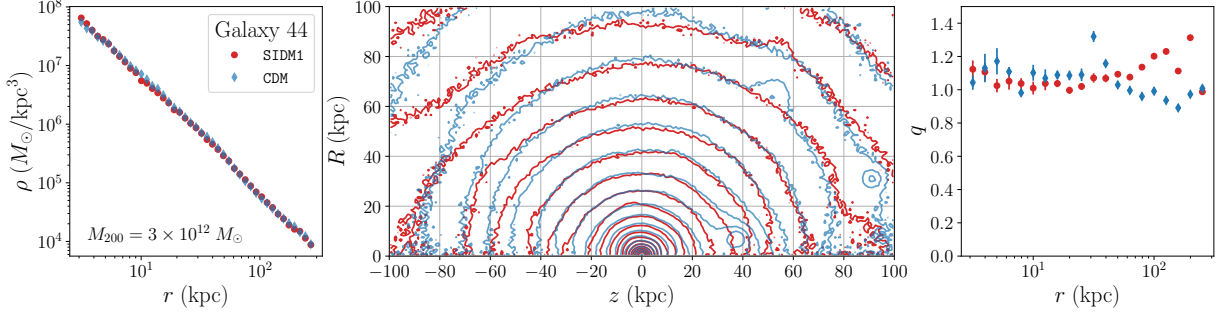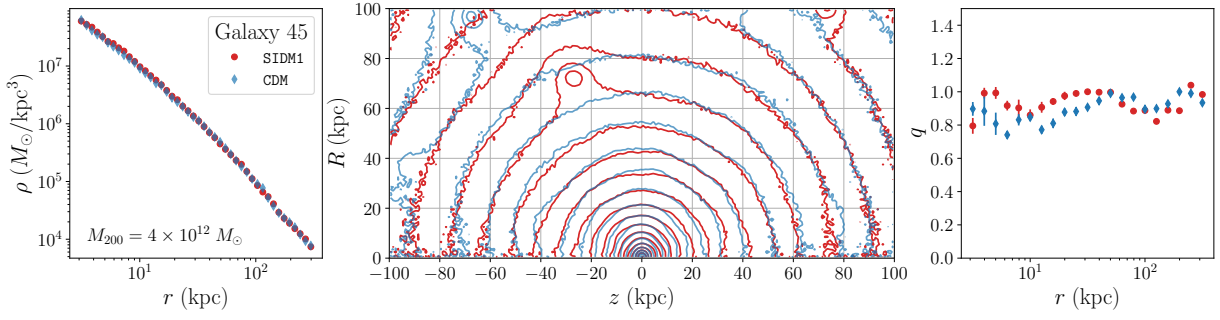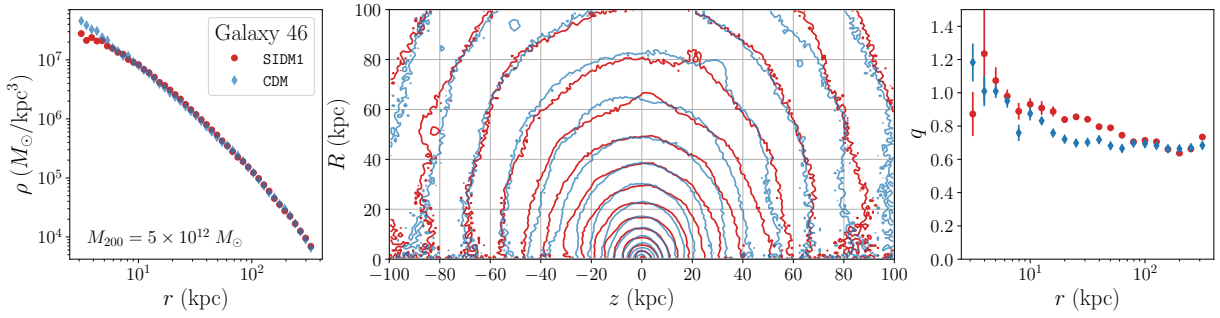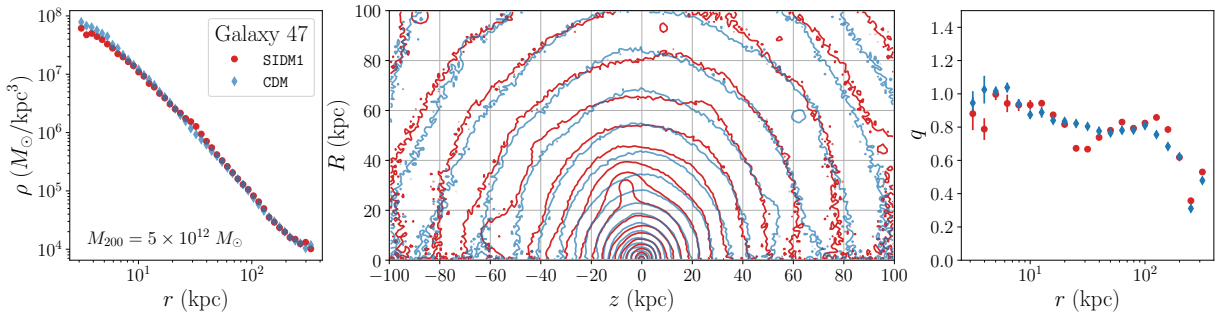

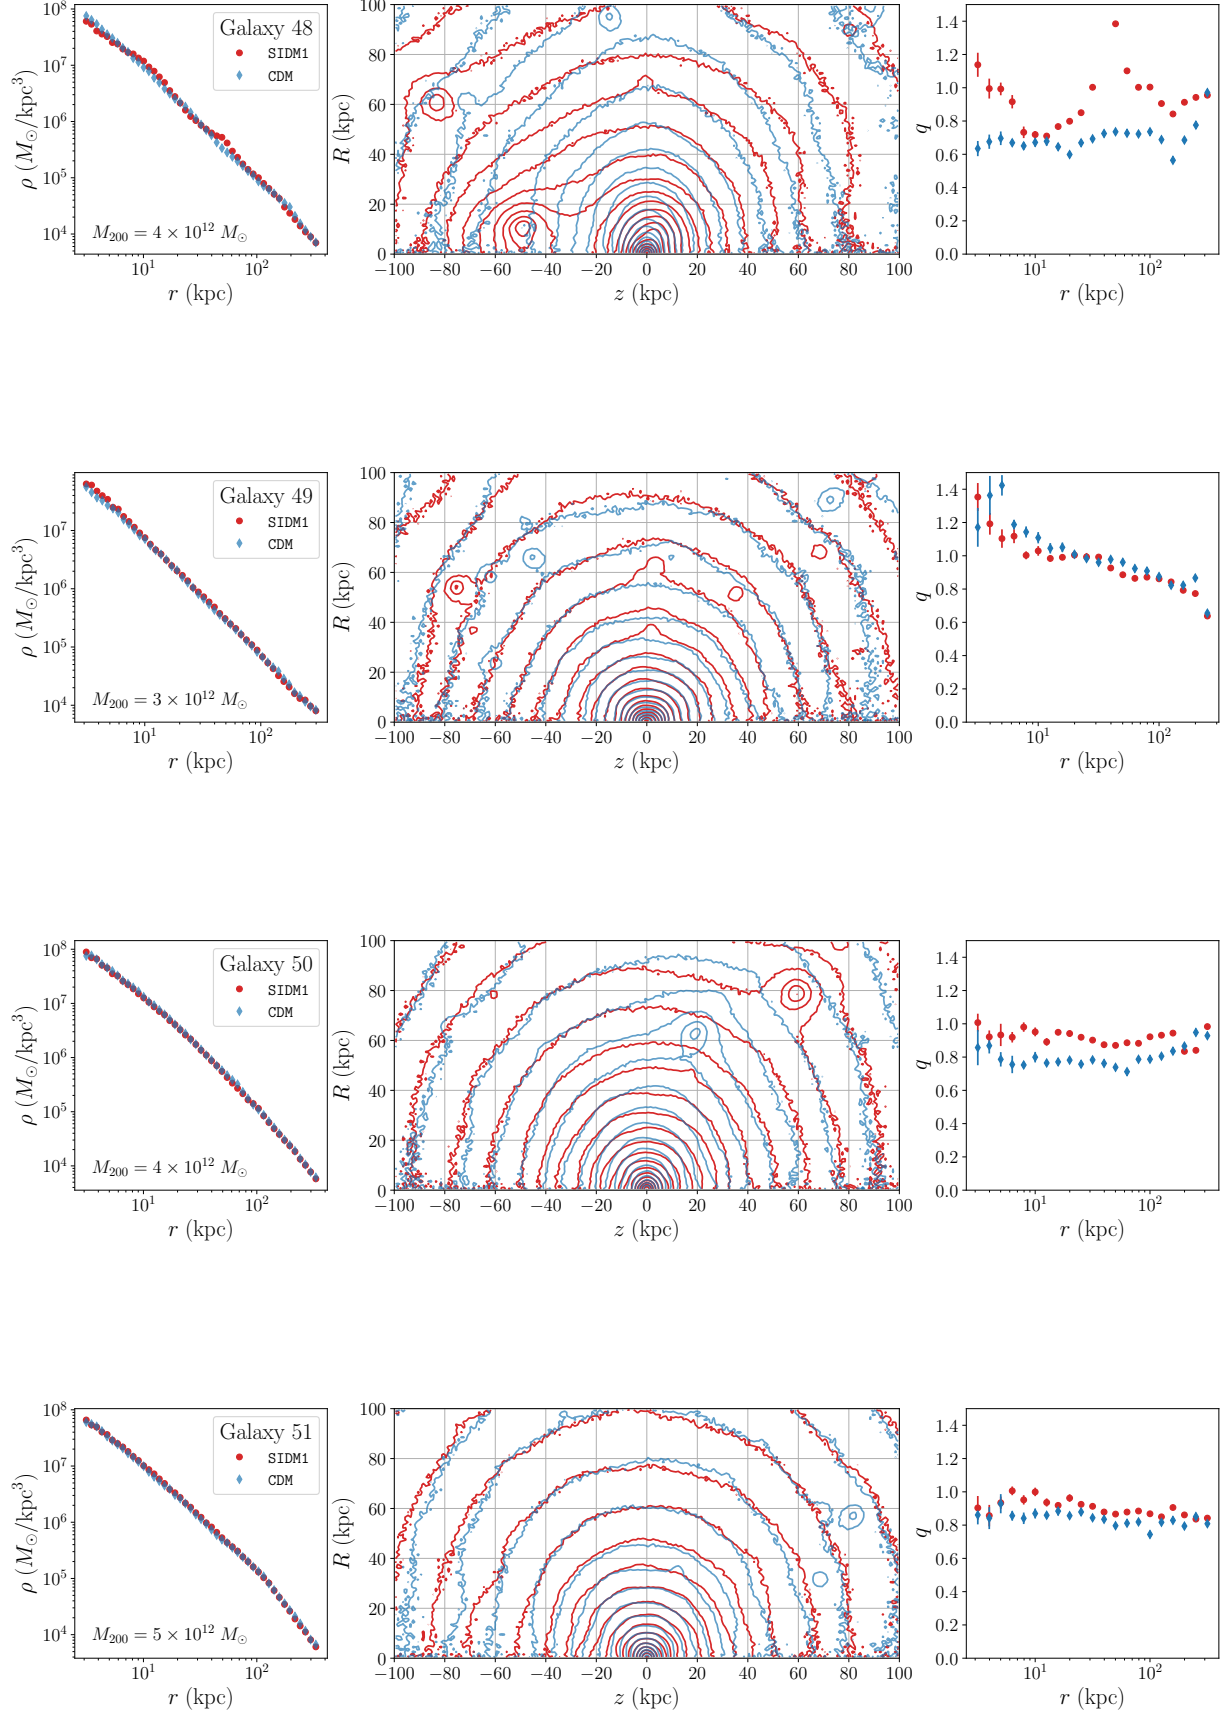

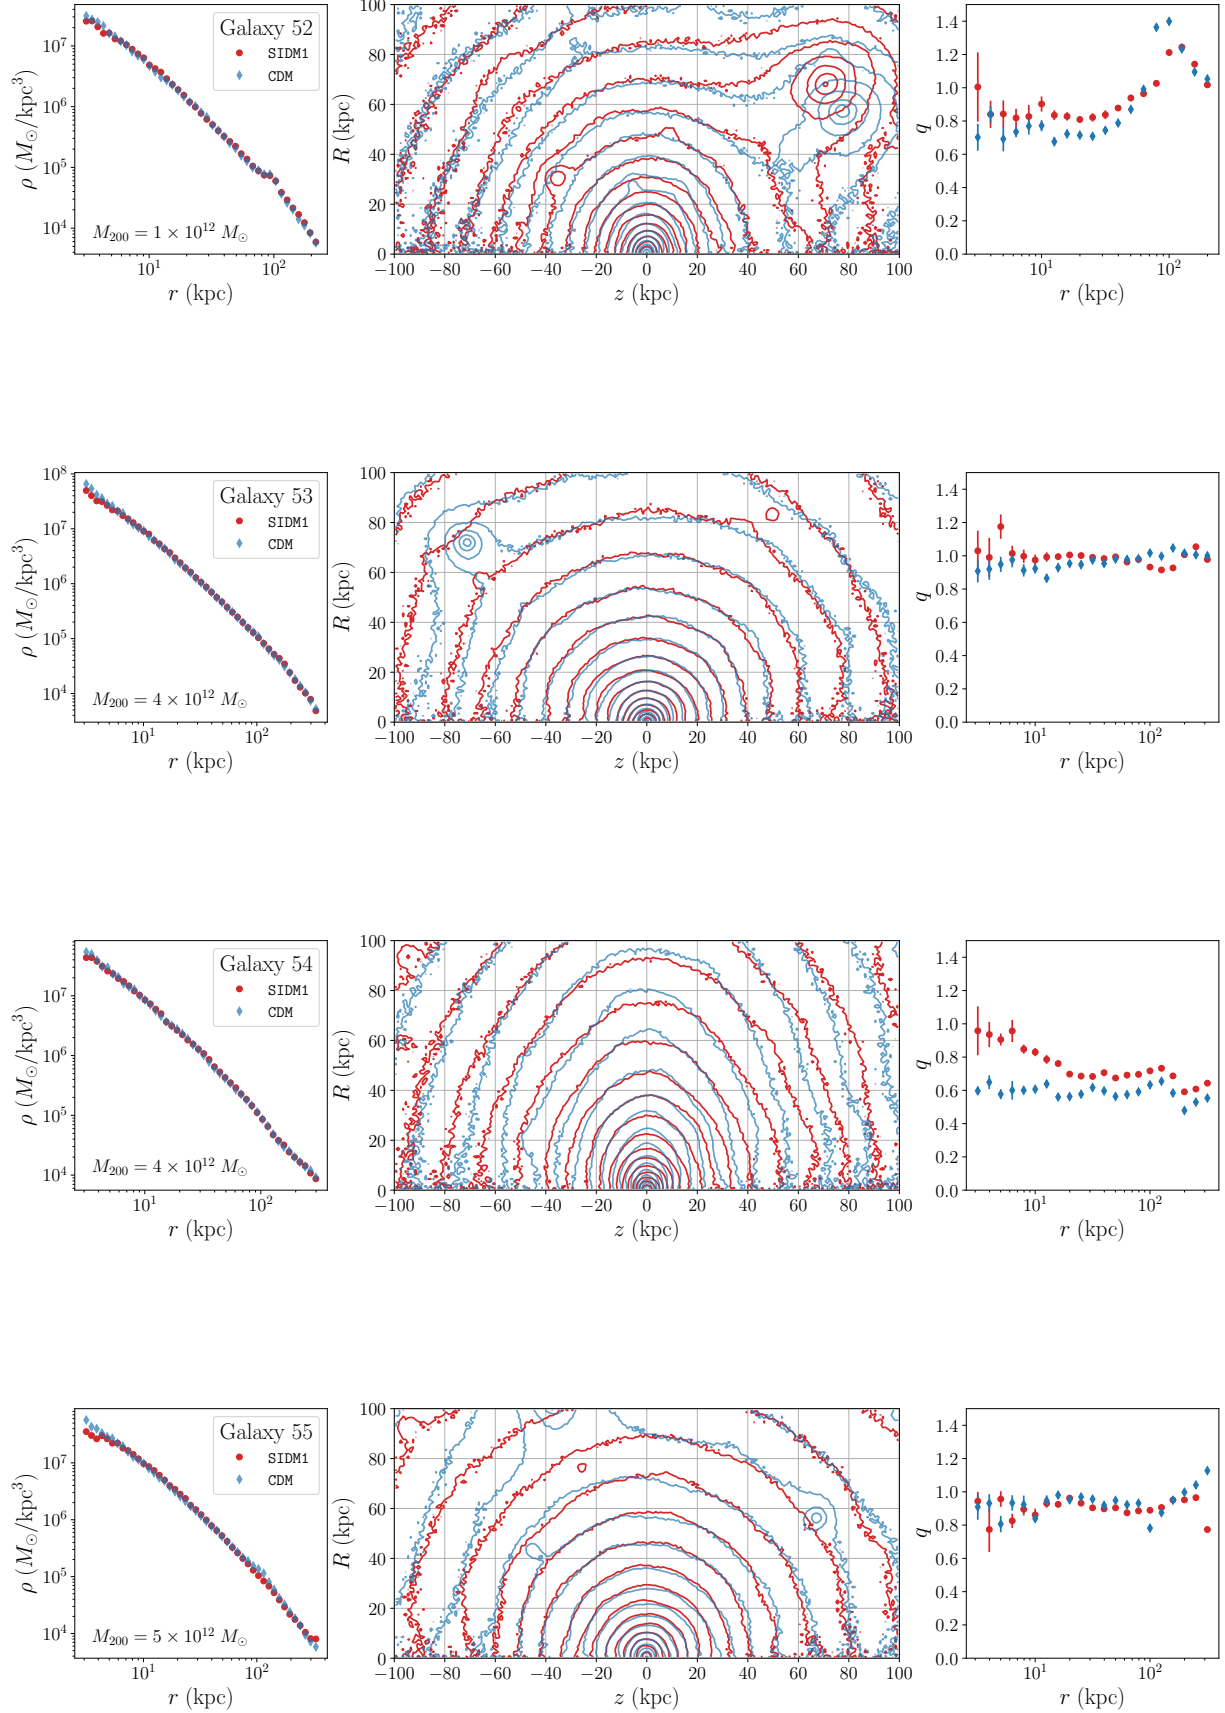

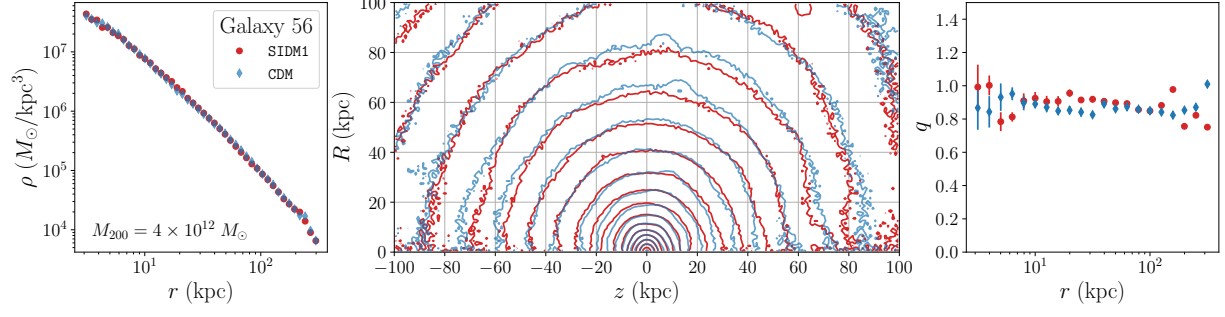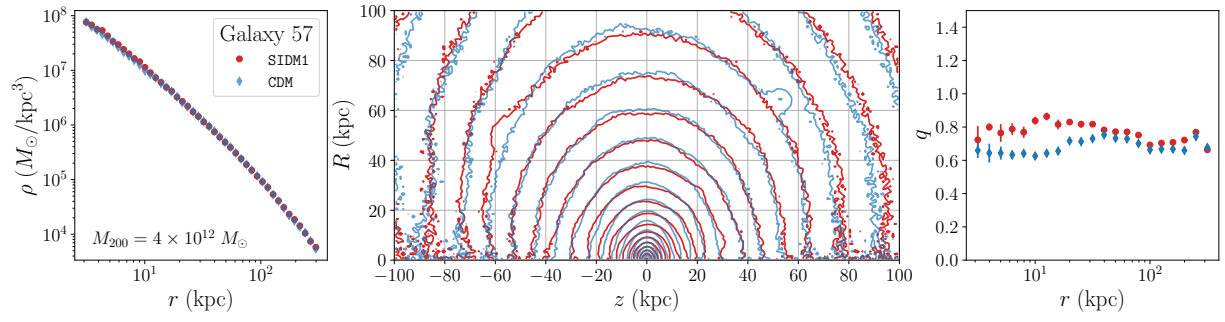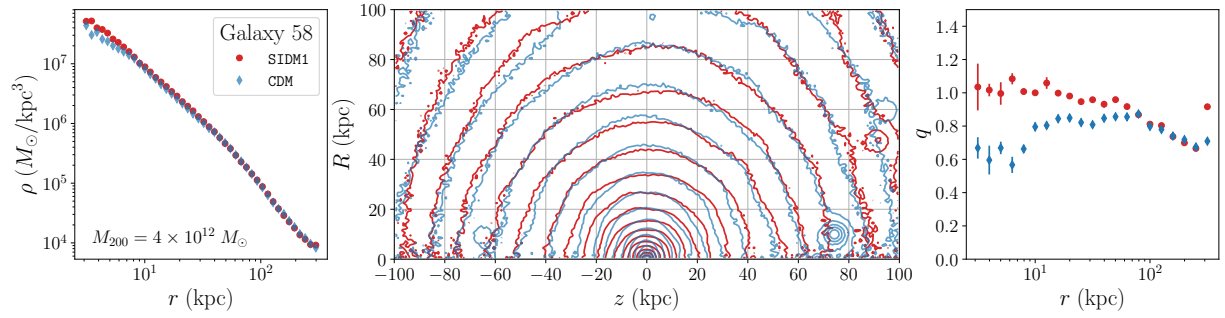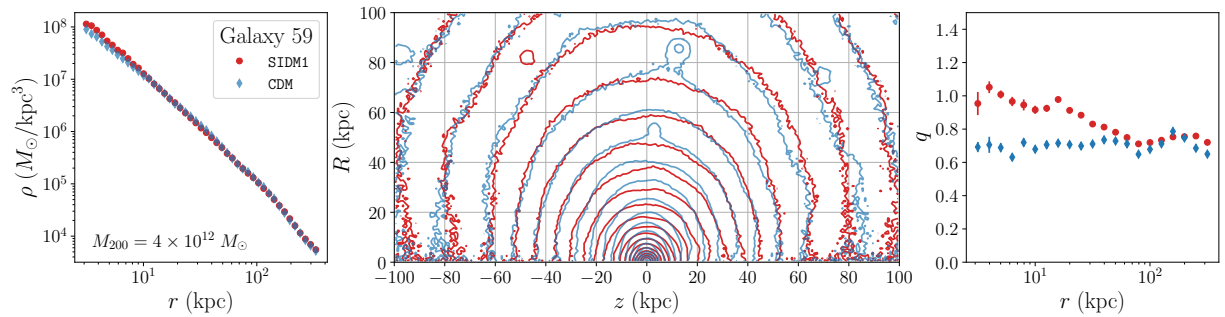



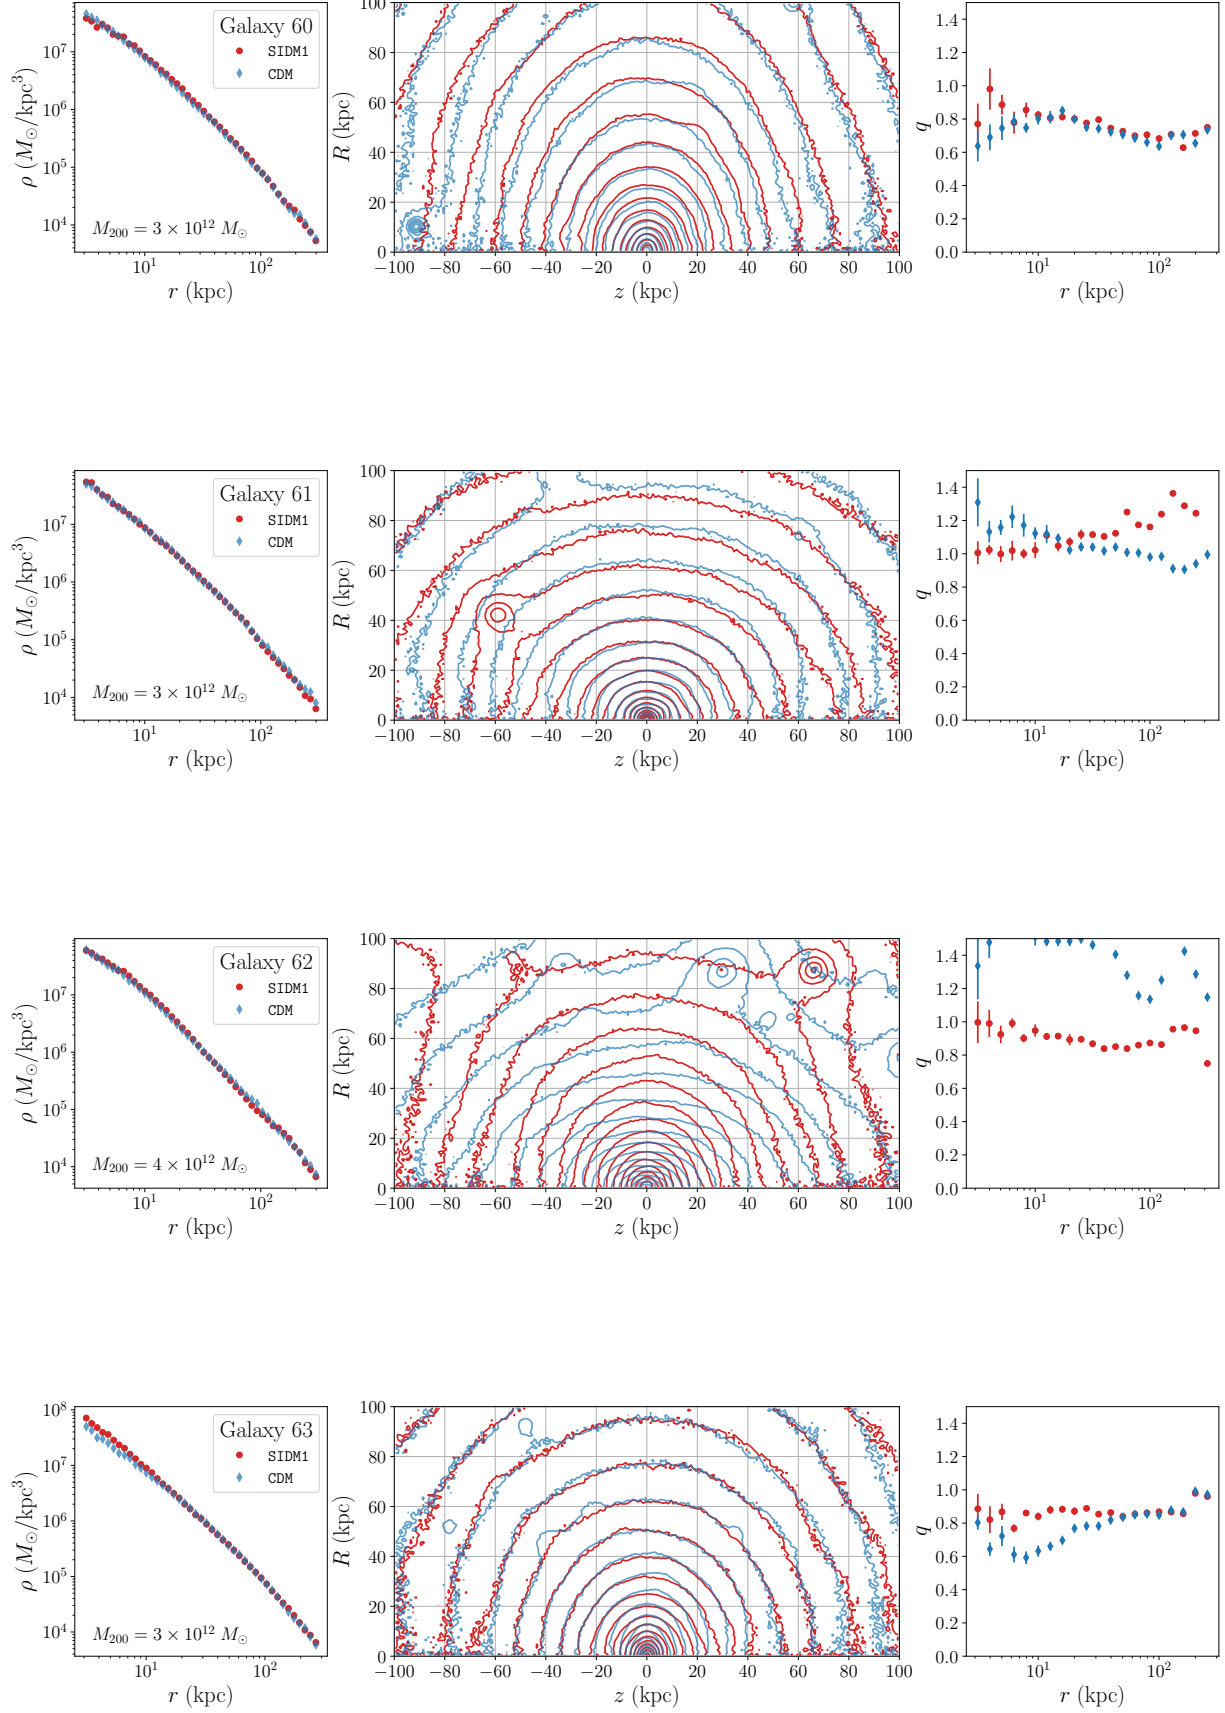



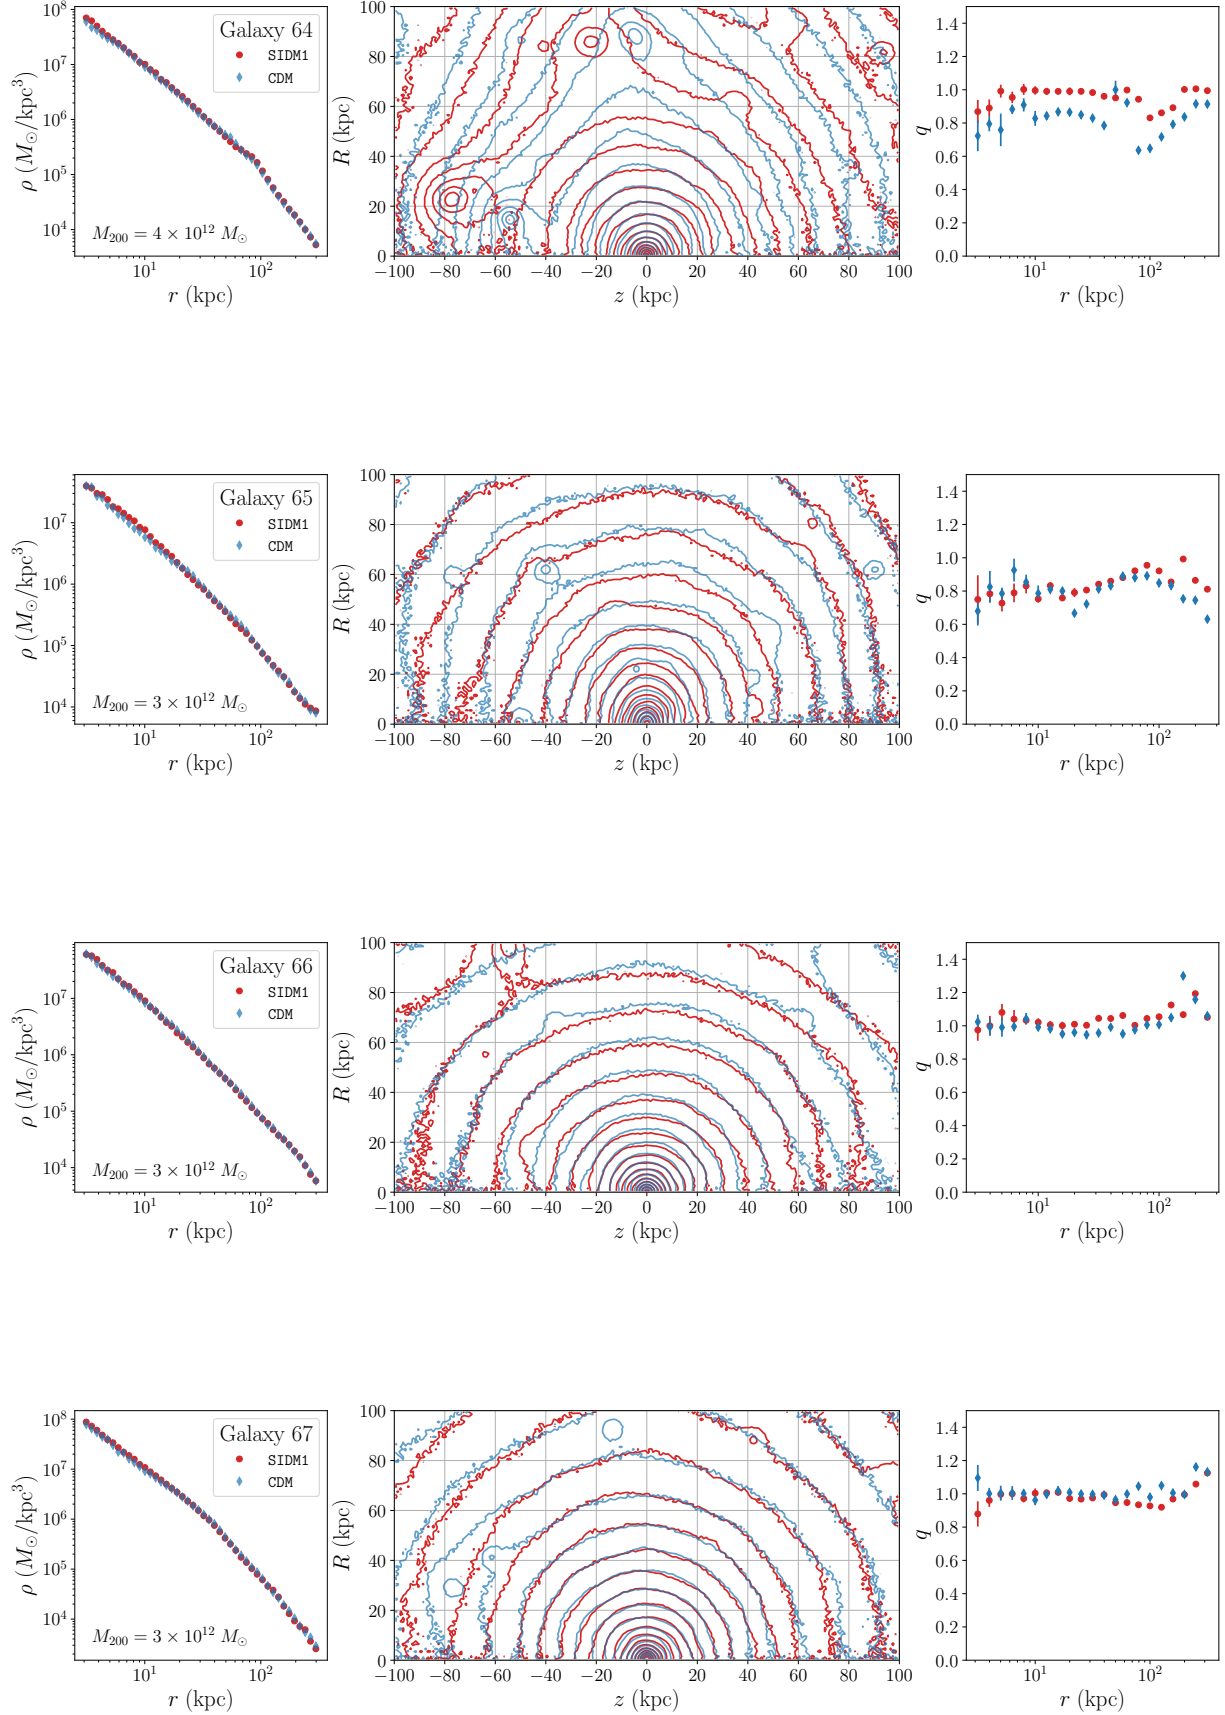

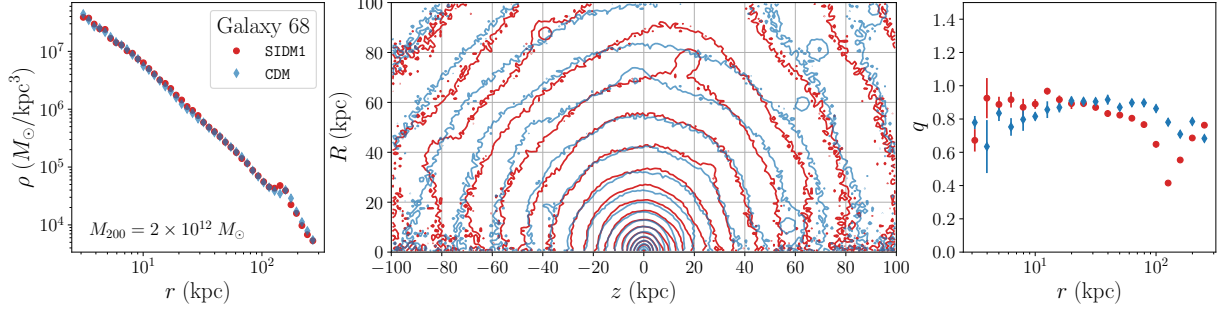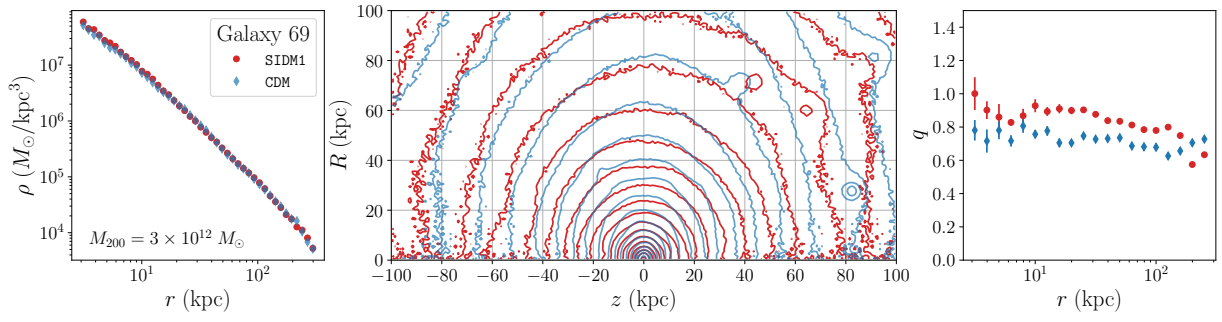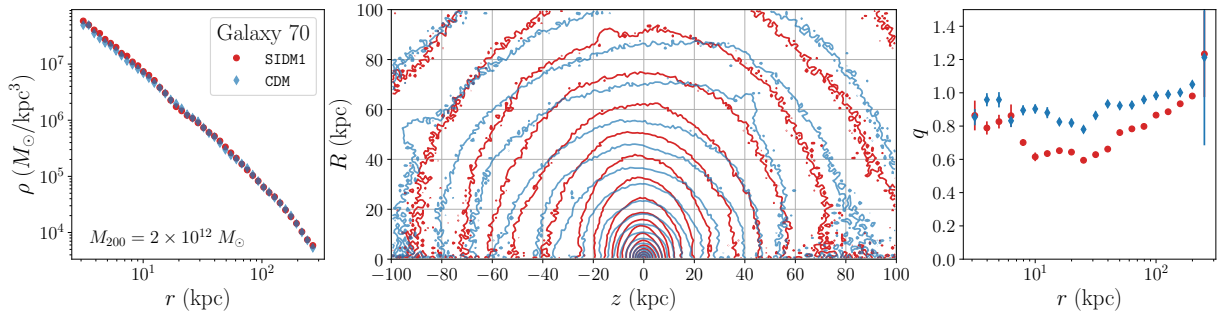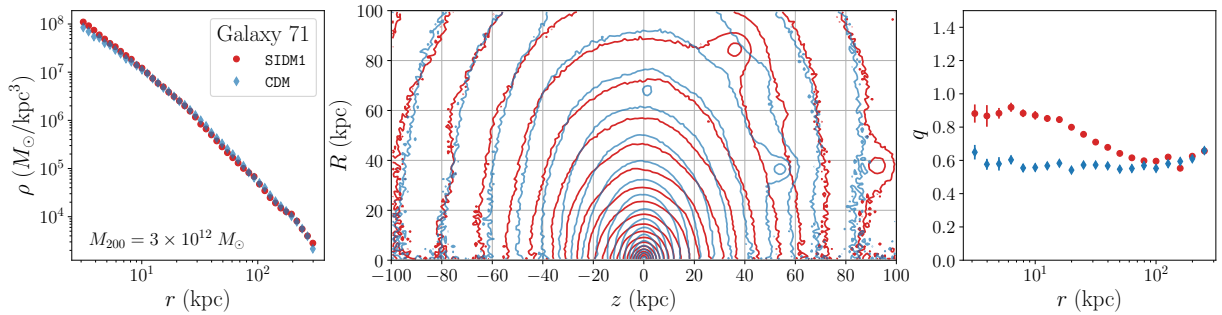

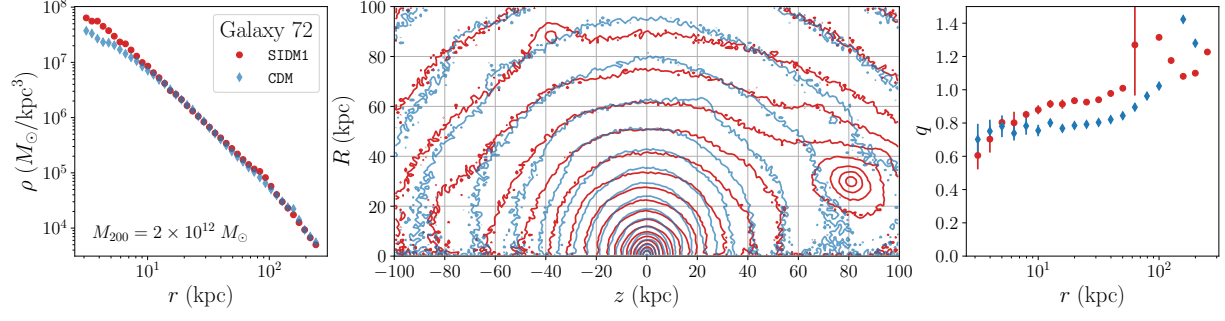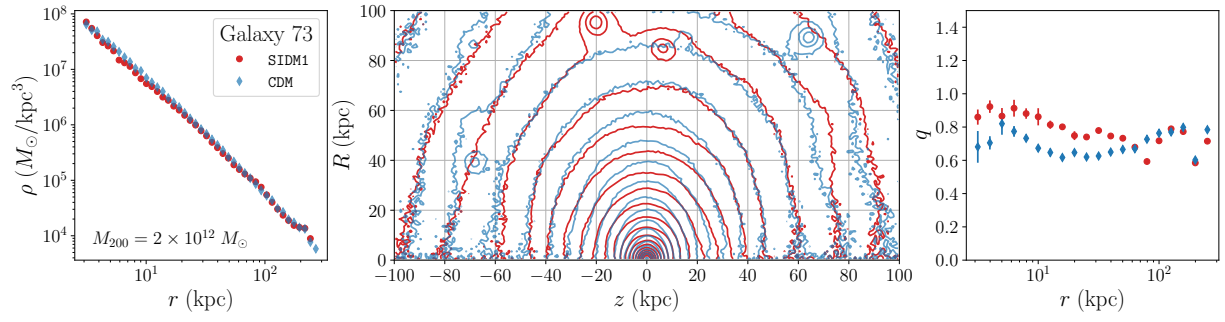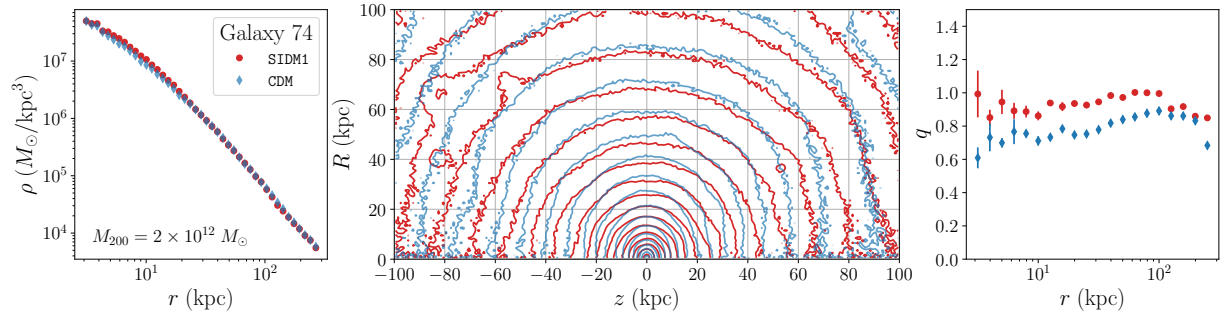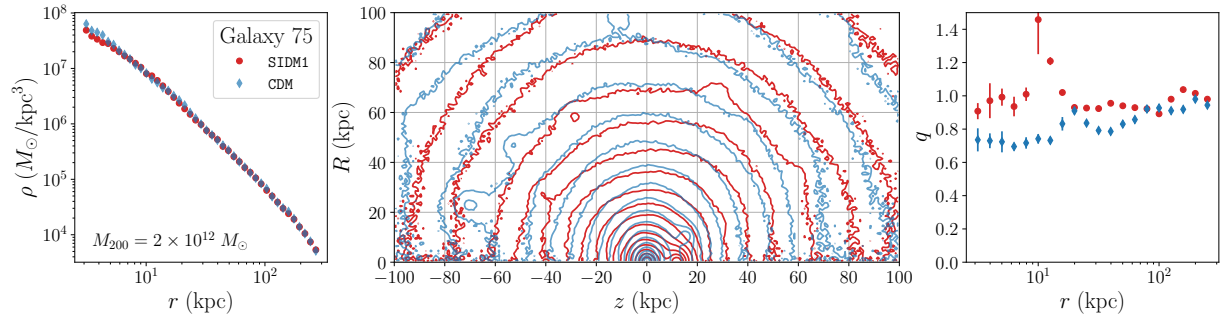

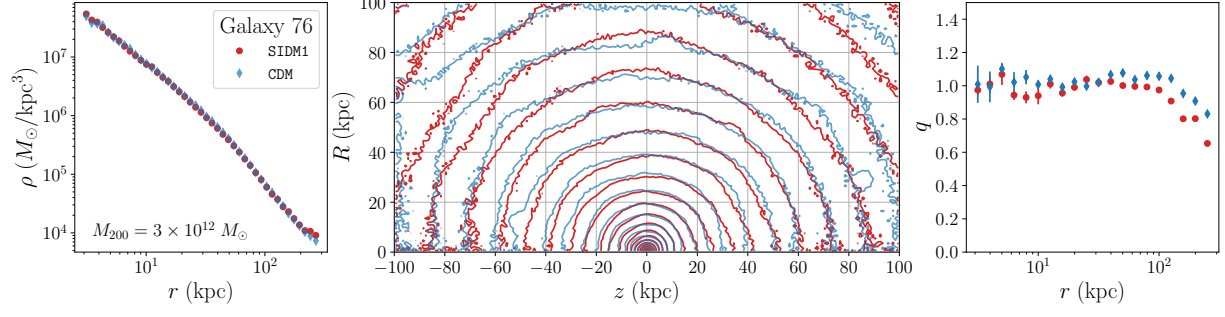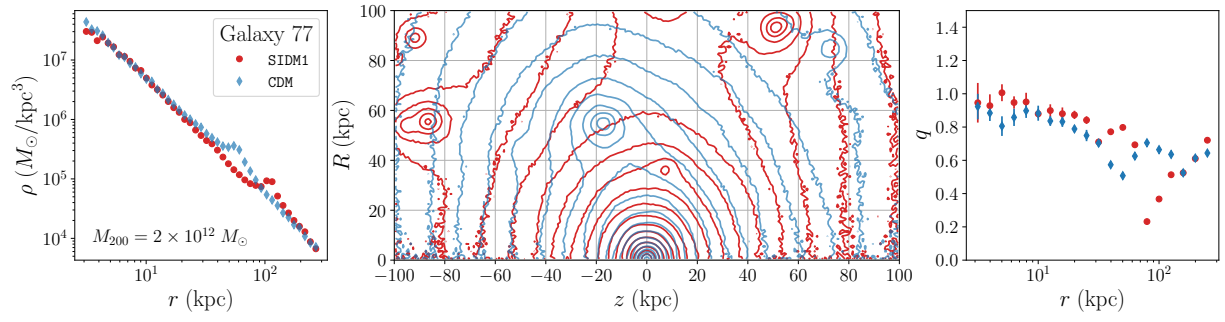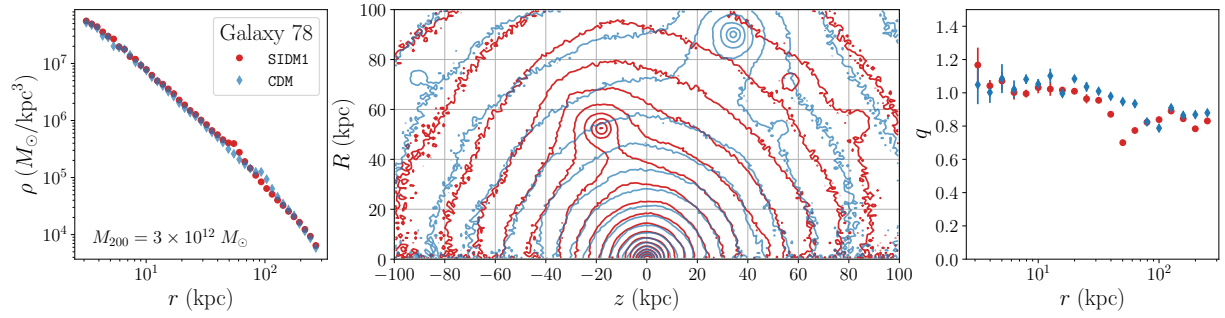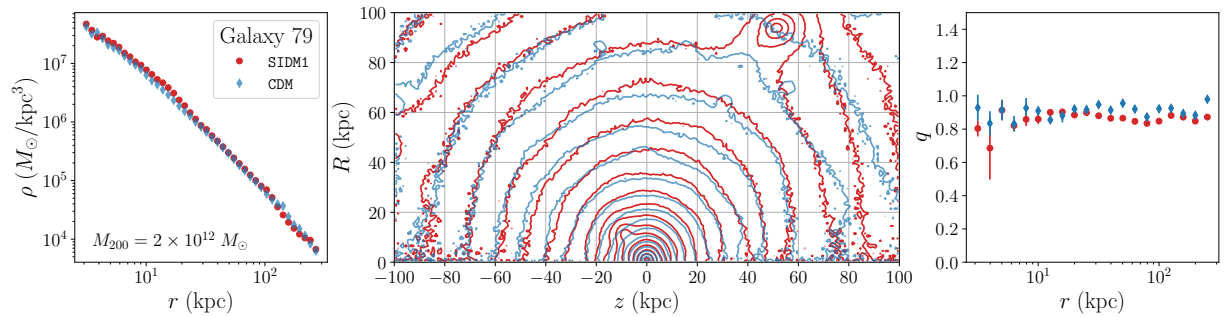

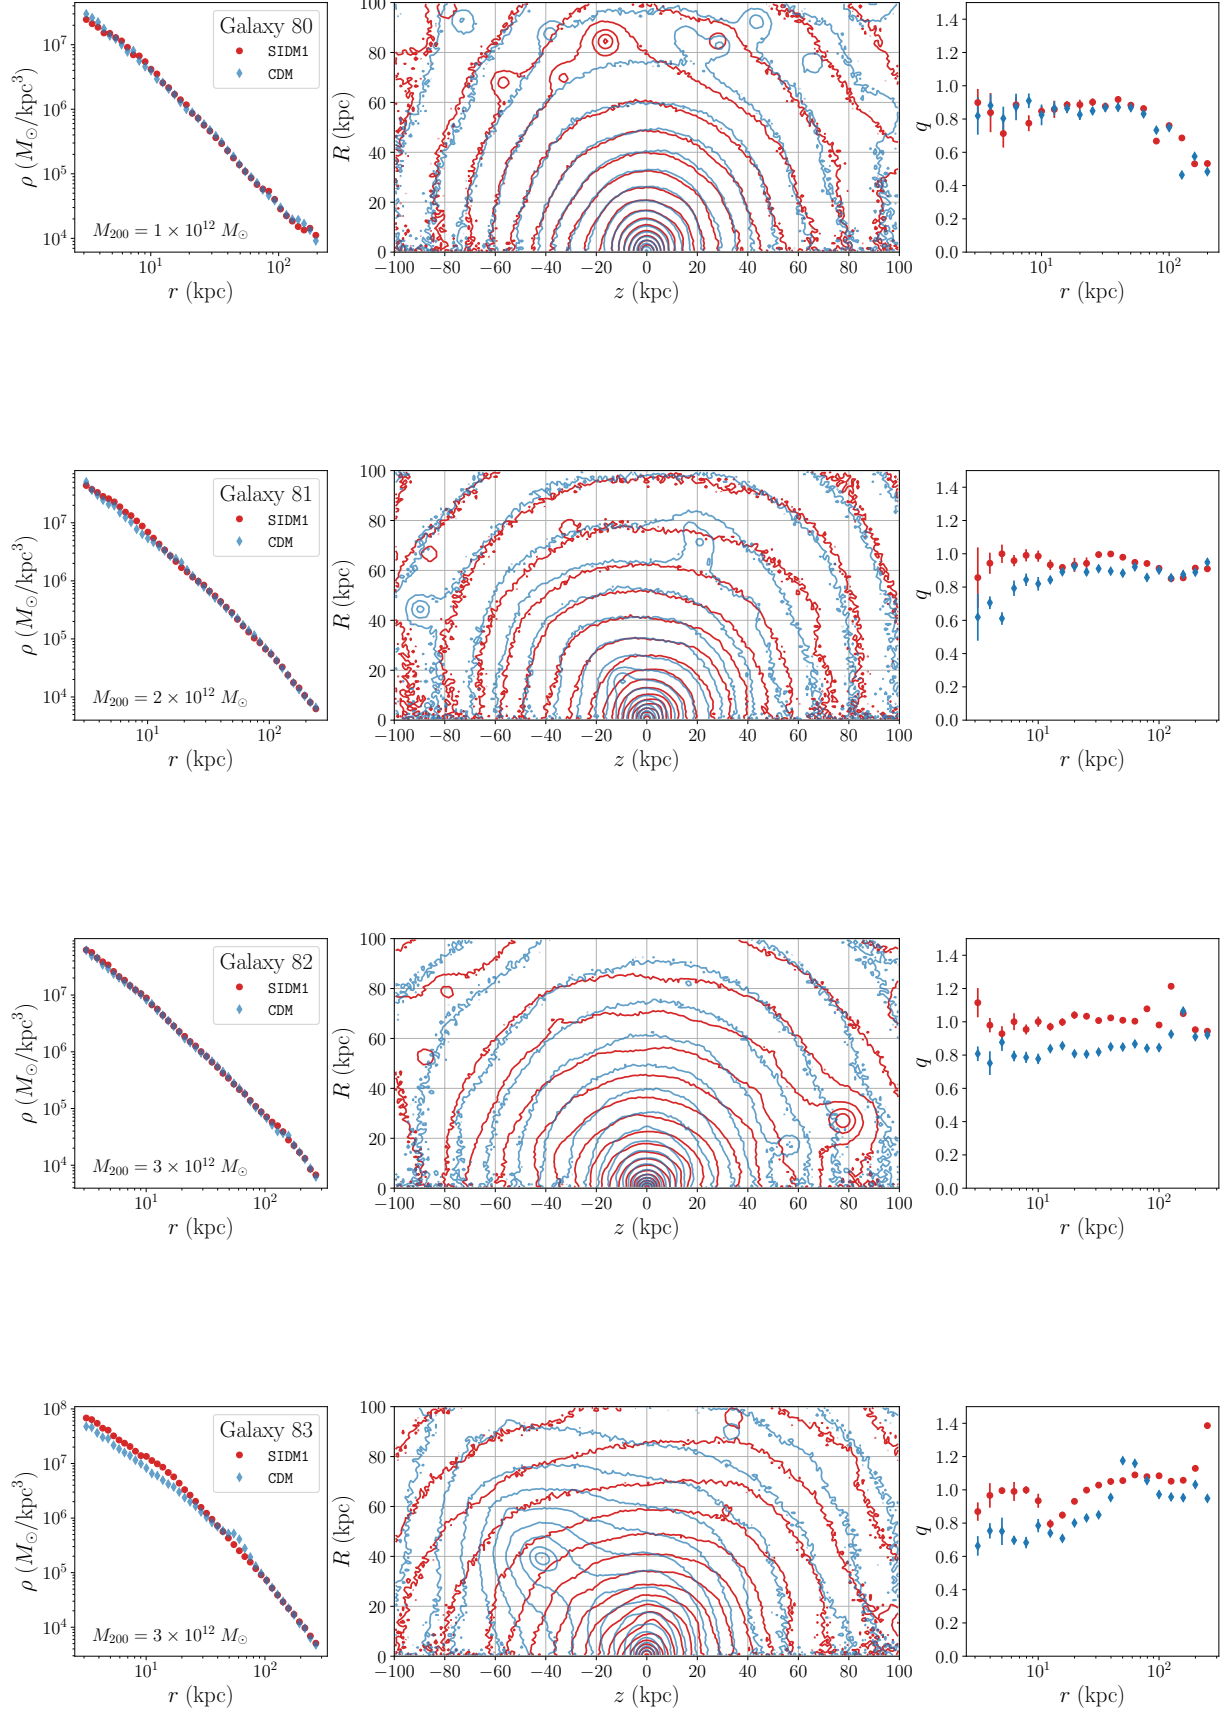



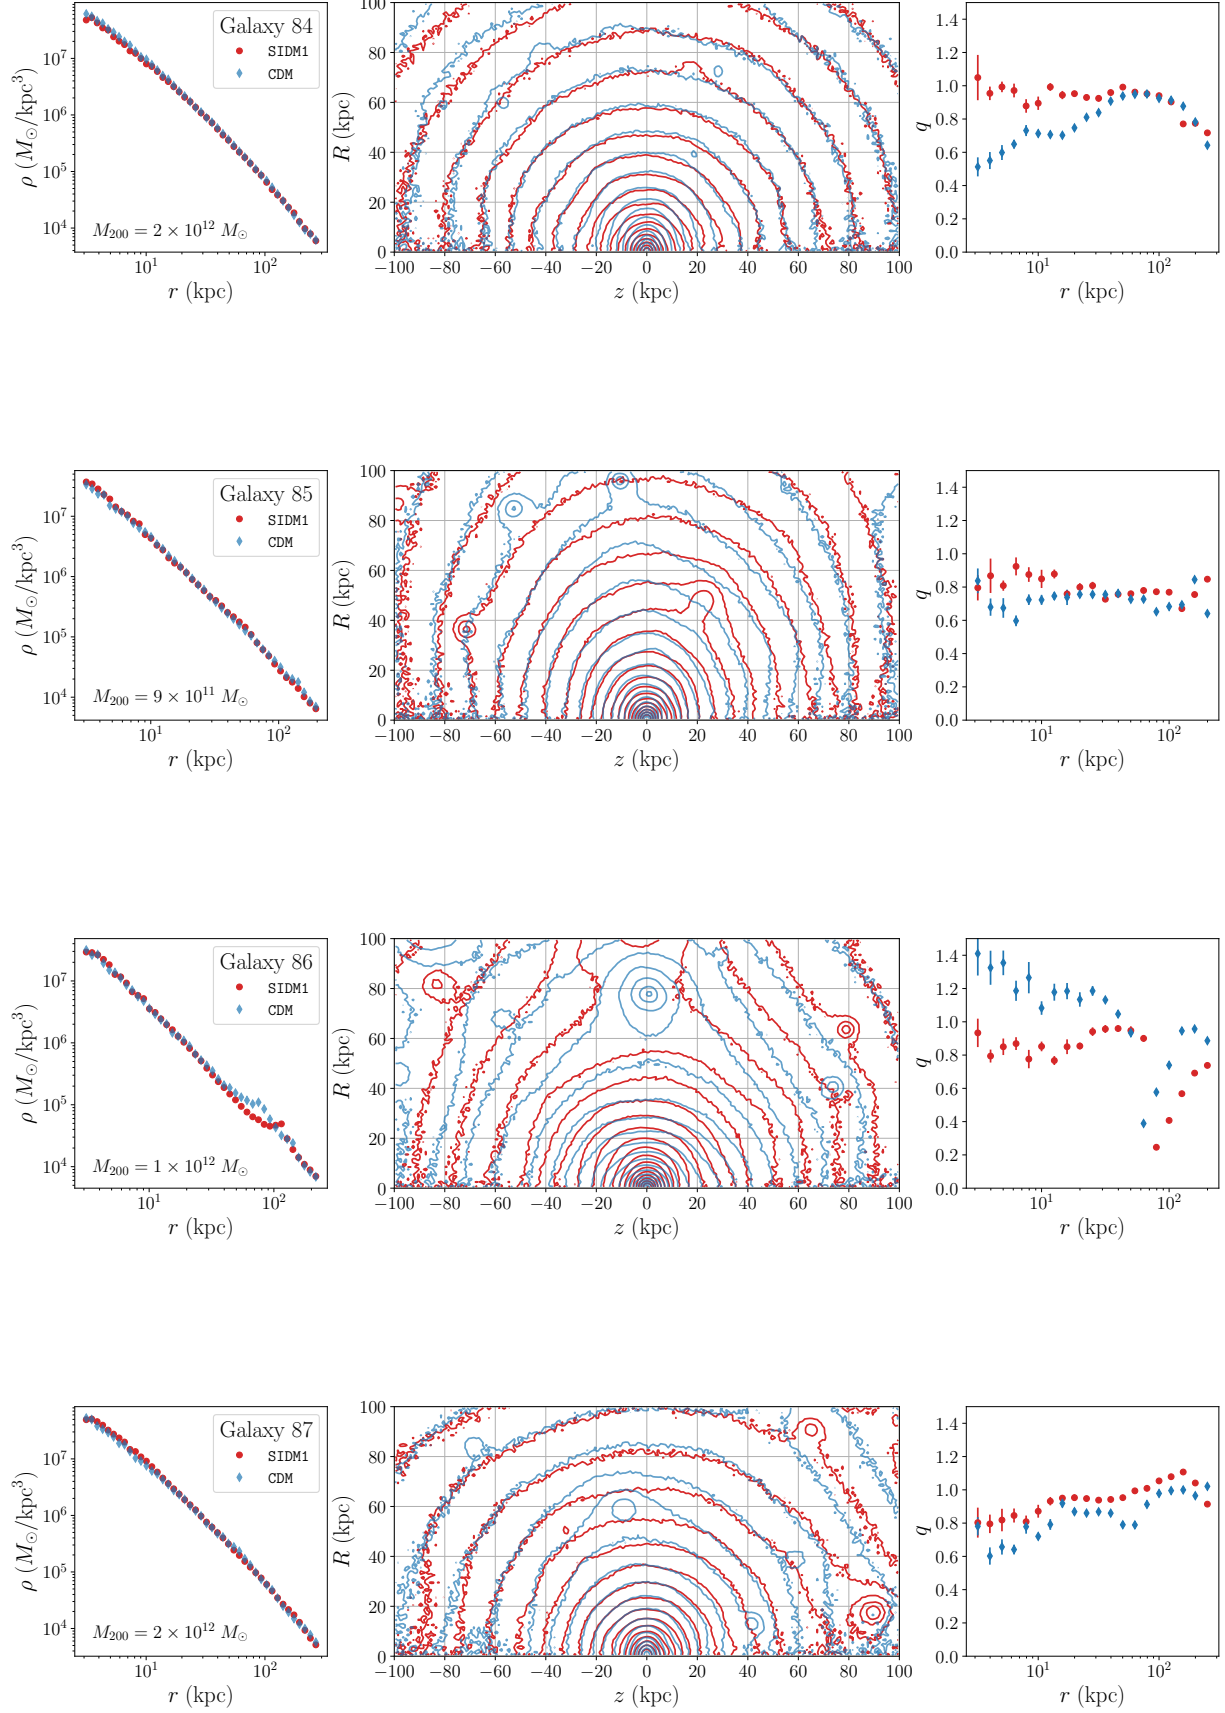



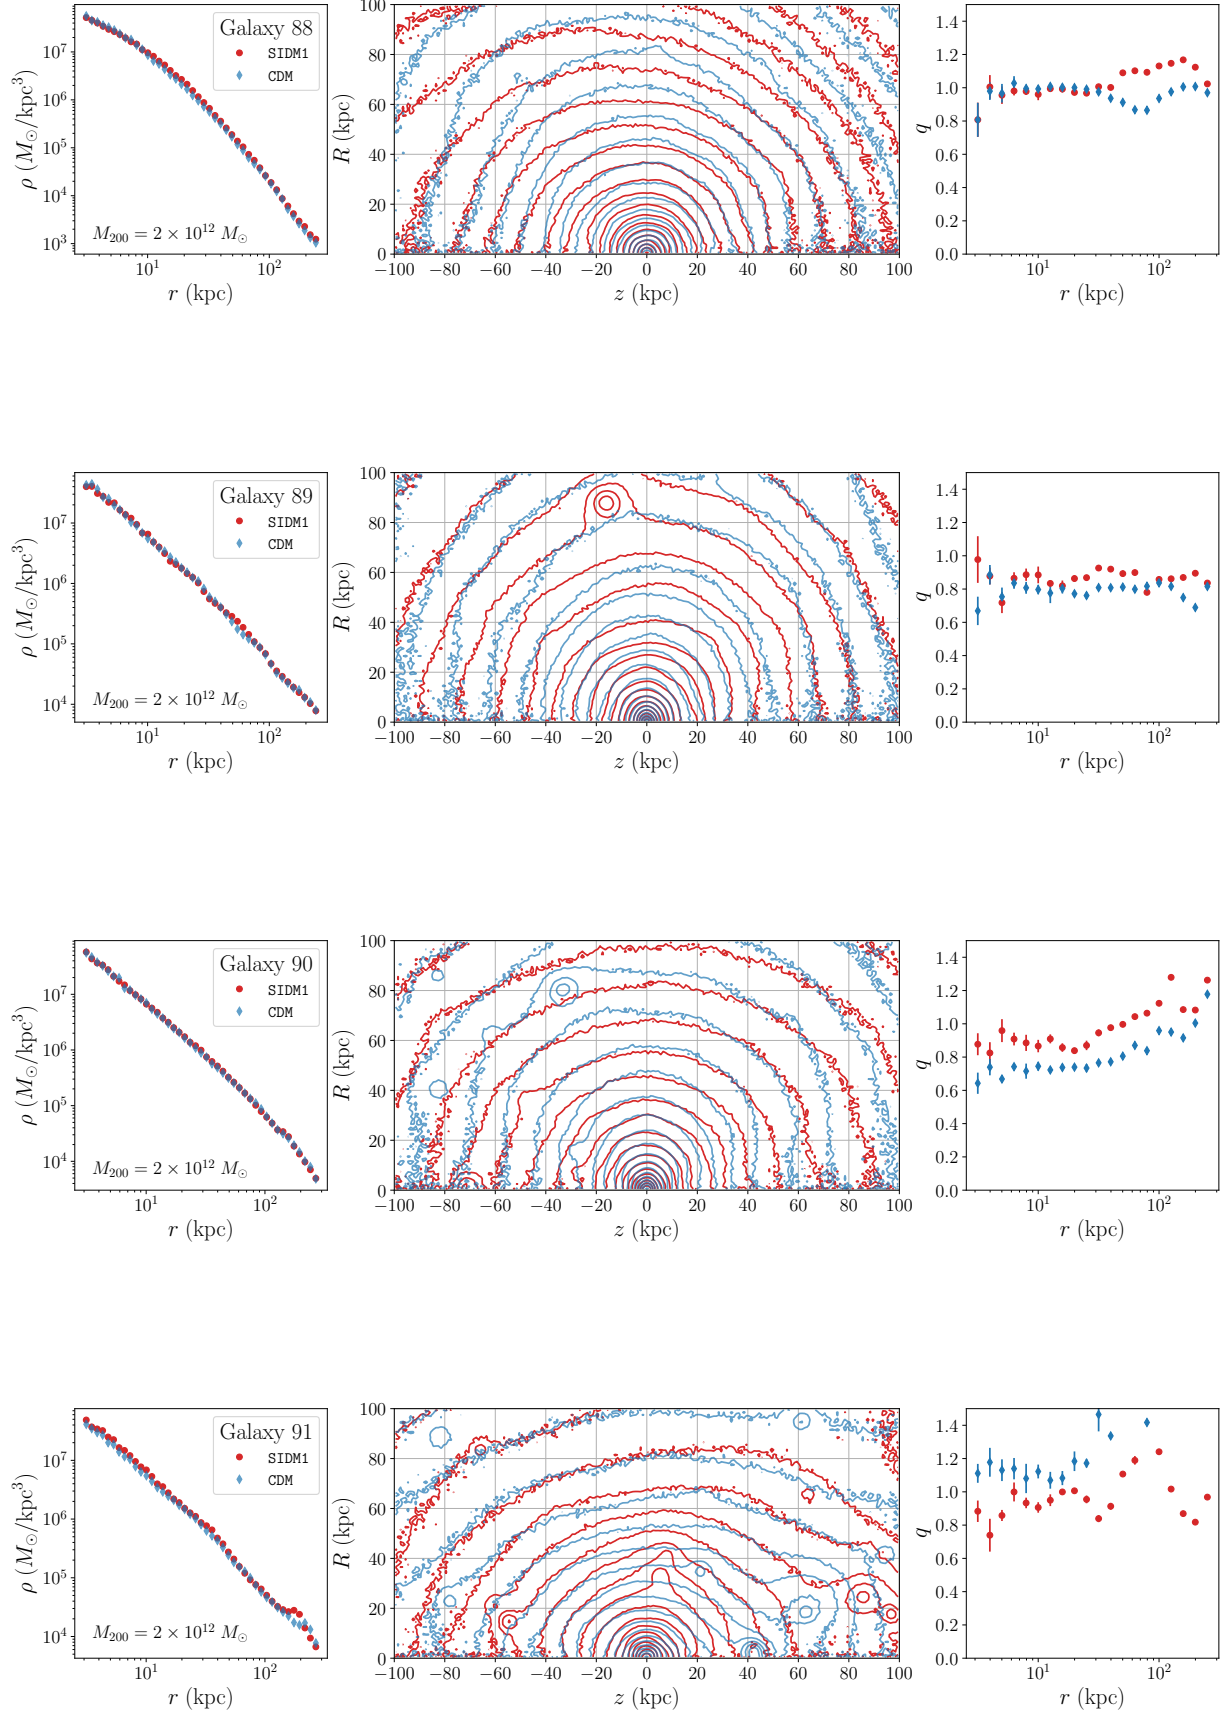

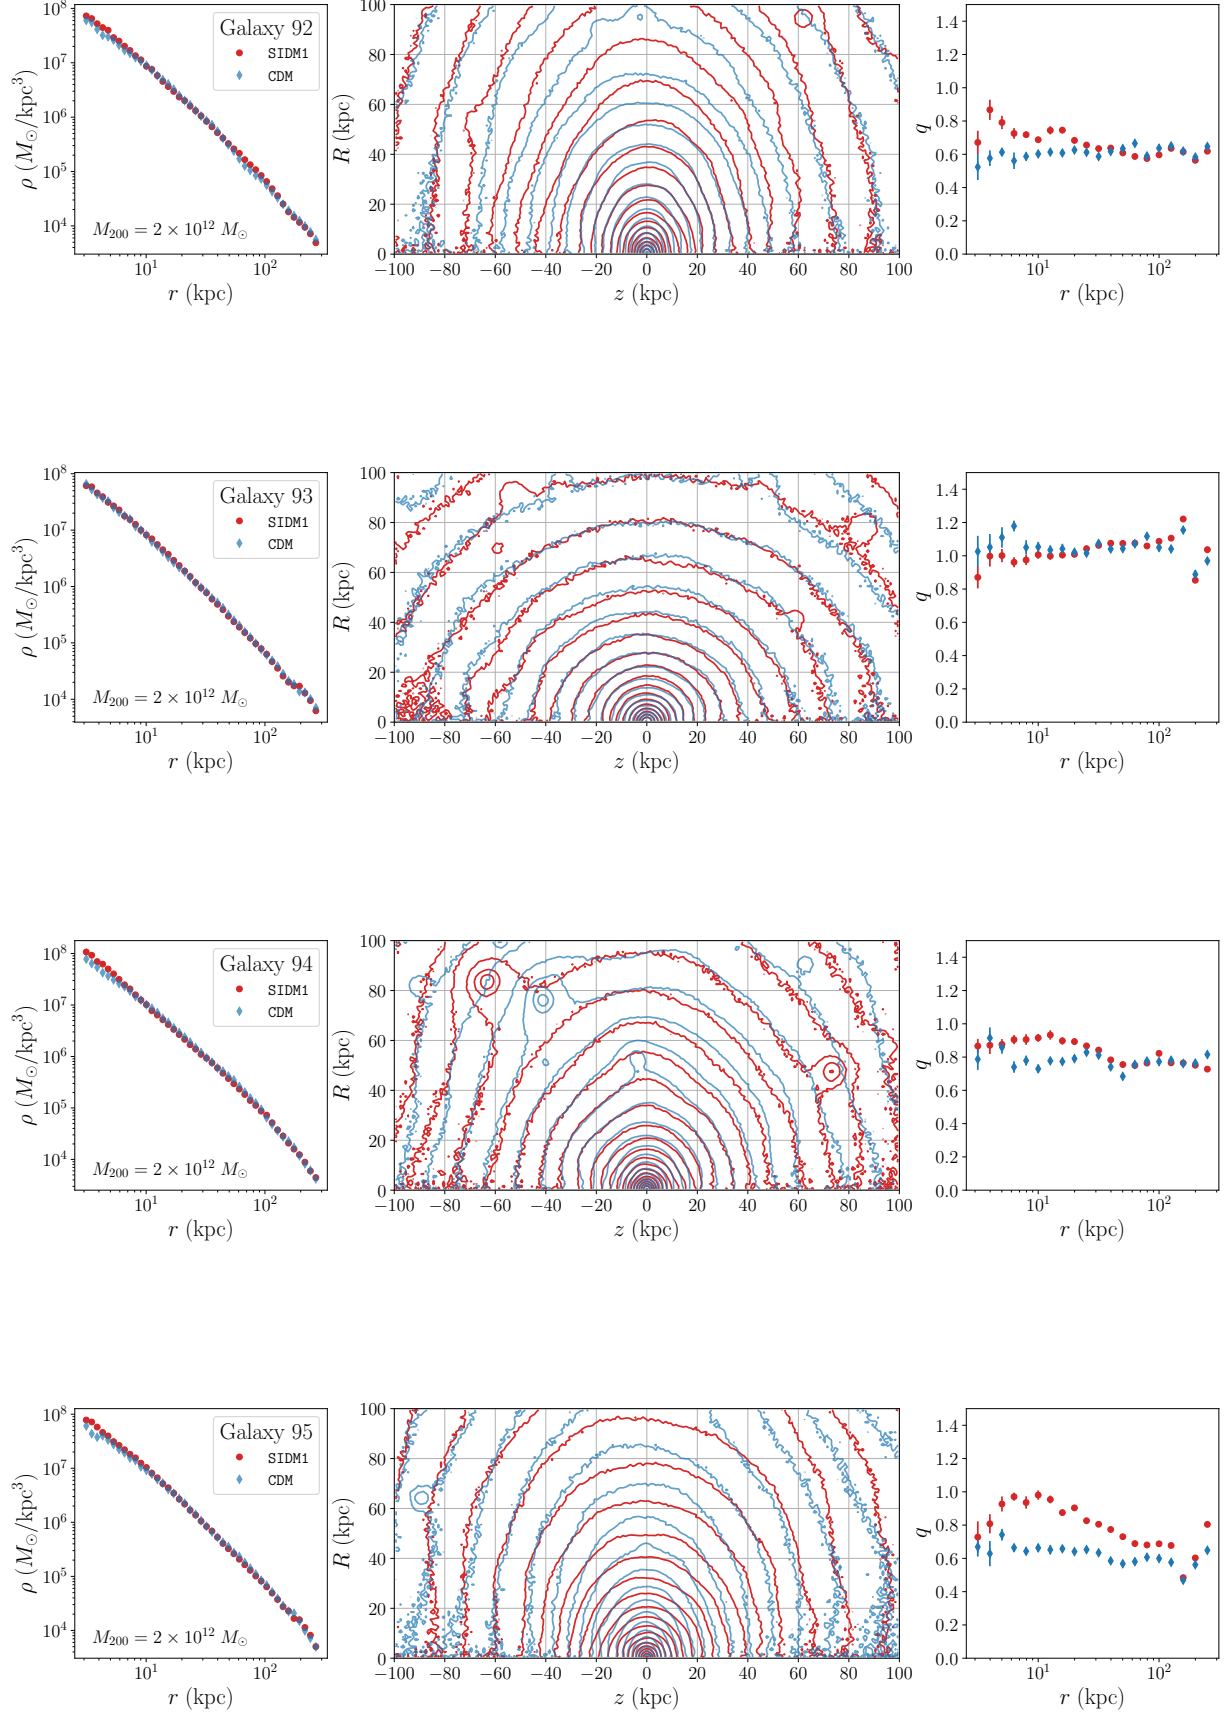

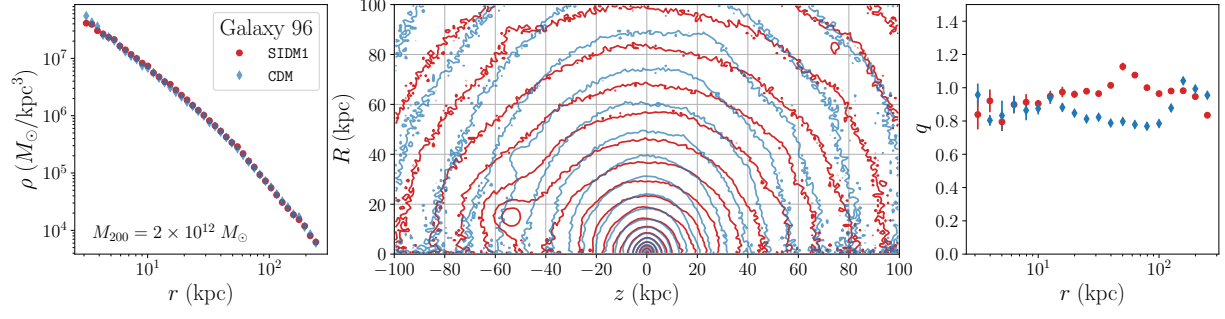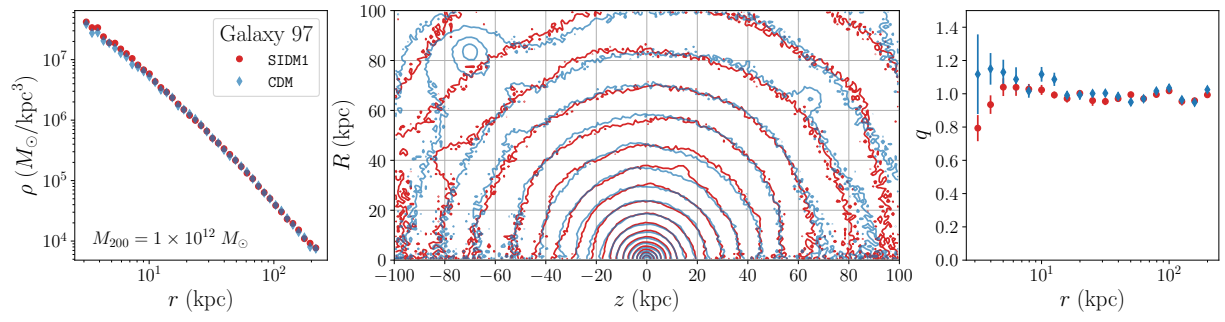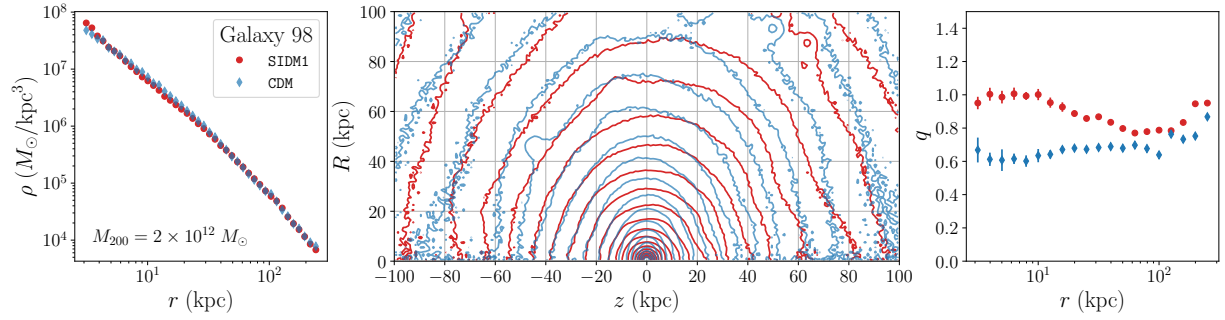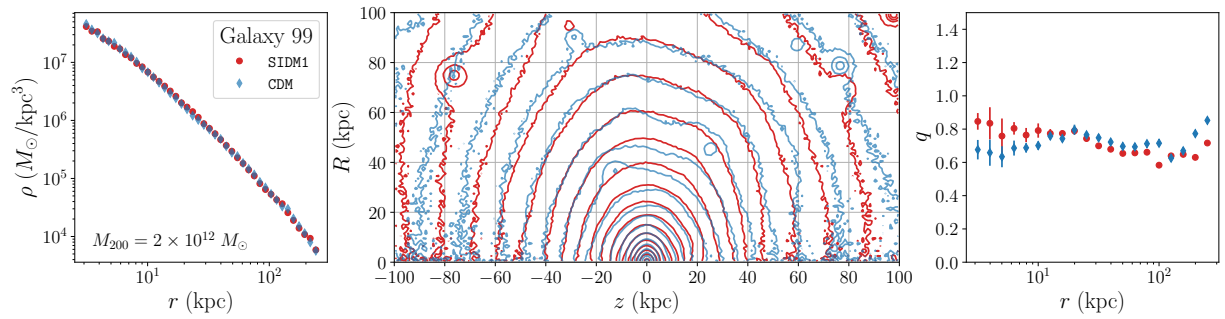

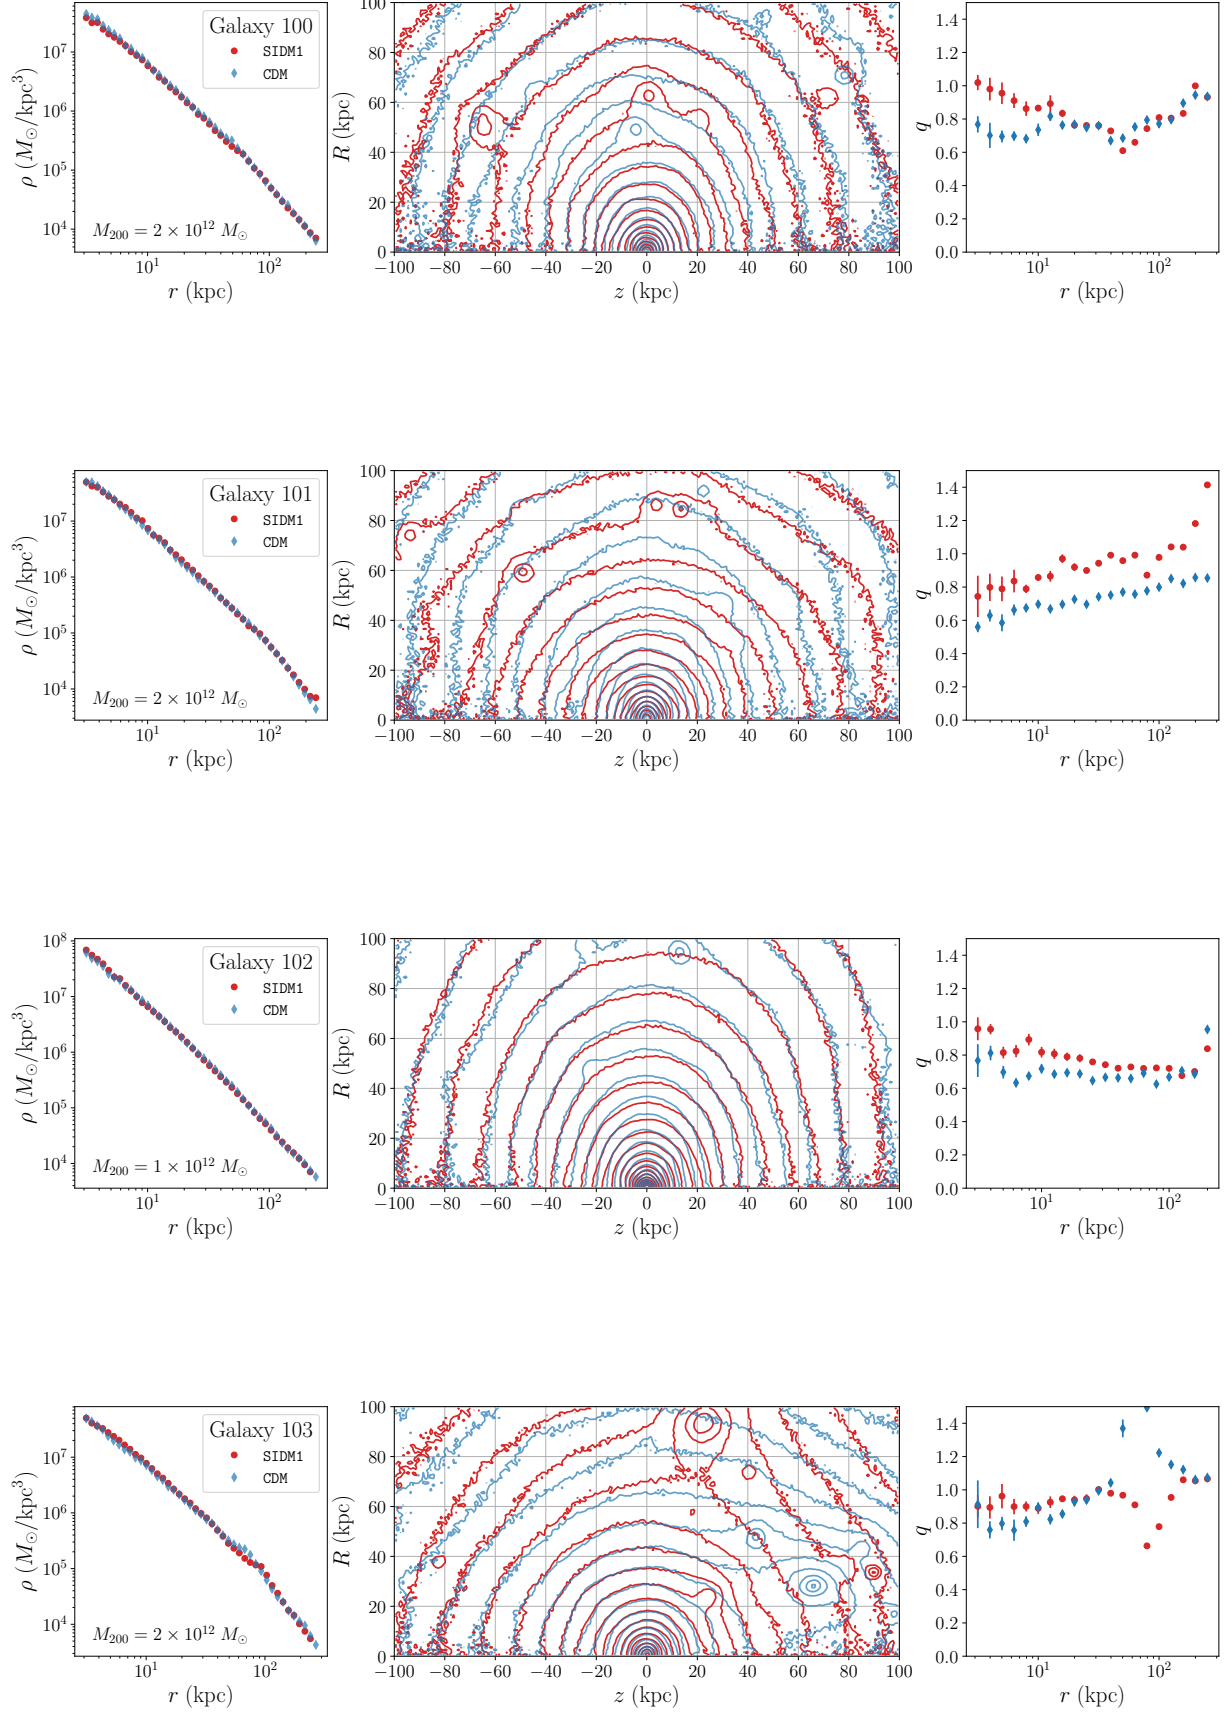

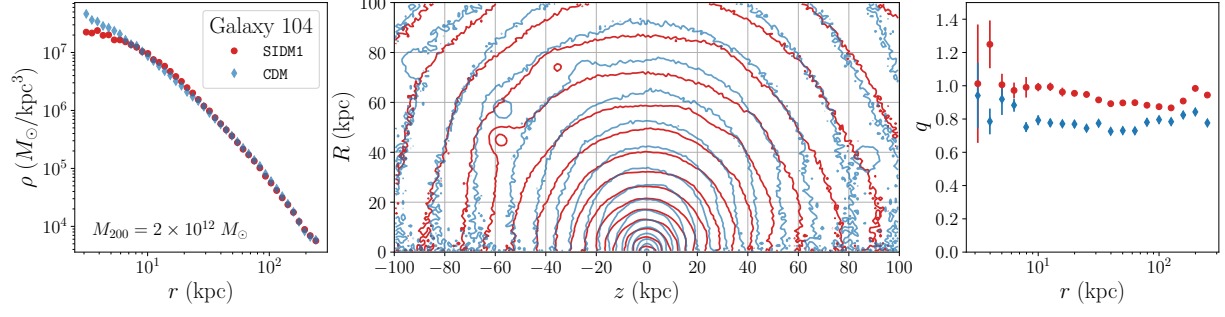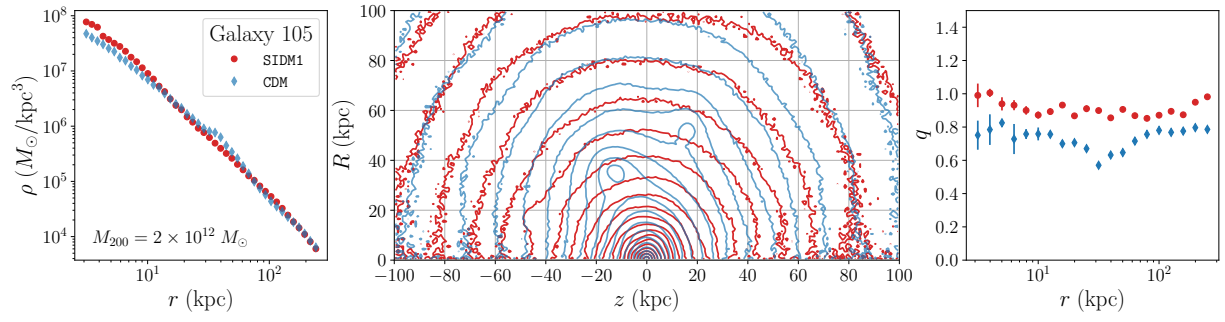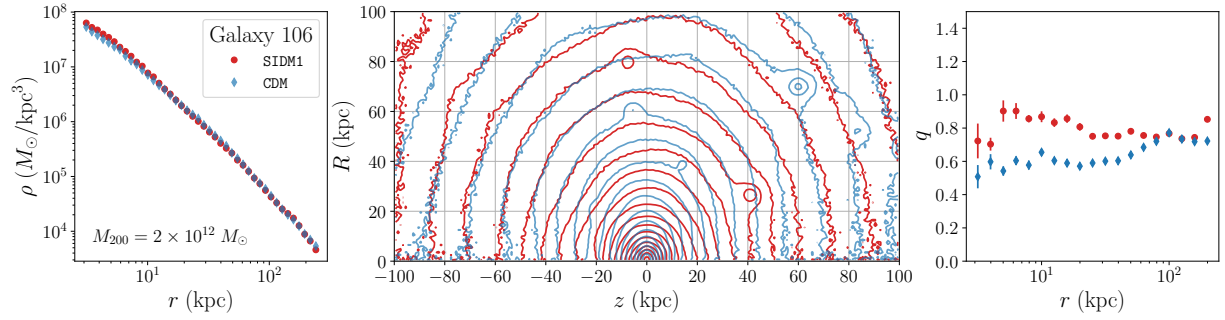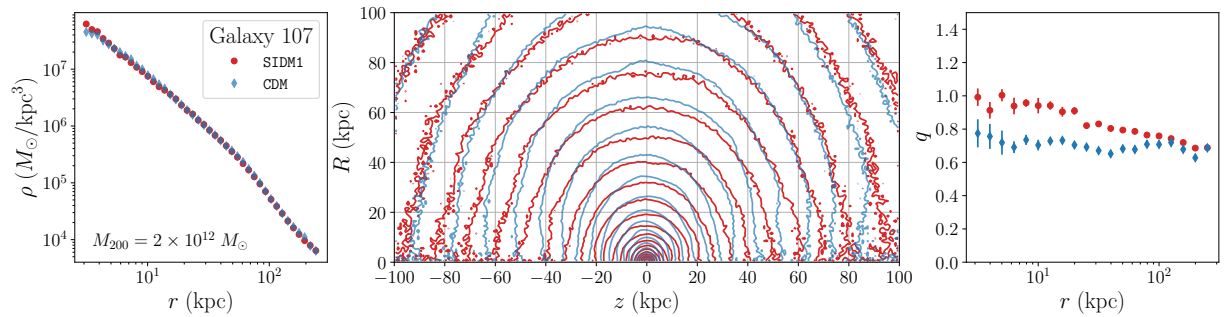



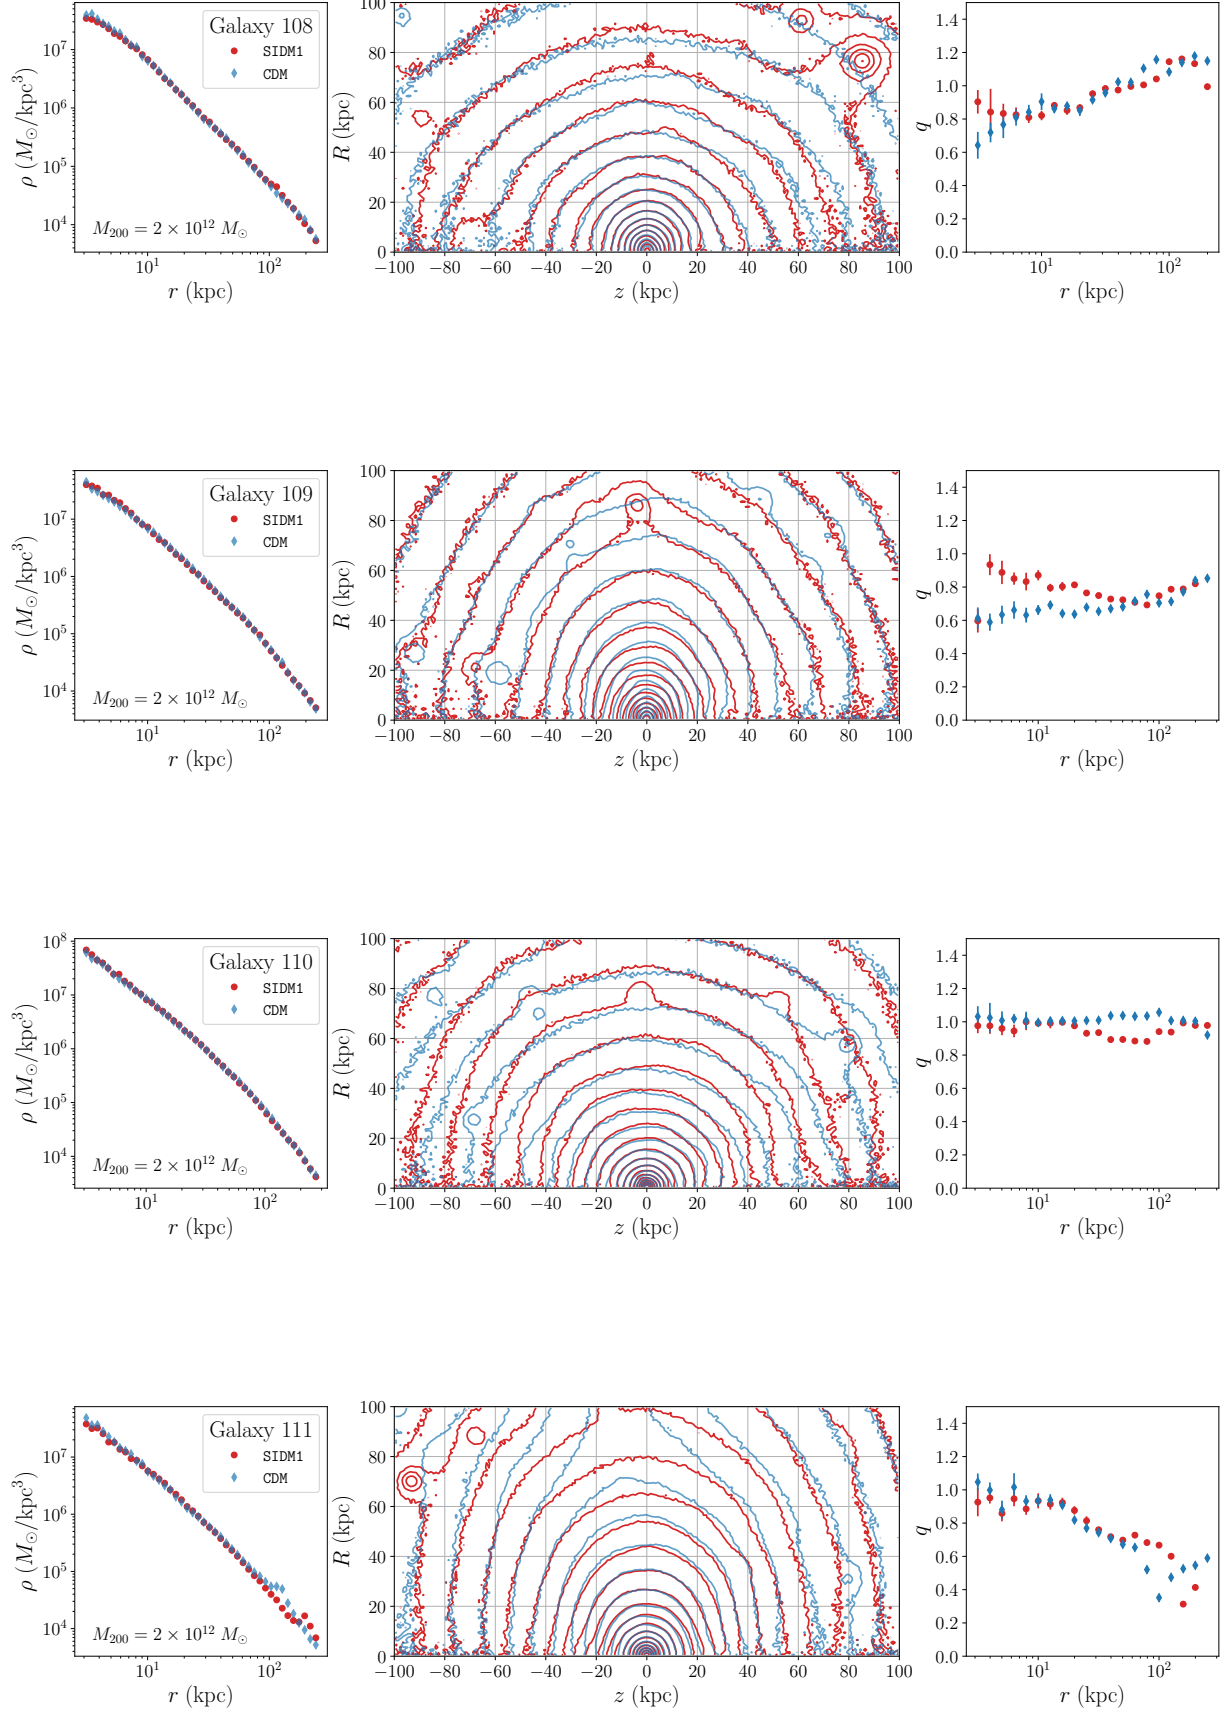



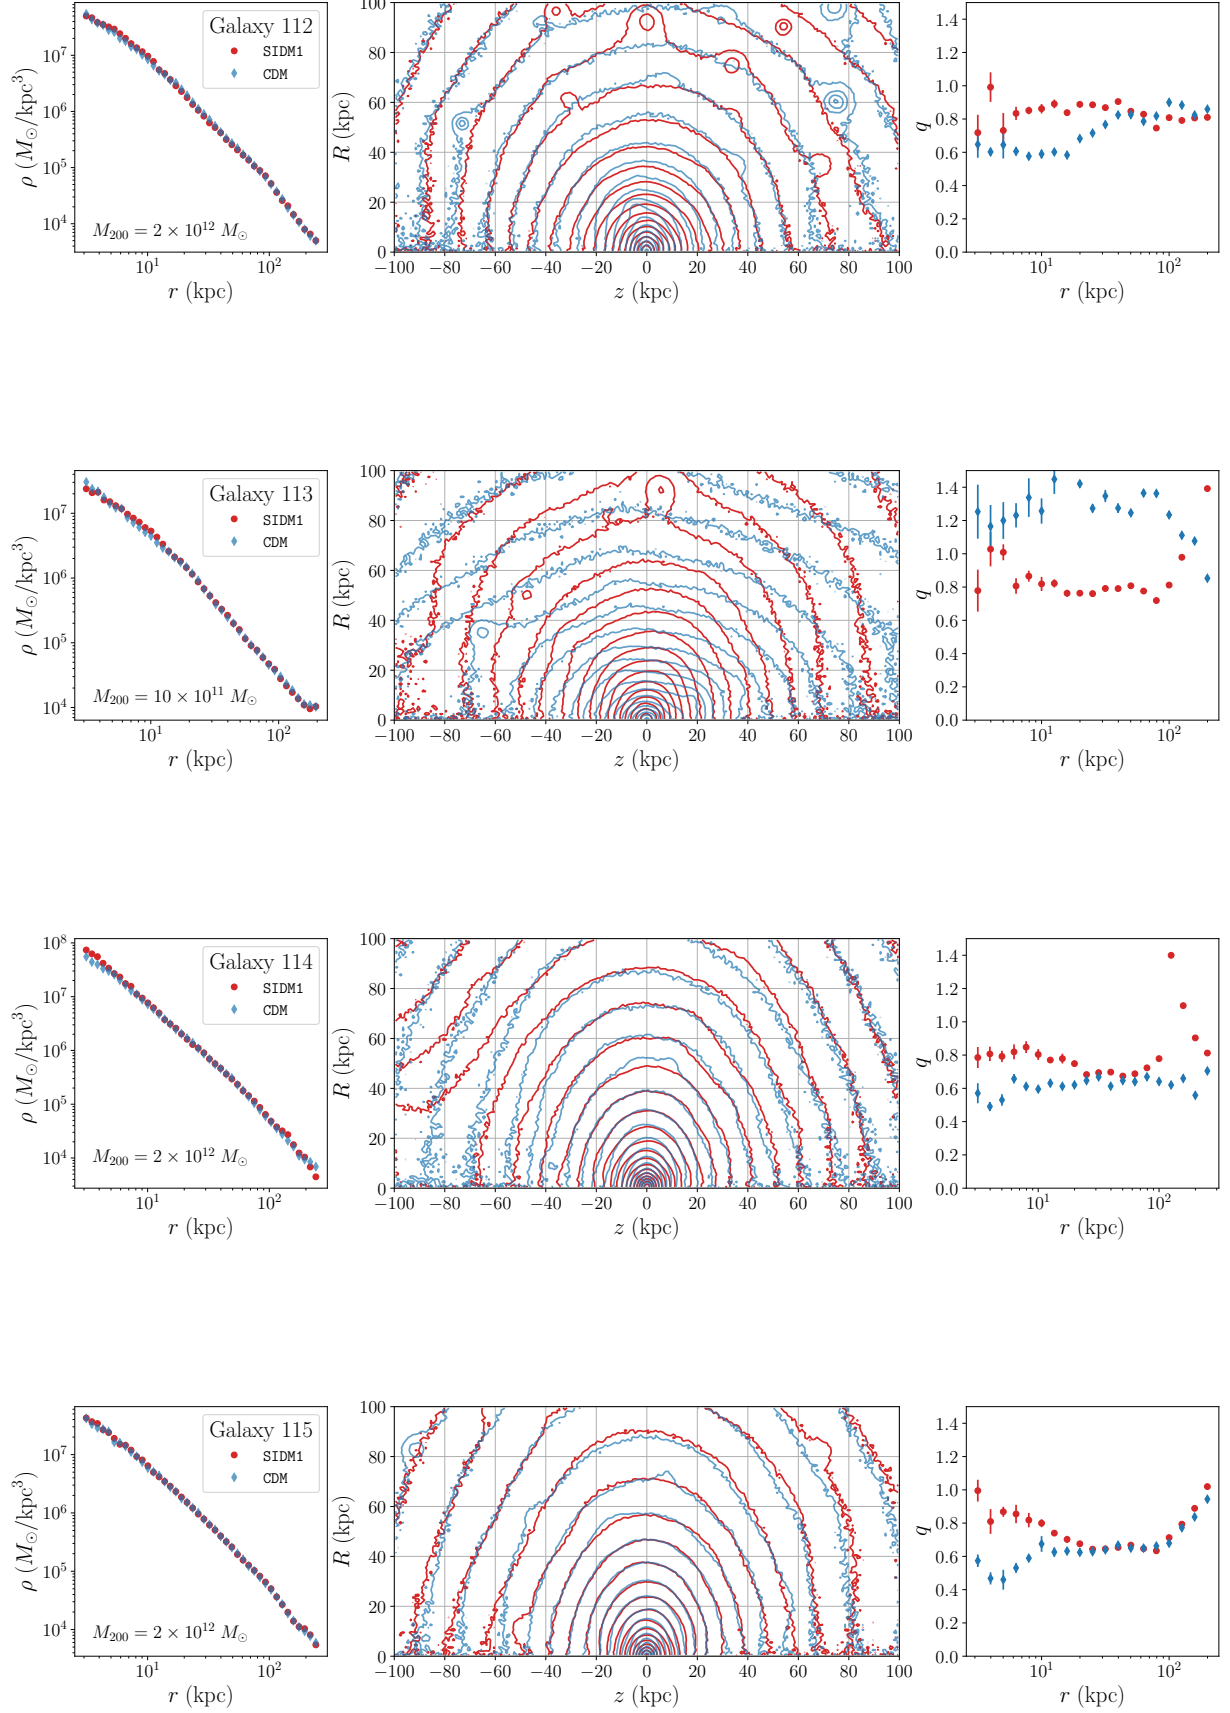

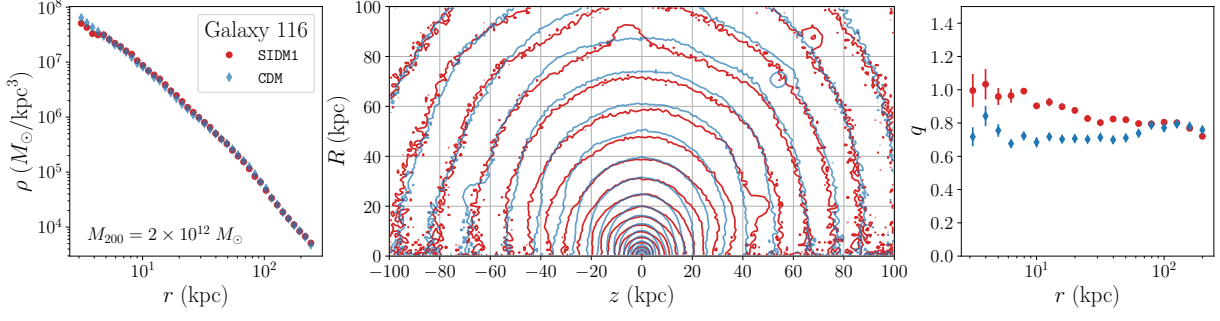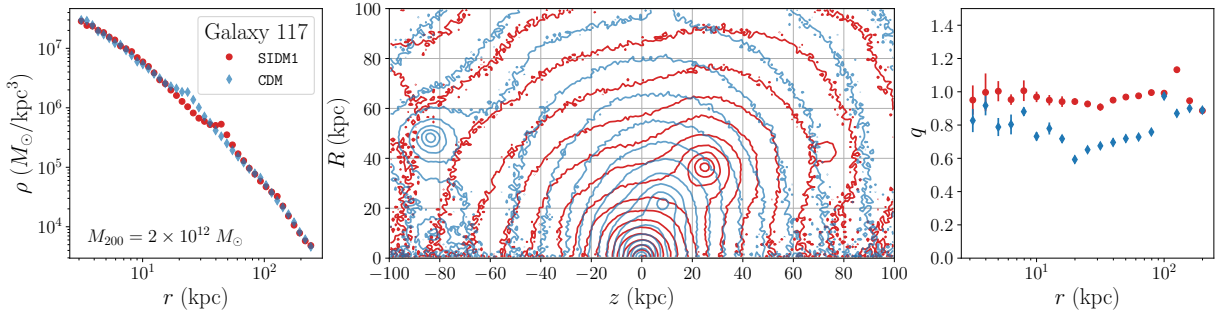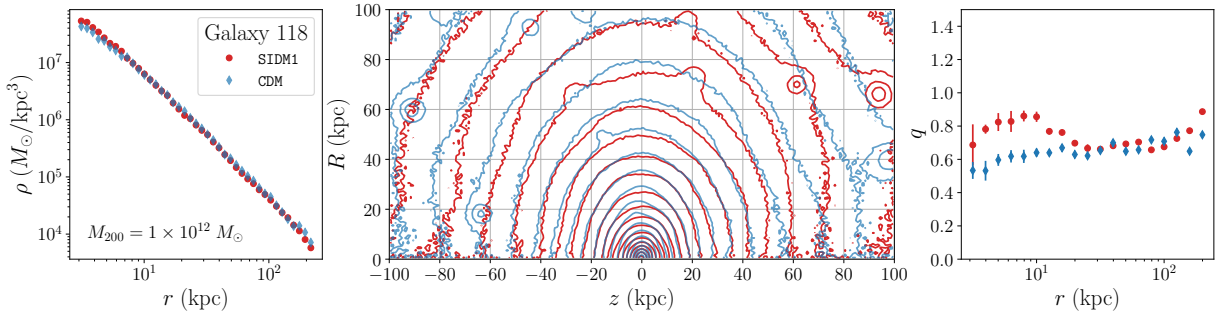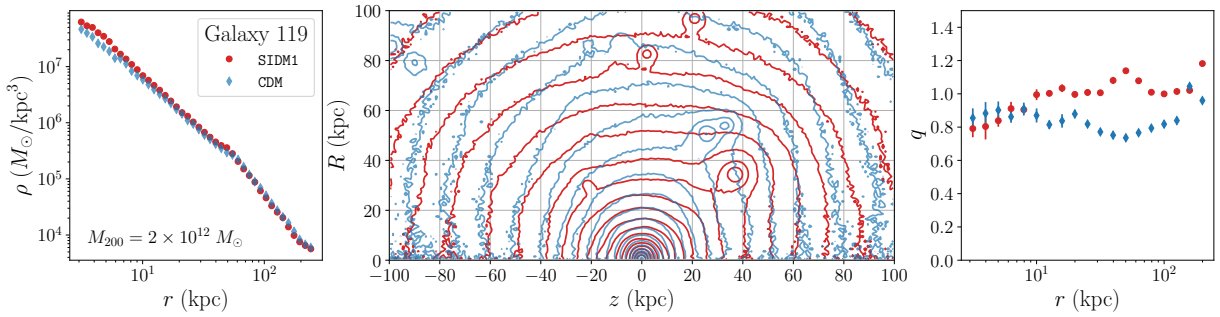

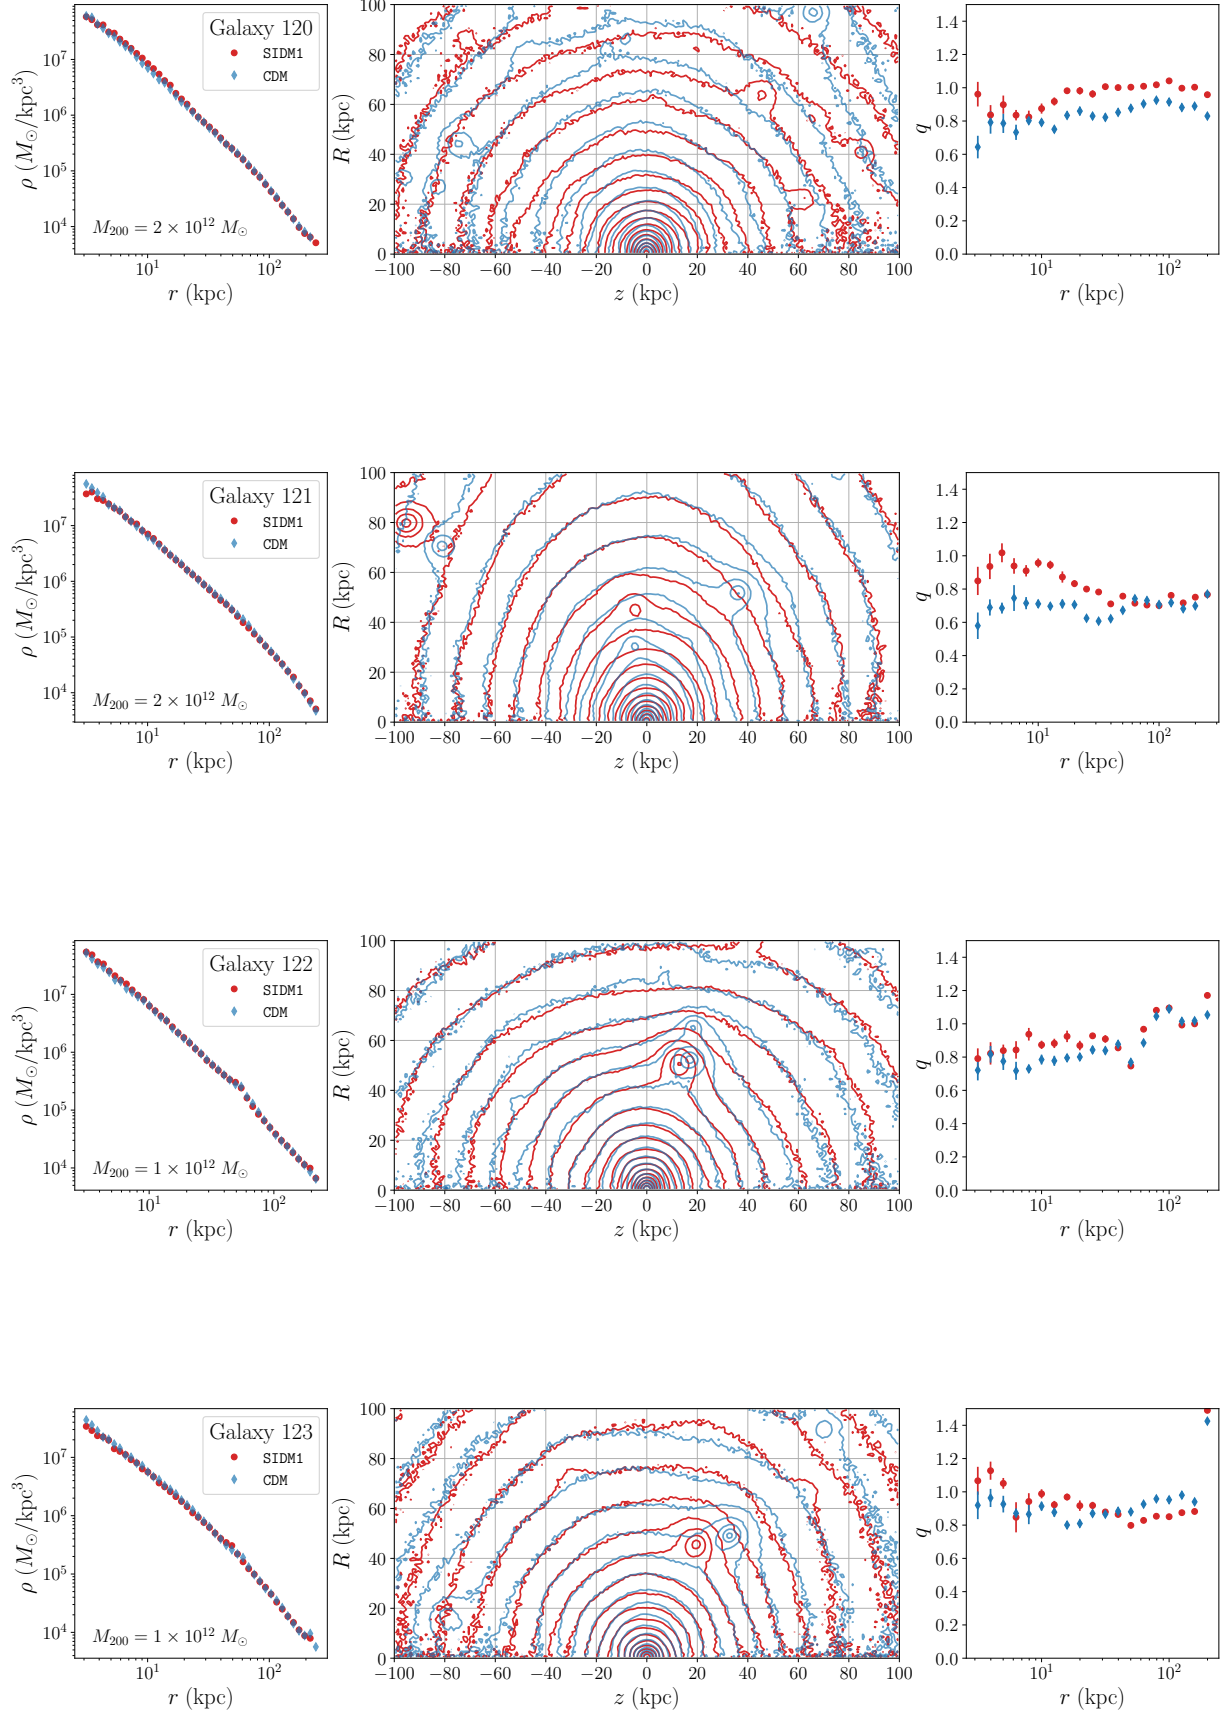

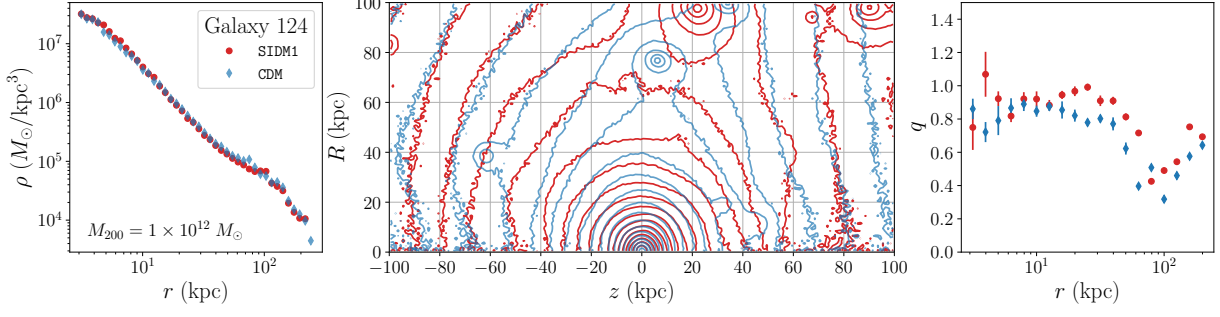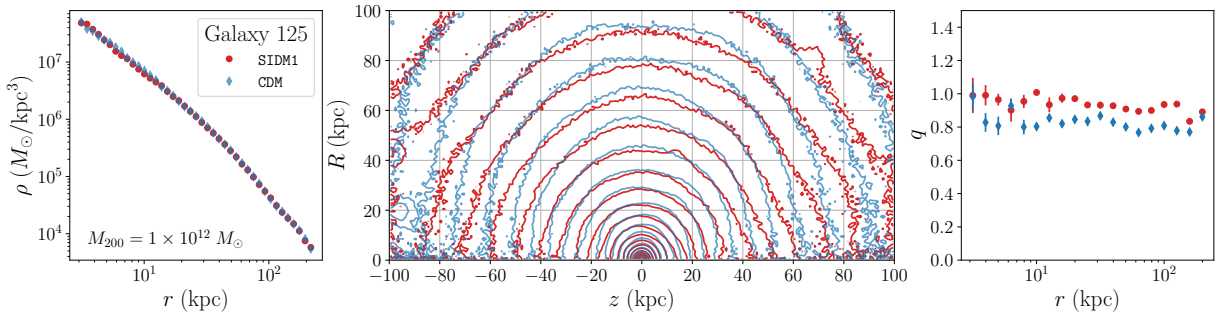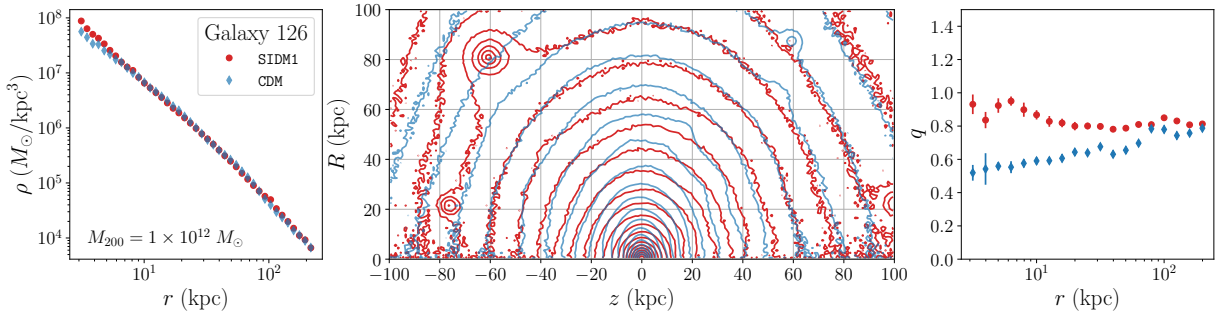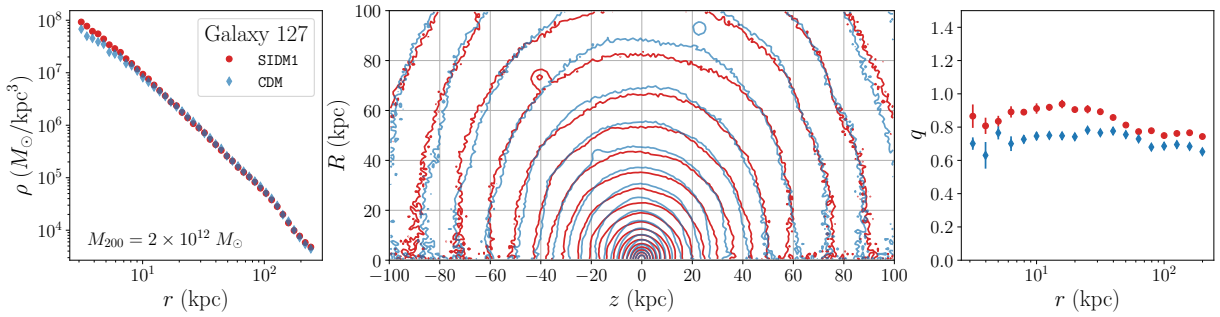

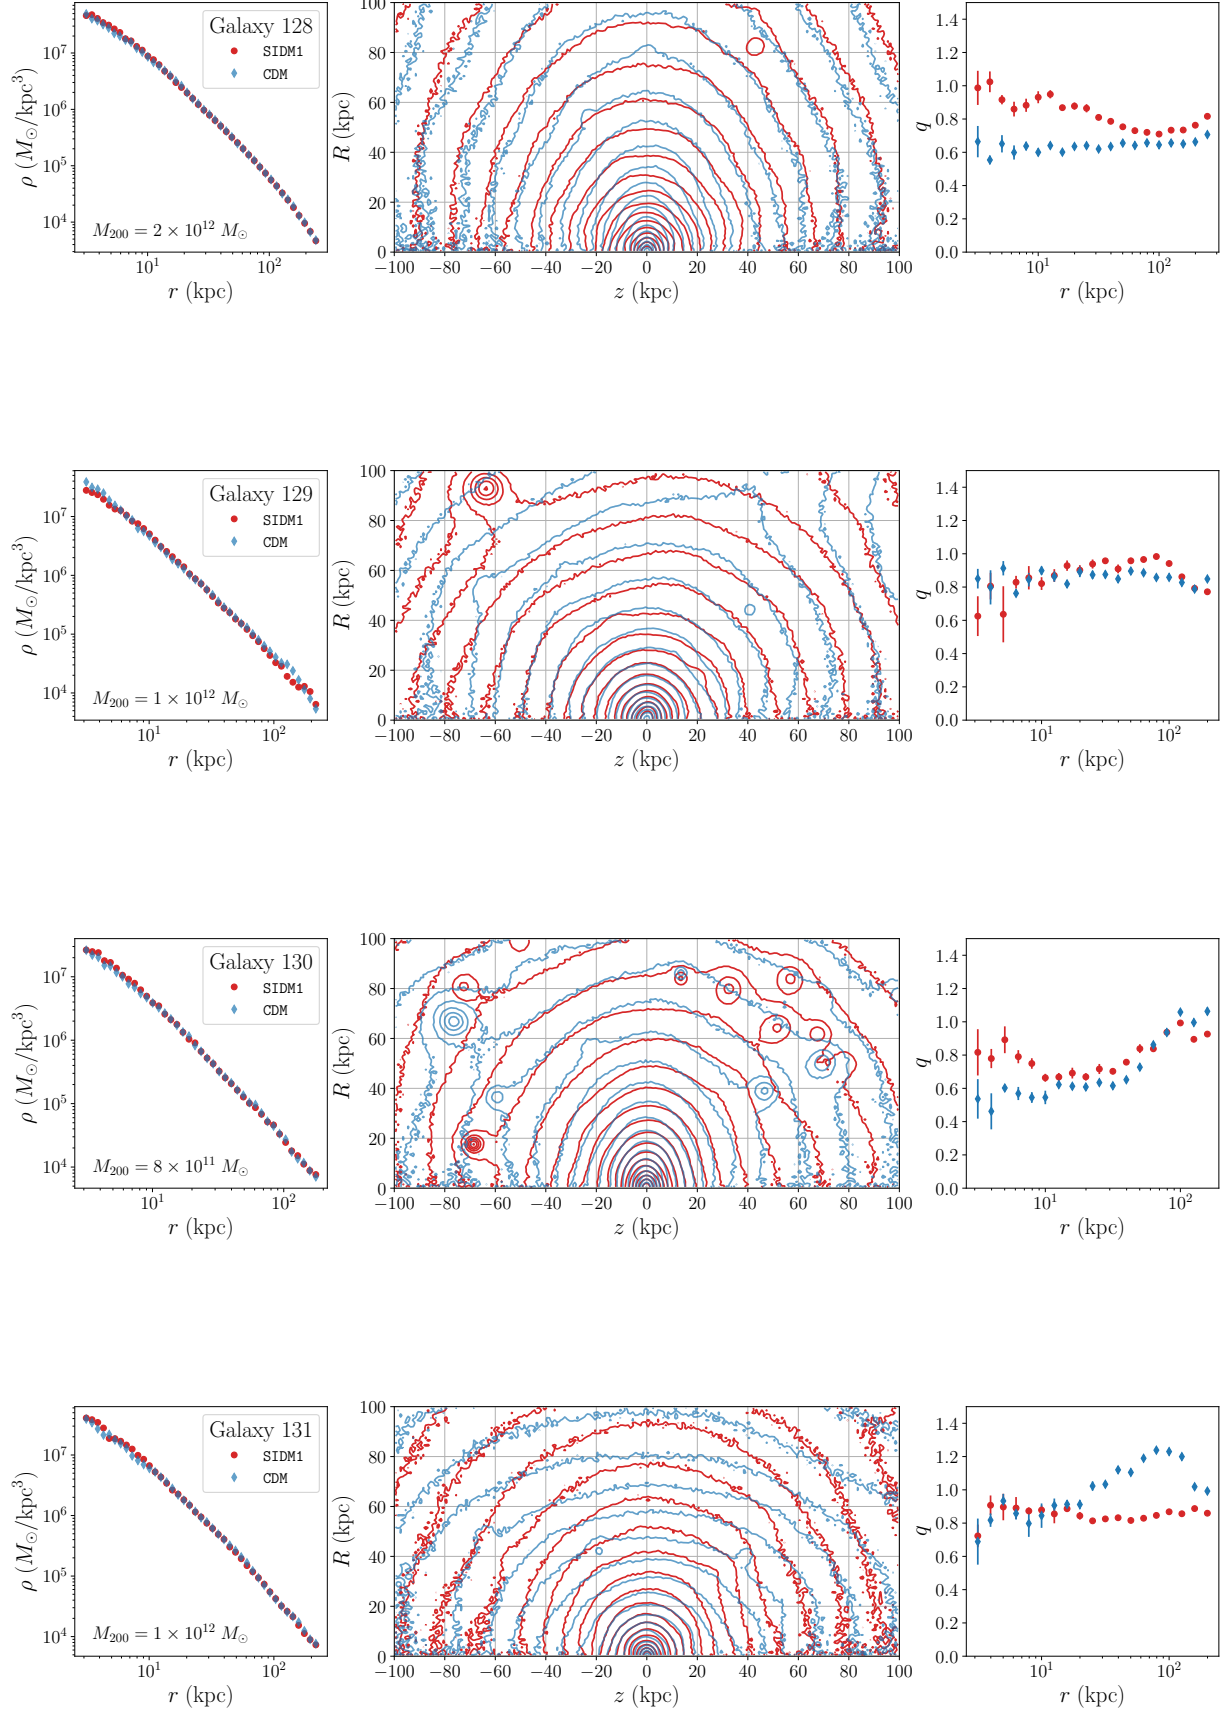



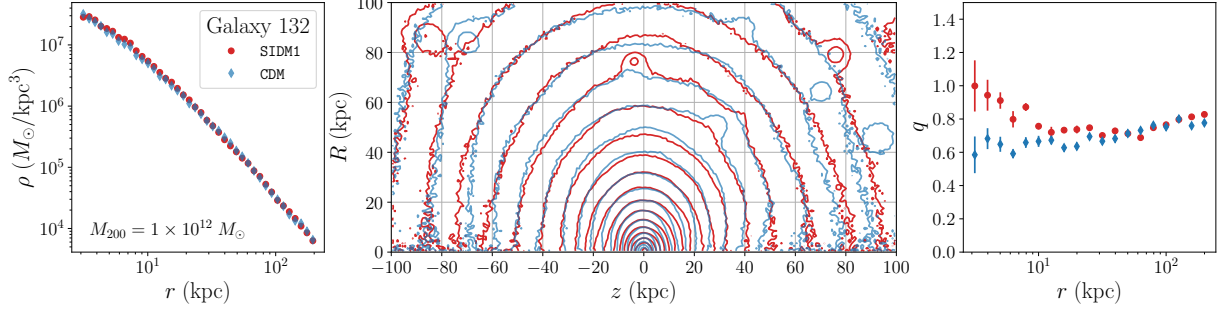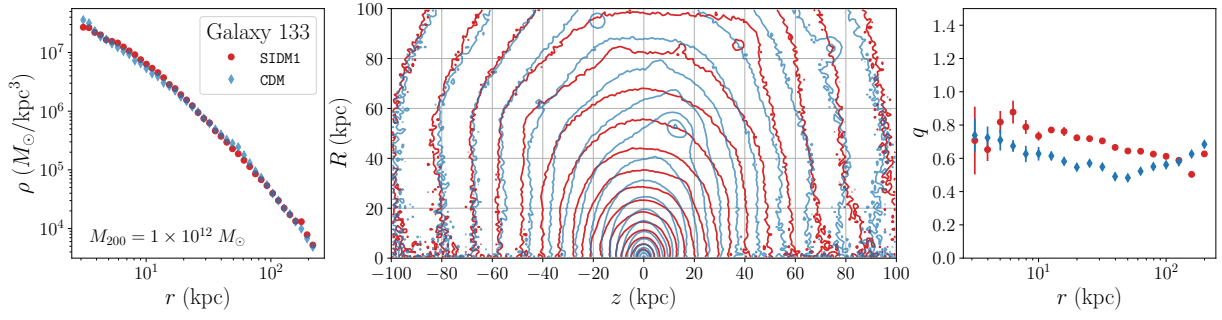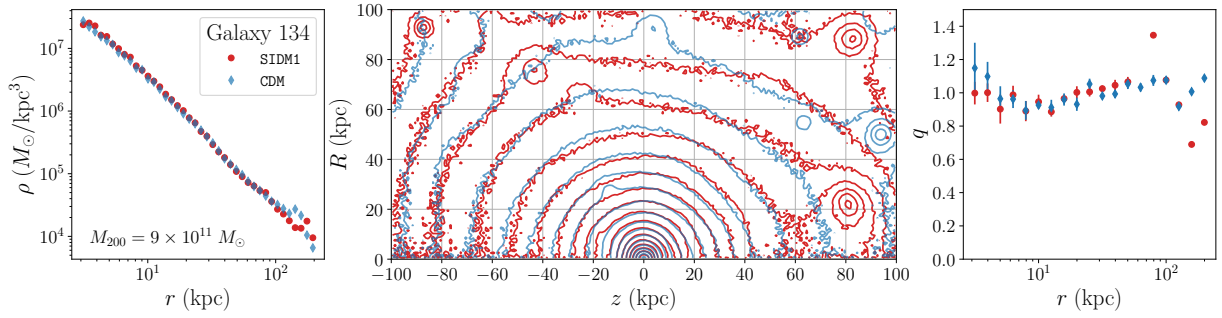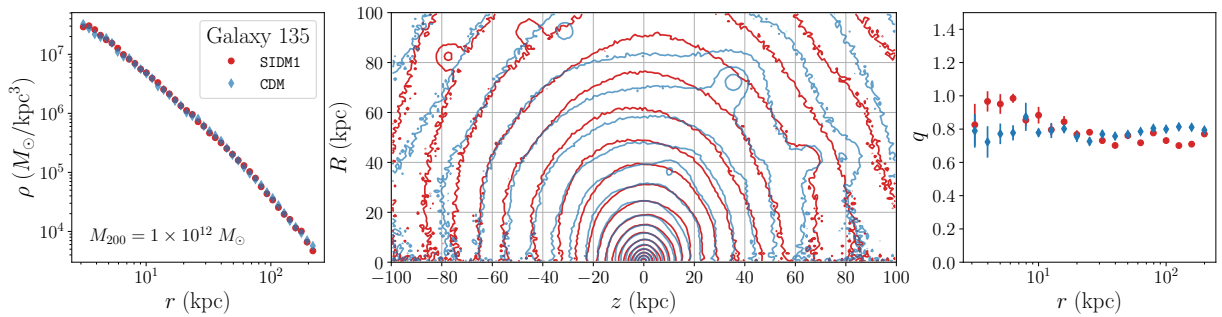

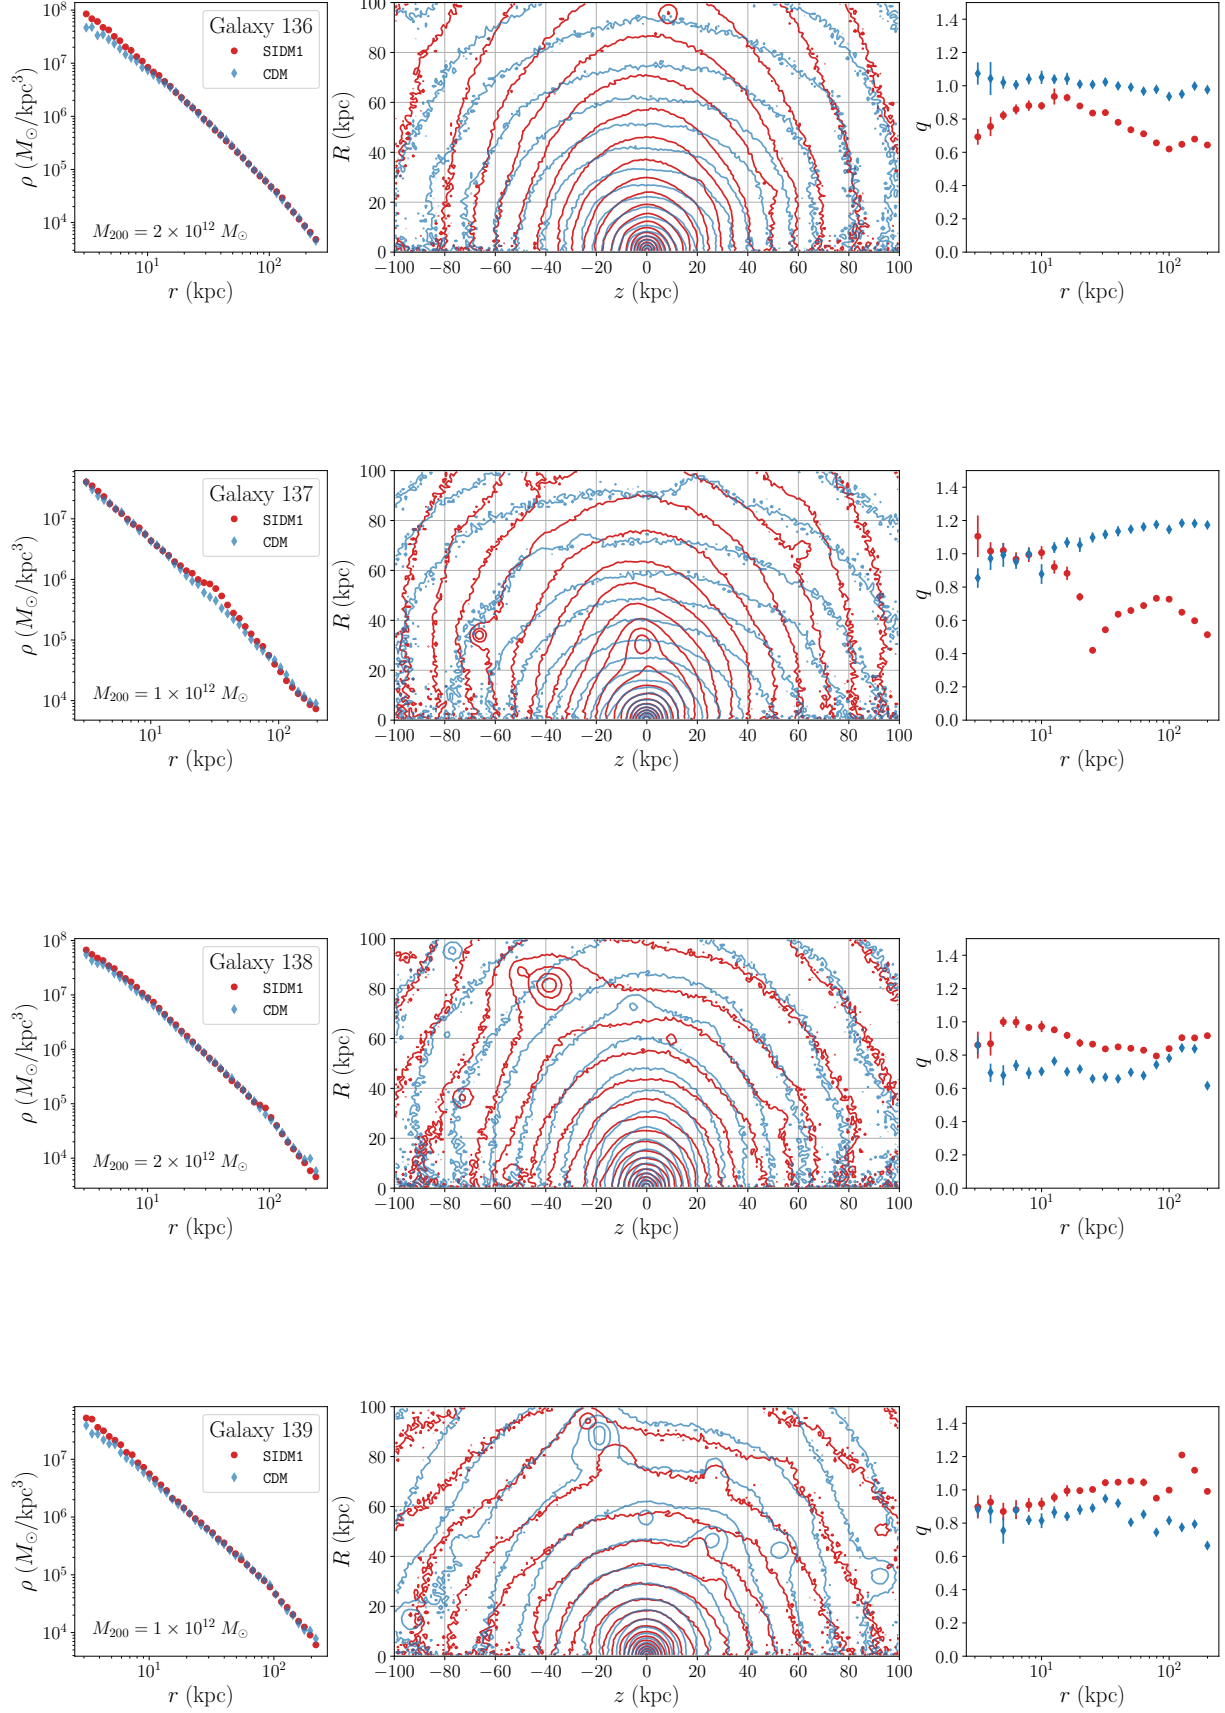

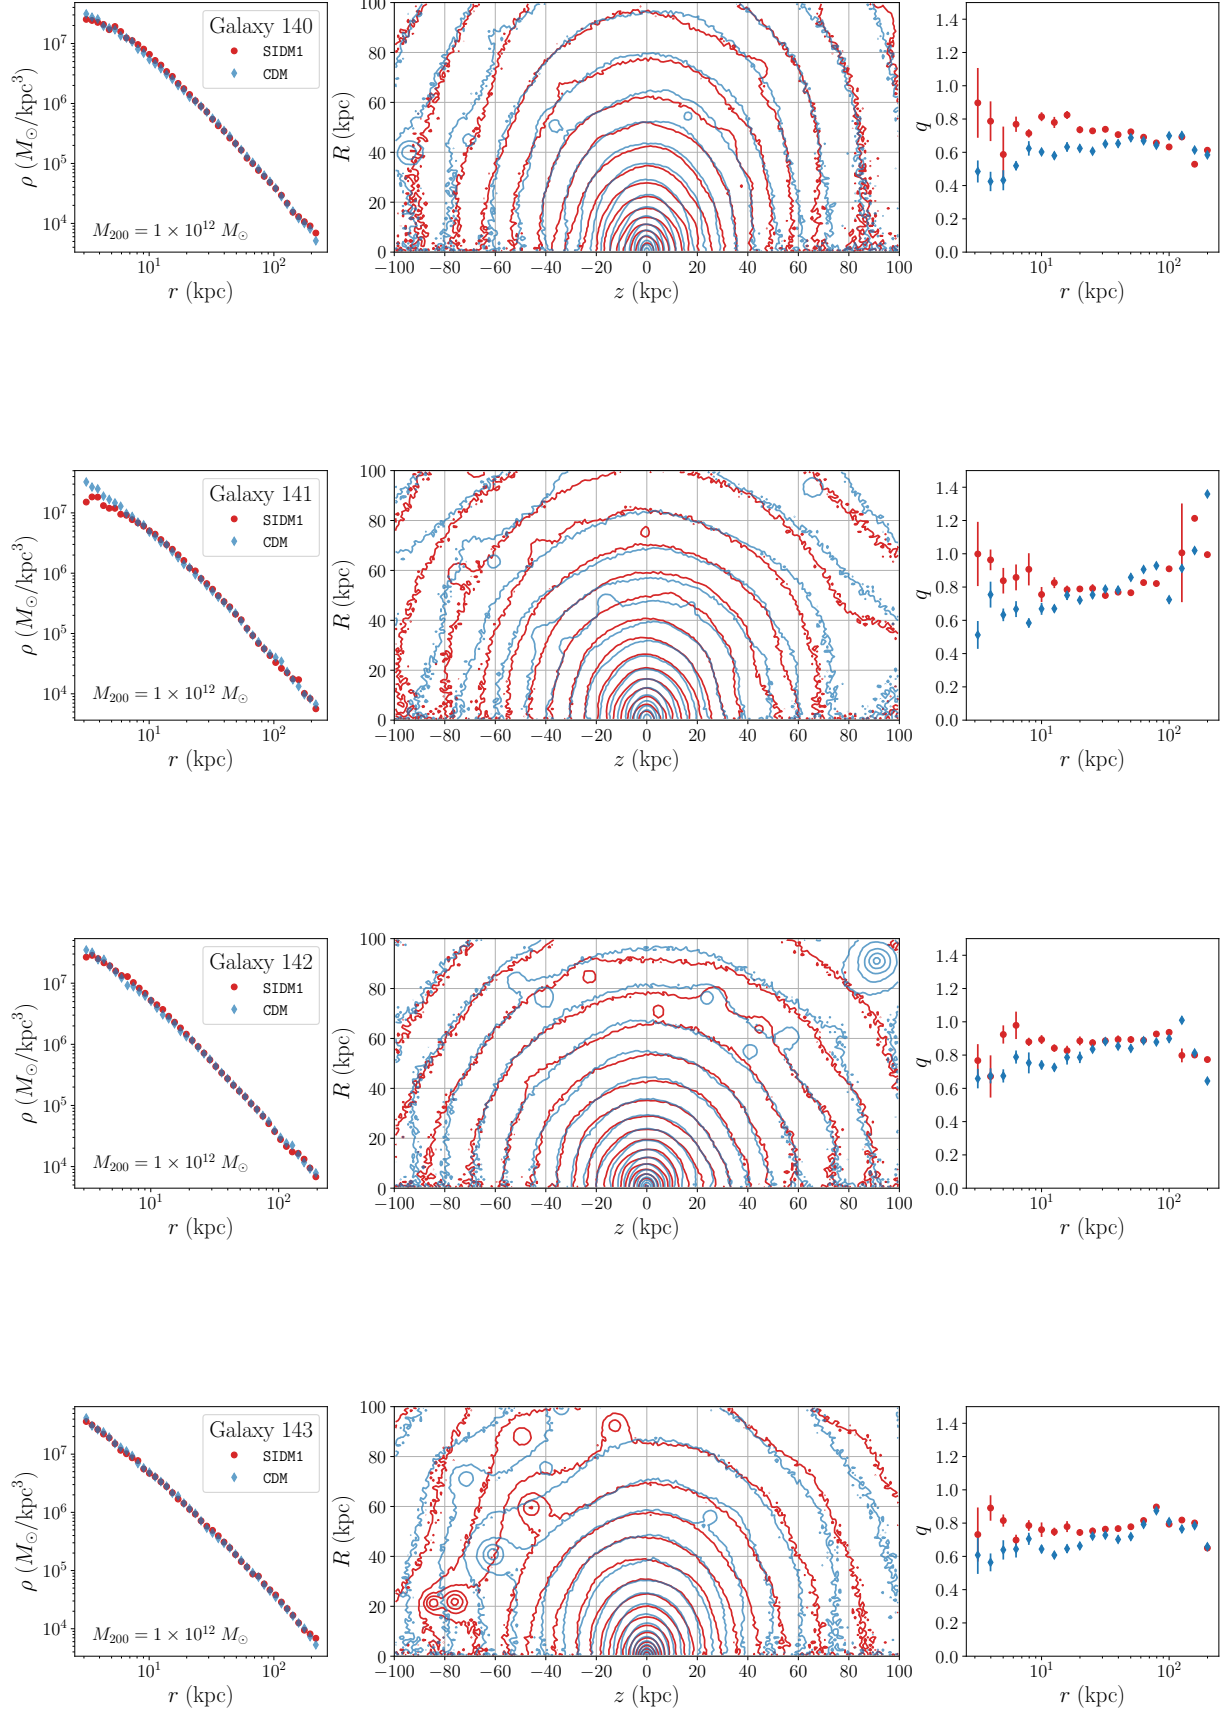

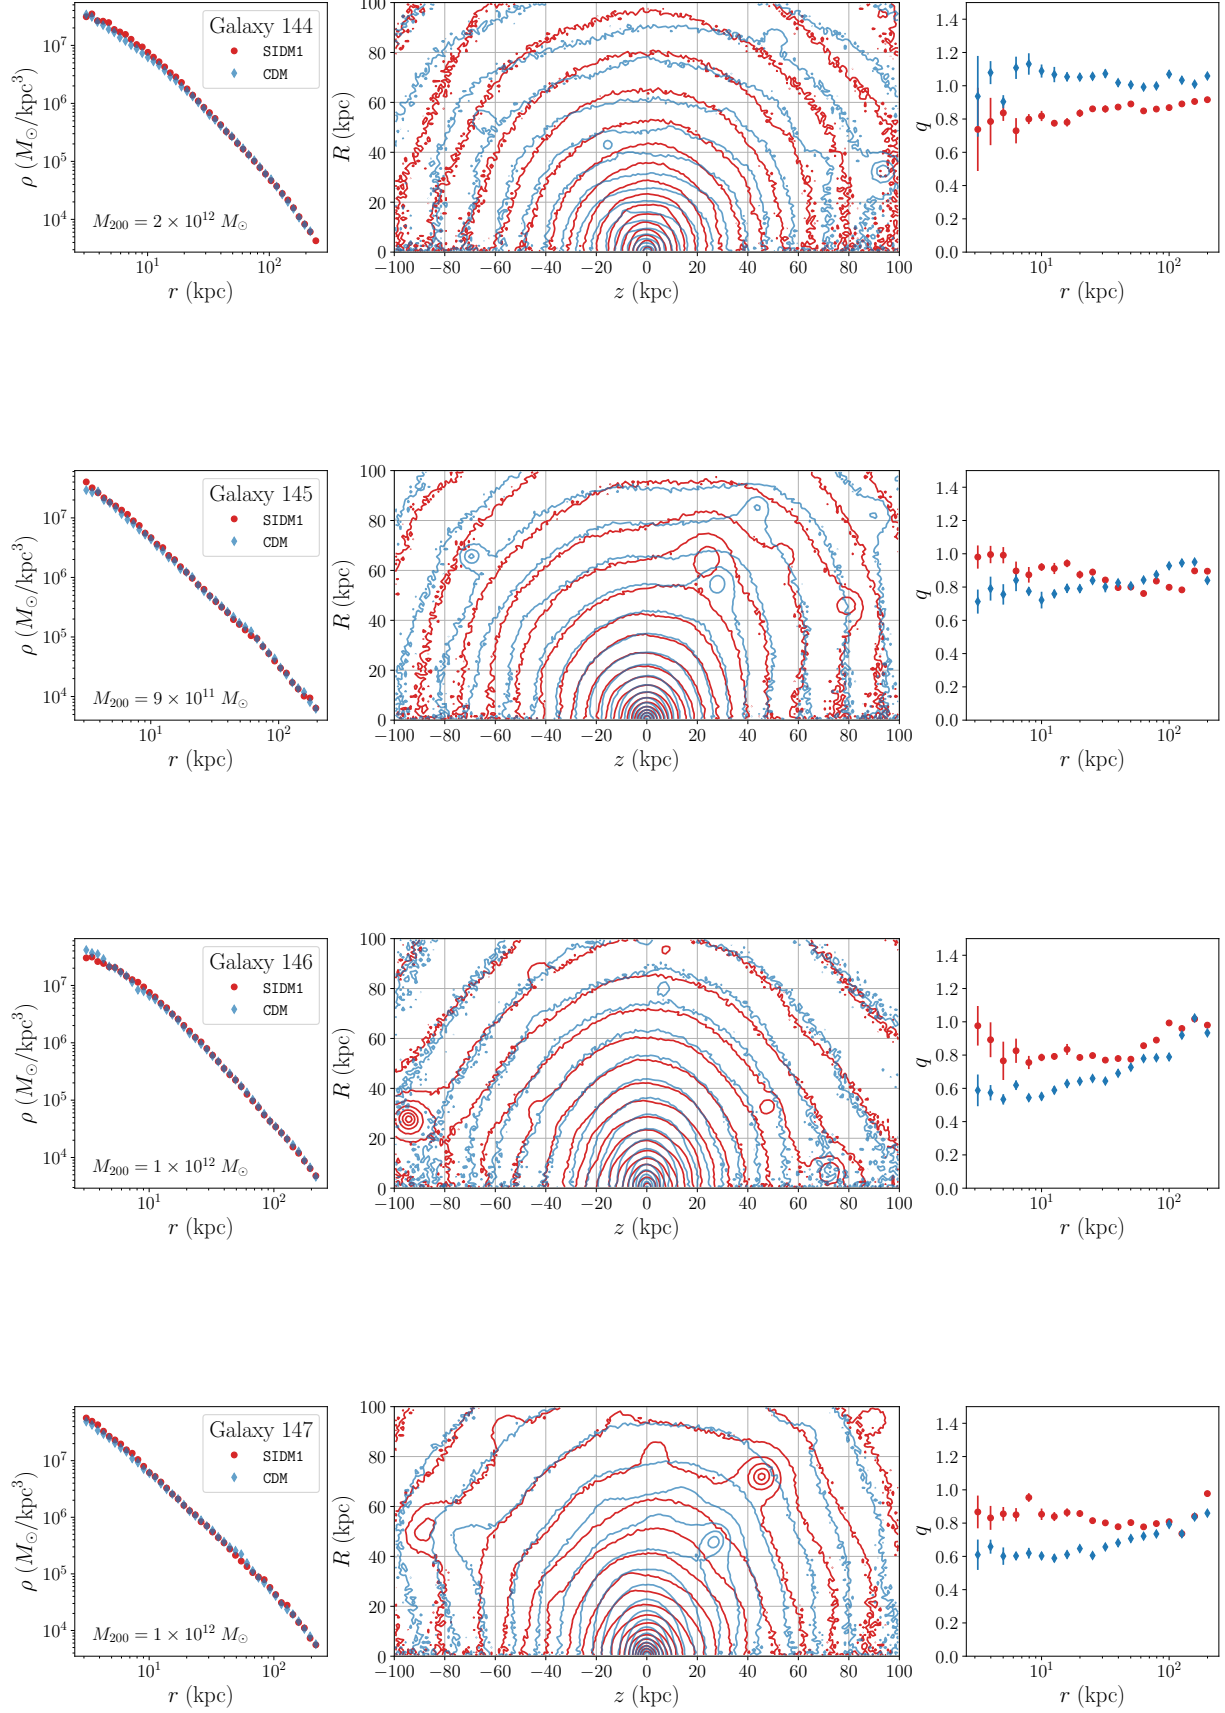

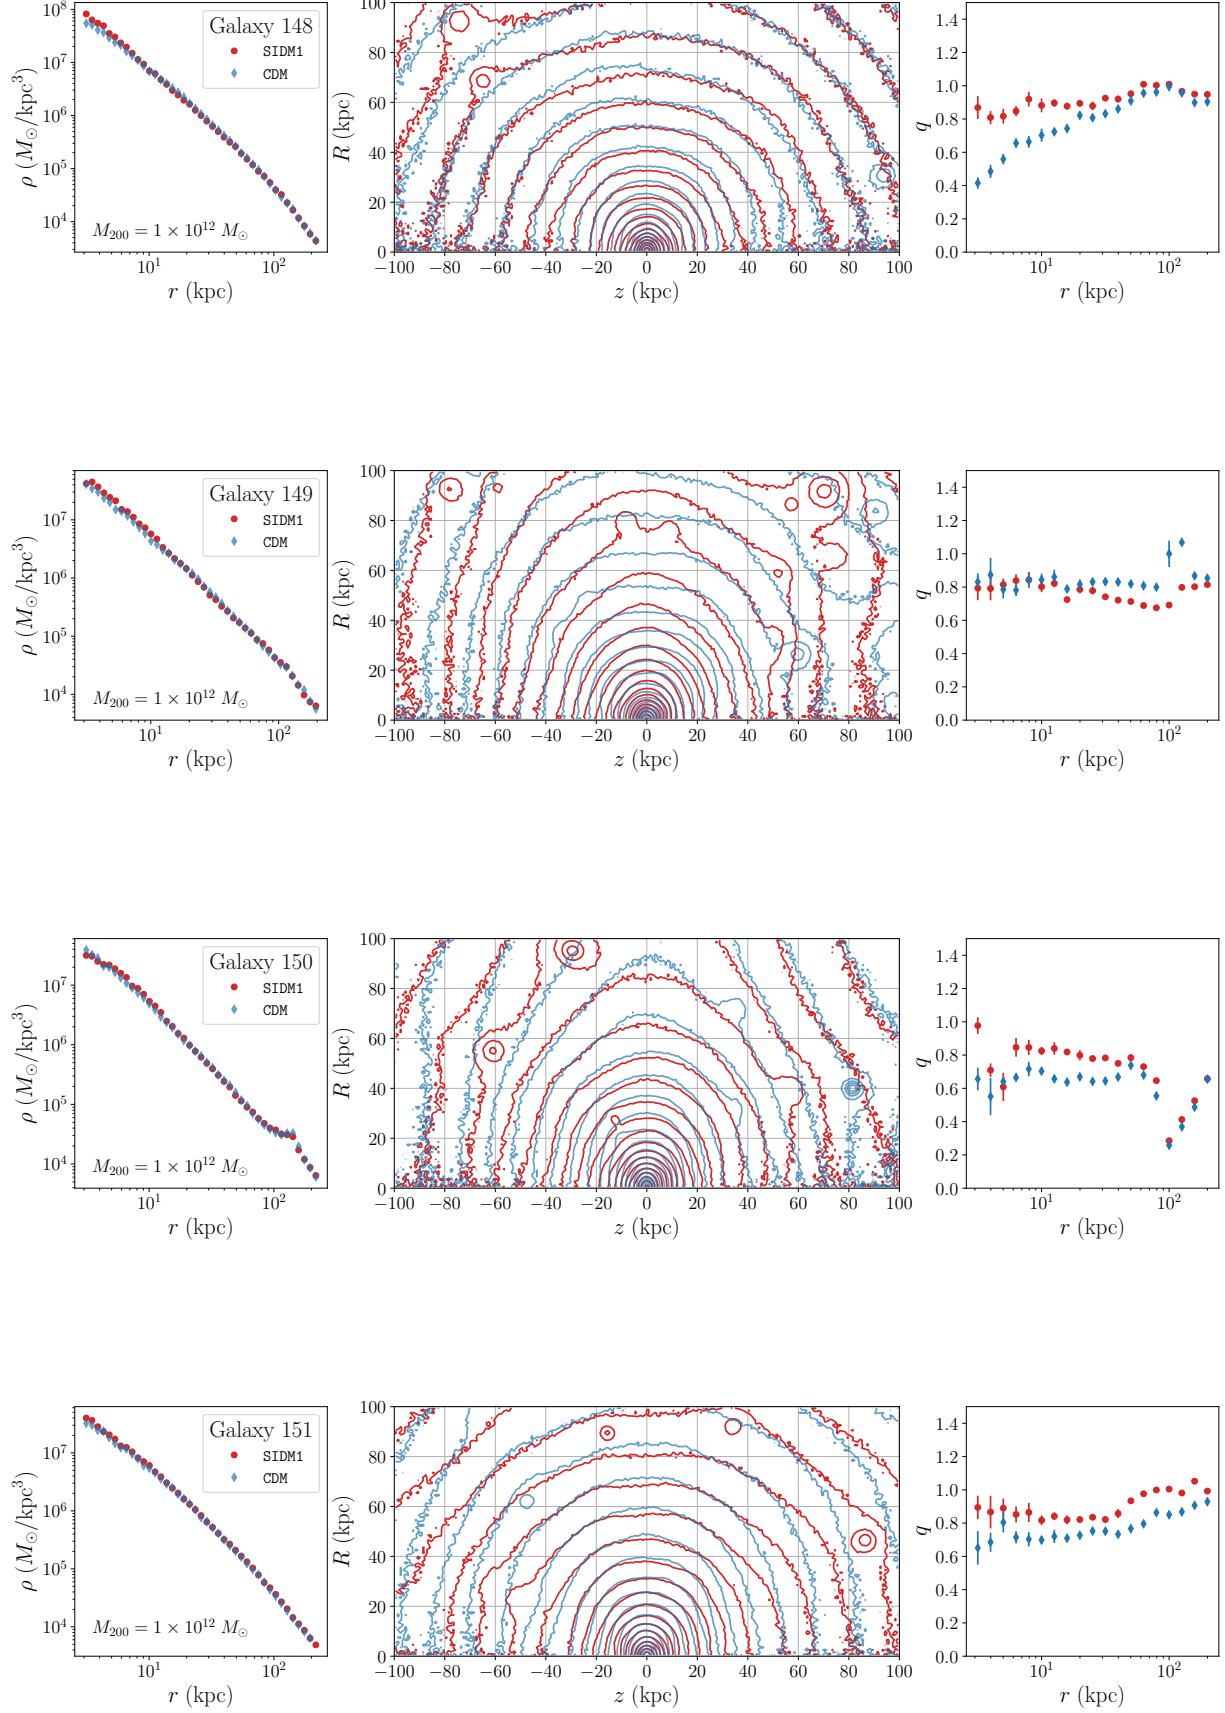



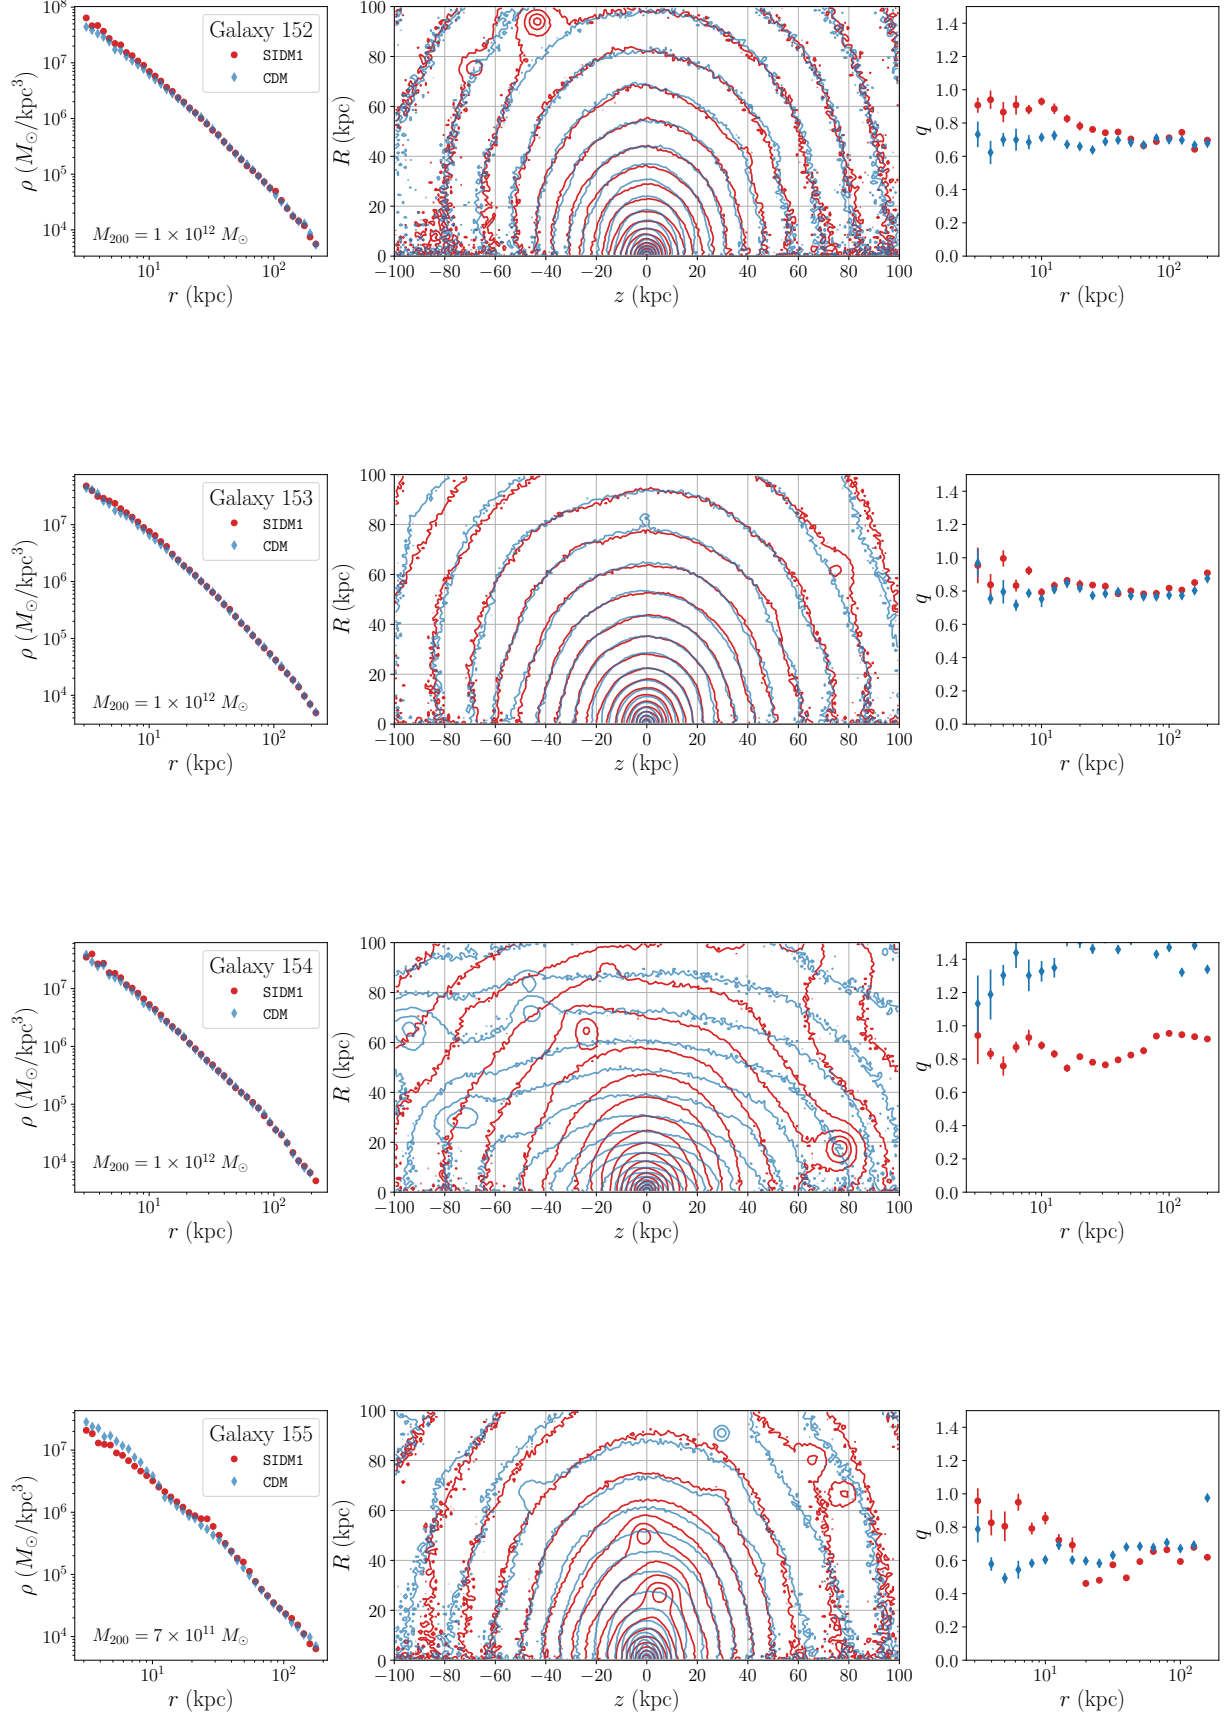

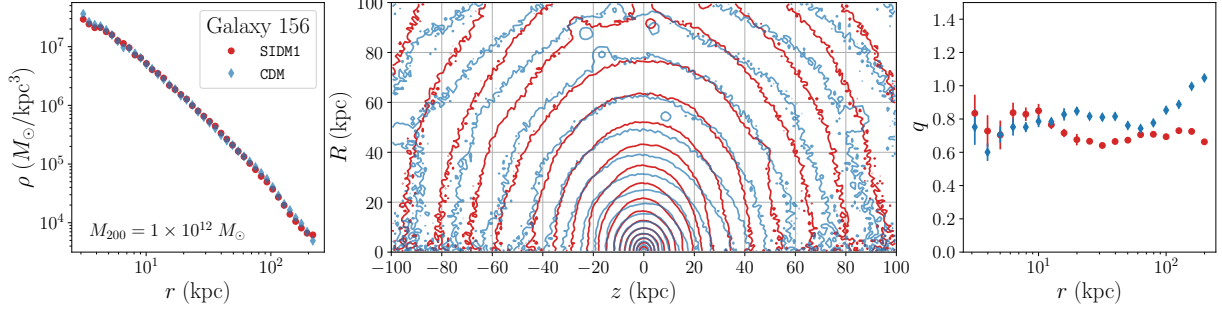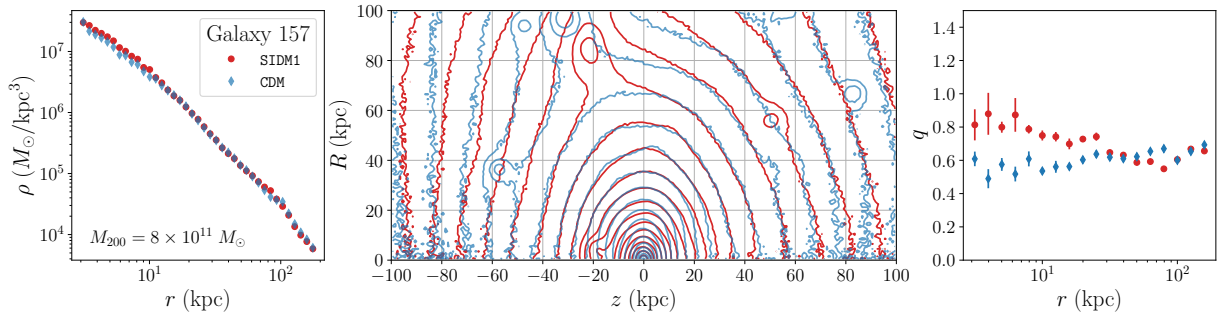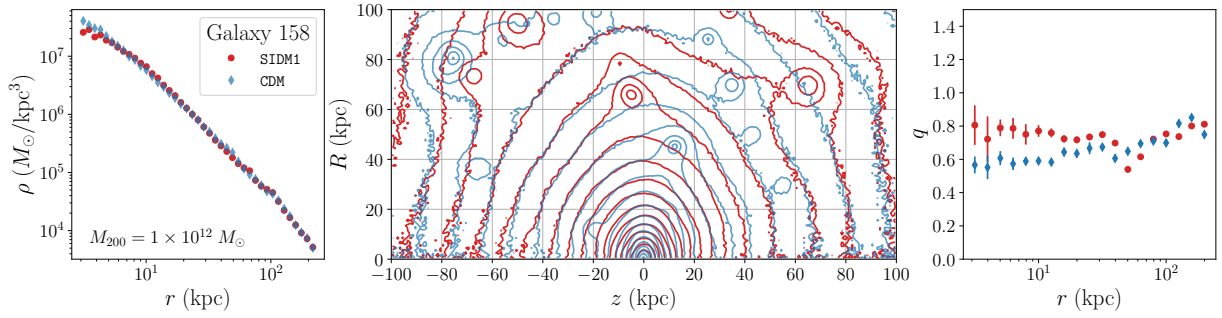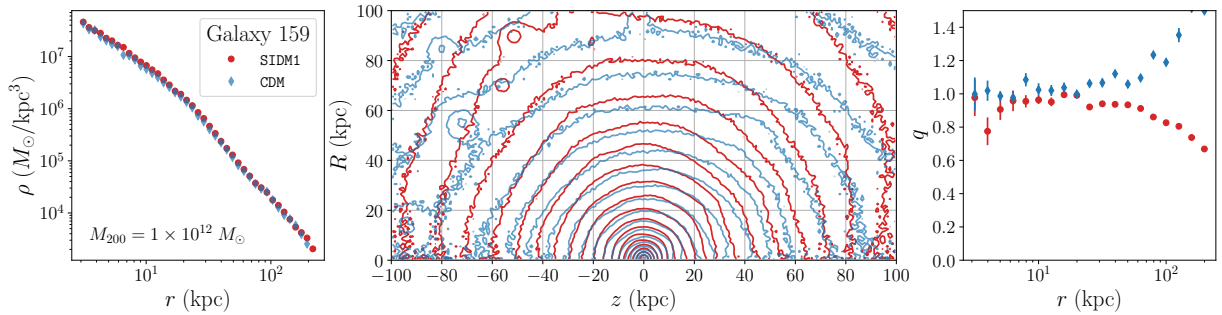

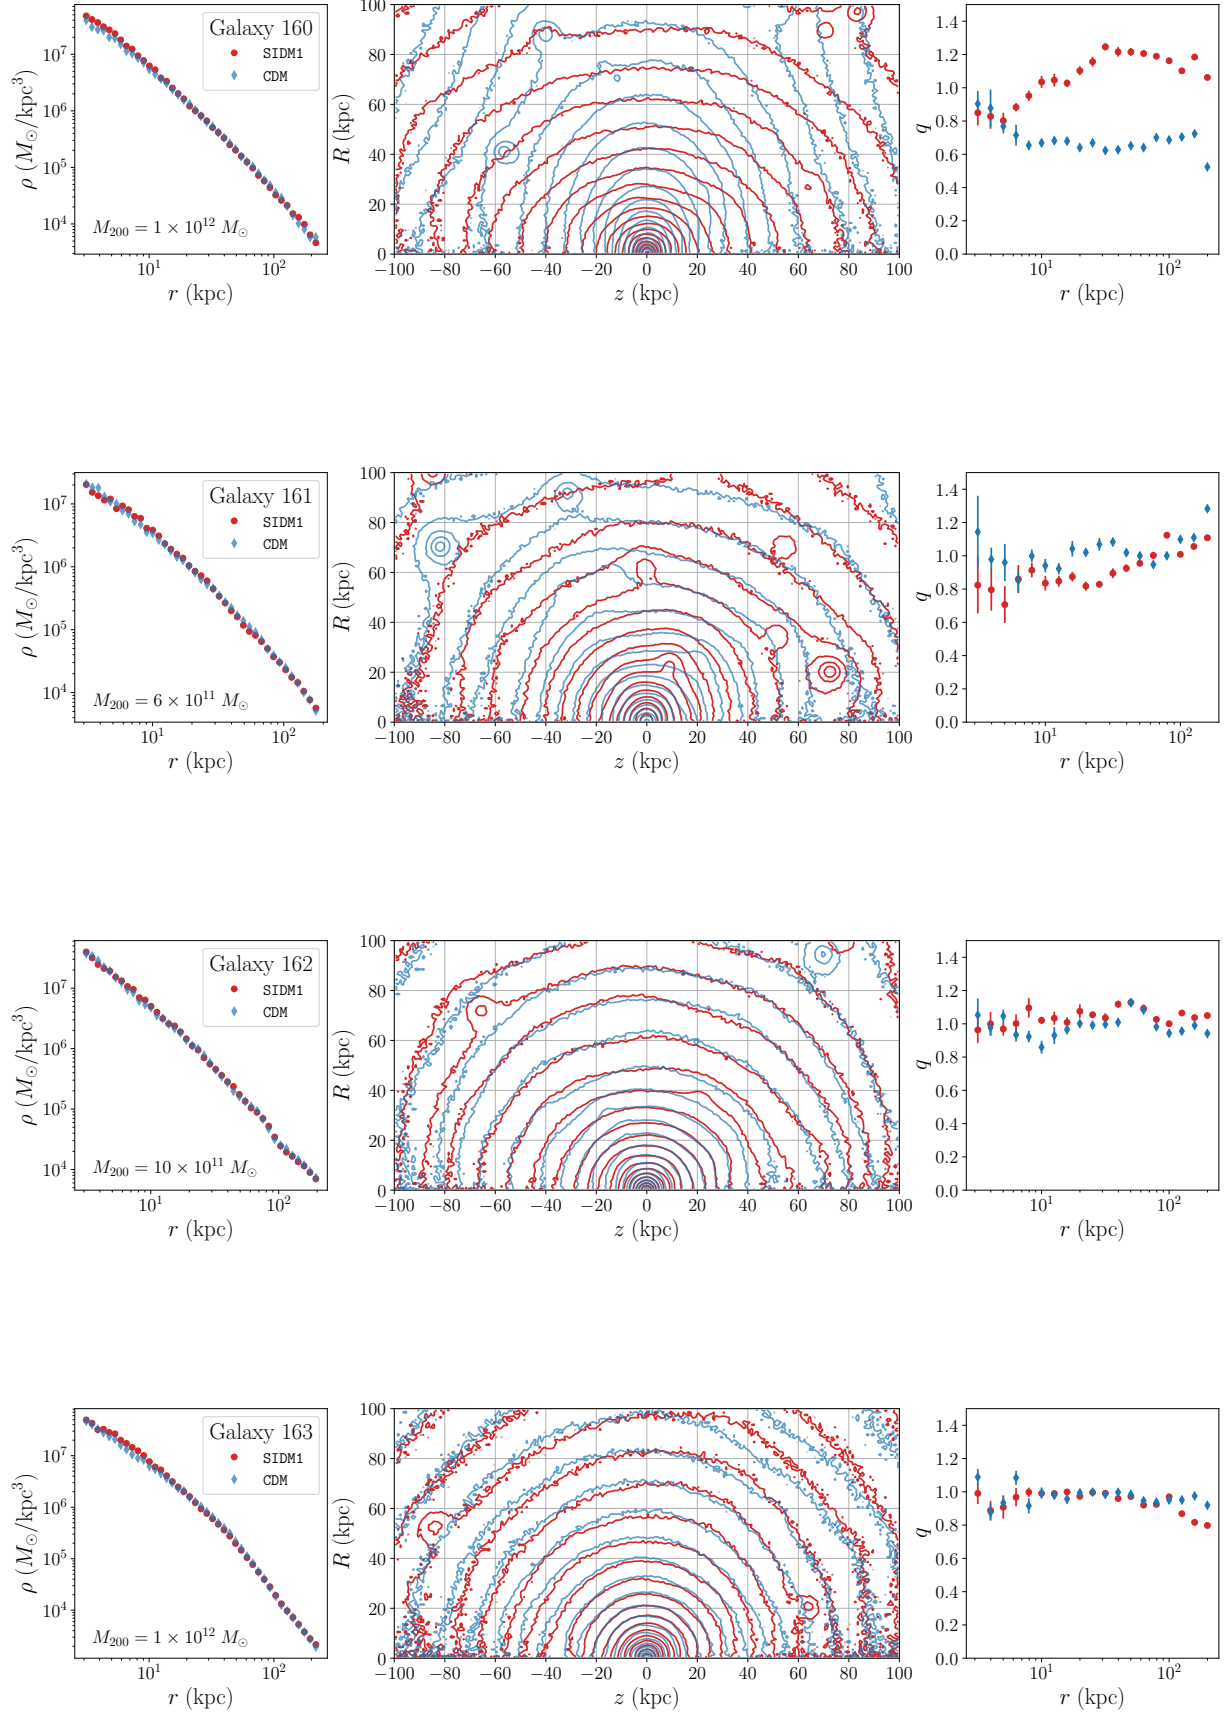

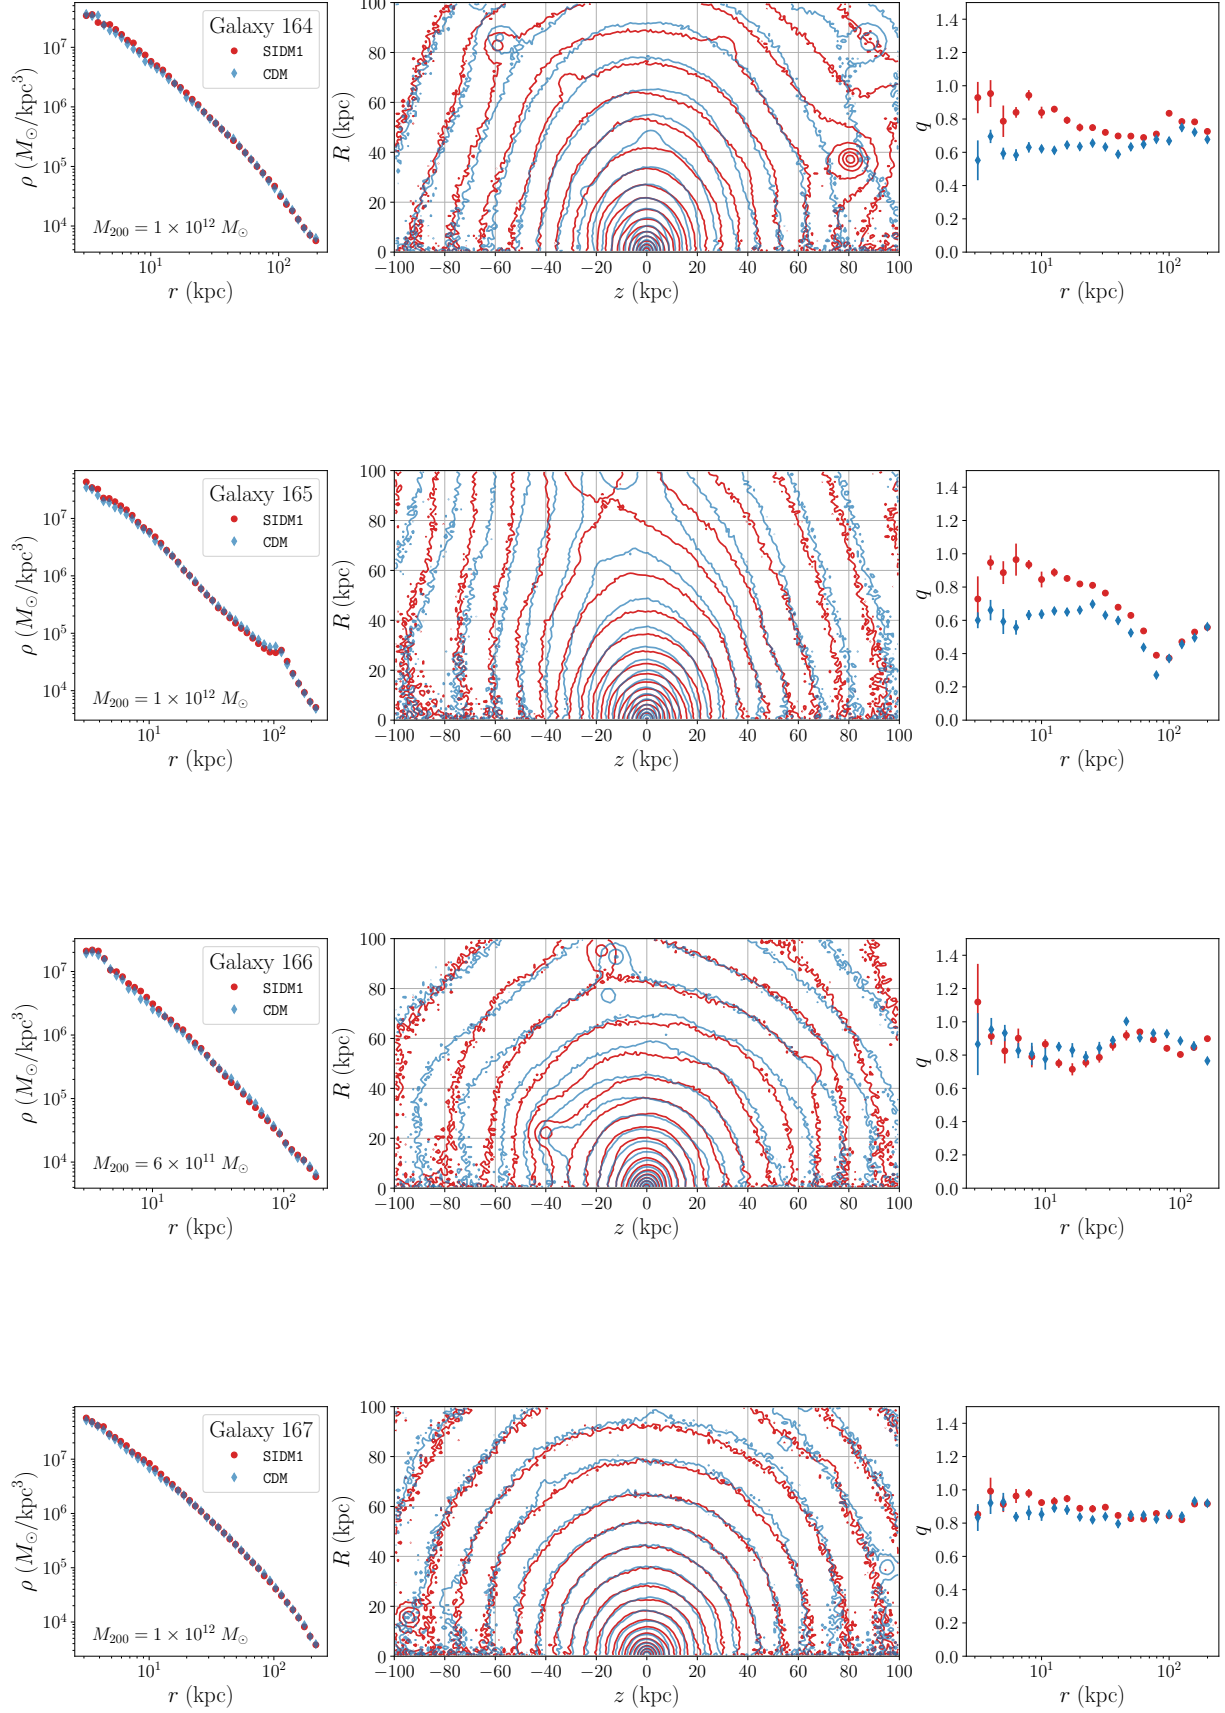

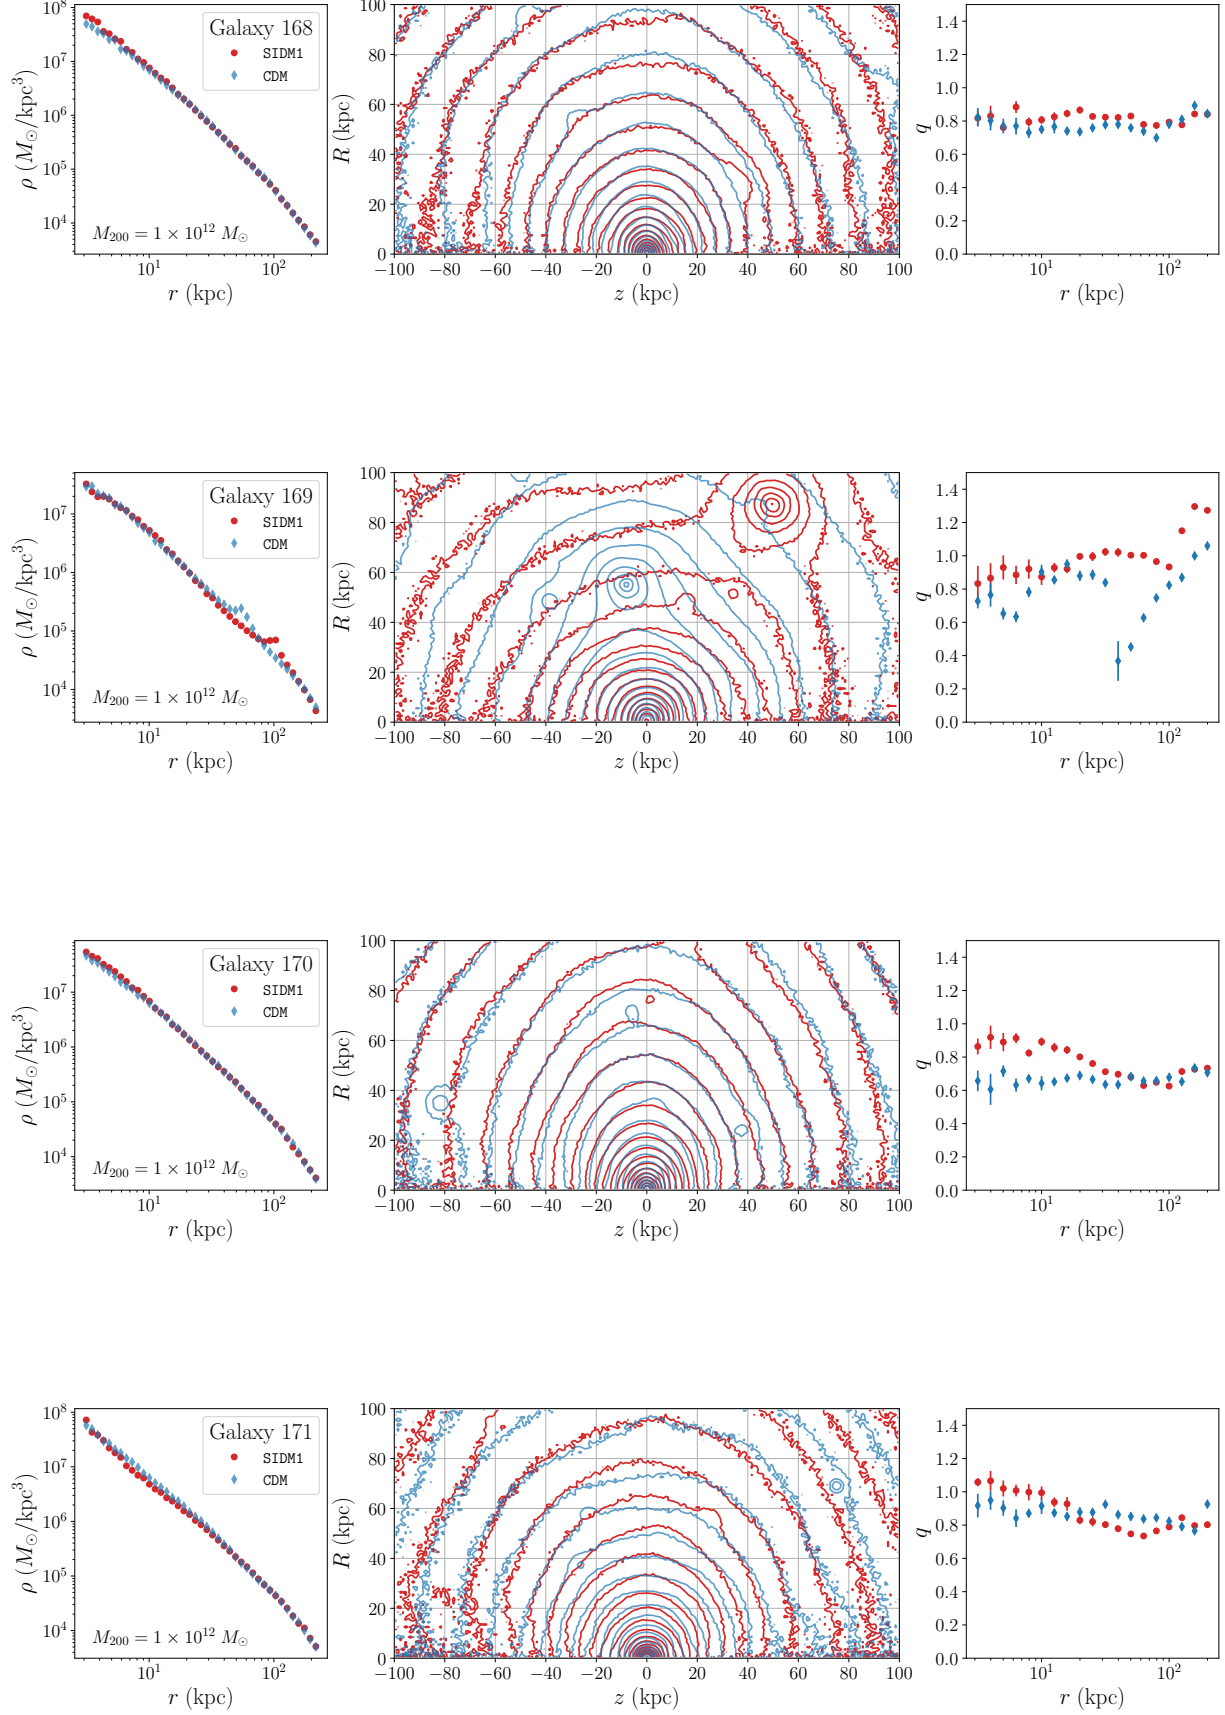



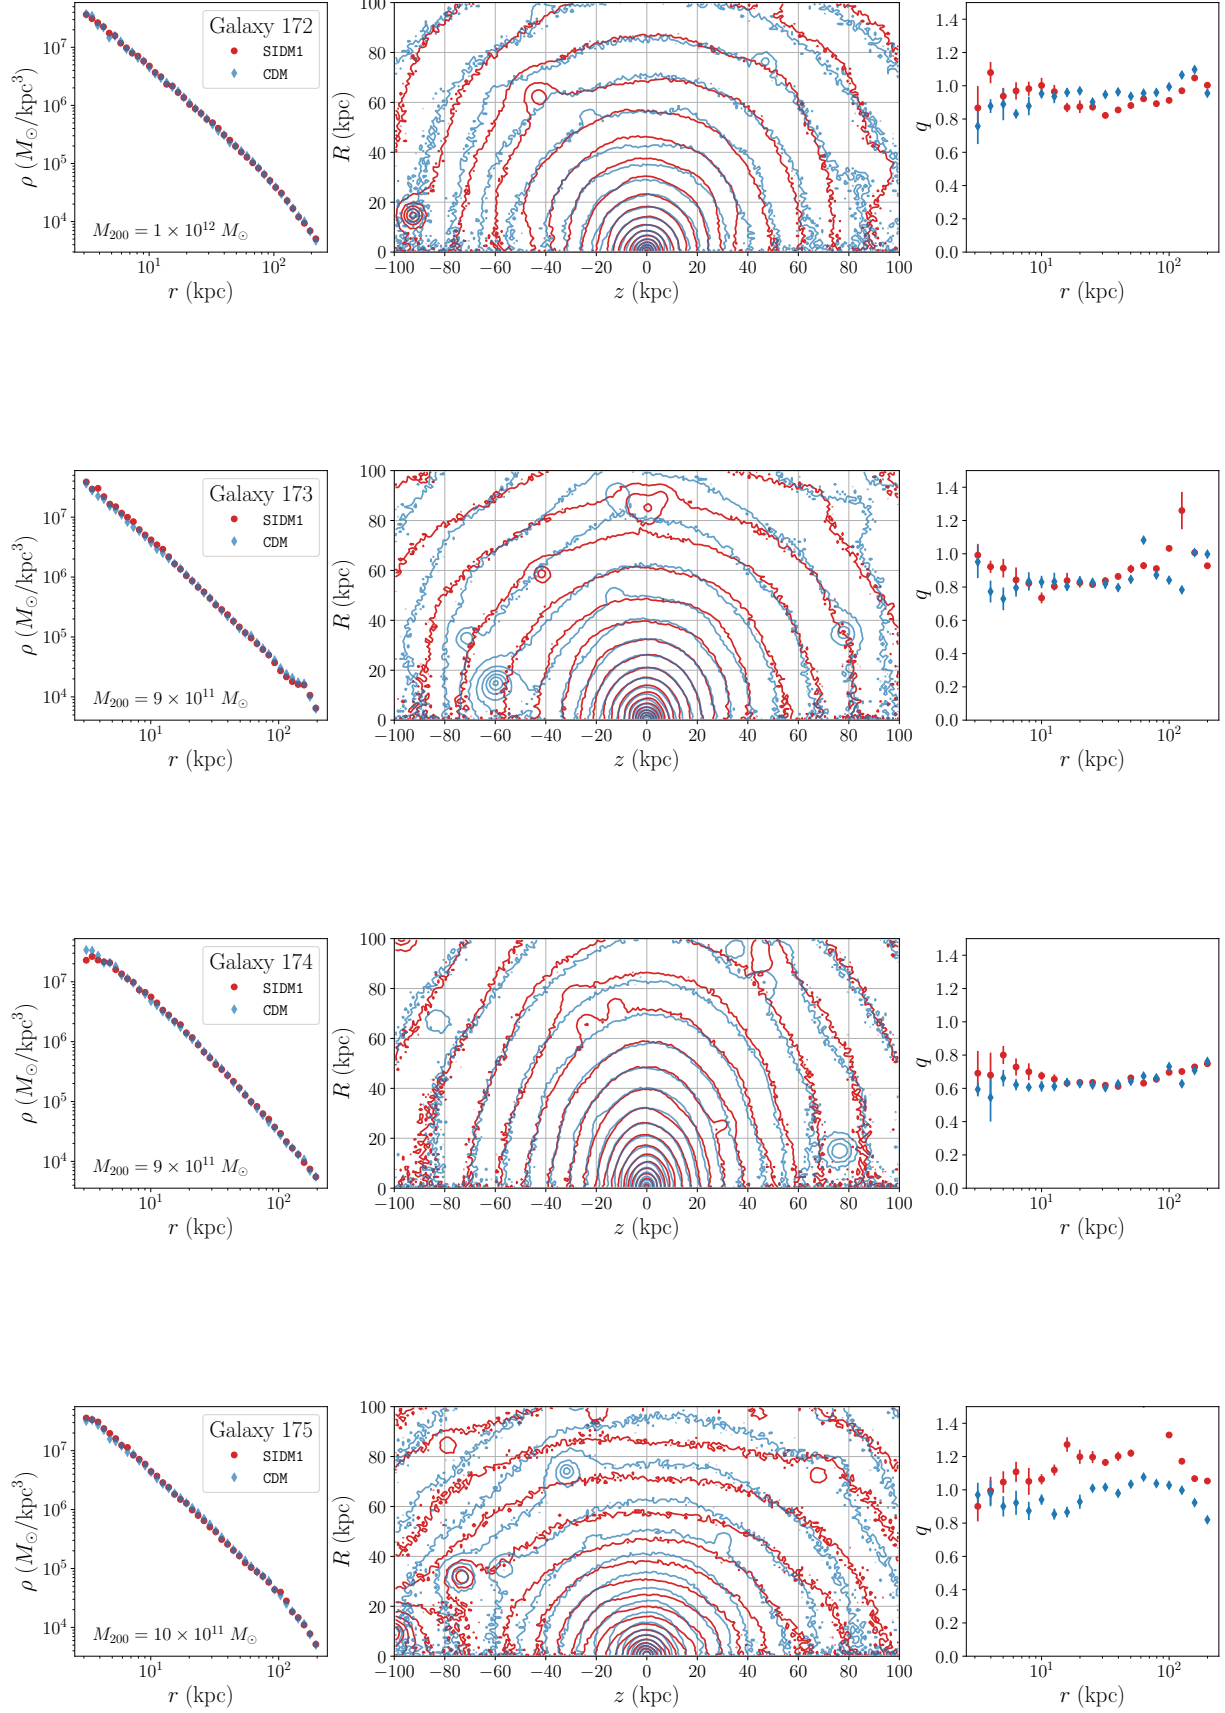

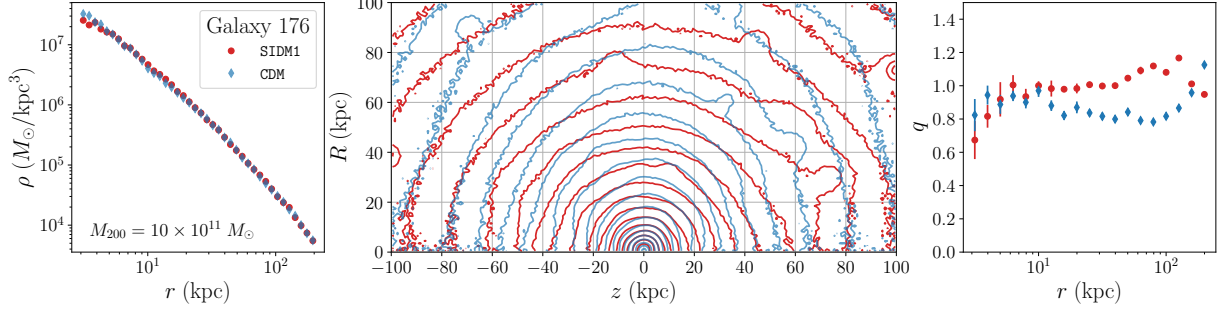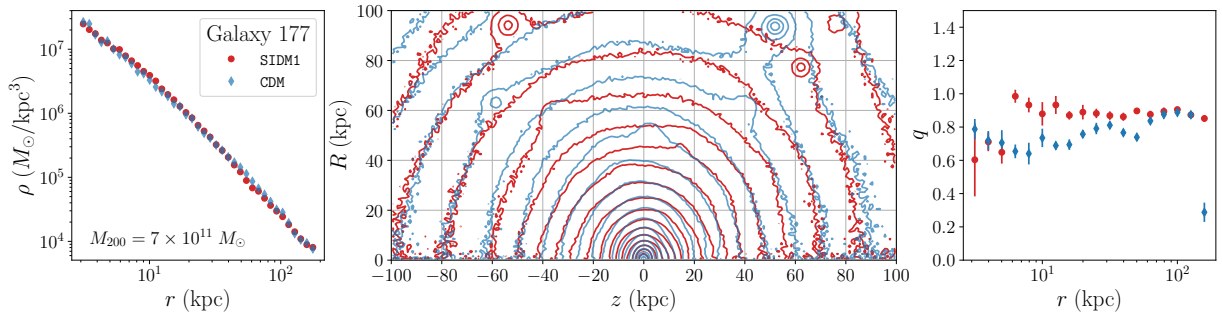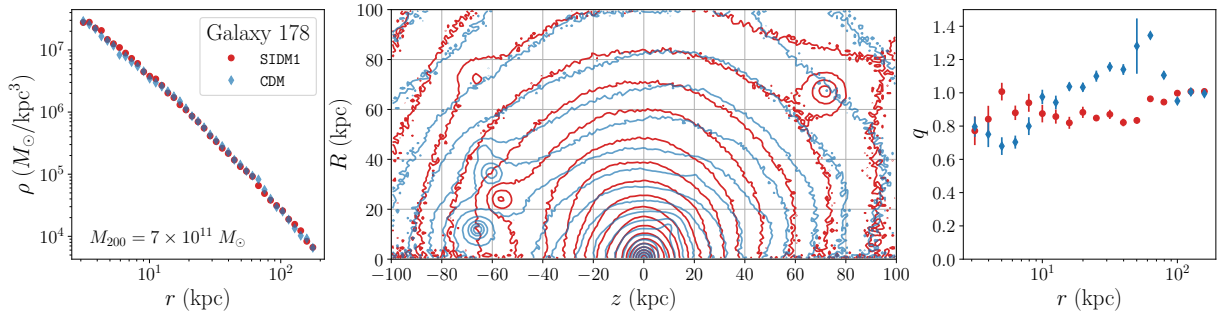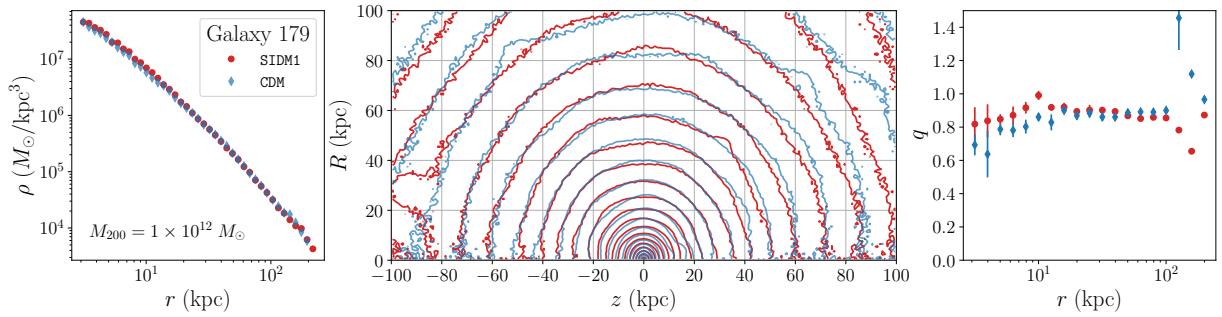

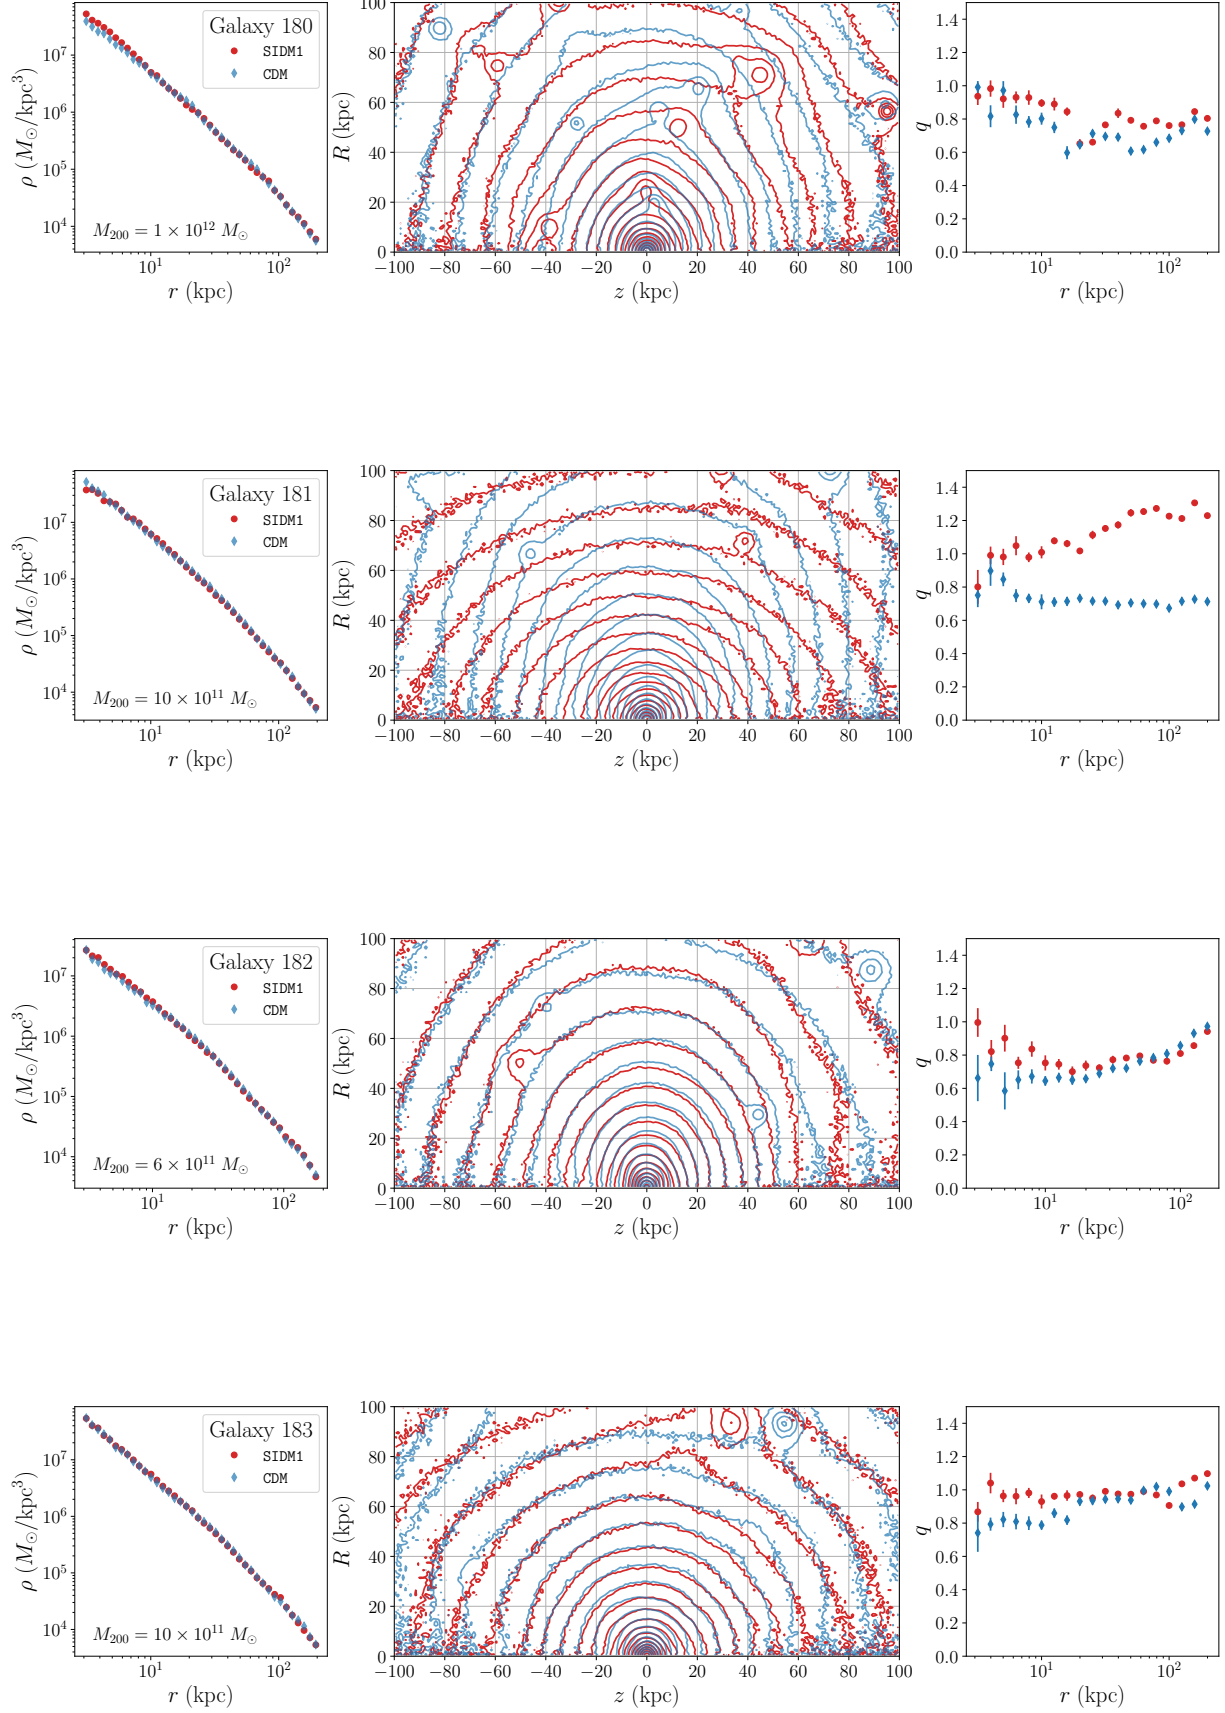

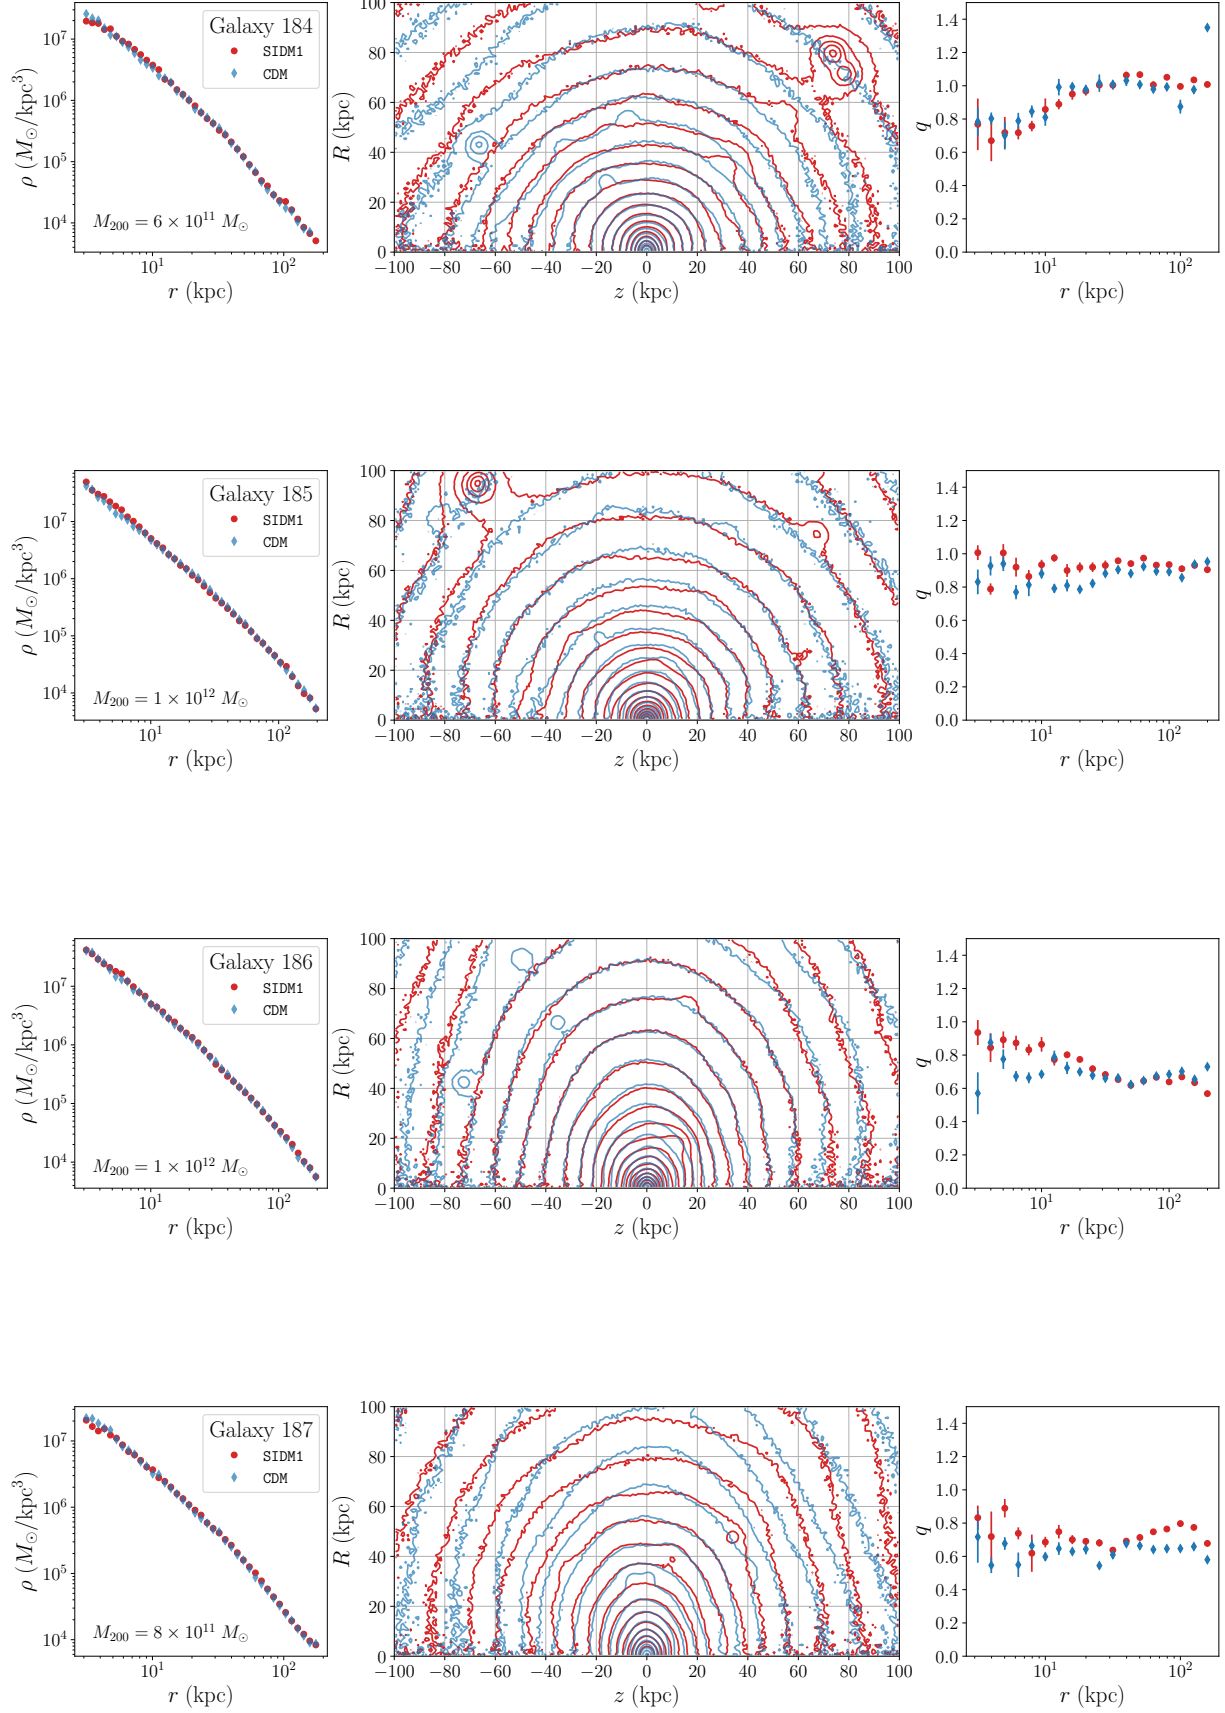

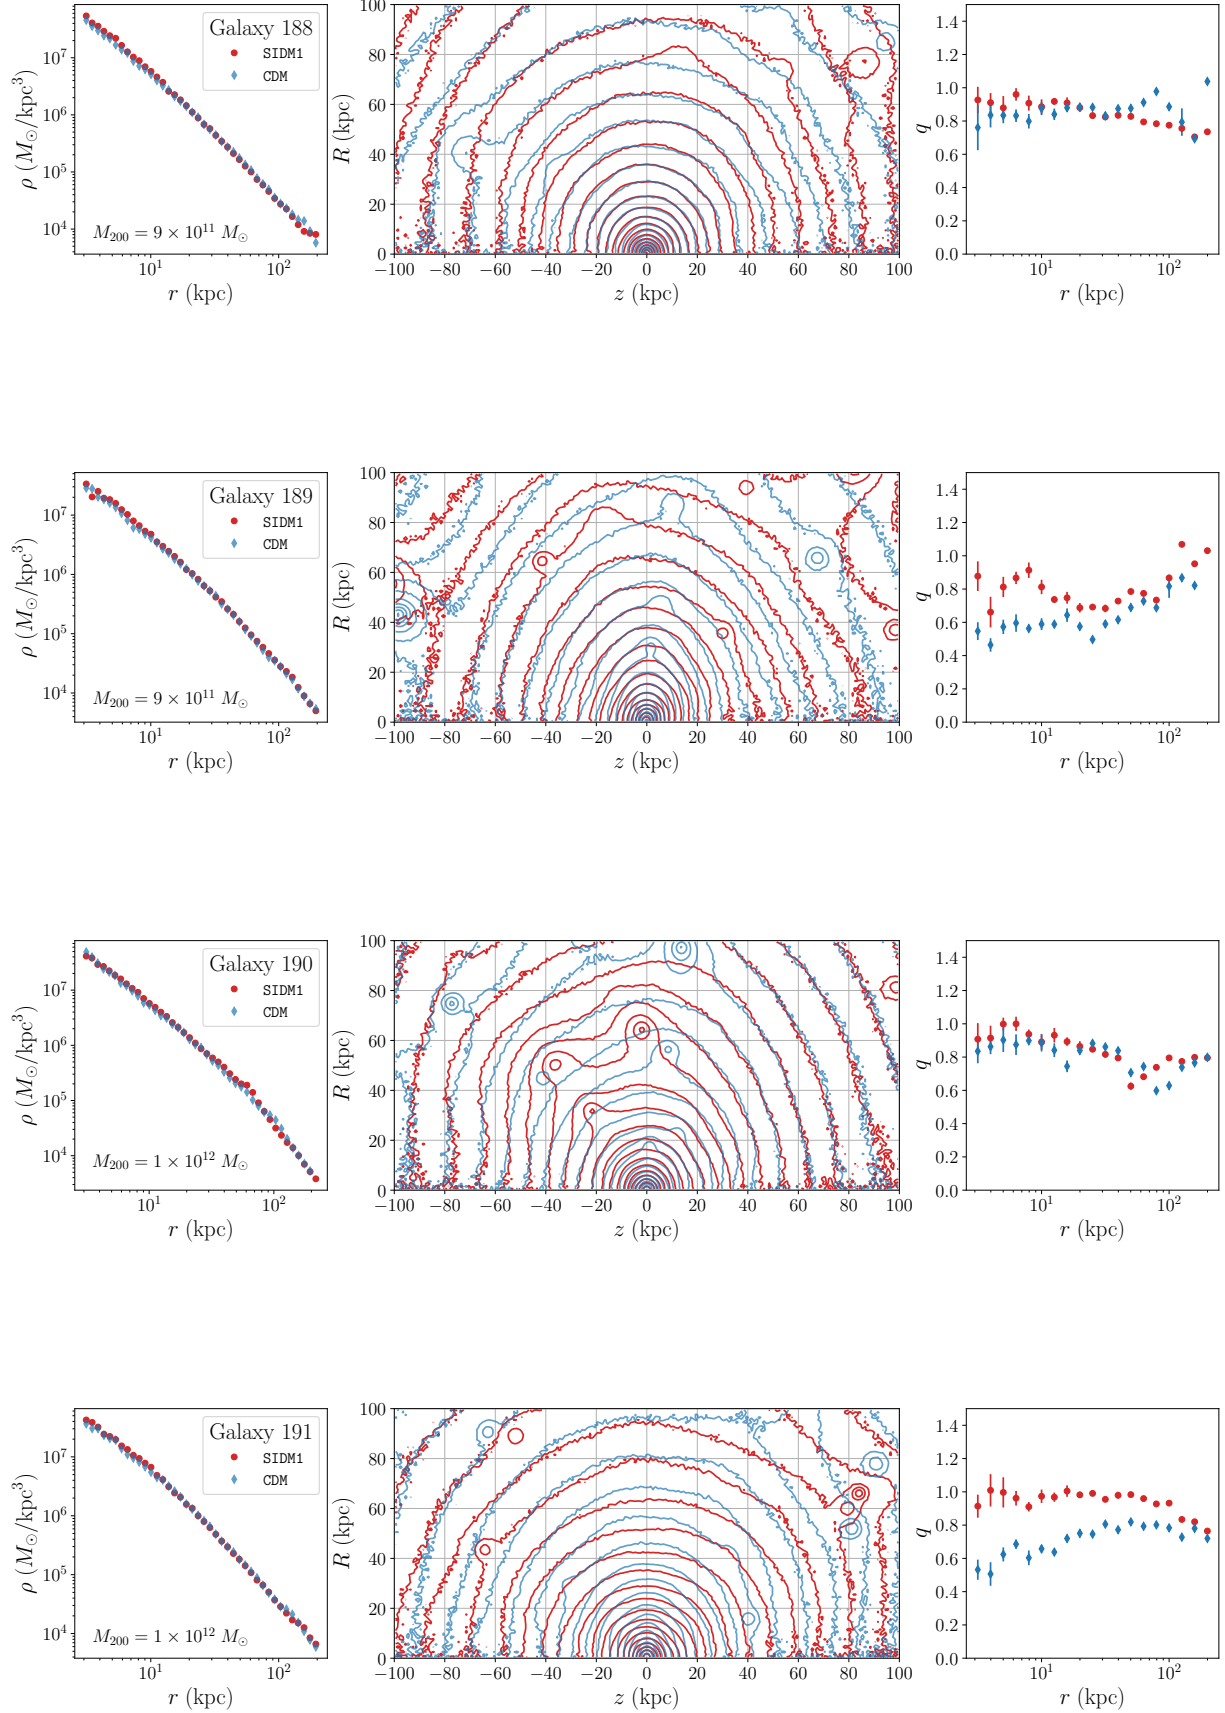



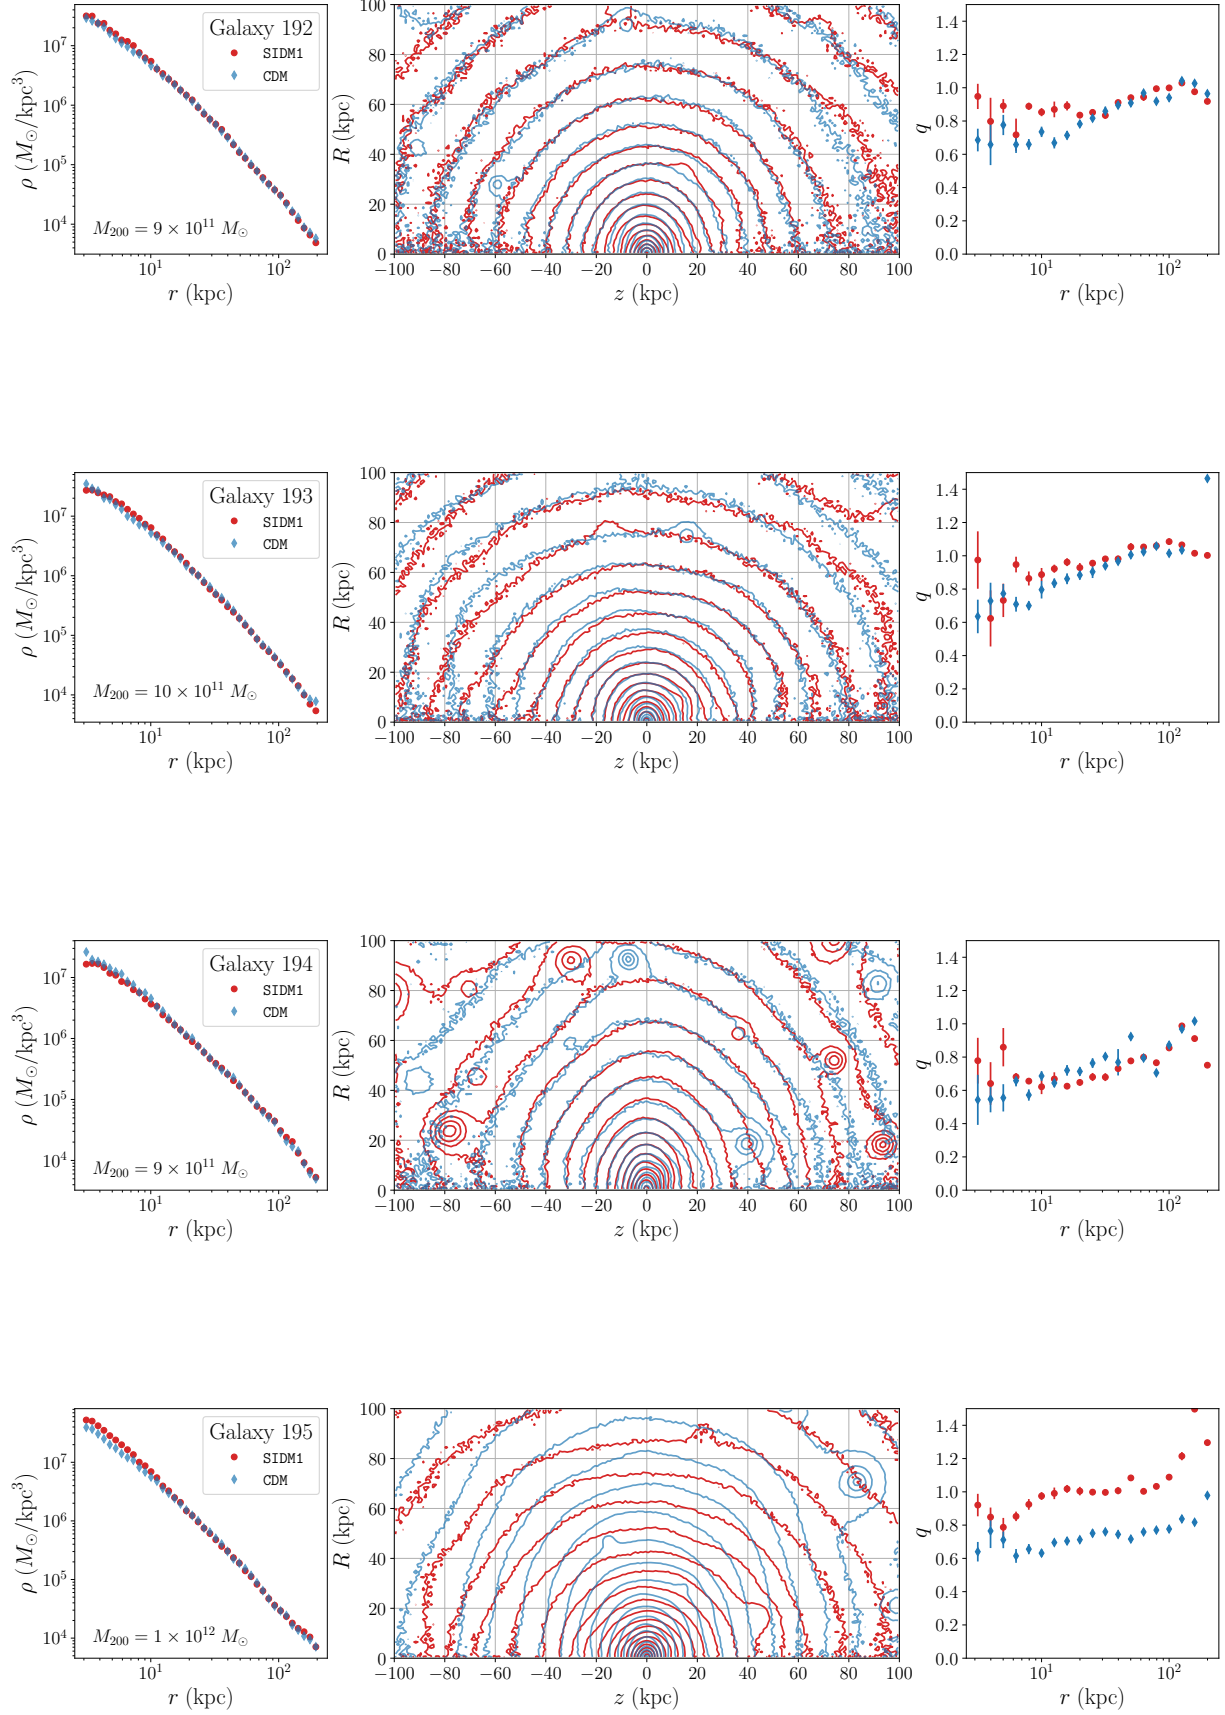

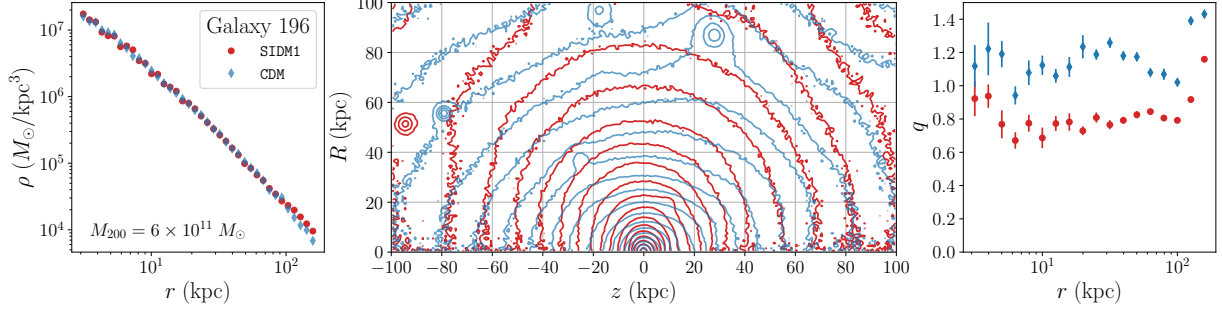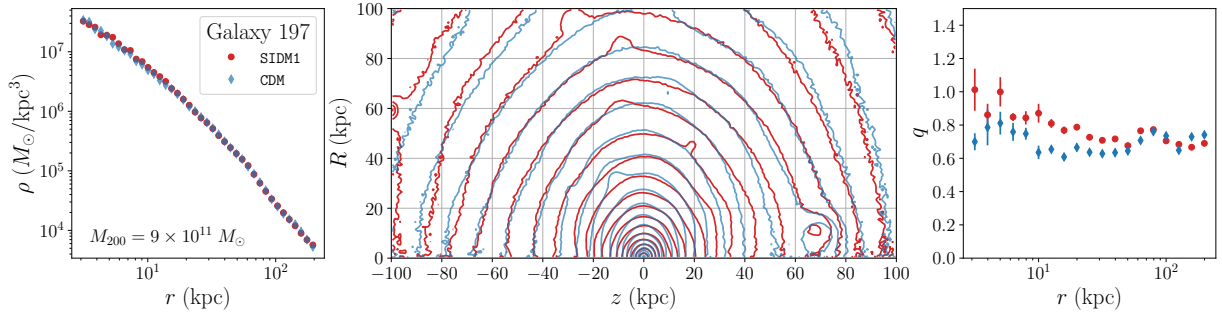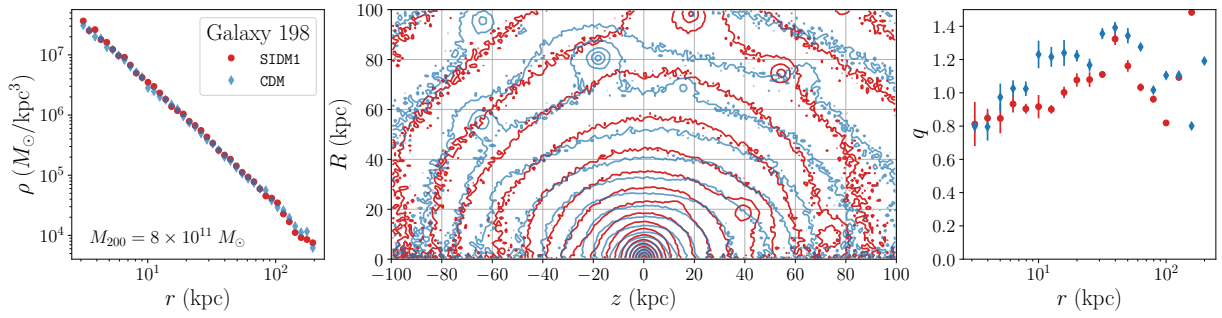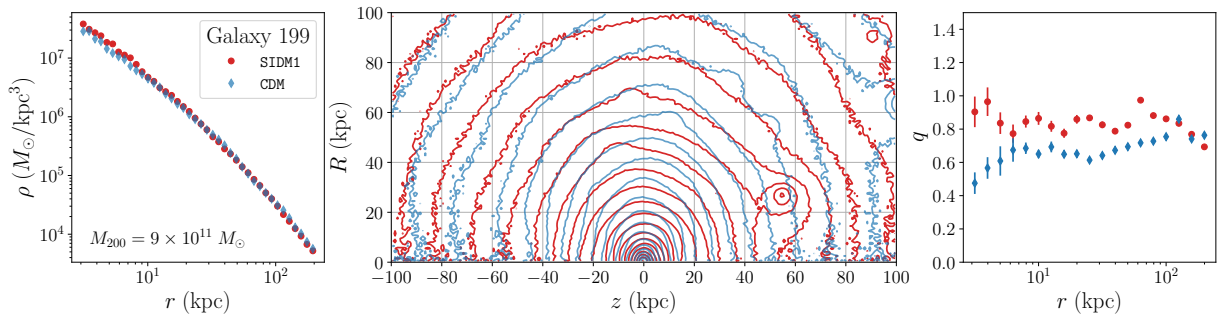

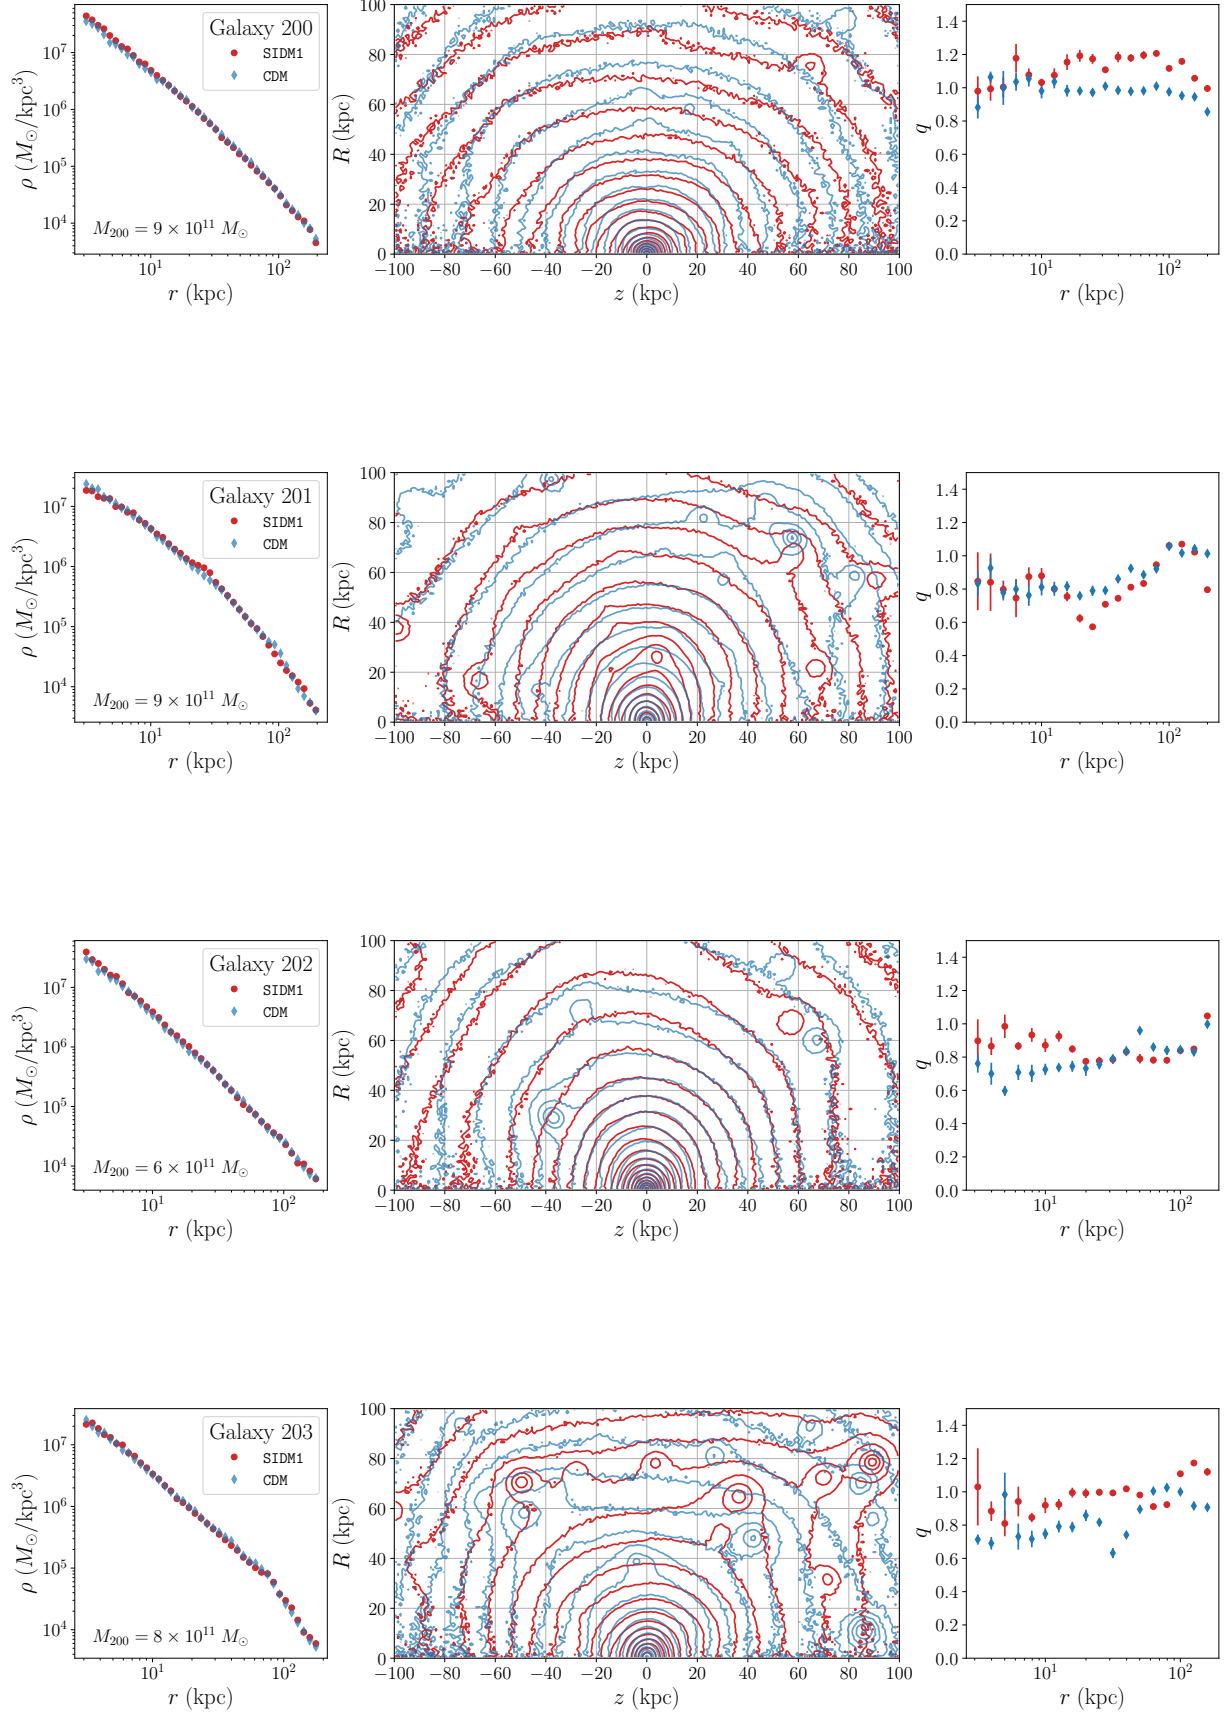

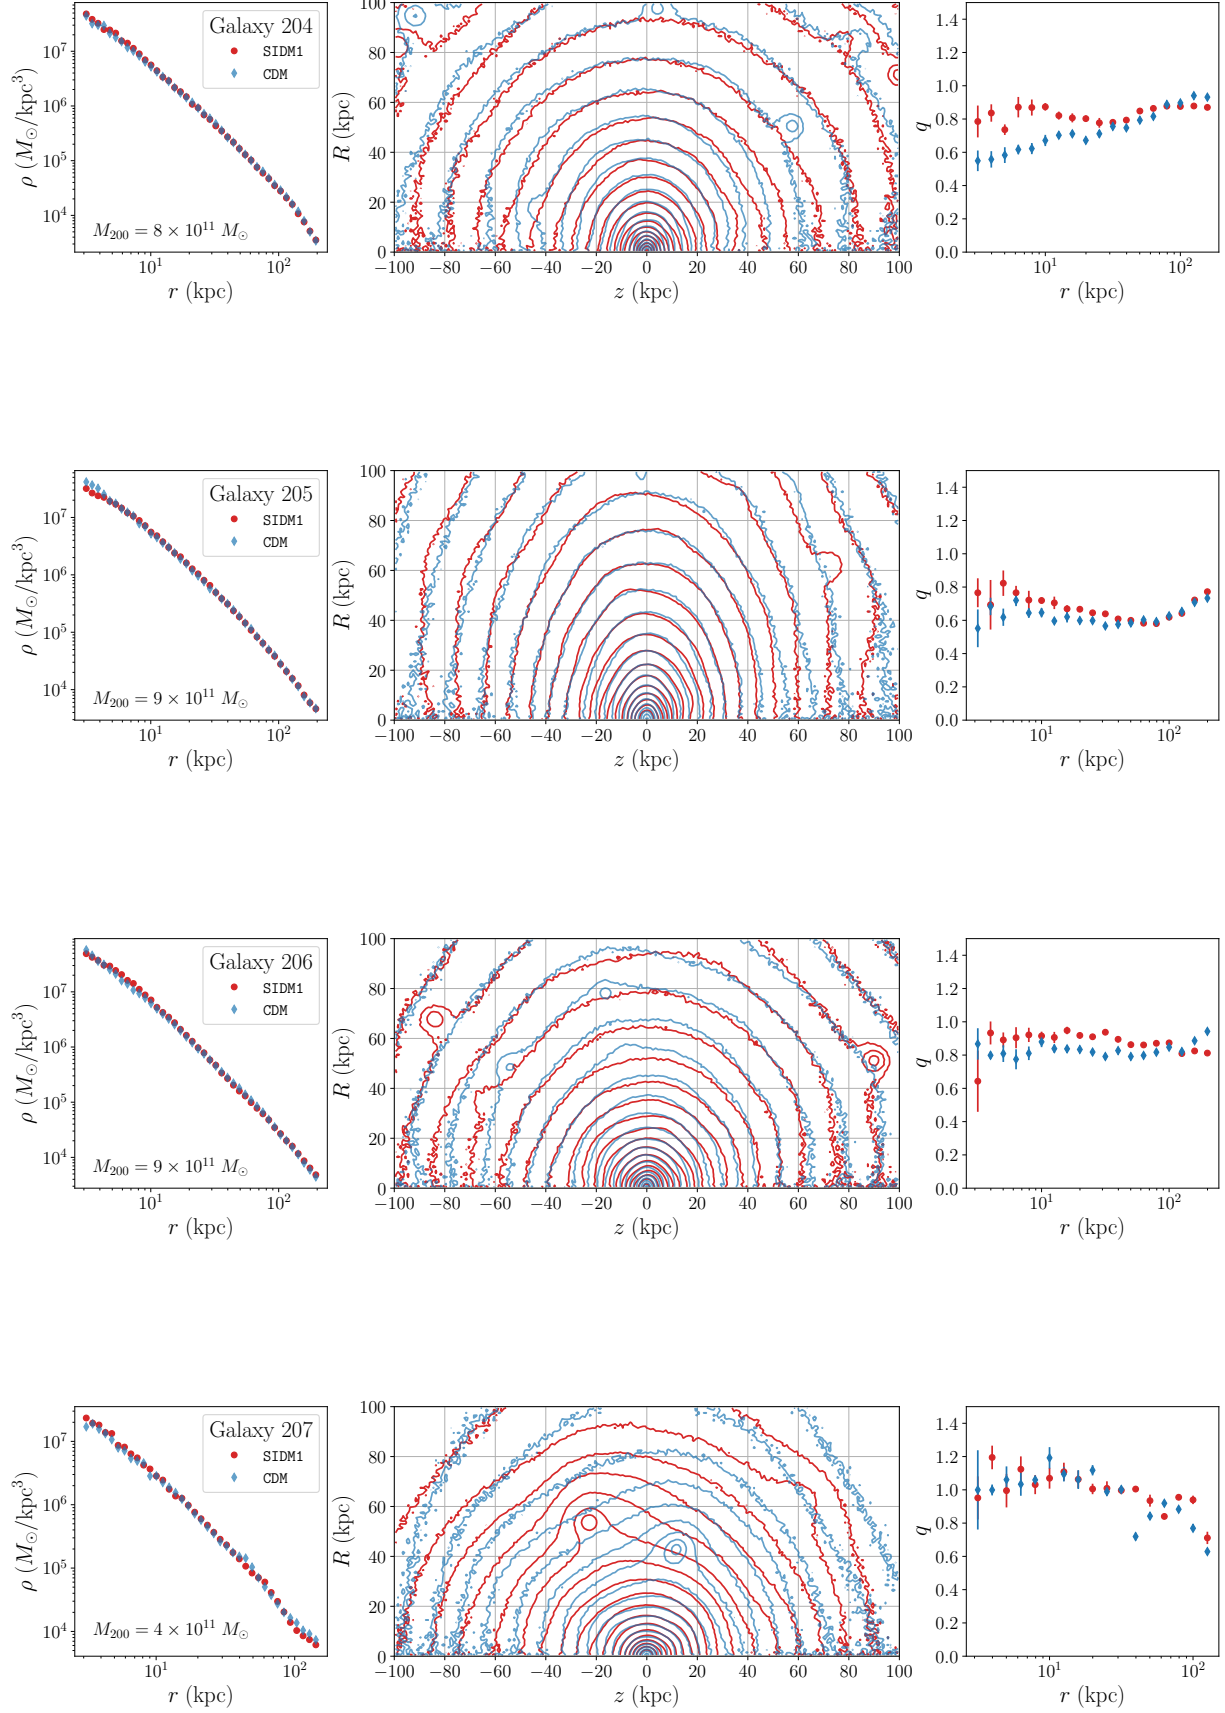

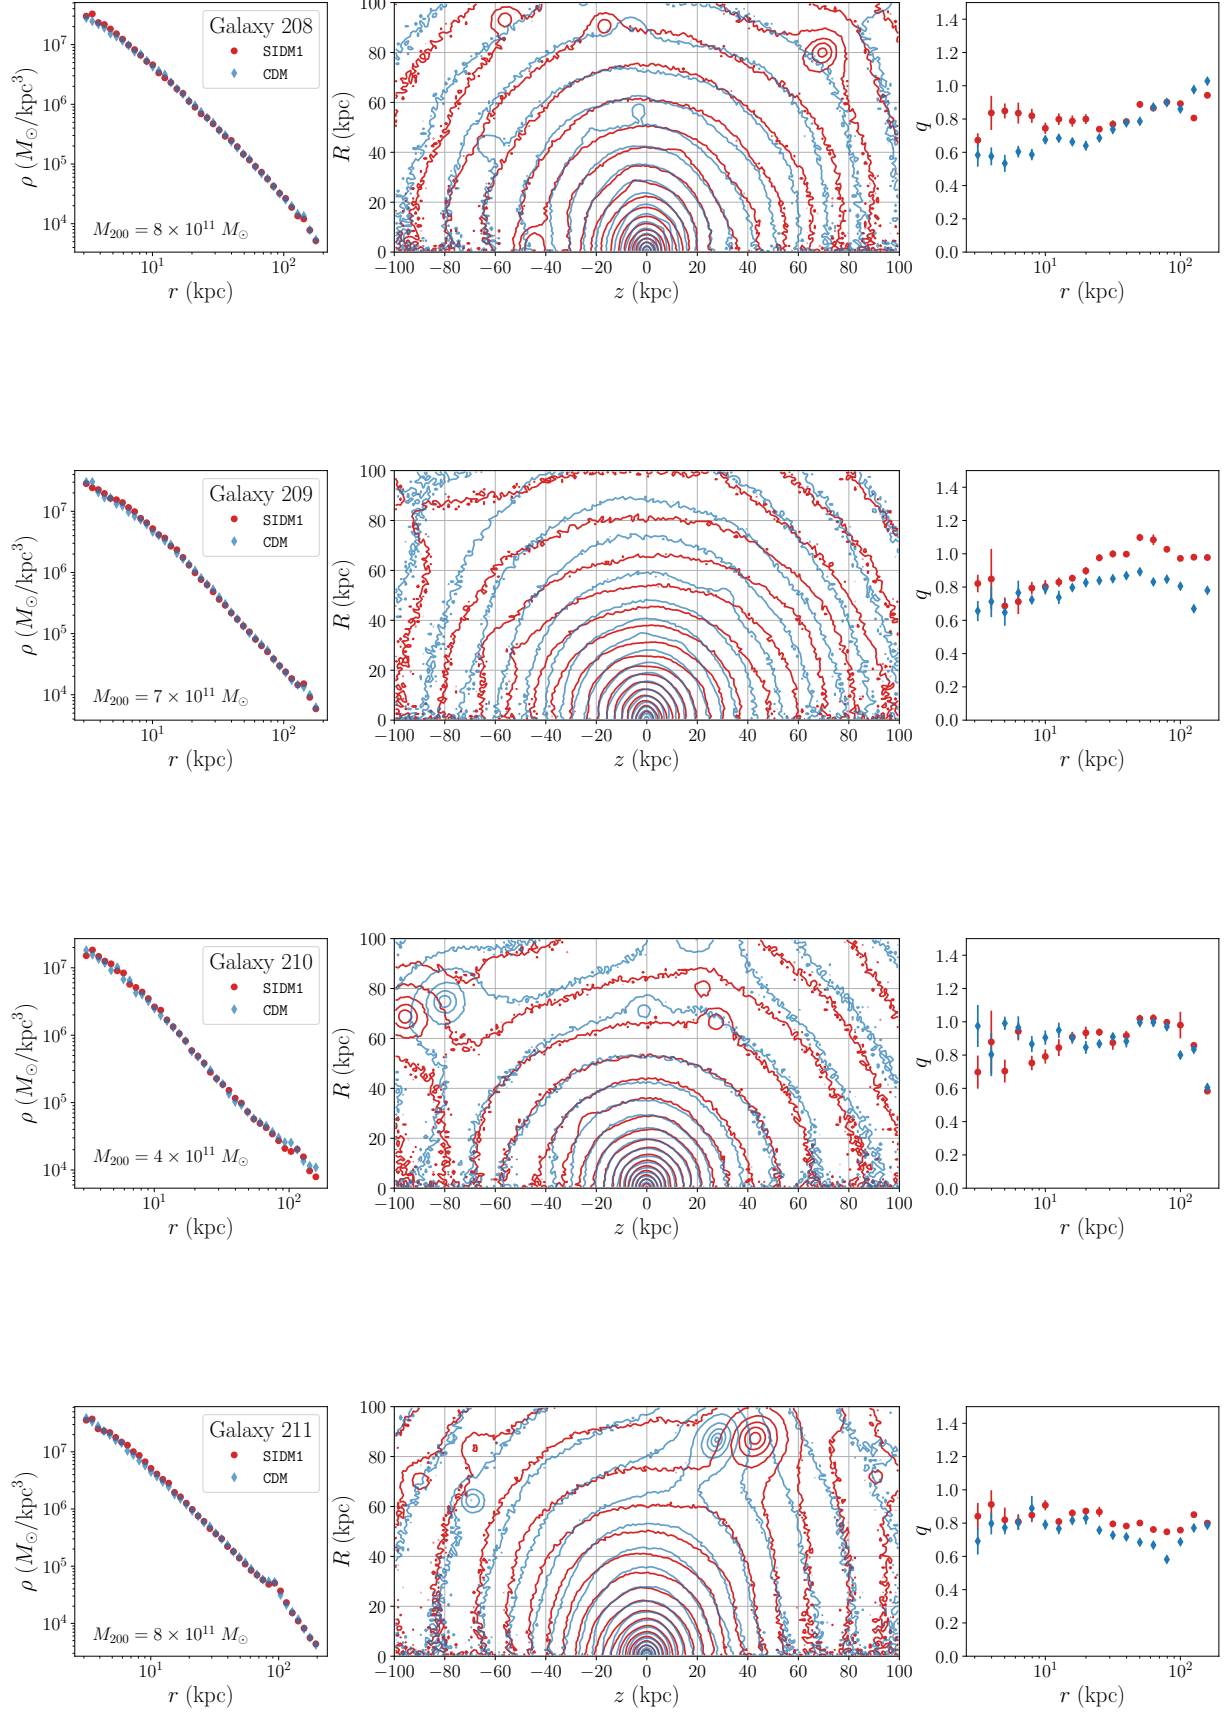



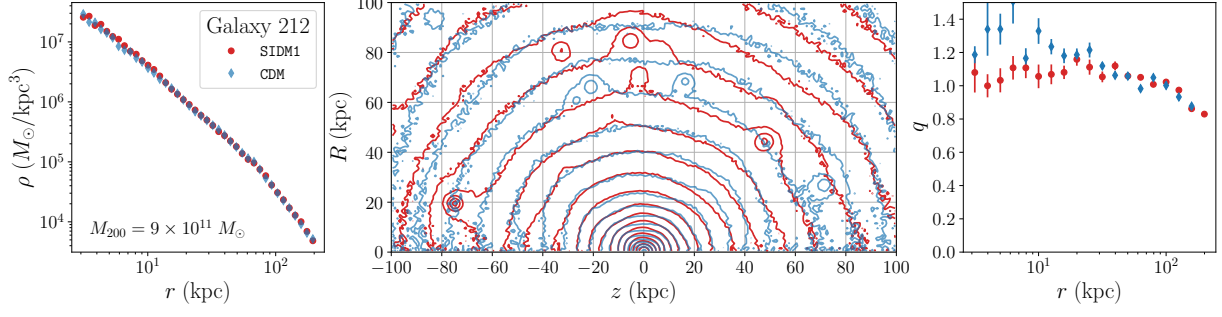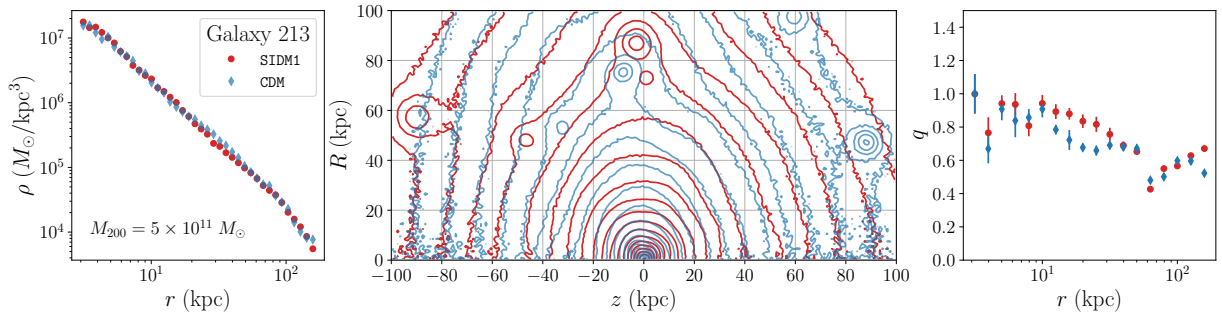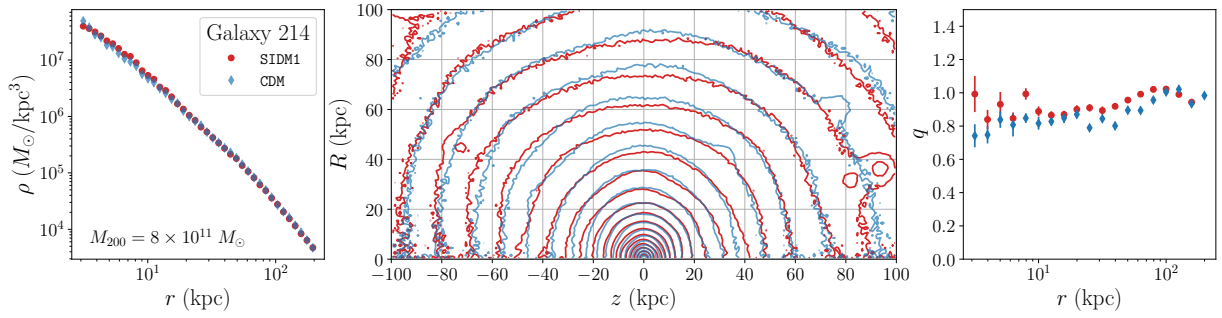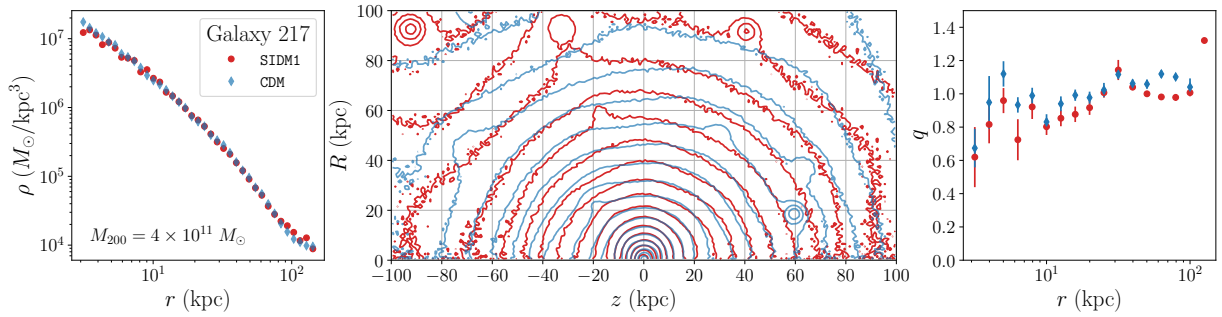

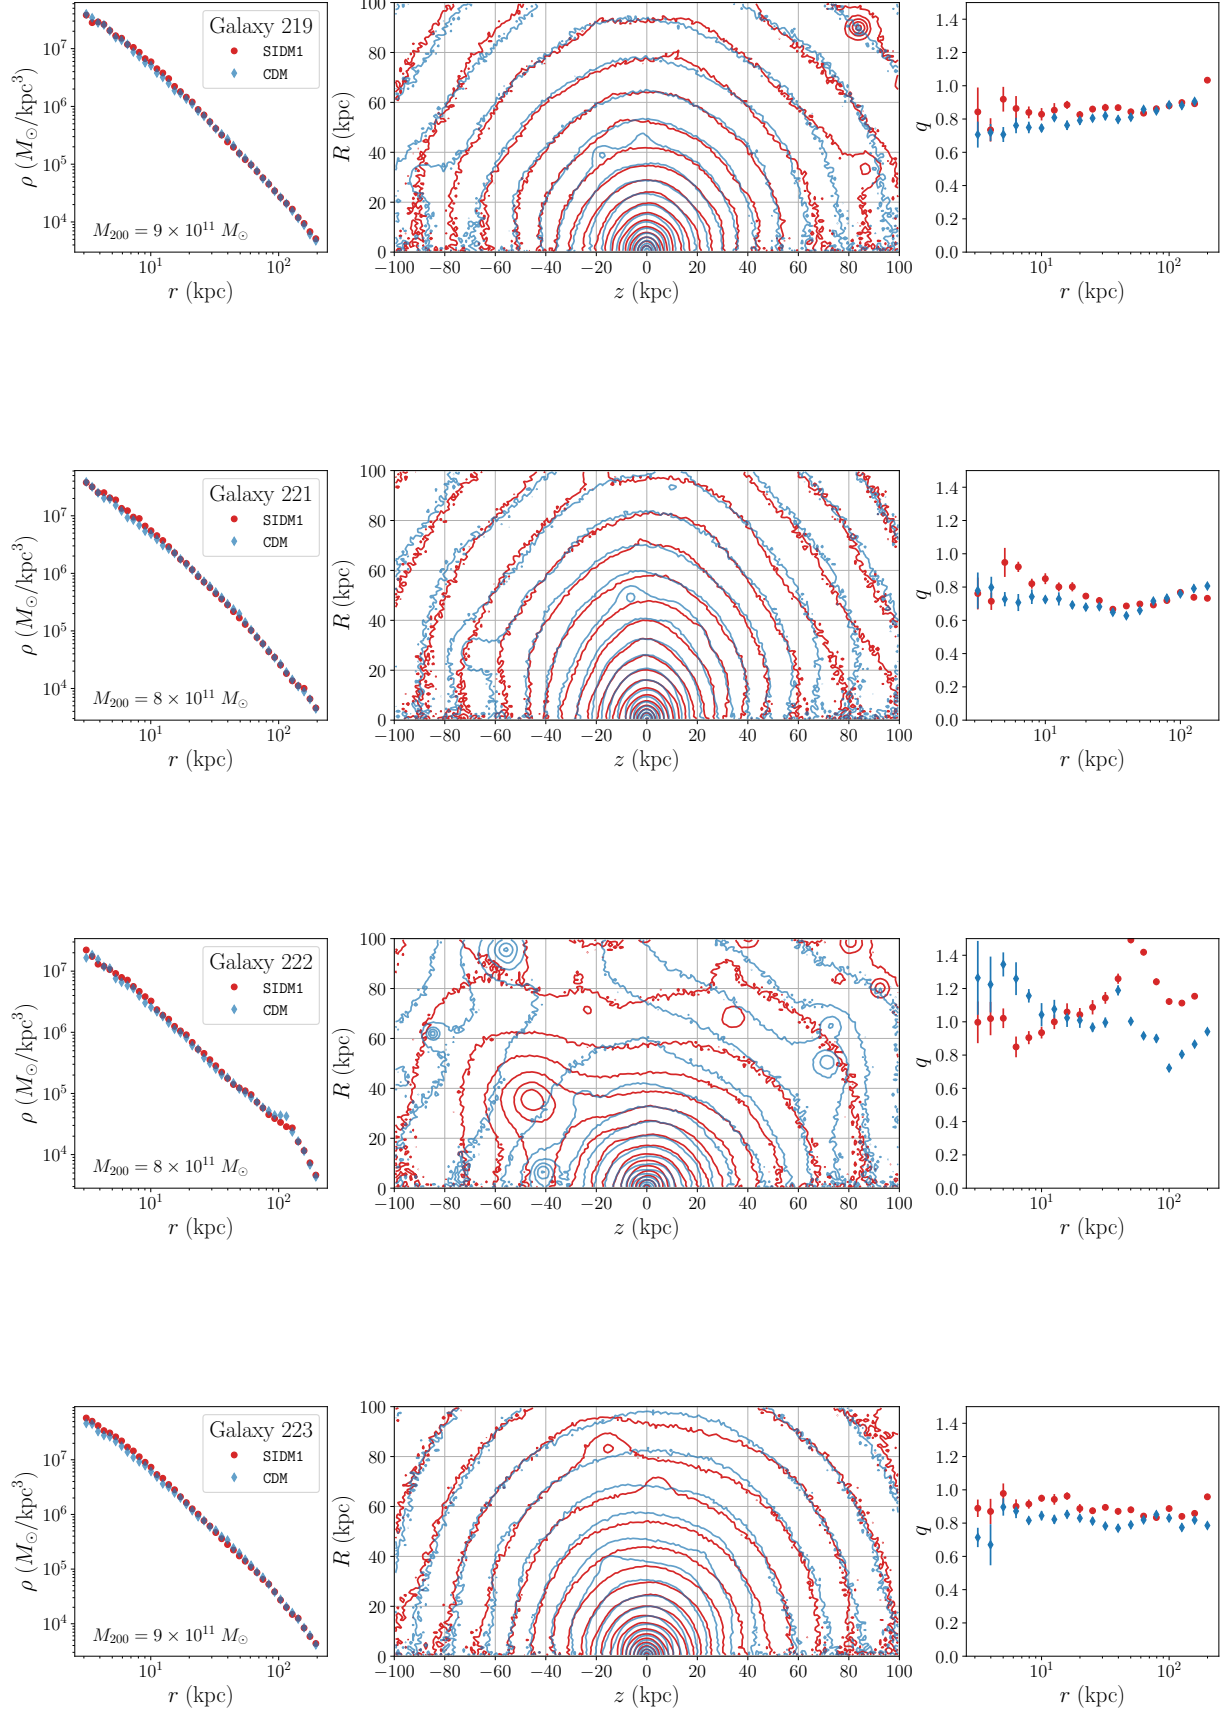

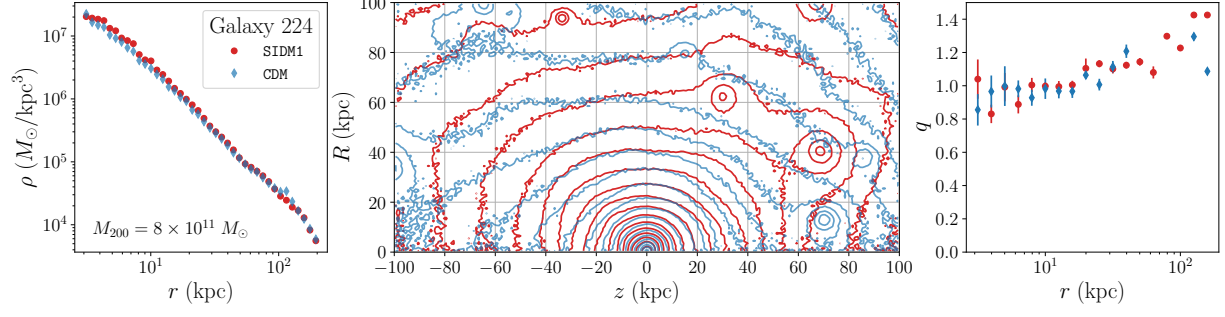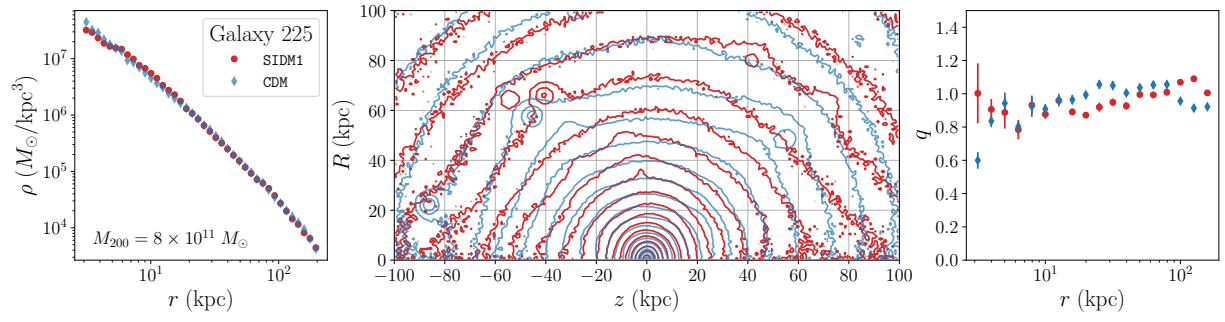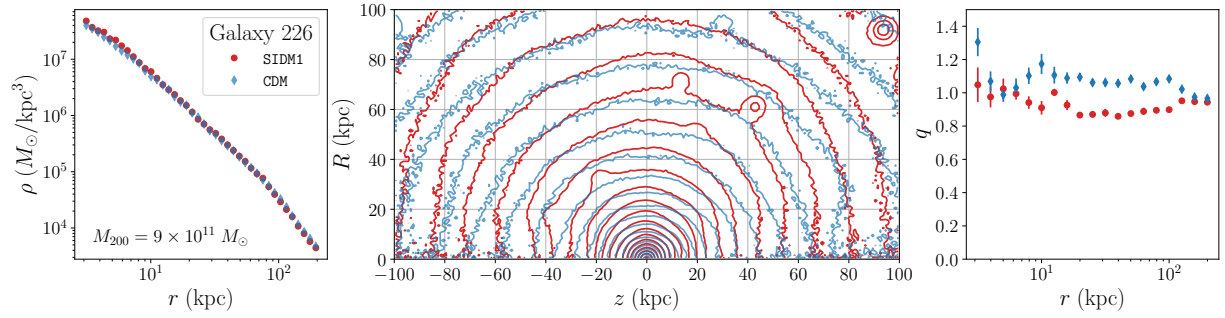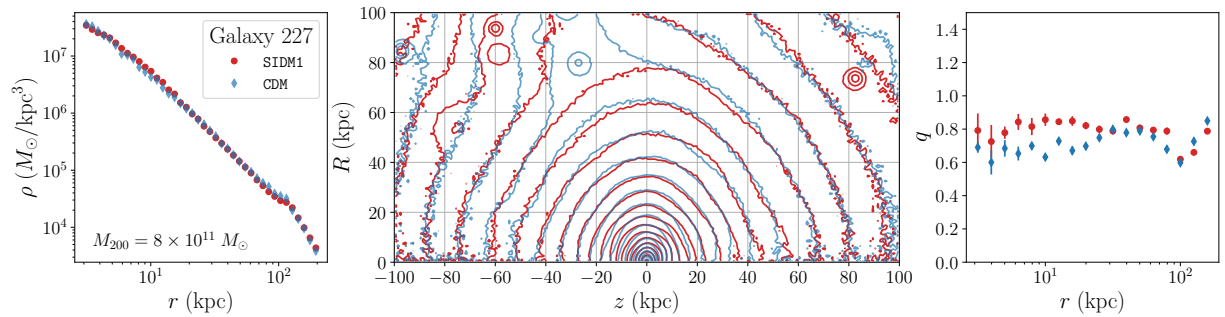

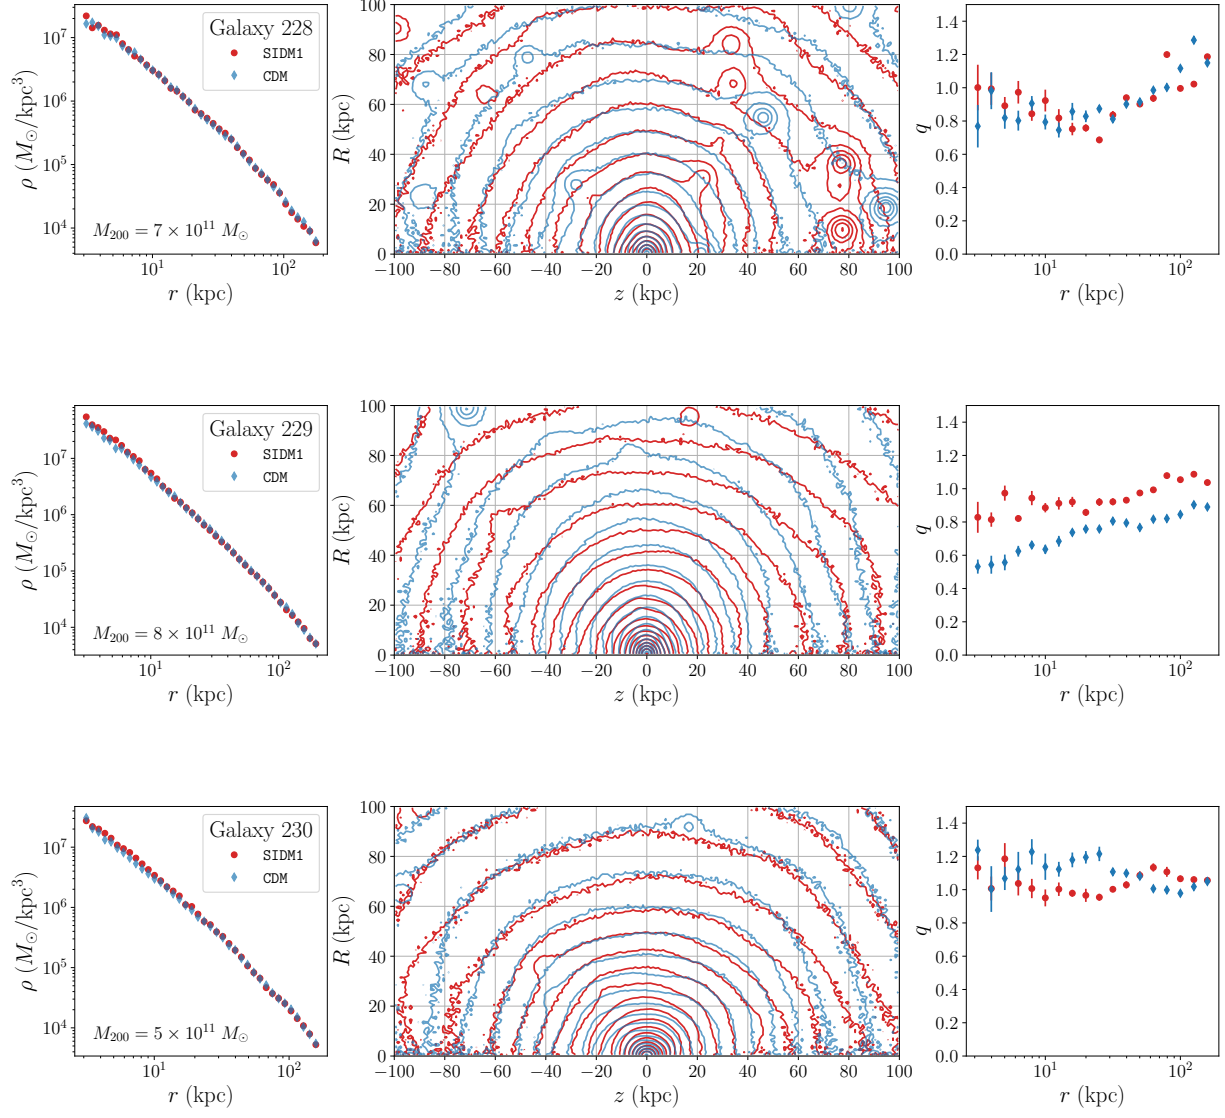


---

[1] A. Robertson et al., Mon. Not. Roy. Astron. Soc. 501 (2021) 4610, 2009.07844.
