# Supplementary material for: Jeans Model for the Shapes of Self-interacting Dark Matter Halos
Source: arXiv:2511.10765 ancillary file (2025-11-13)
Supplement: Supplementary file 2 [file Ancillary2.pdf]

## Ancillary material 2: Modeling the CDM halos in the Eagle-50 simulations set. This material is associated to the submission, Jeans Model for the Shapes of Self-interacting Dark Matter Halos

Yilber Fabian Bautista, Andrew Robertson, Laura Sagunski, Adam Smith-Orlik, and Sean Tulin

The plots in this ancillary file compare various analytic models for the spherically averaged density profiles (left panels) and halo shape profiles (center panels) of the CDM systems in the EAGLE-50 simulation of CDM plus baryons presented in Ref. [1]. The right panels show the results for the analytic (including adiabatic contraction, AC) azimuthally averaged iso-density contours (dashed lines), compared with the simulated data (solid lines). Further details are provided in Section IV-B of the main text.

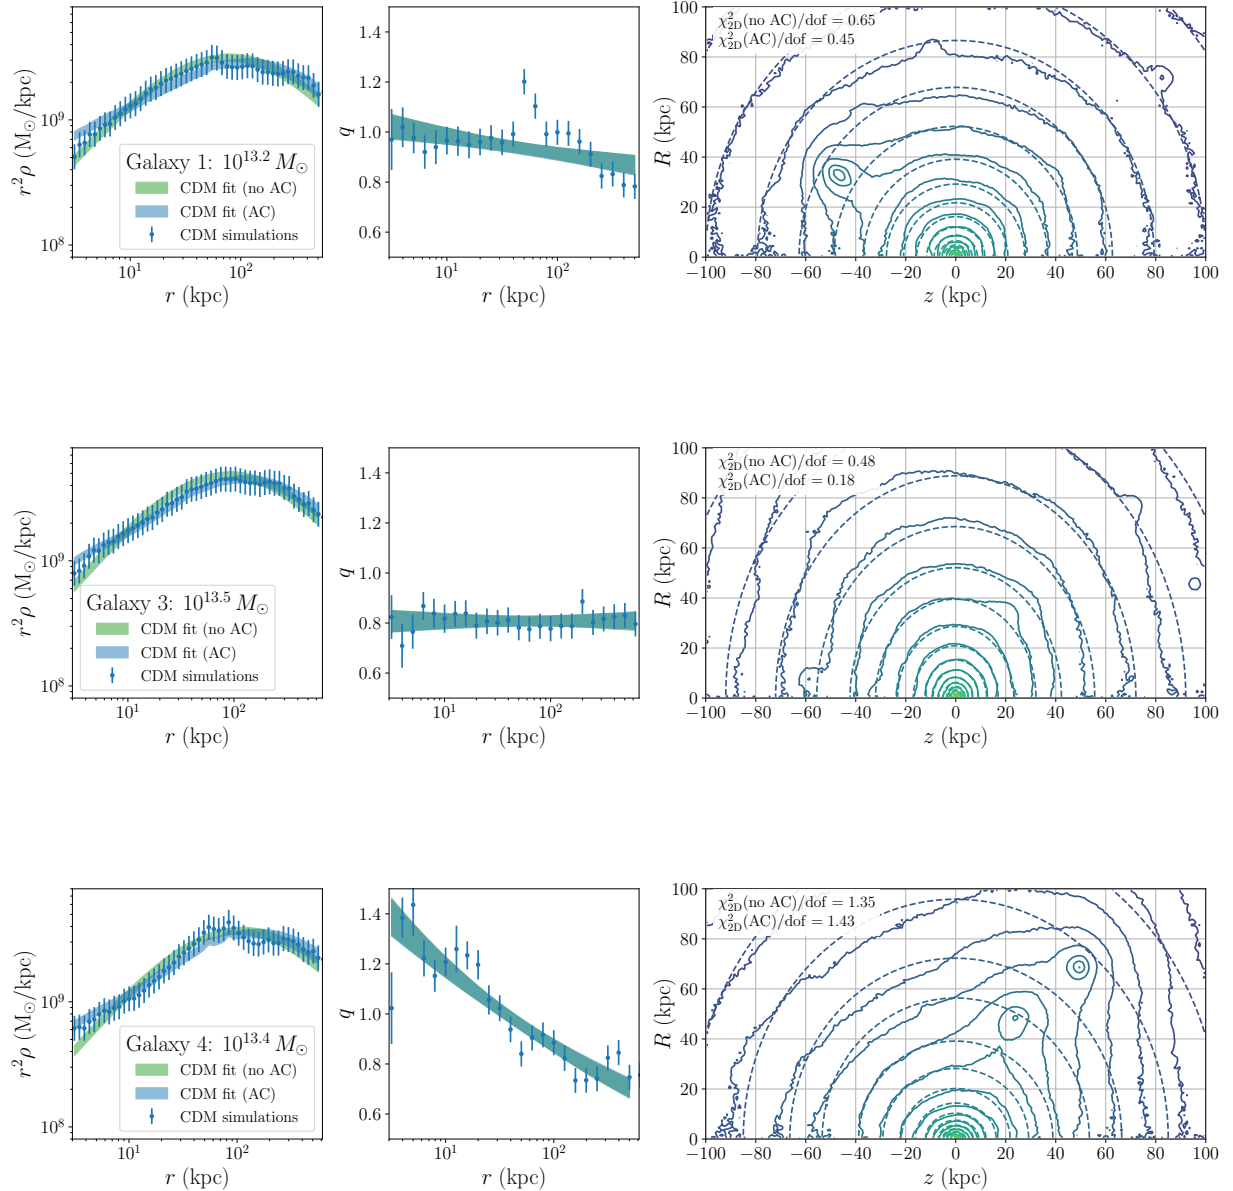

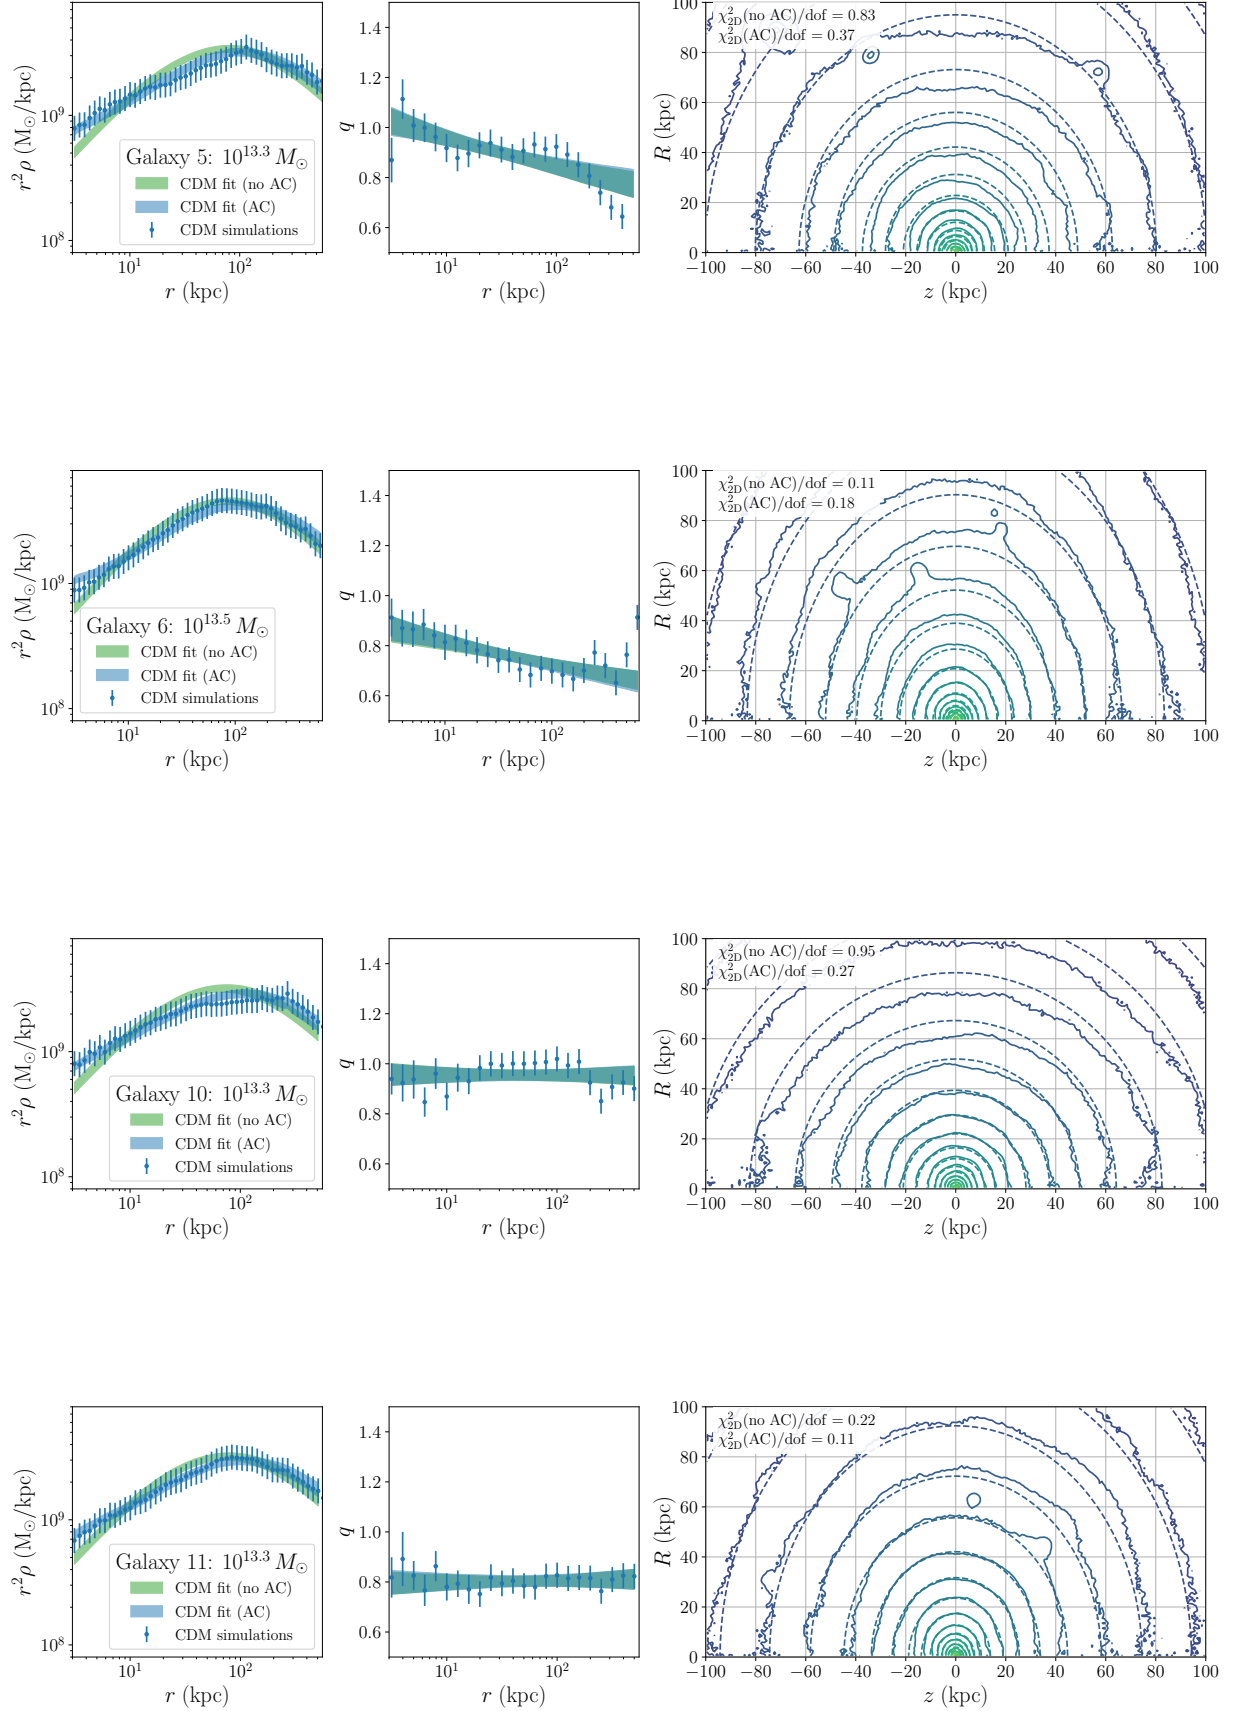

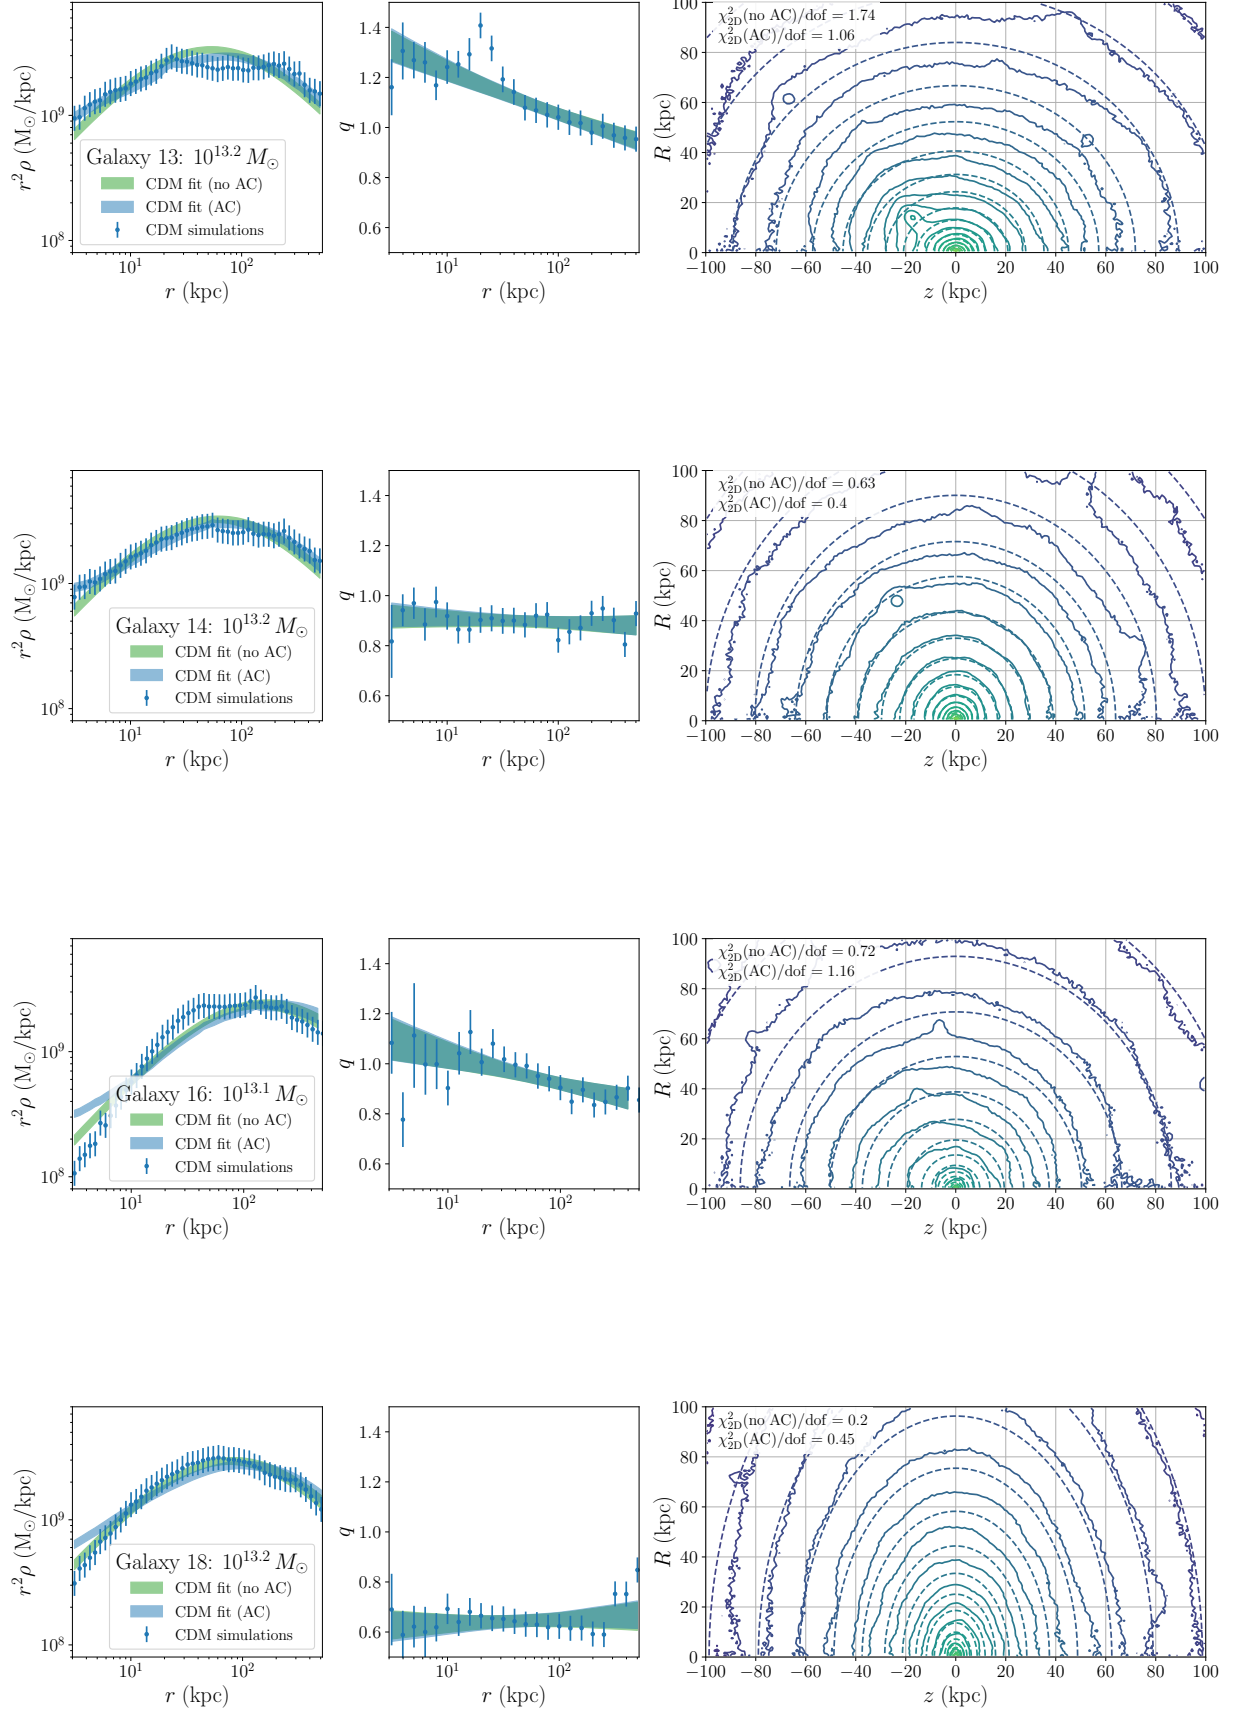

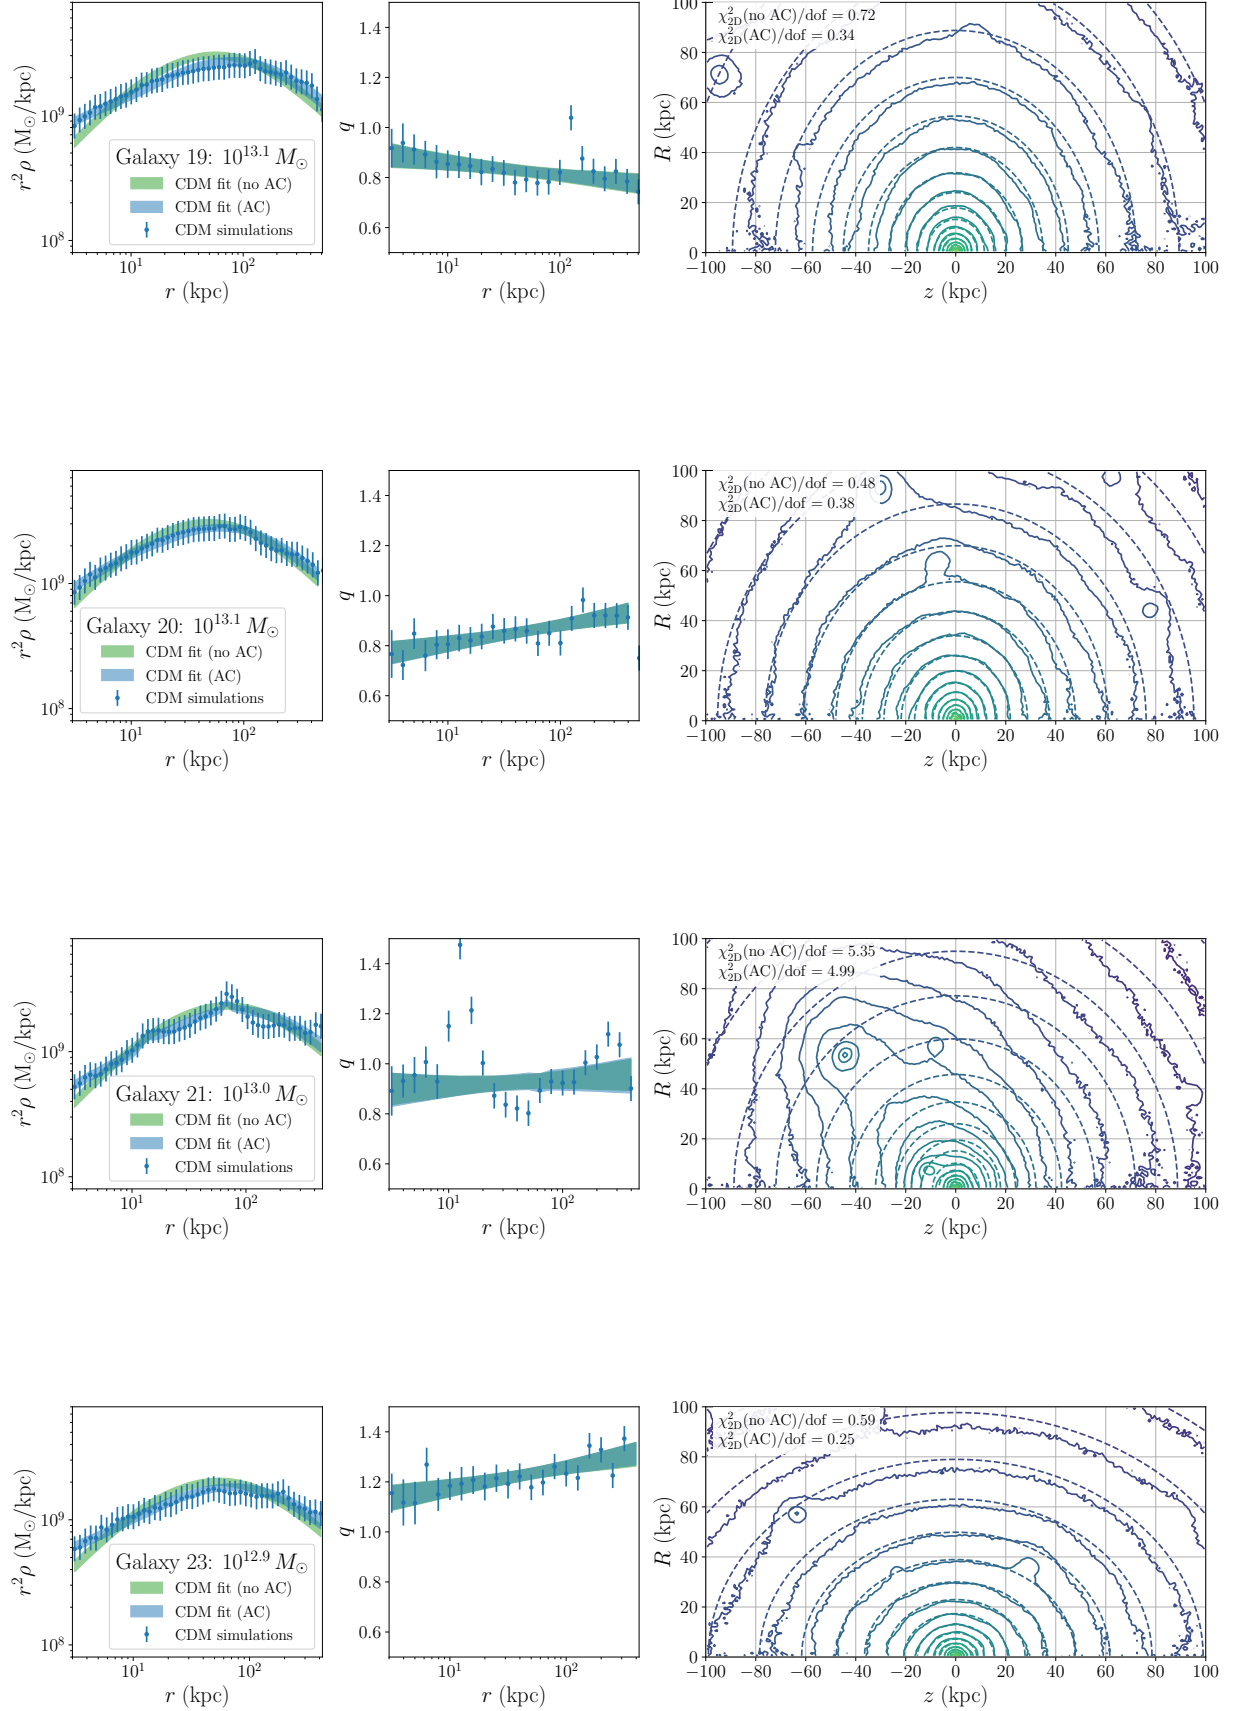



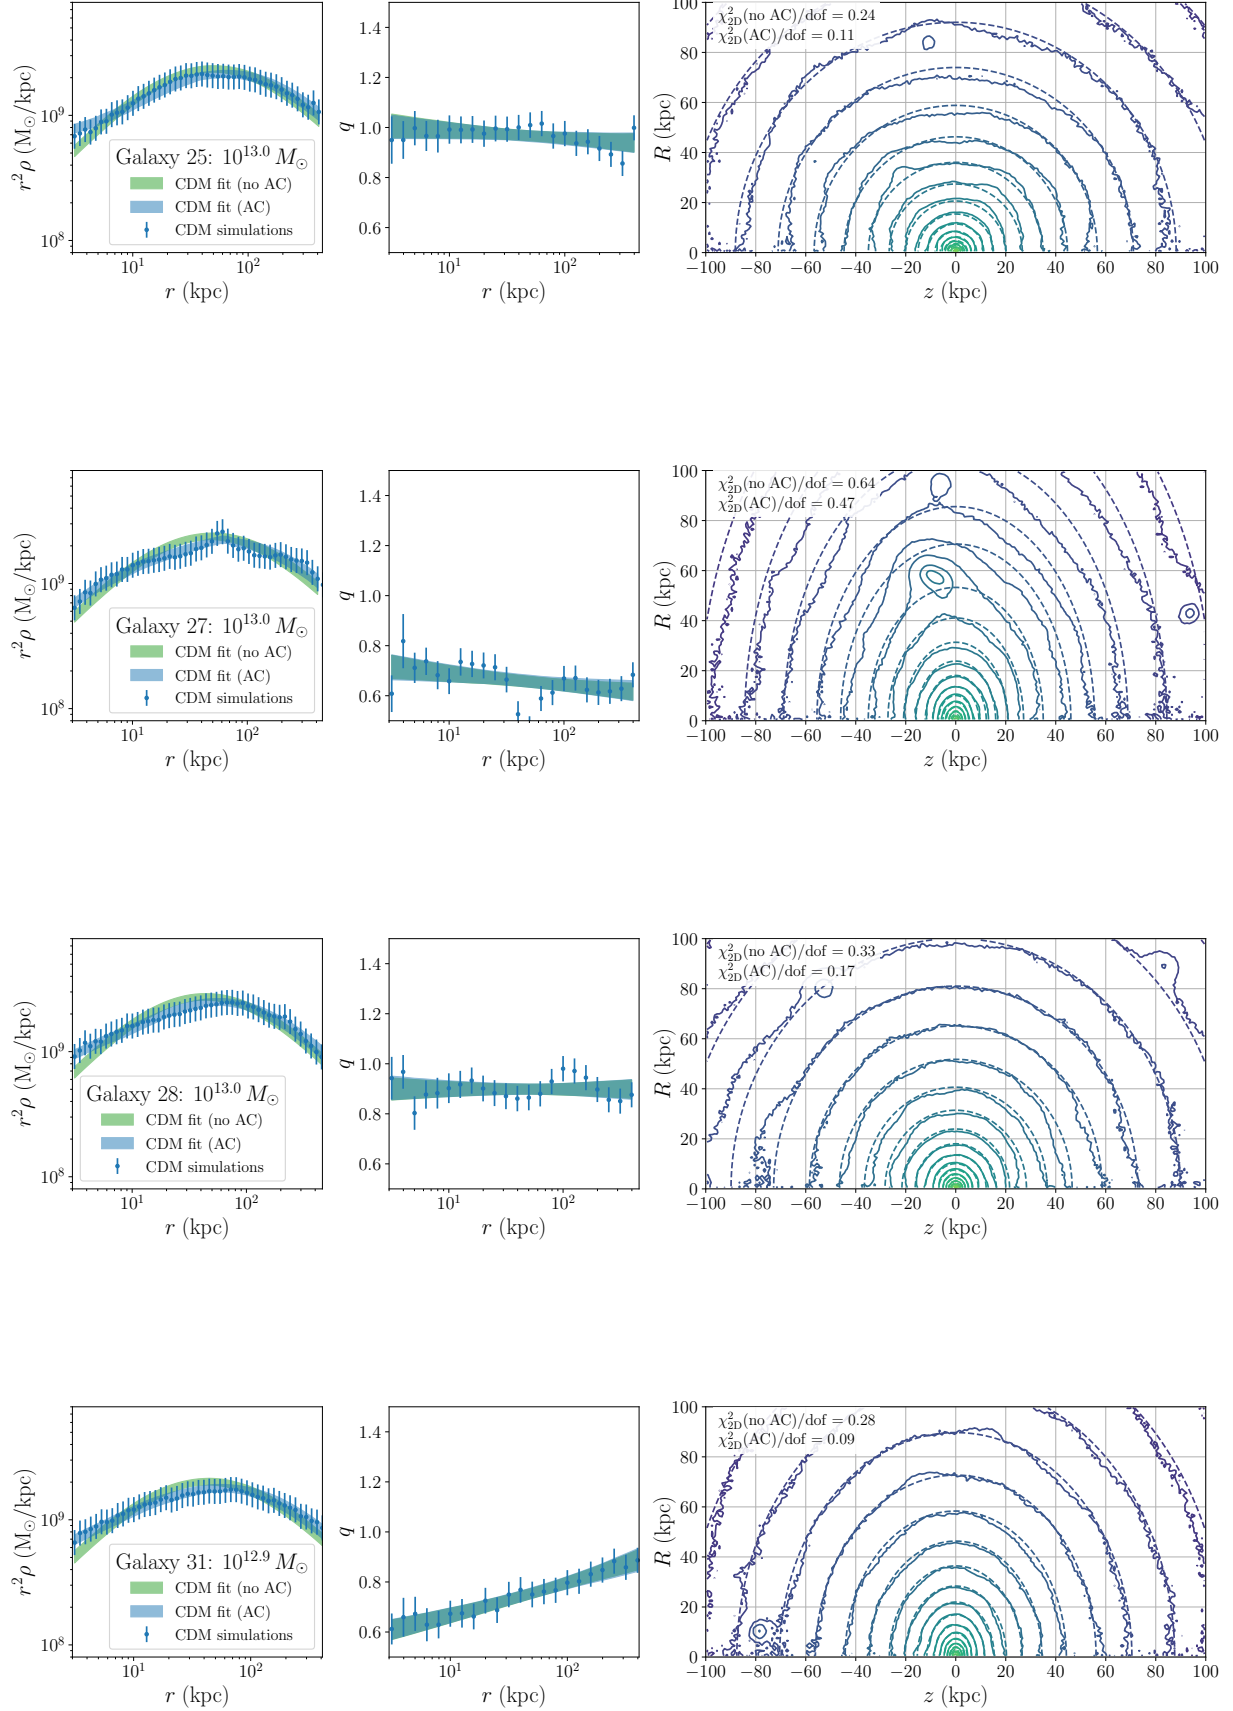

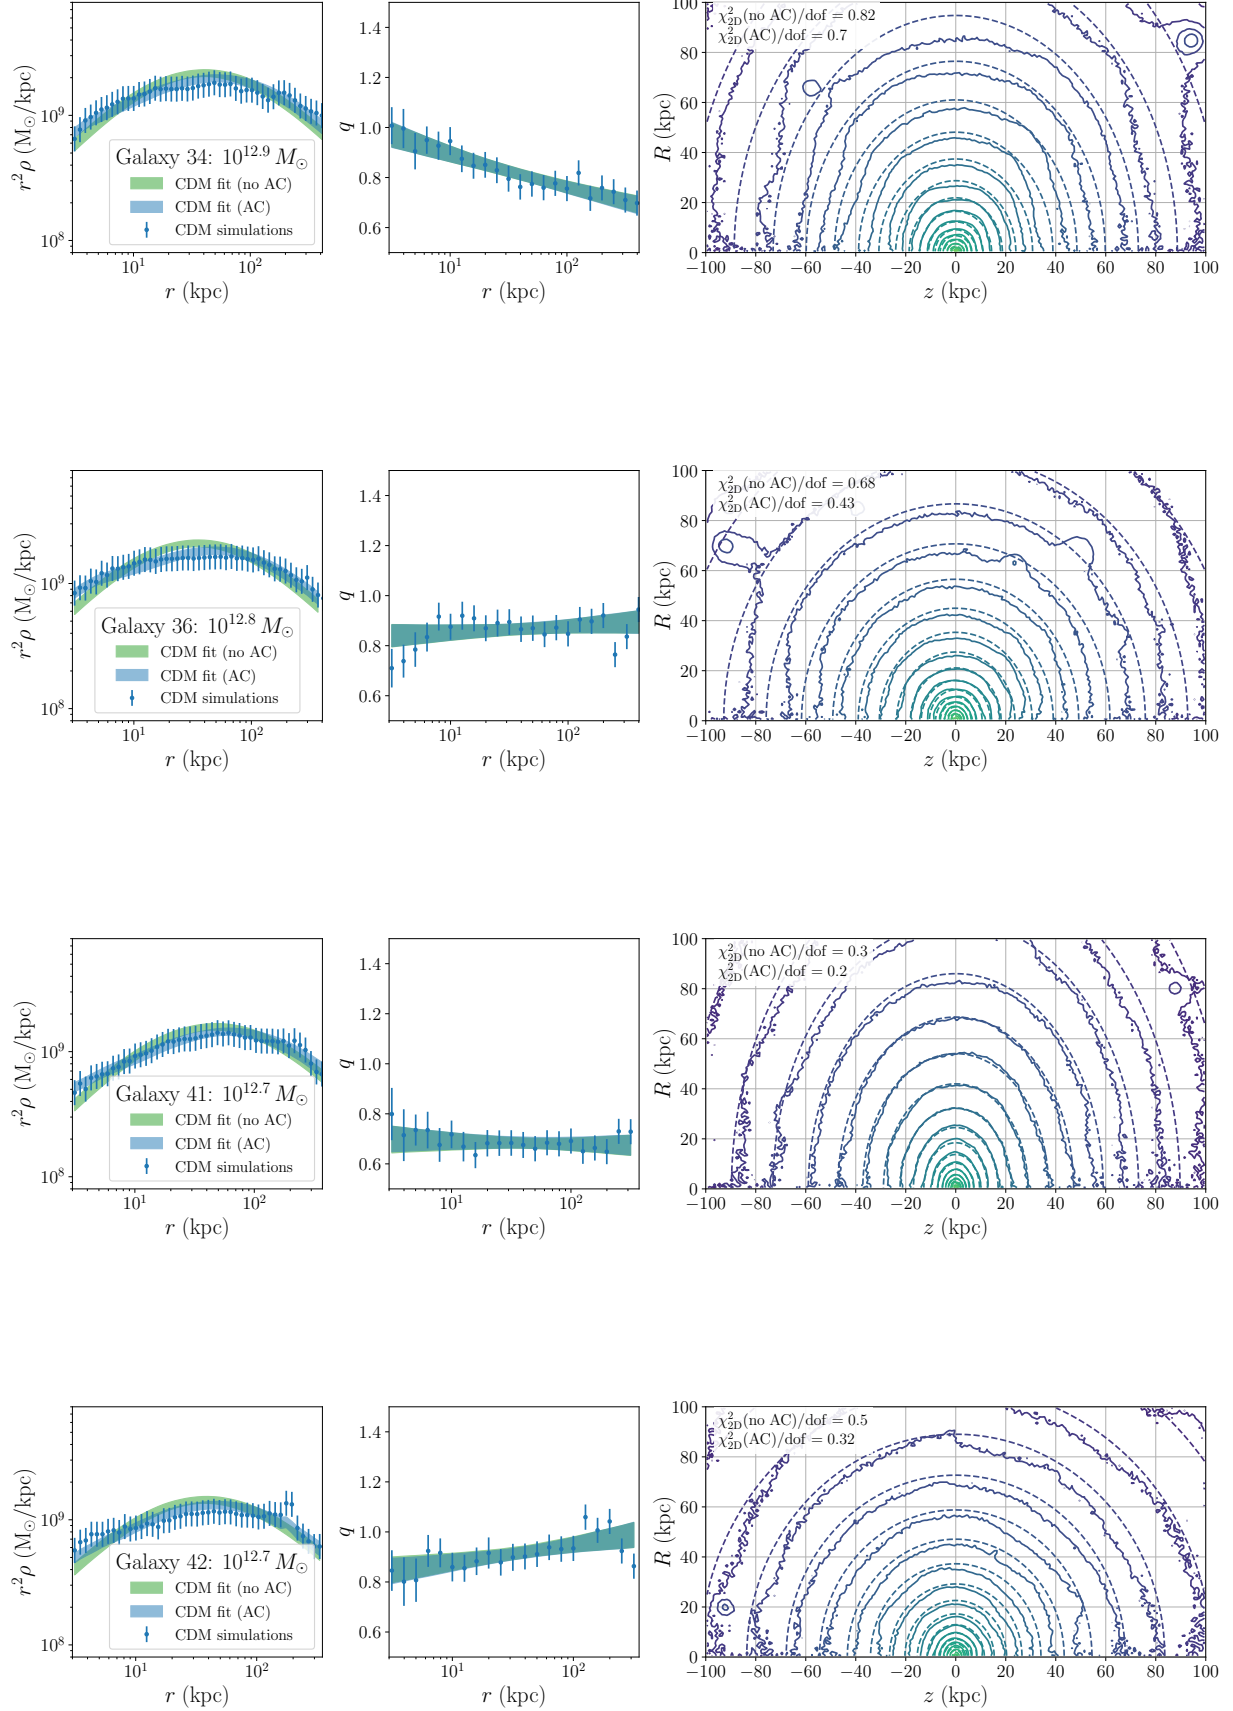

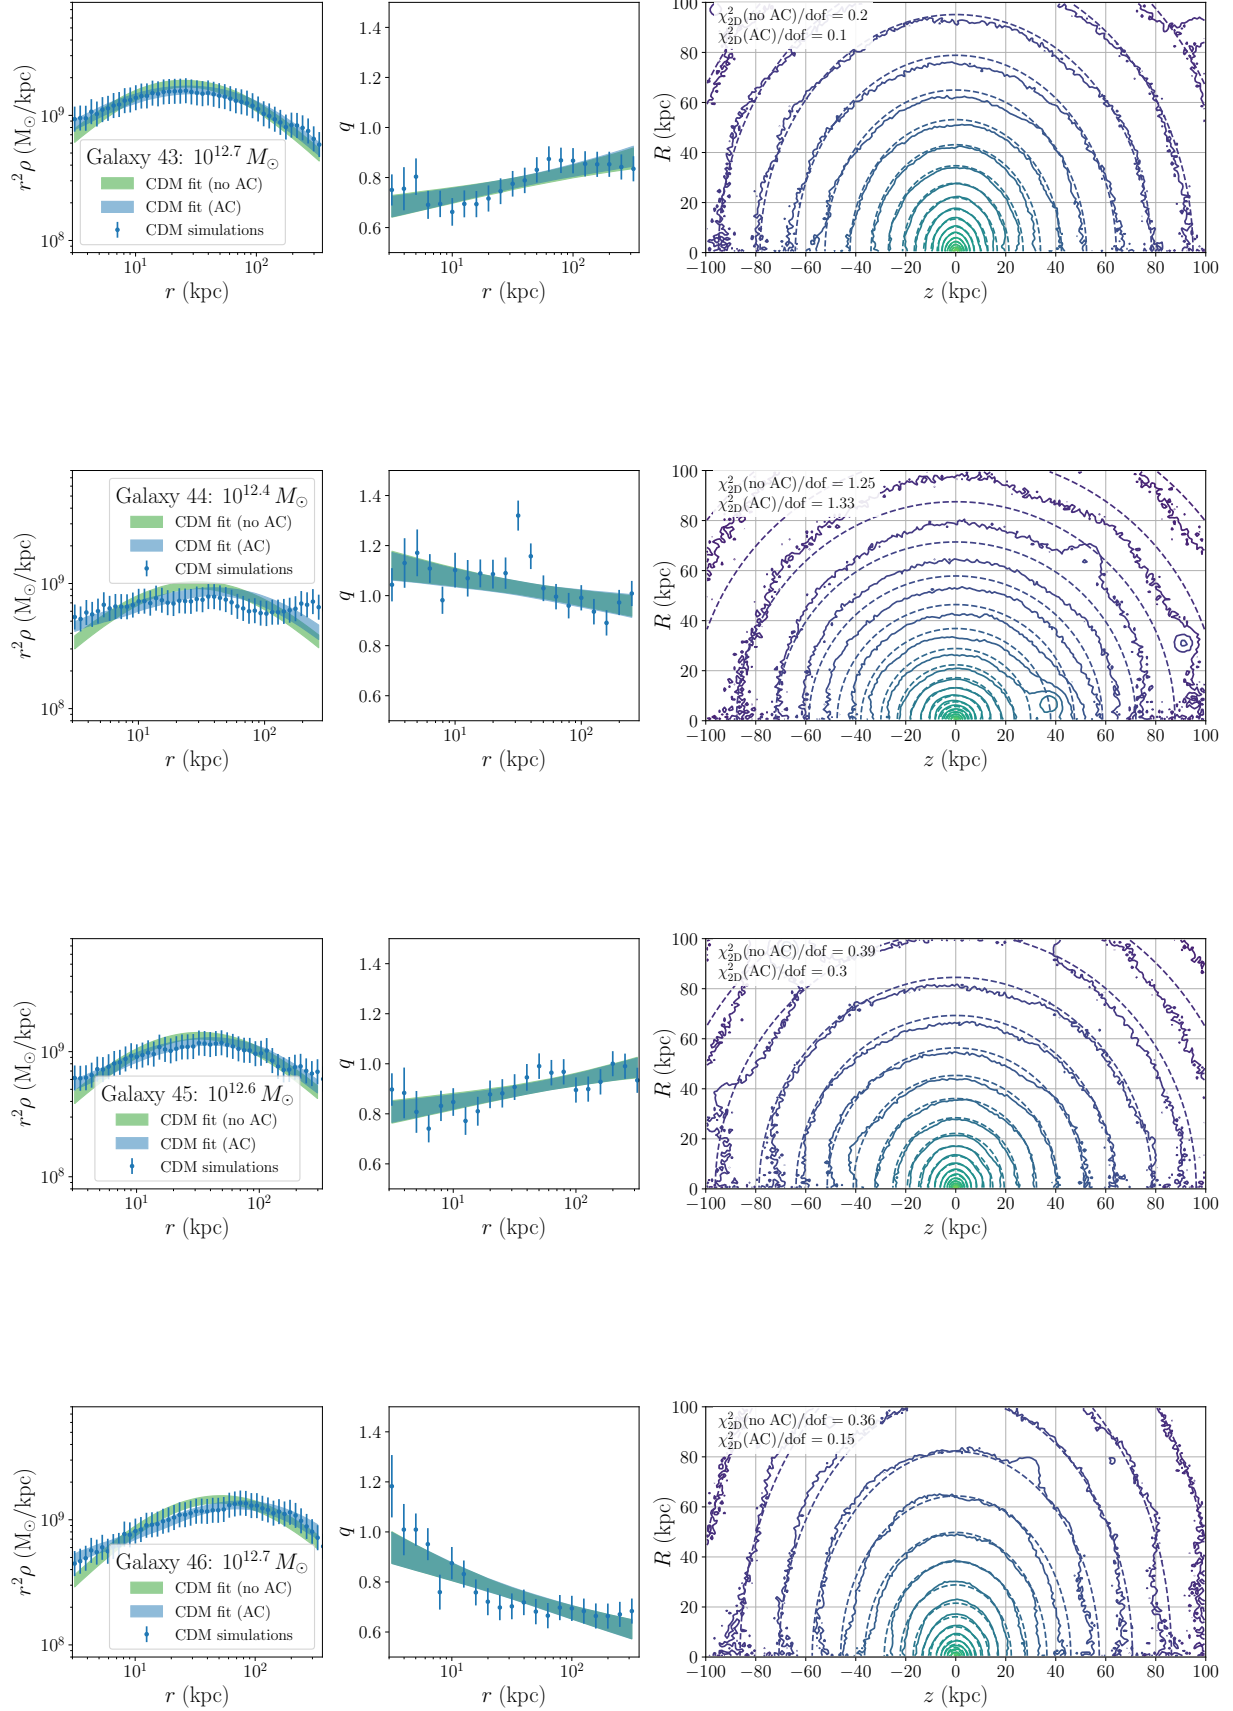

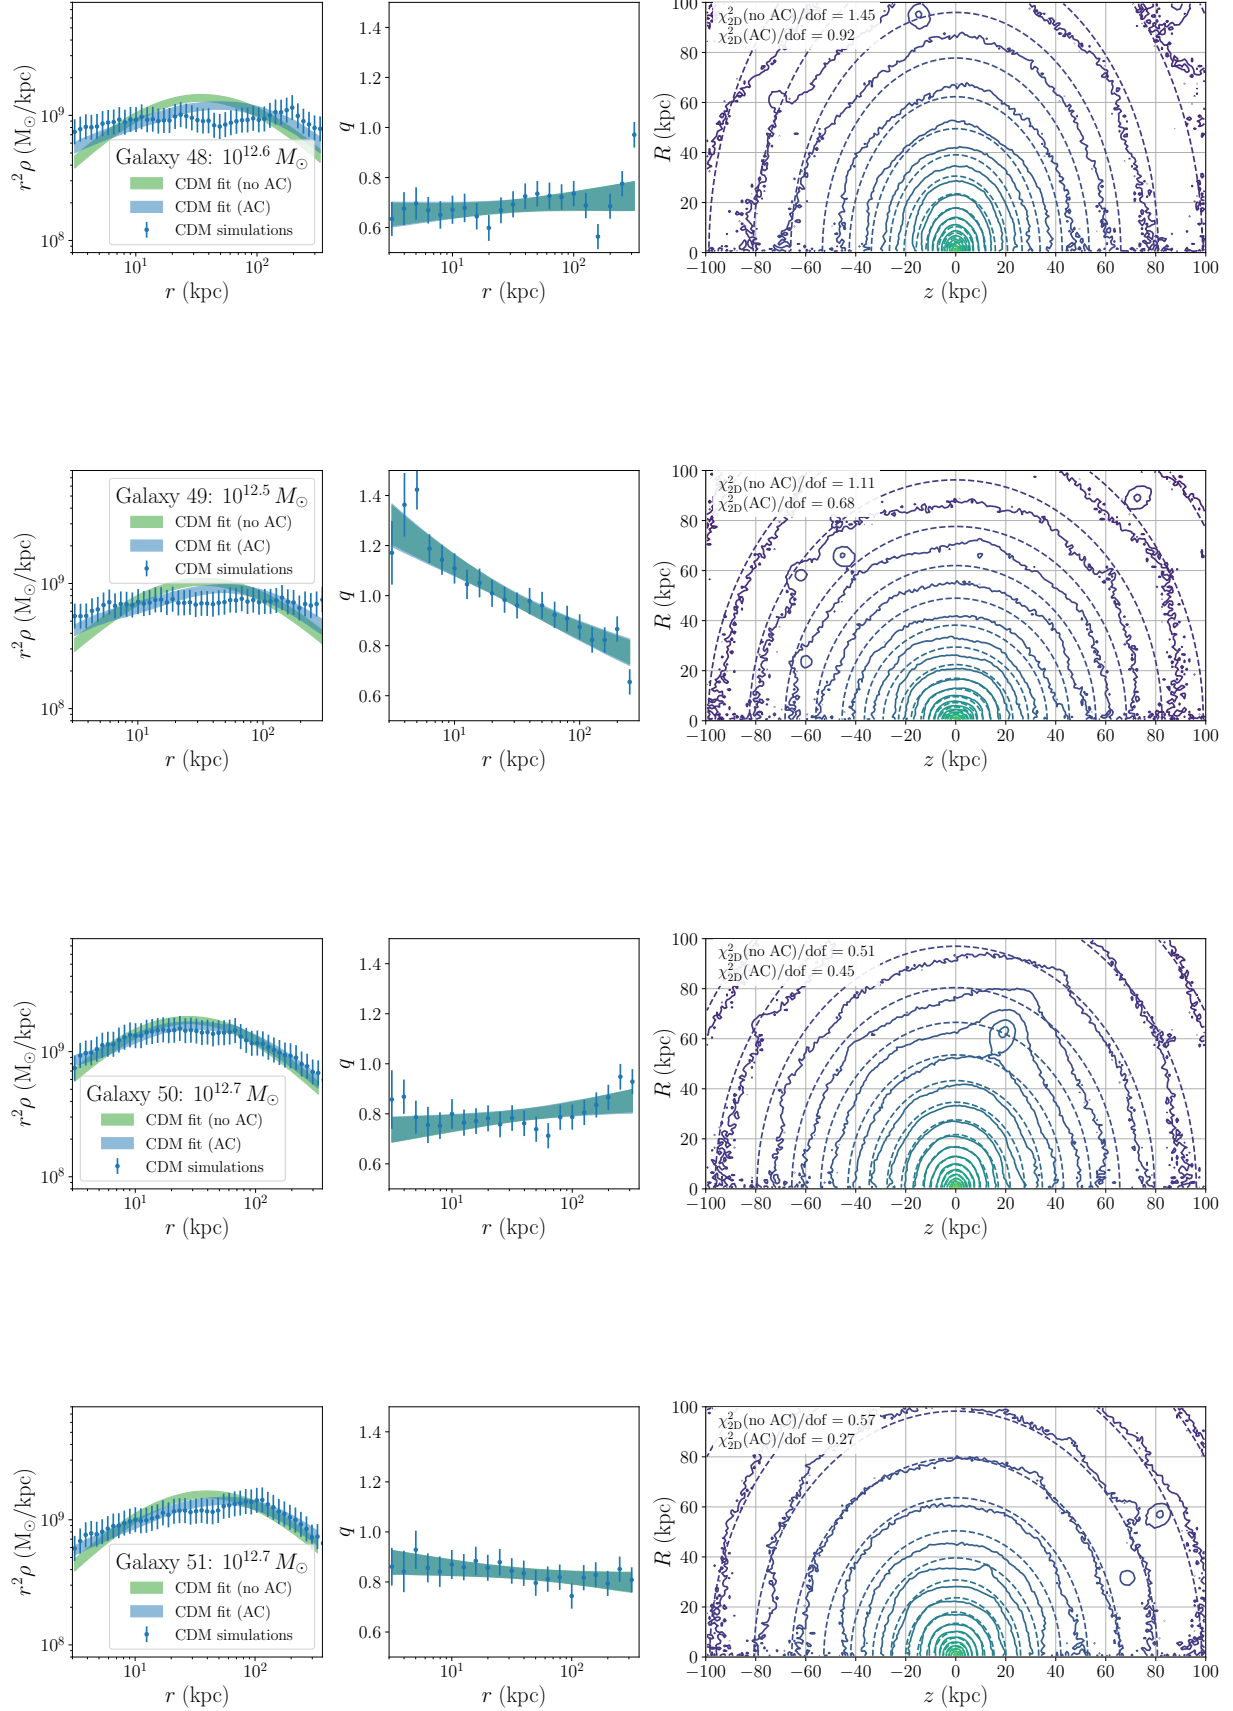

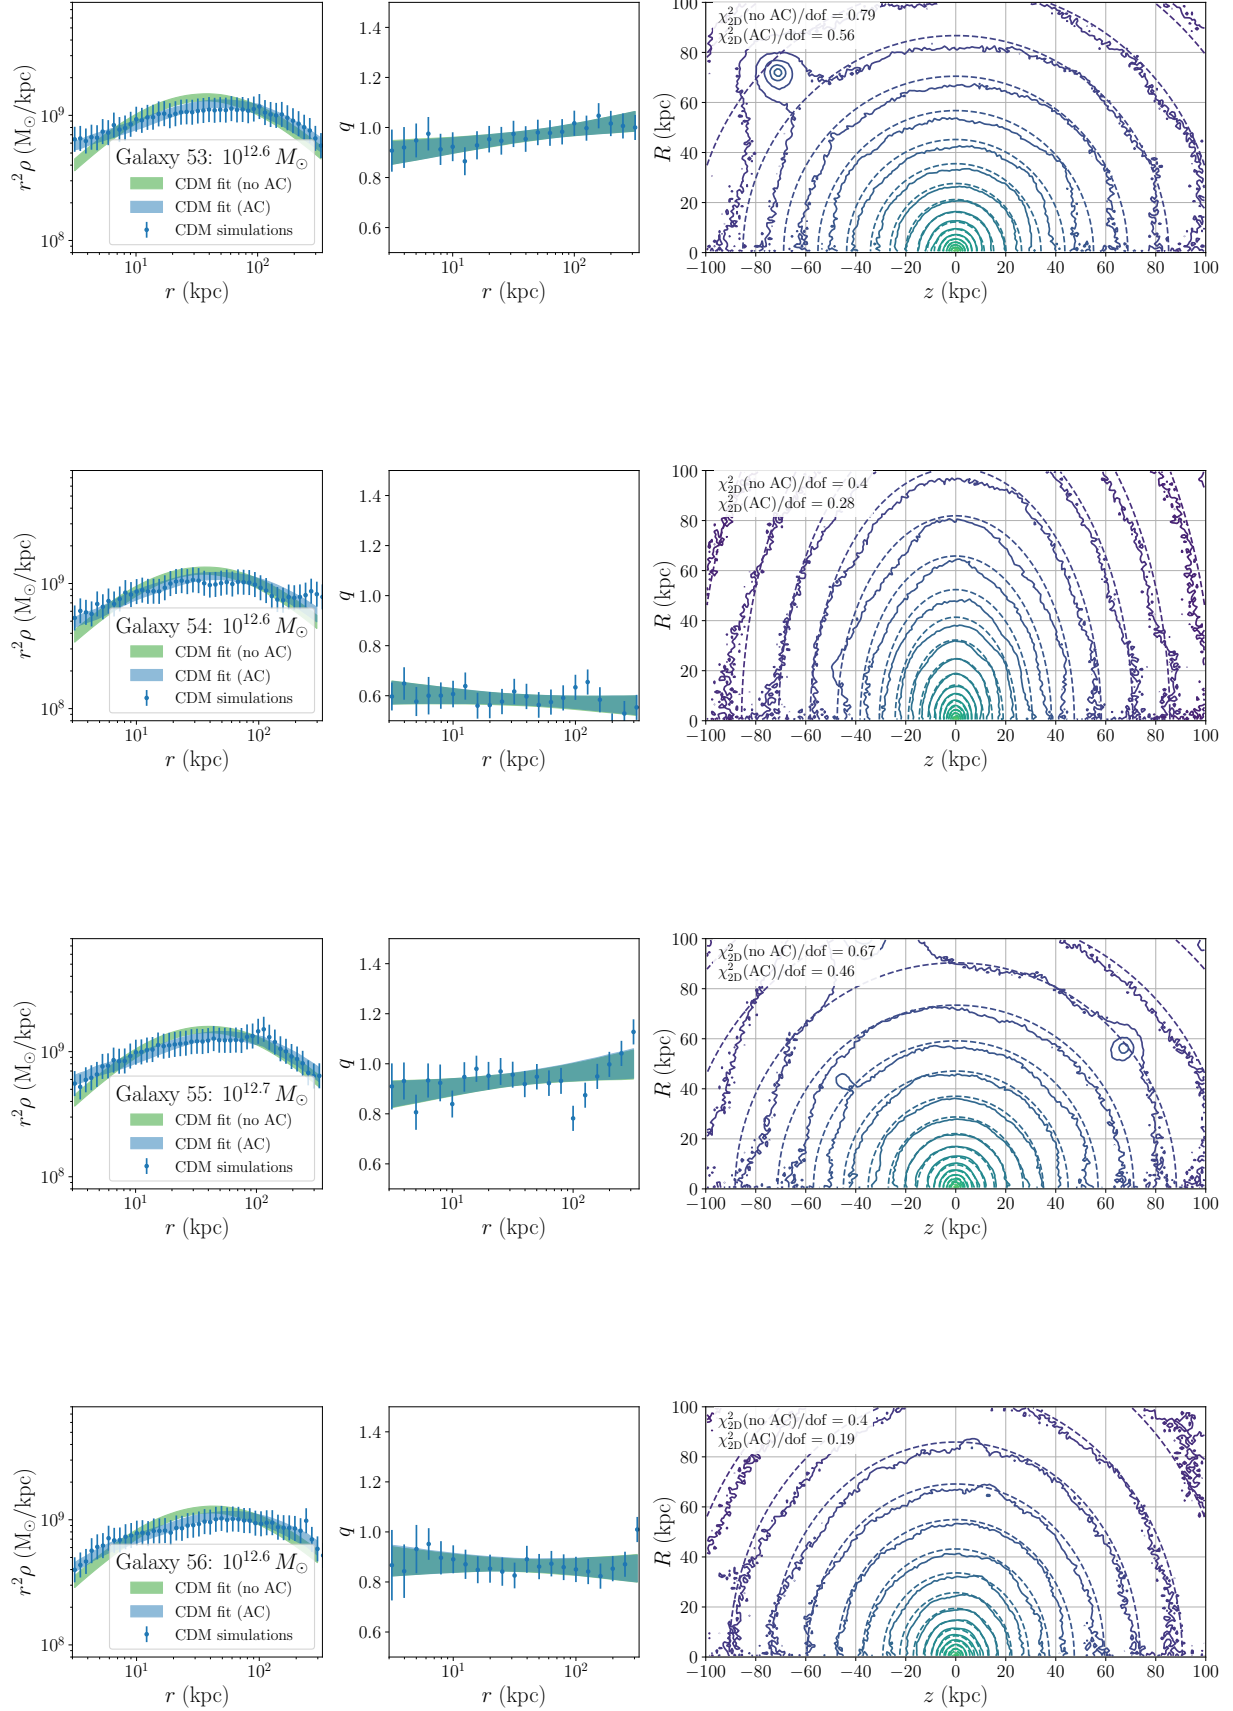

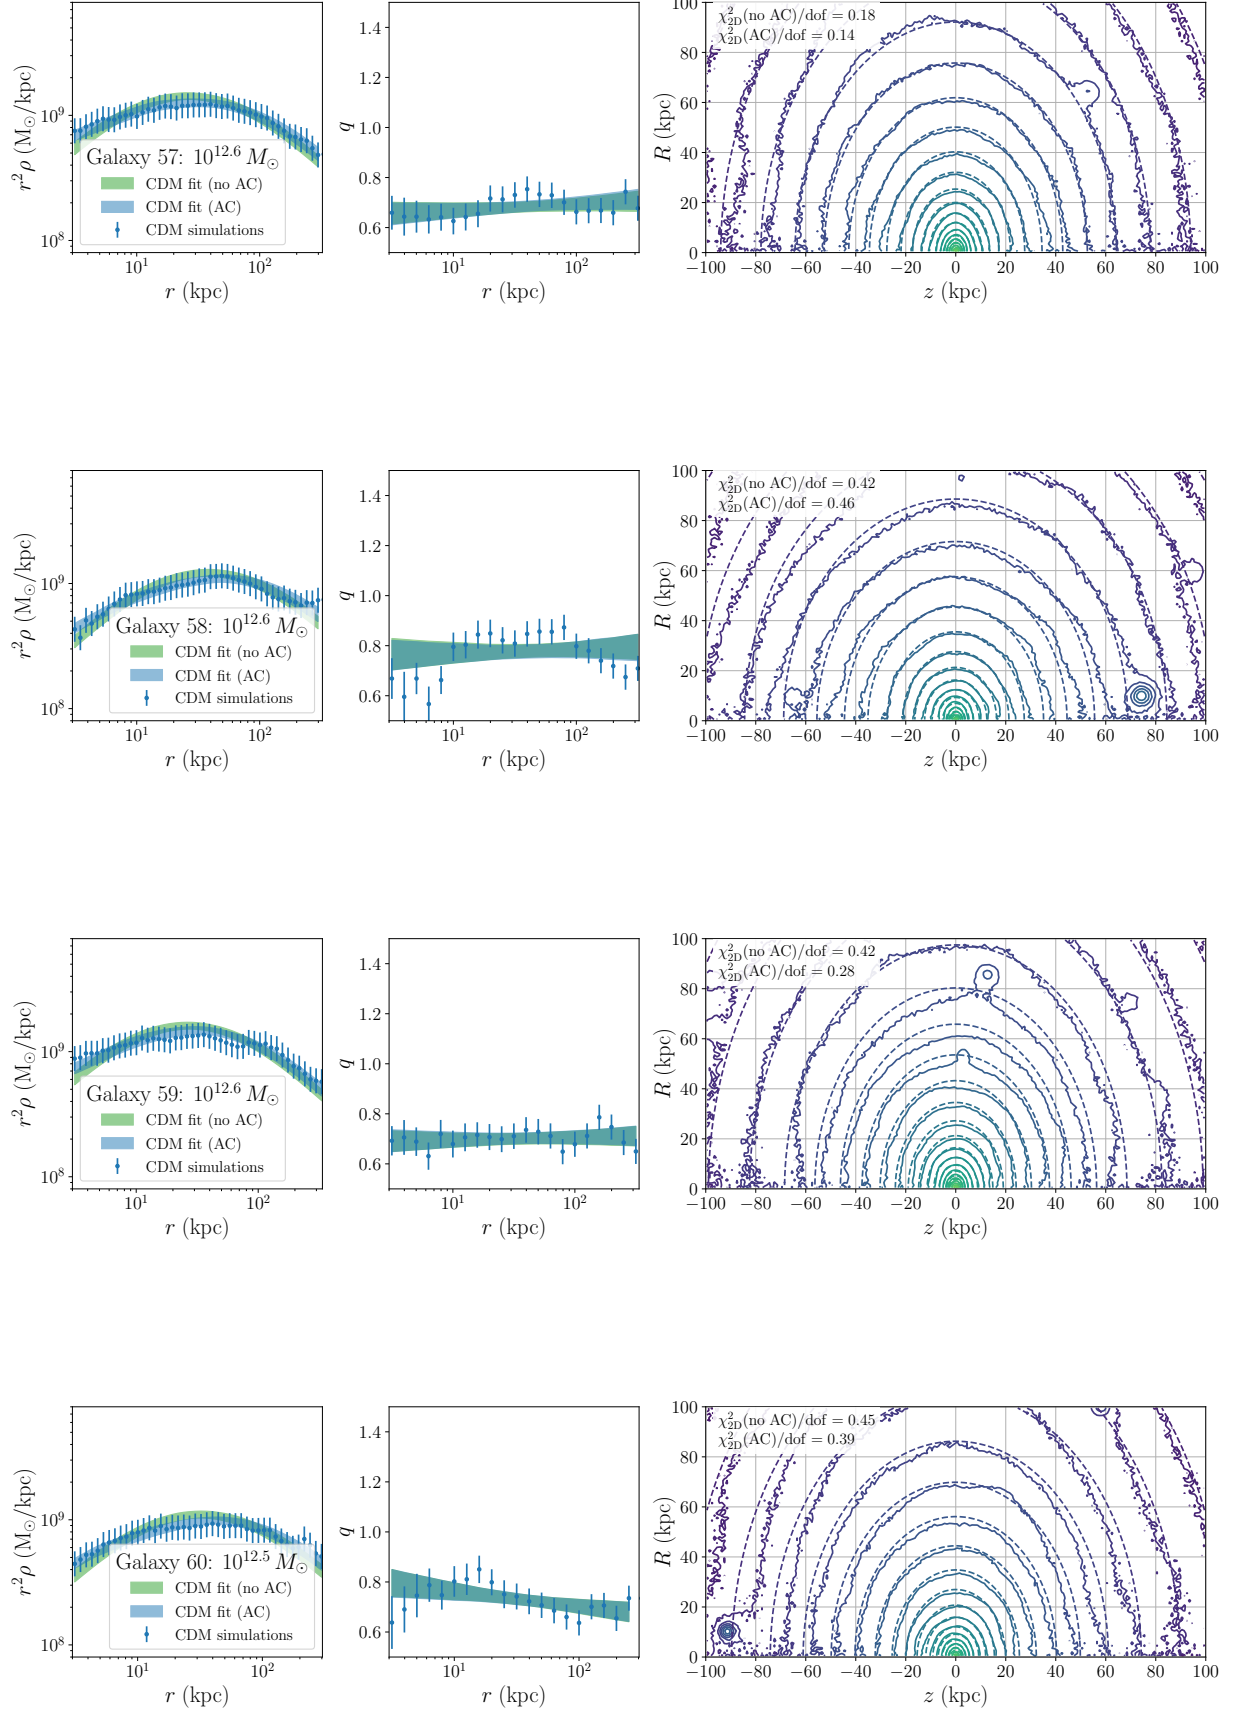



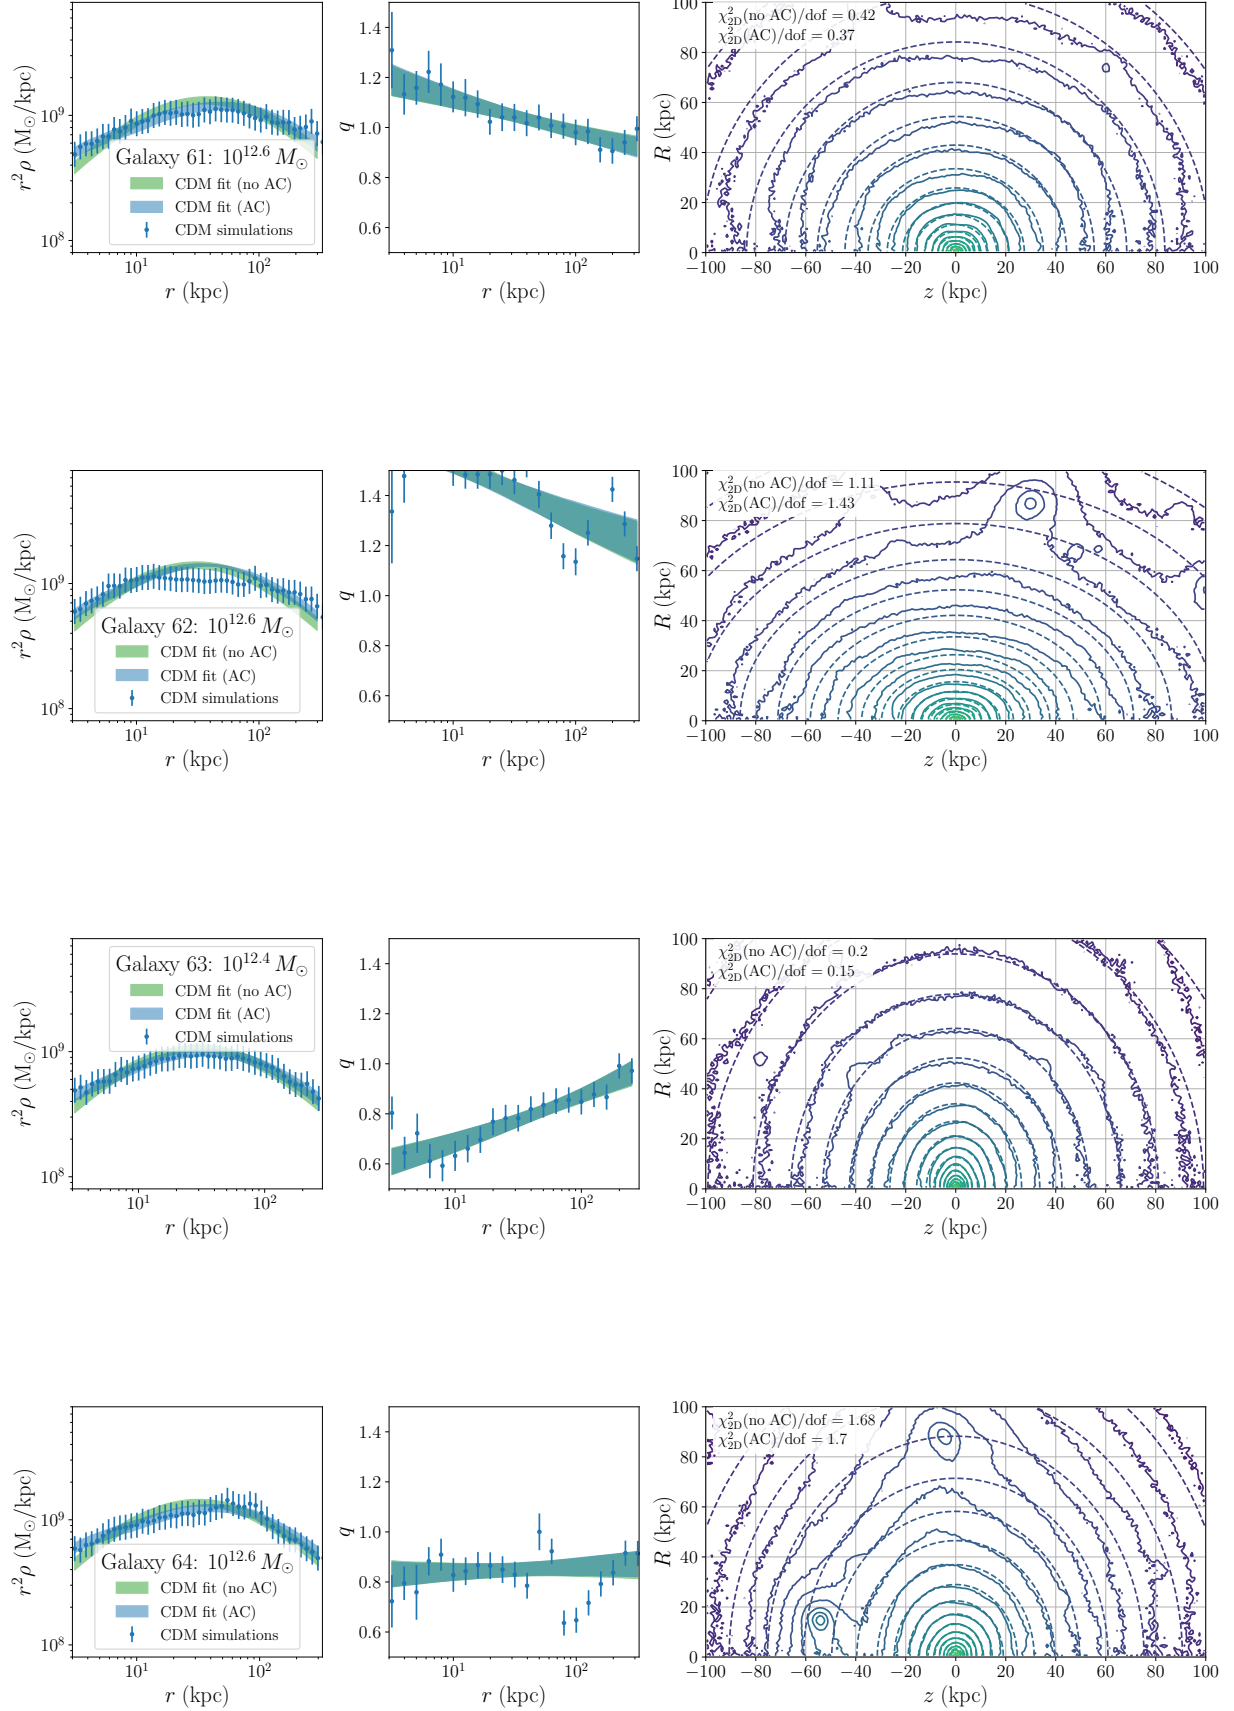



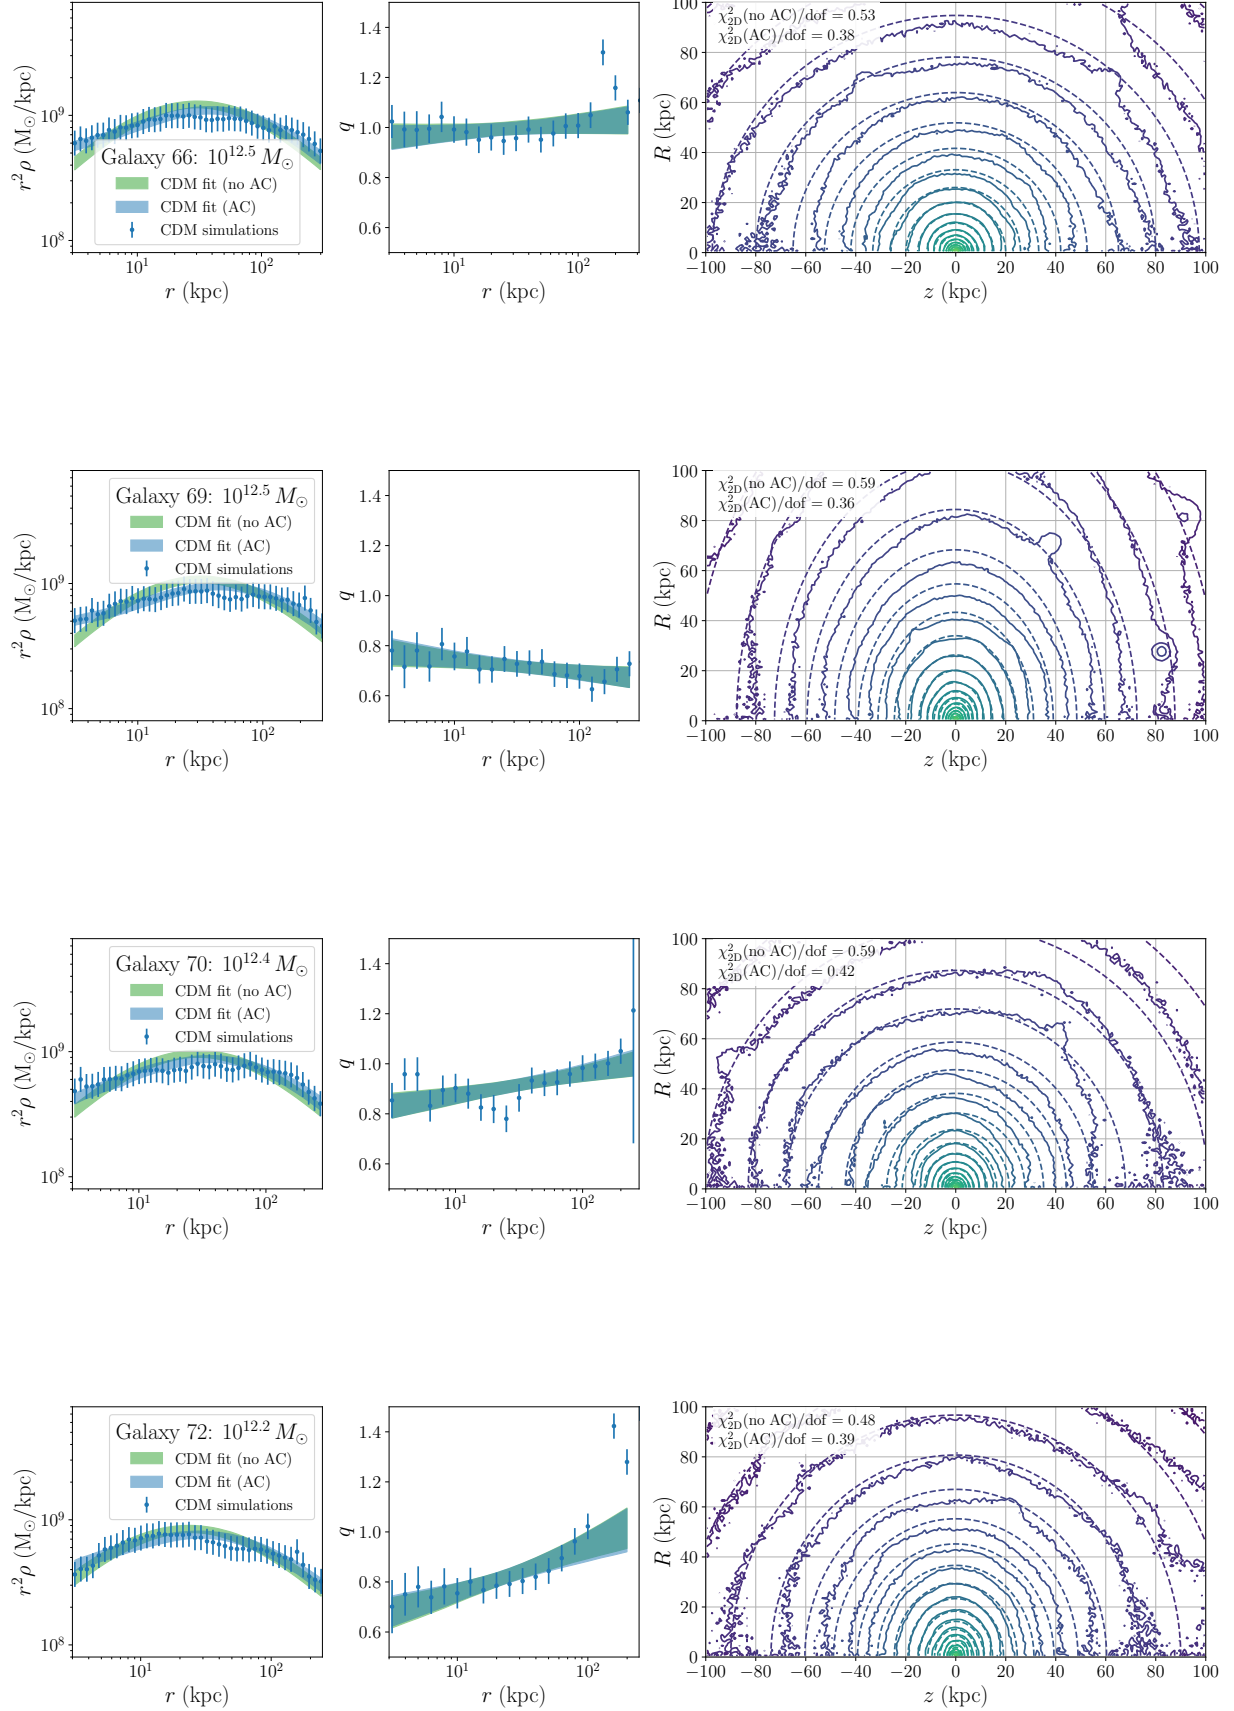

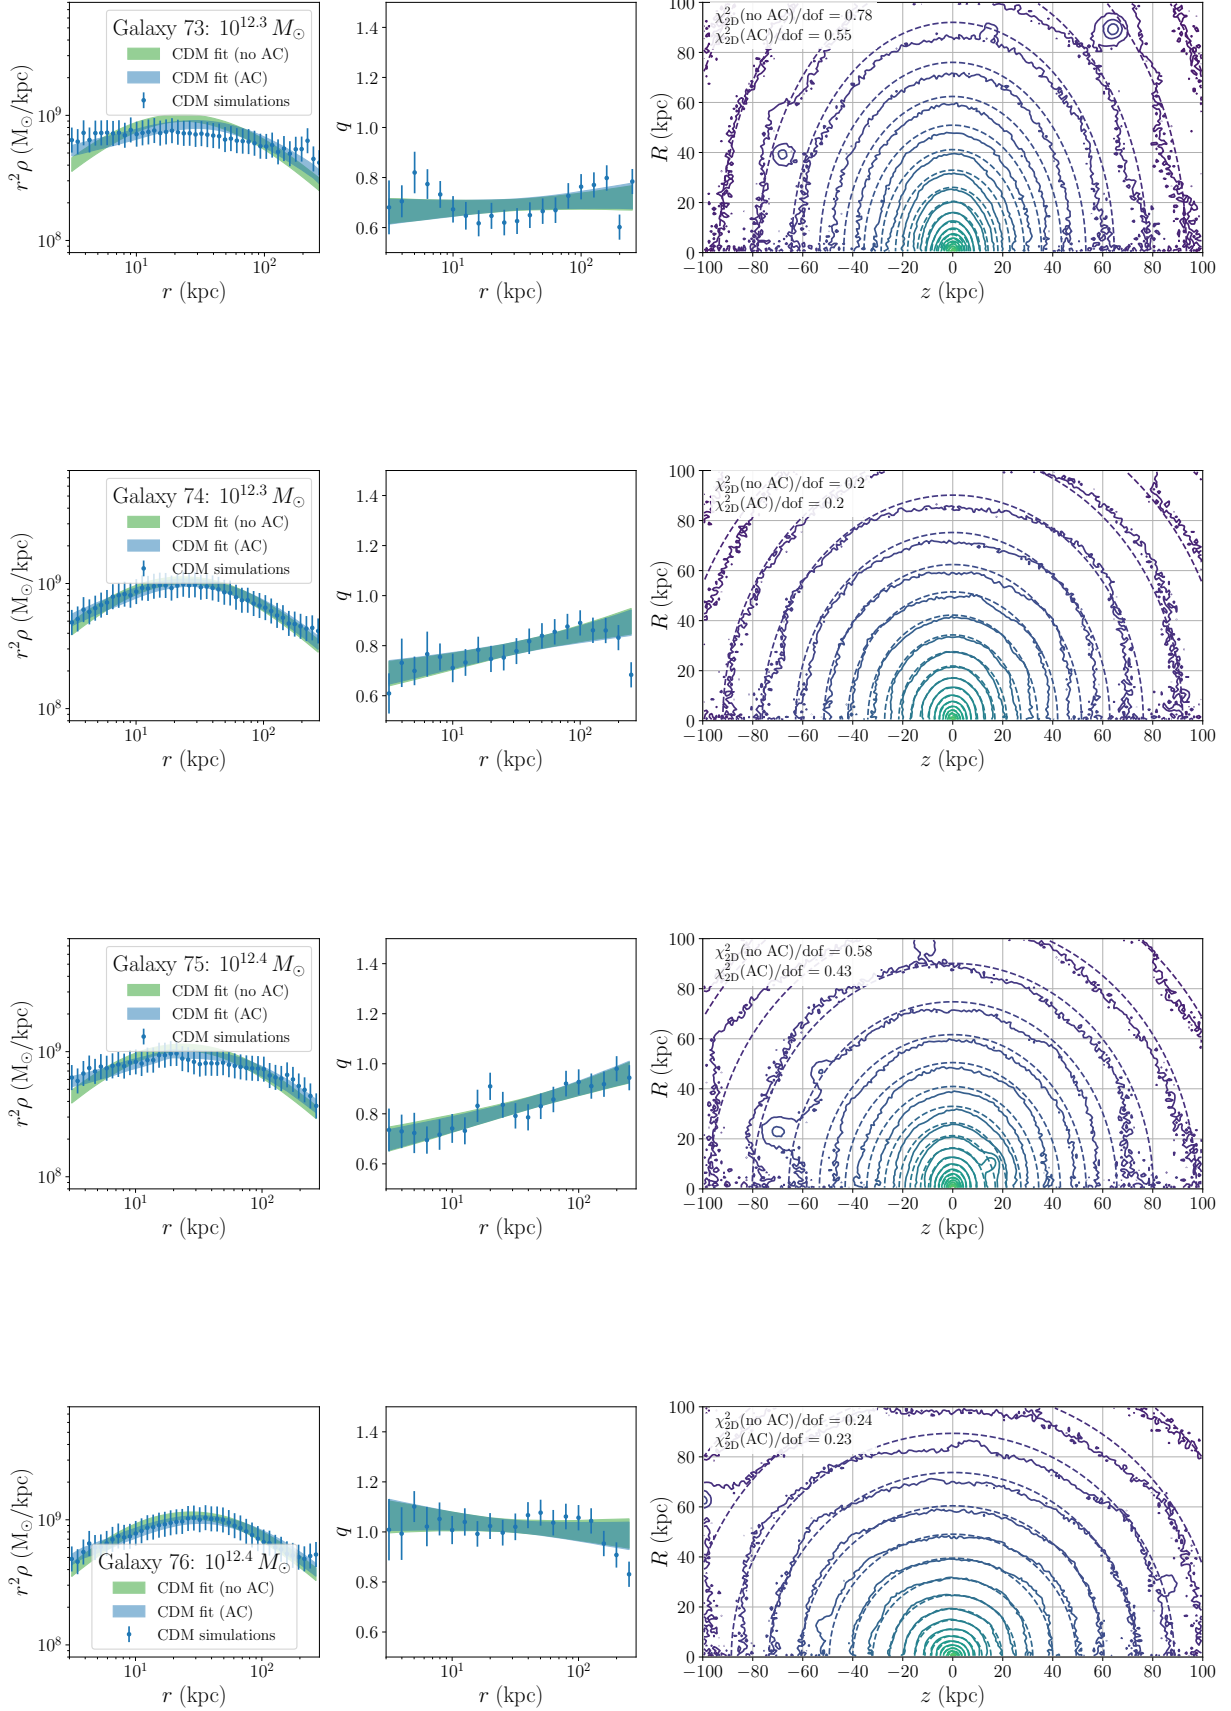

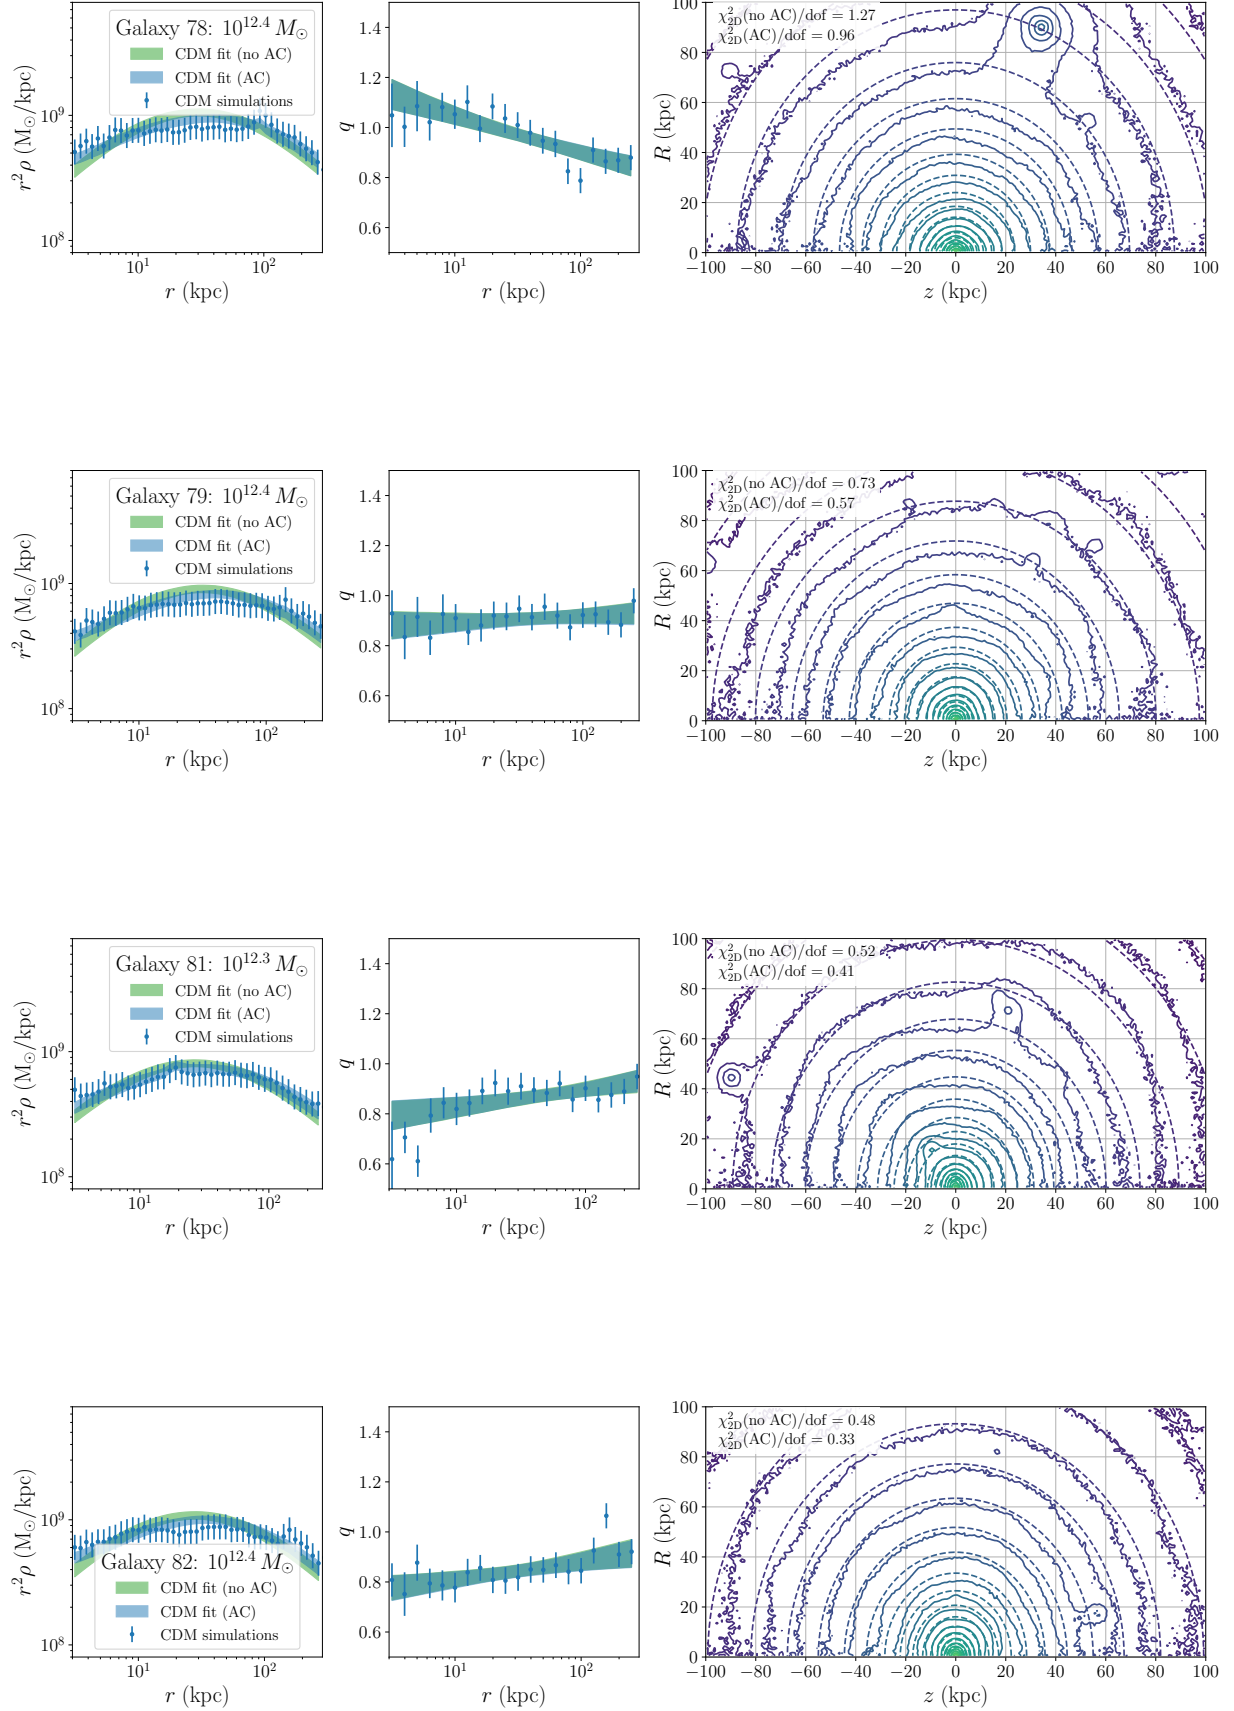

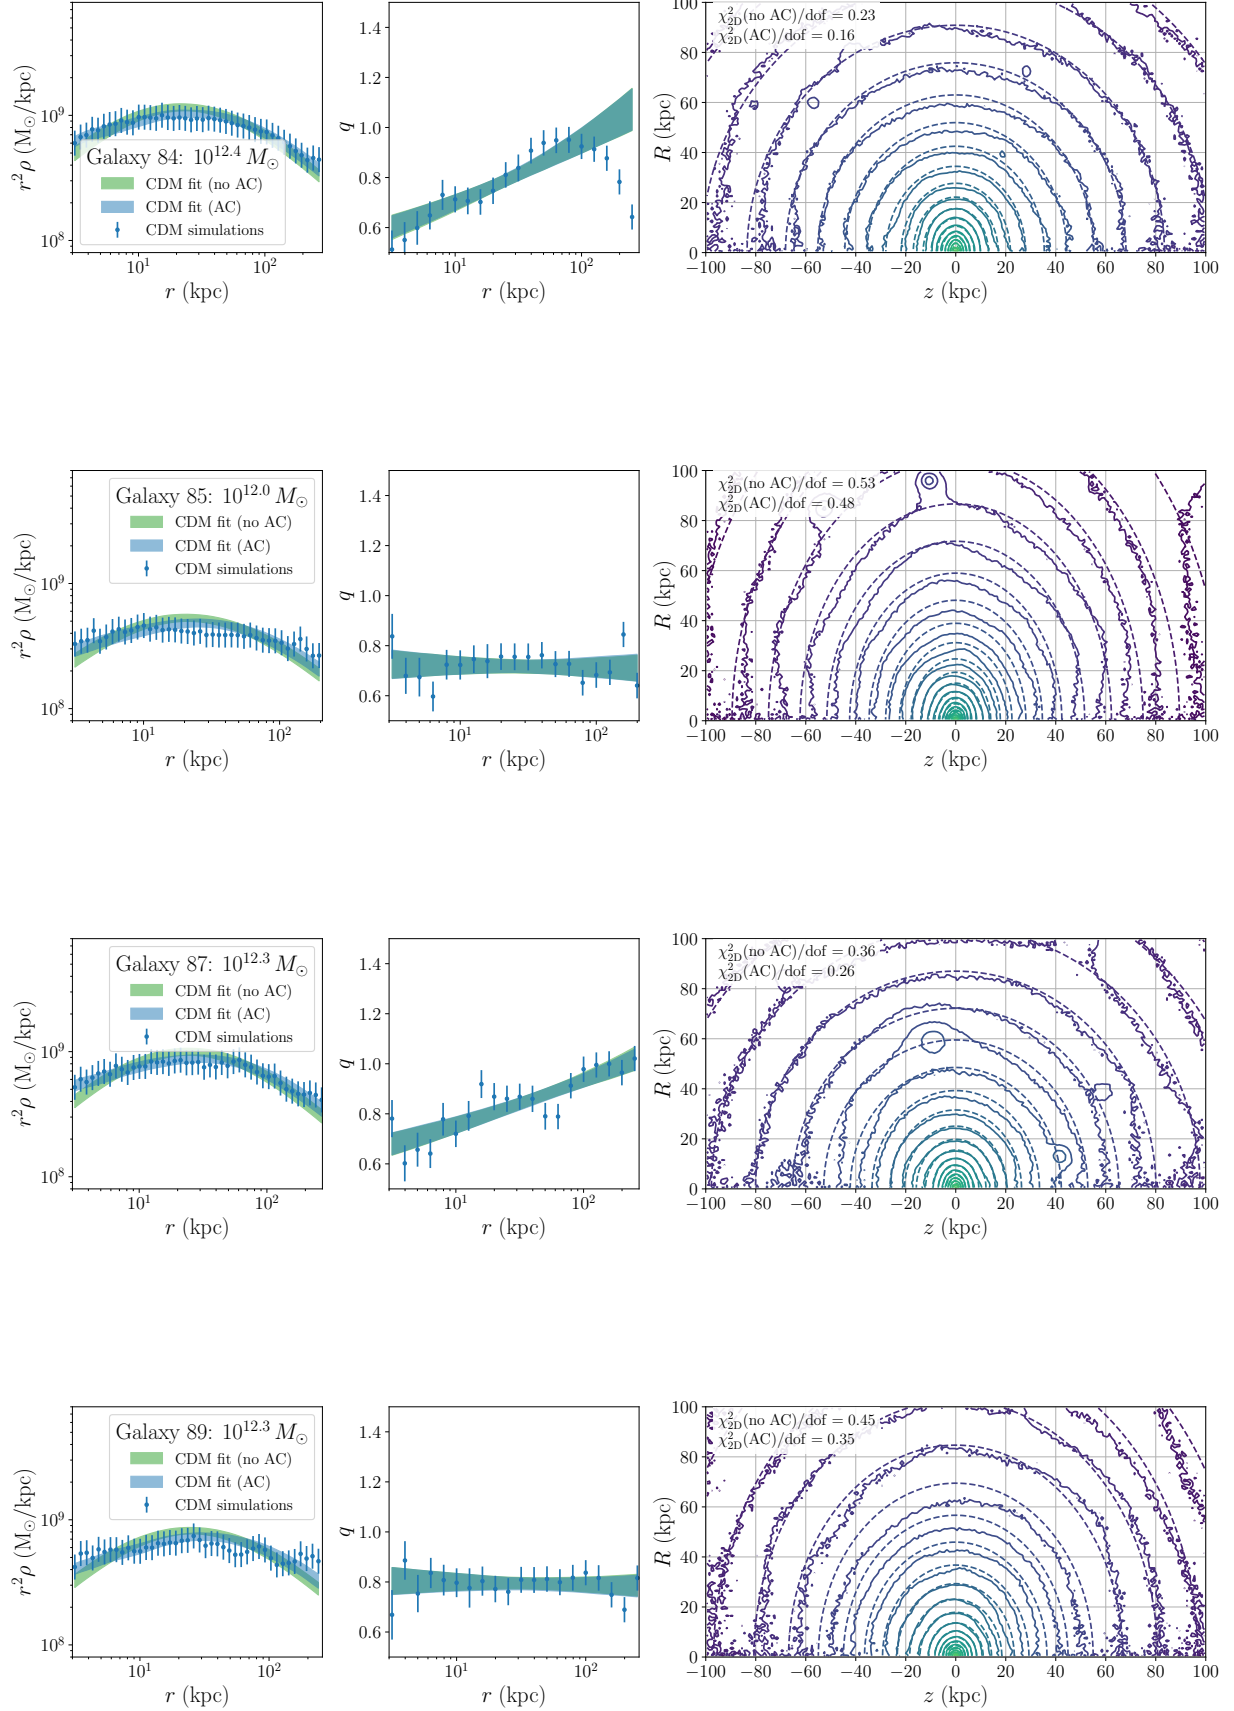

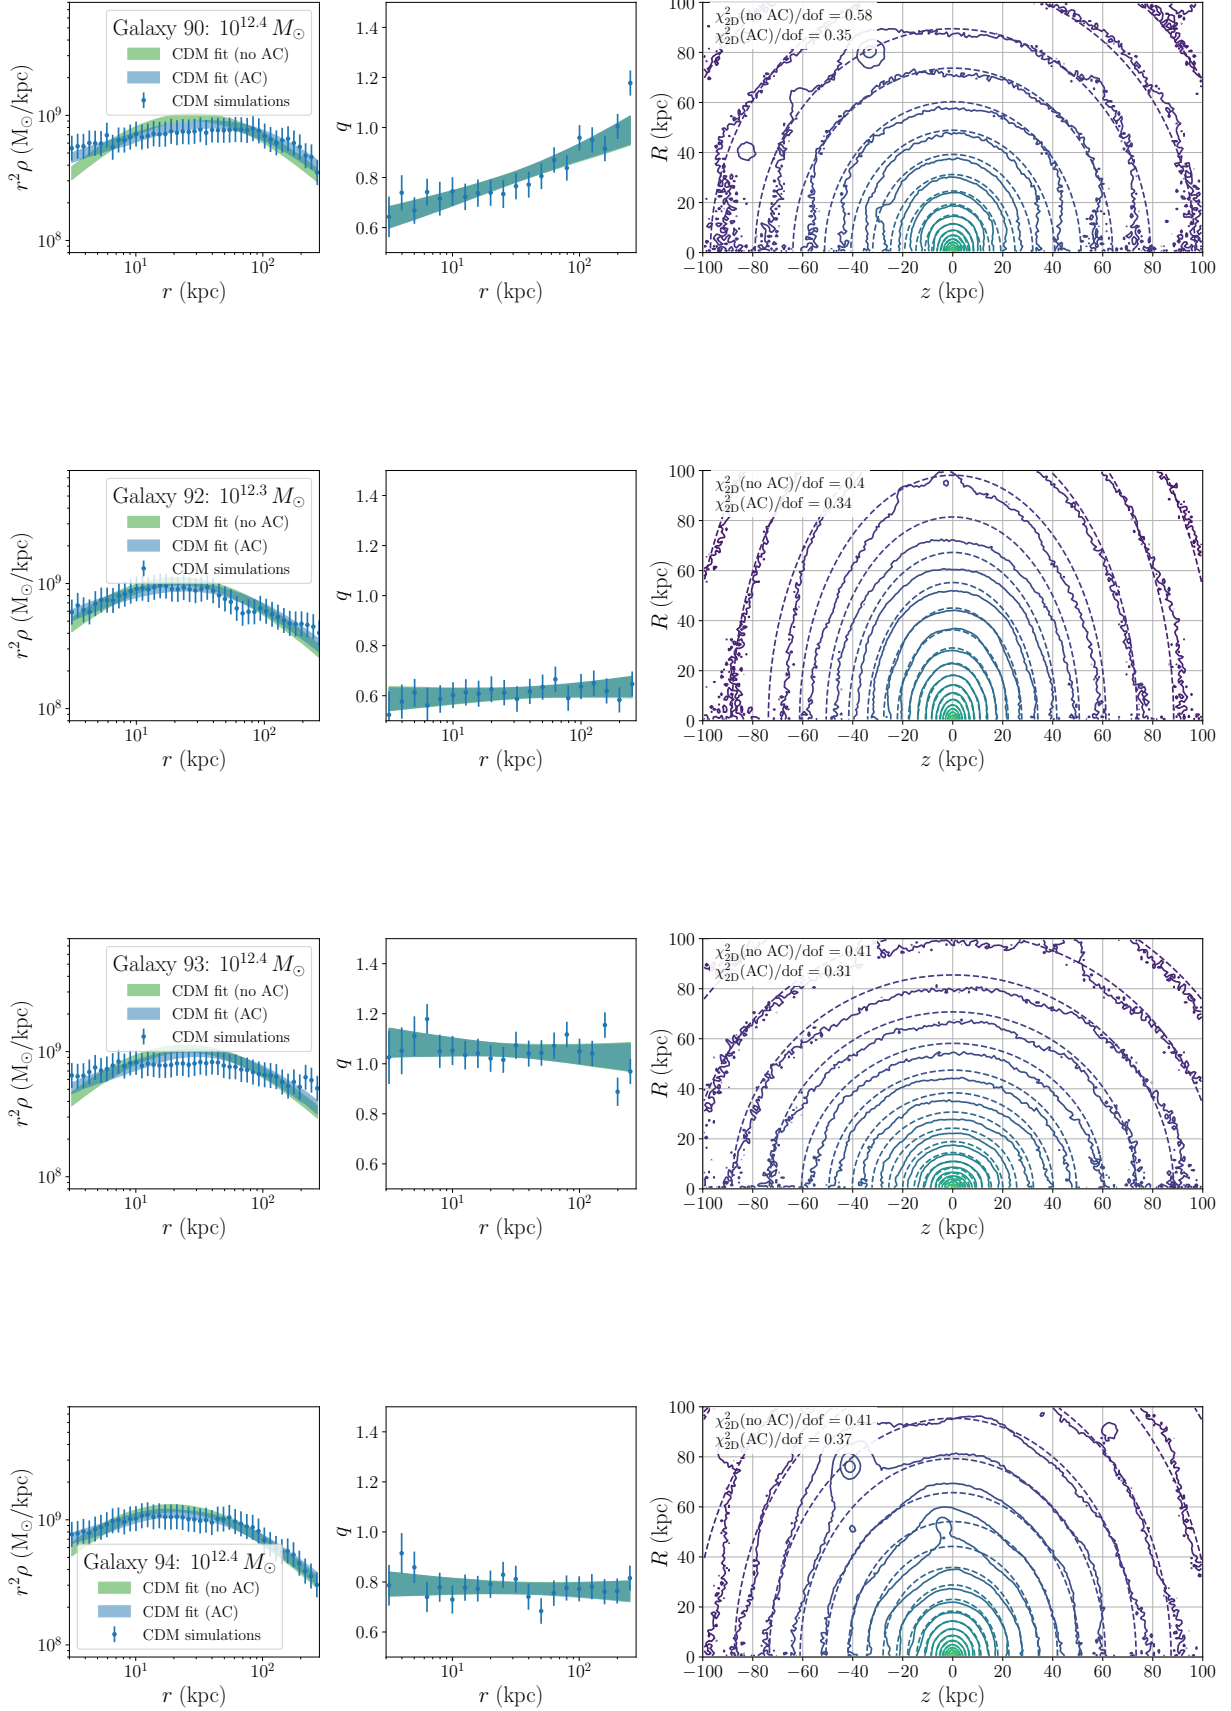

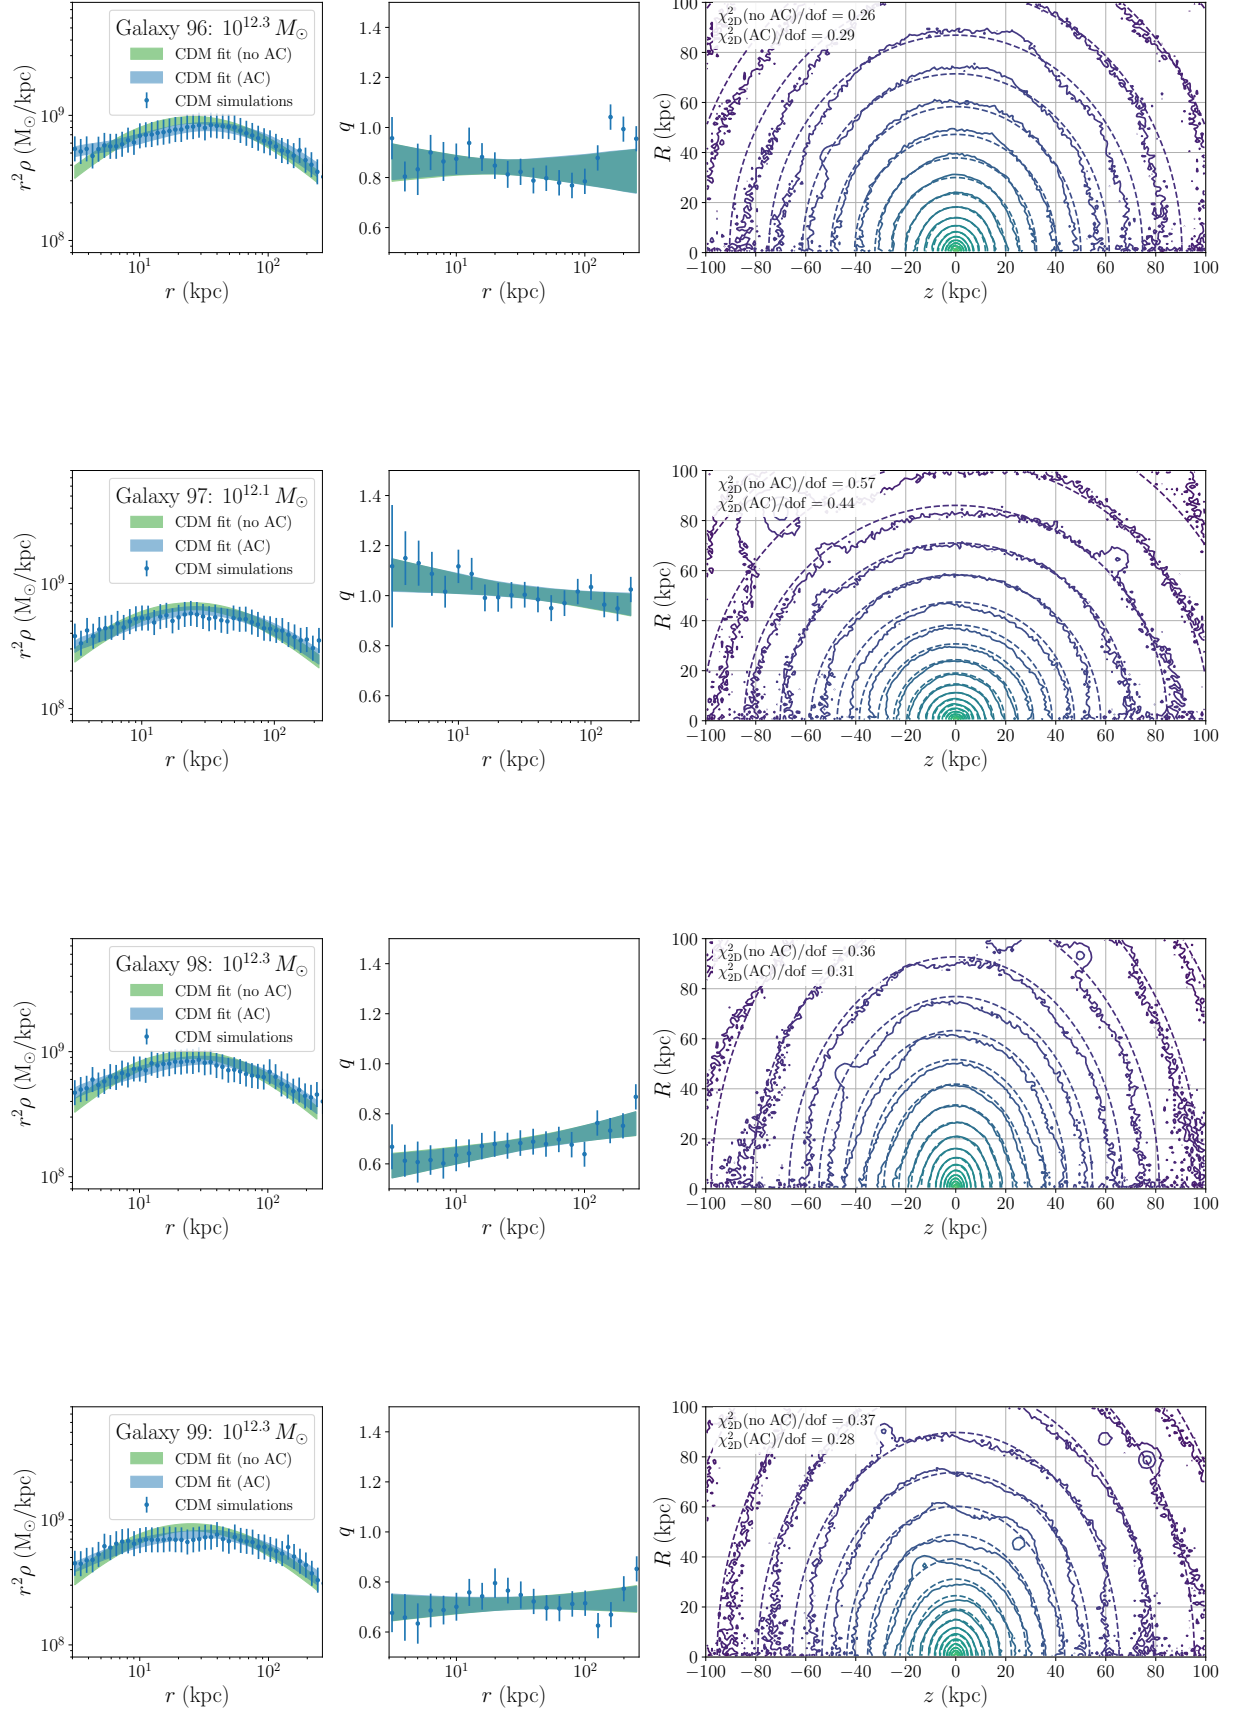



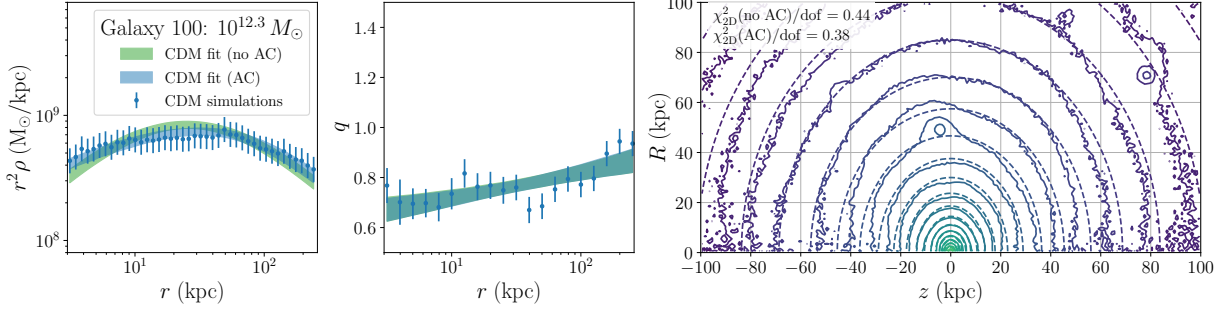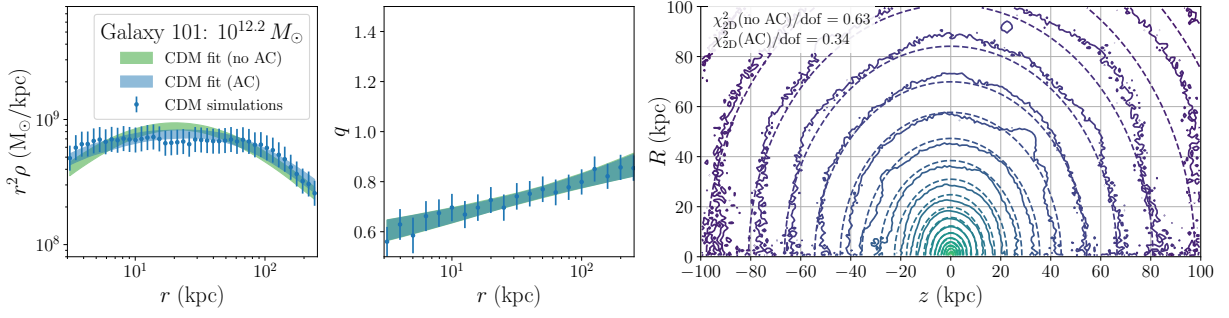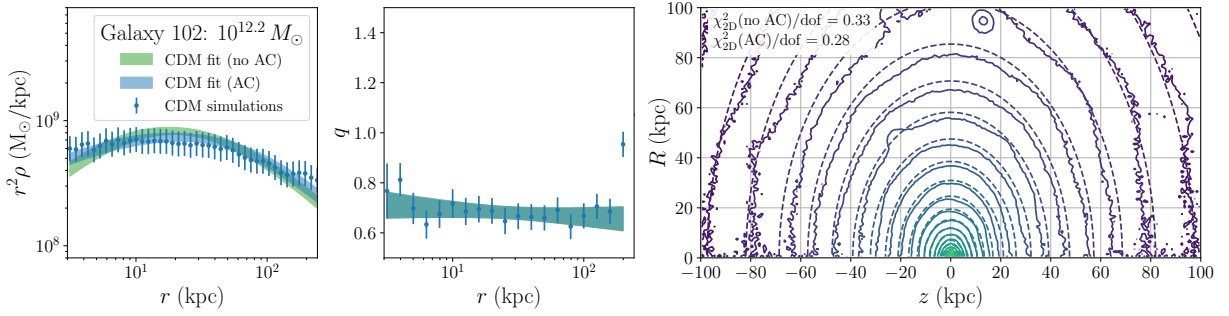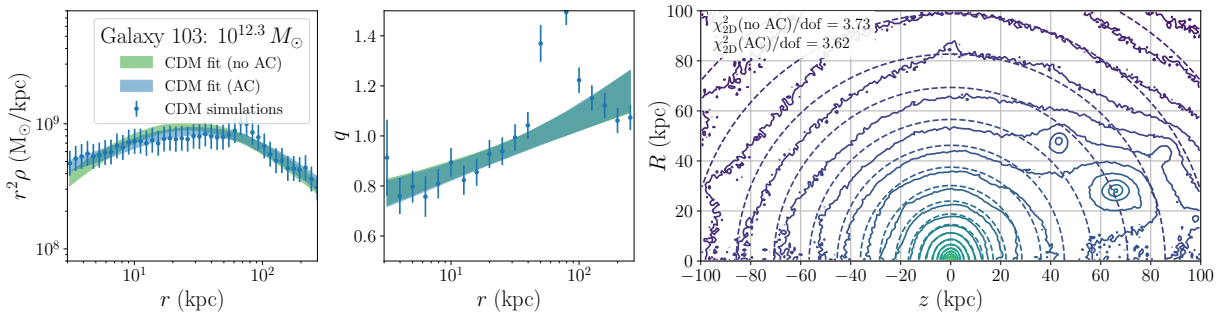



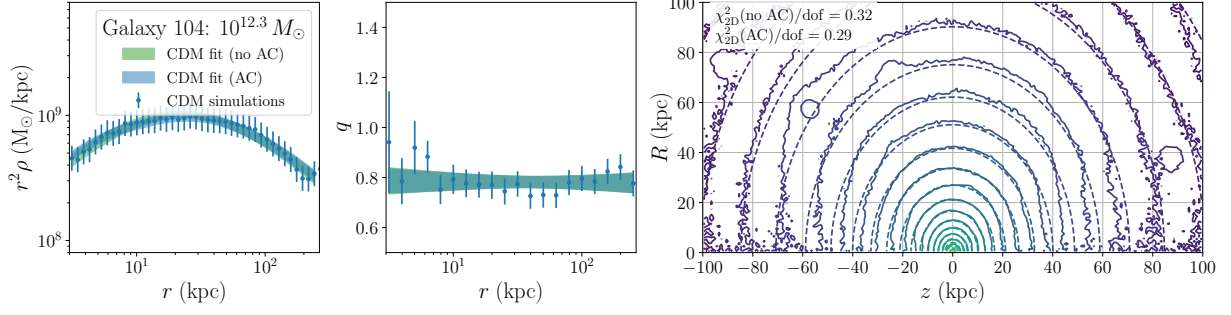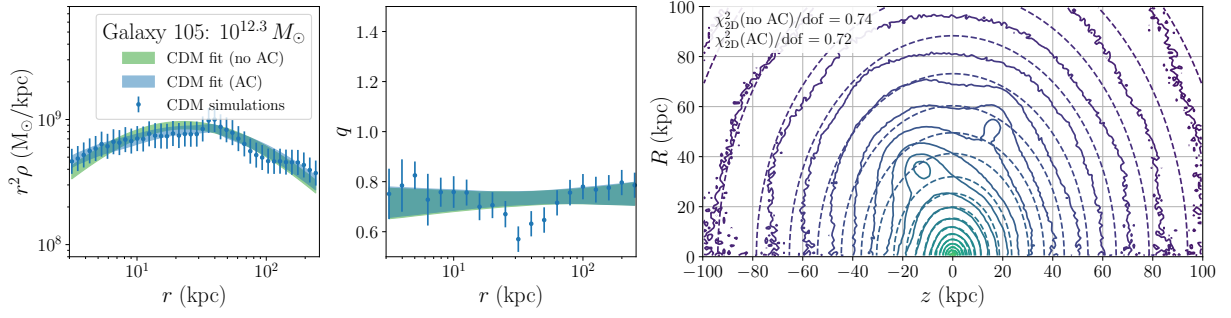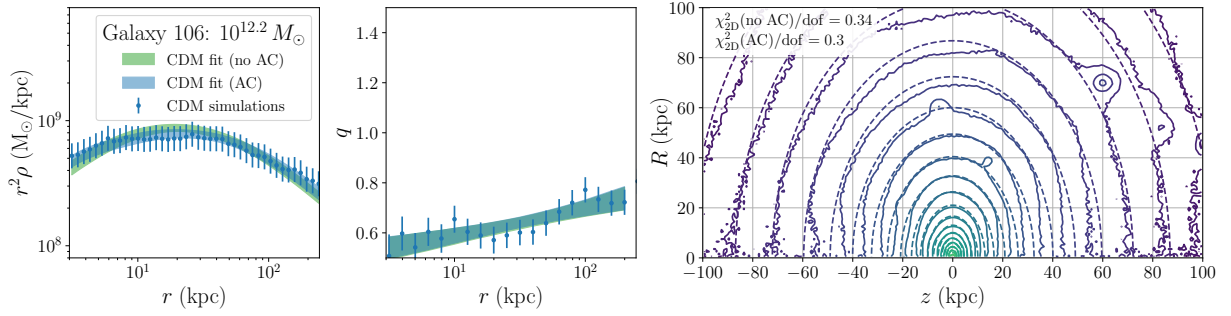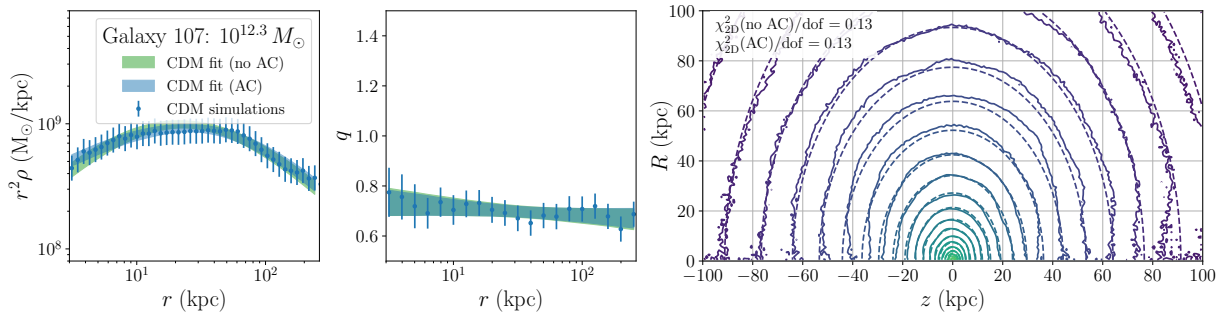

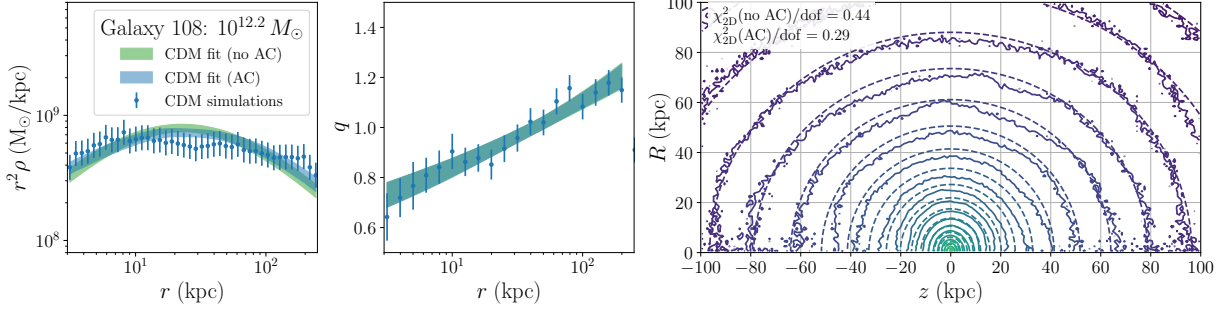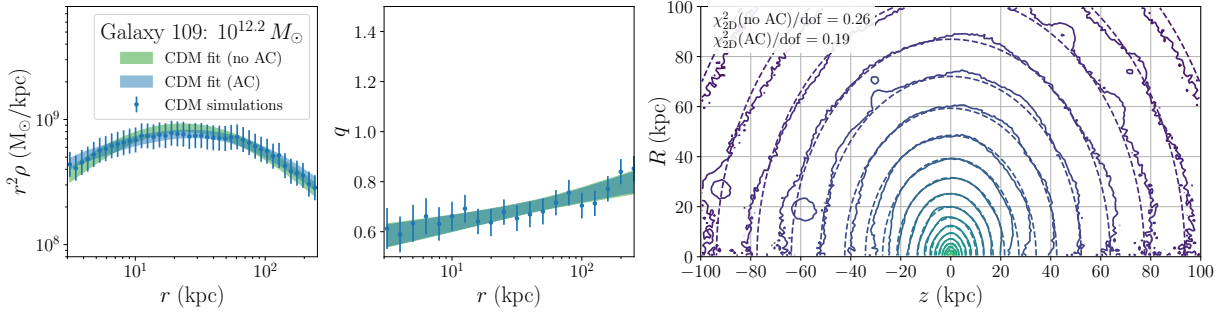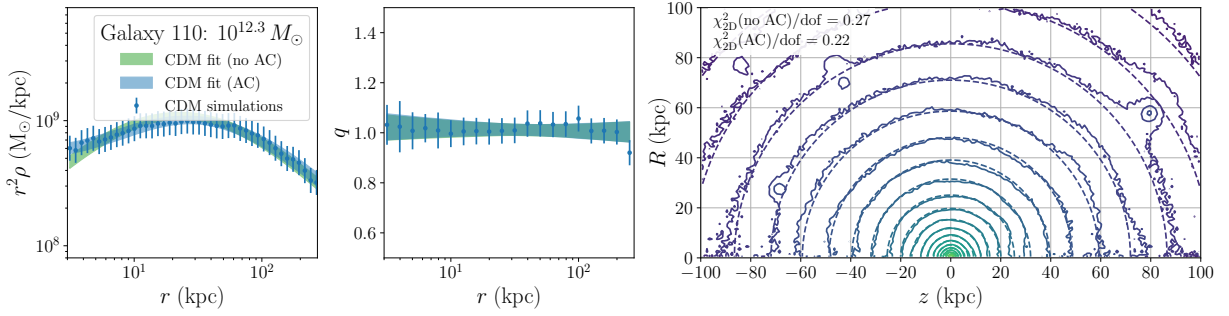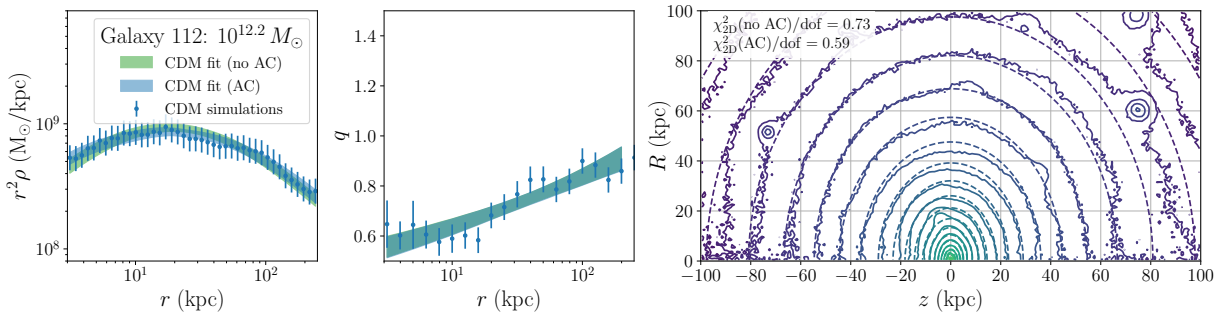

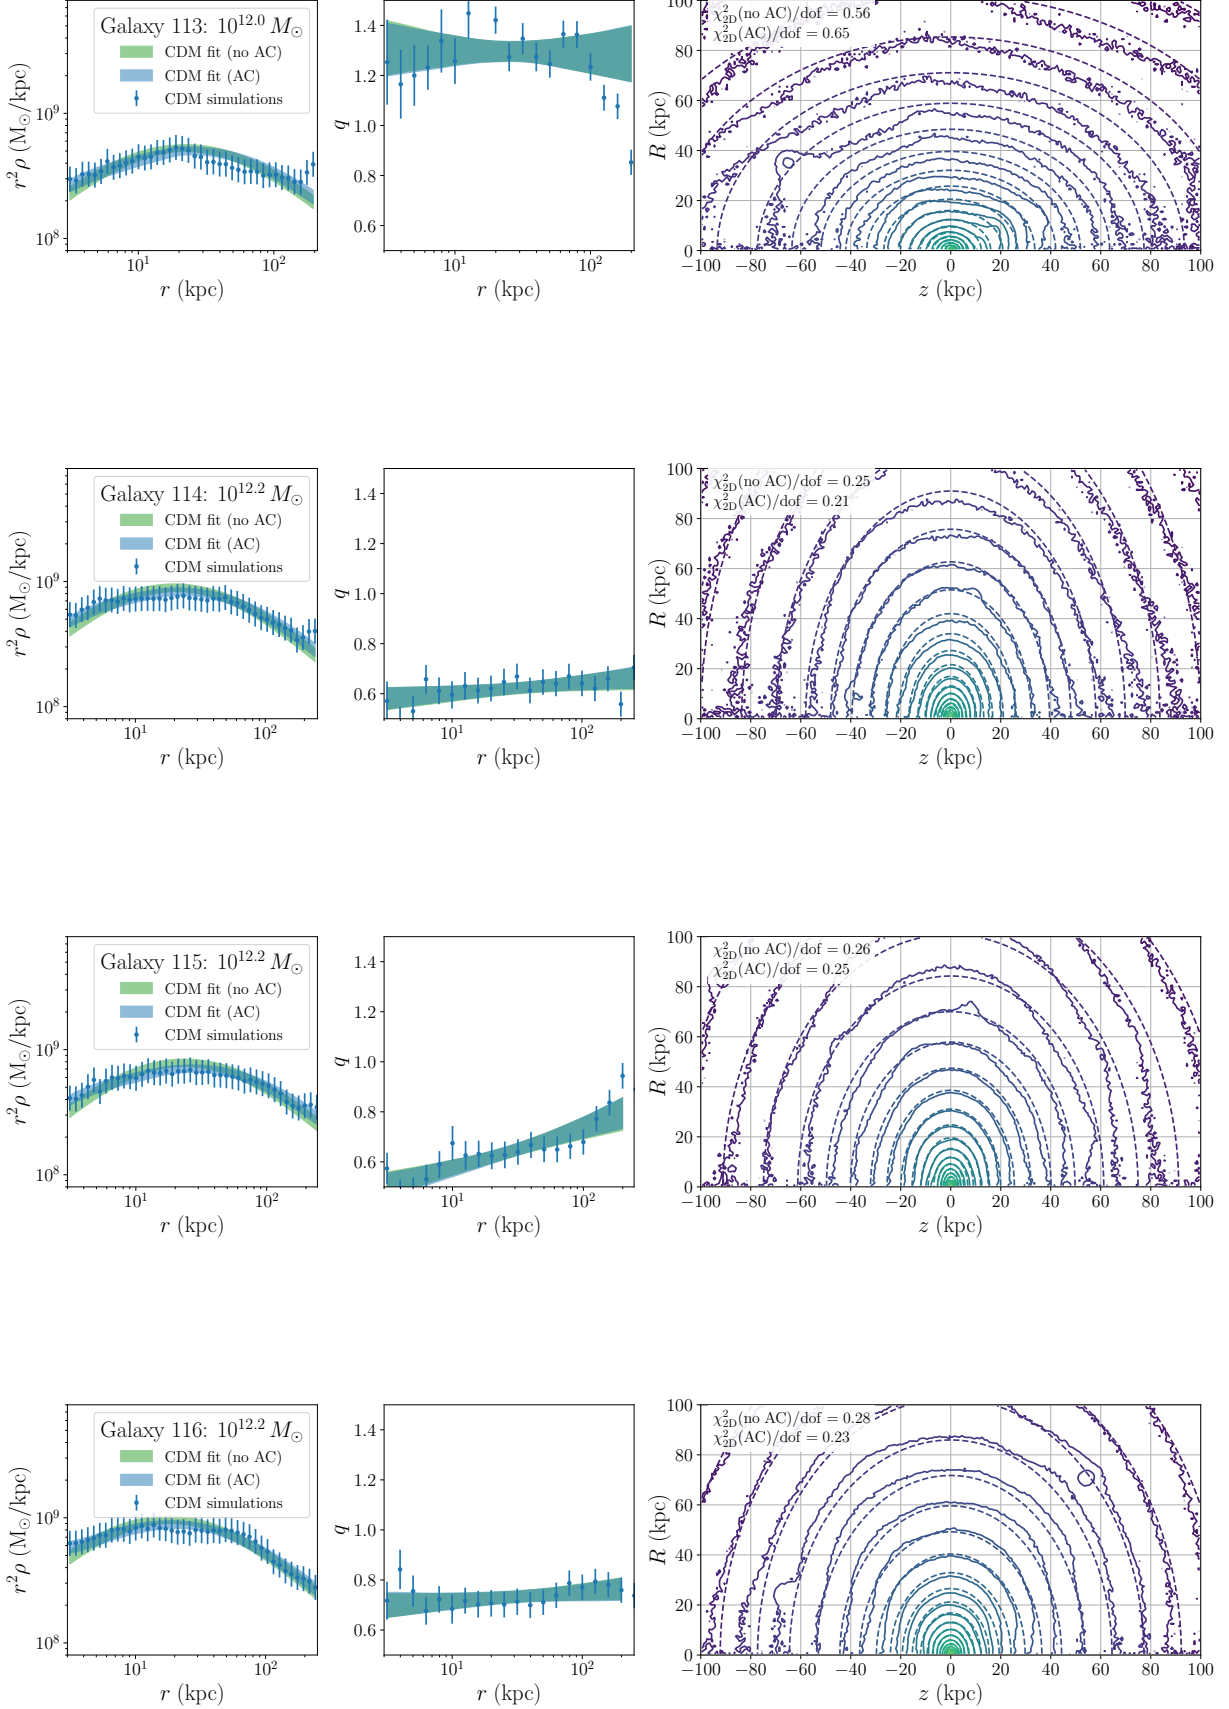

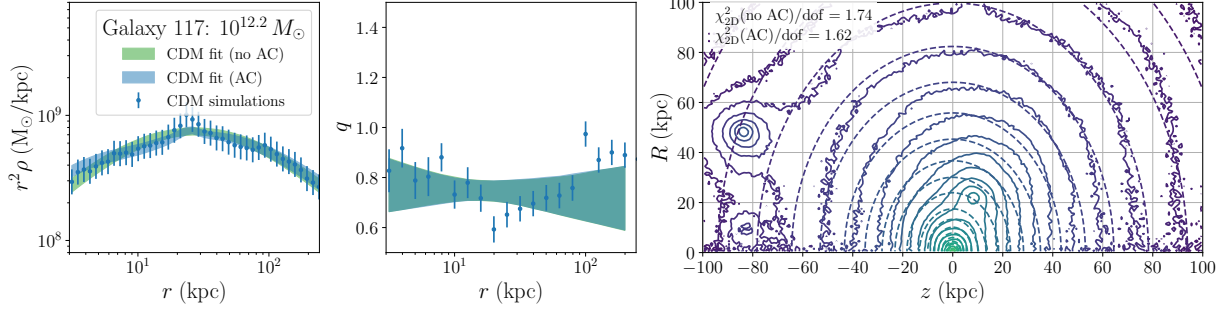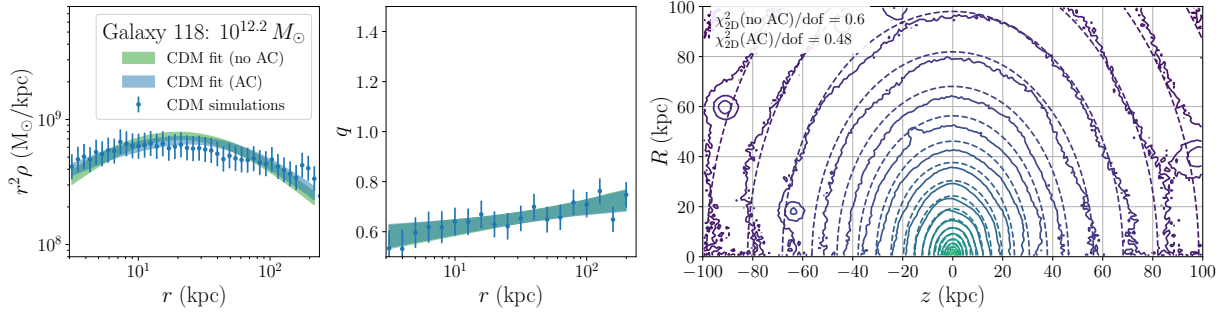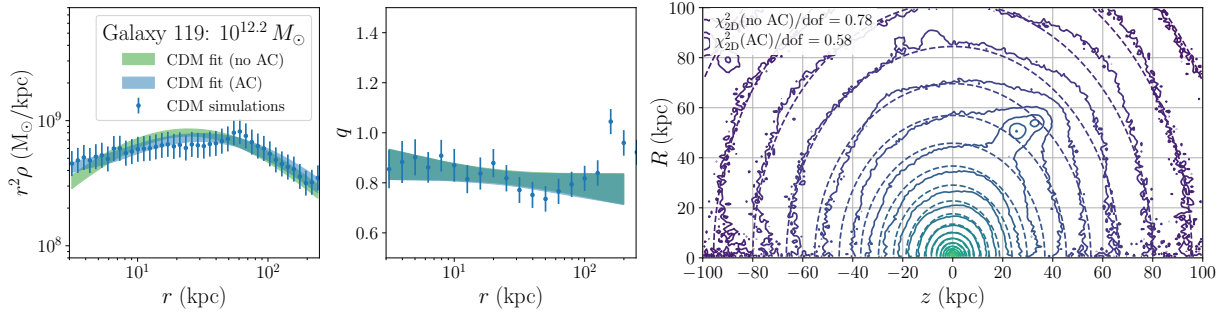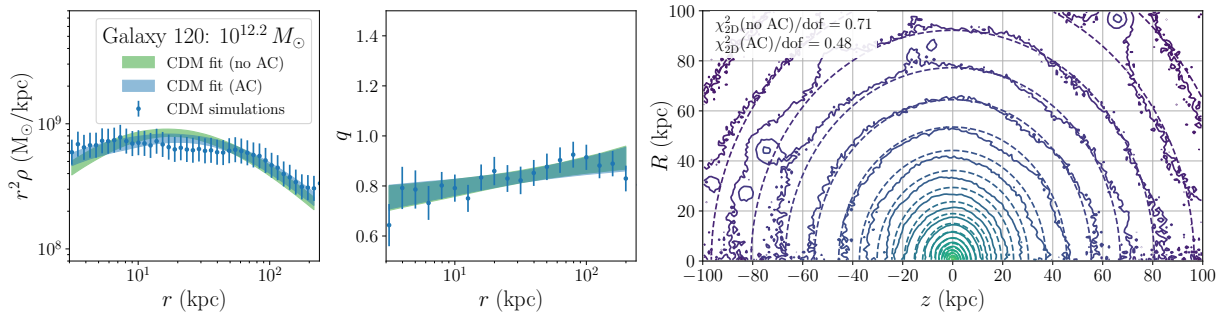

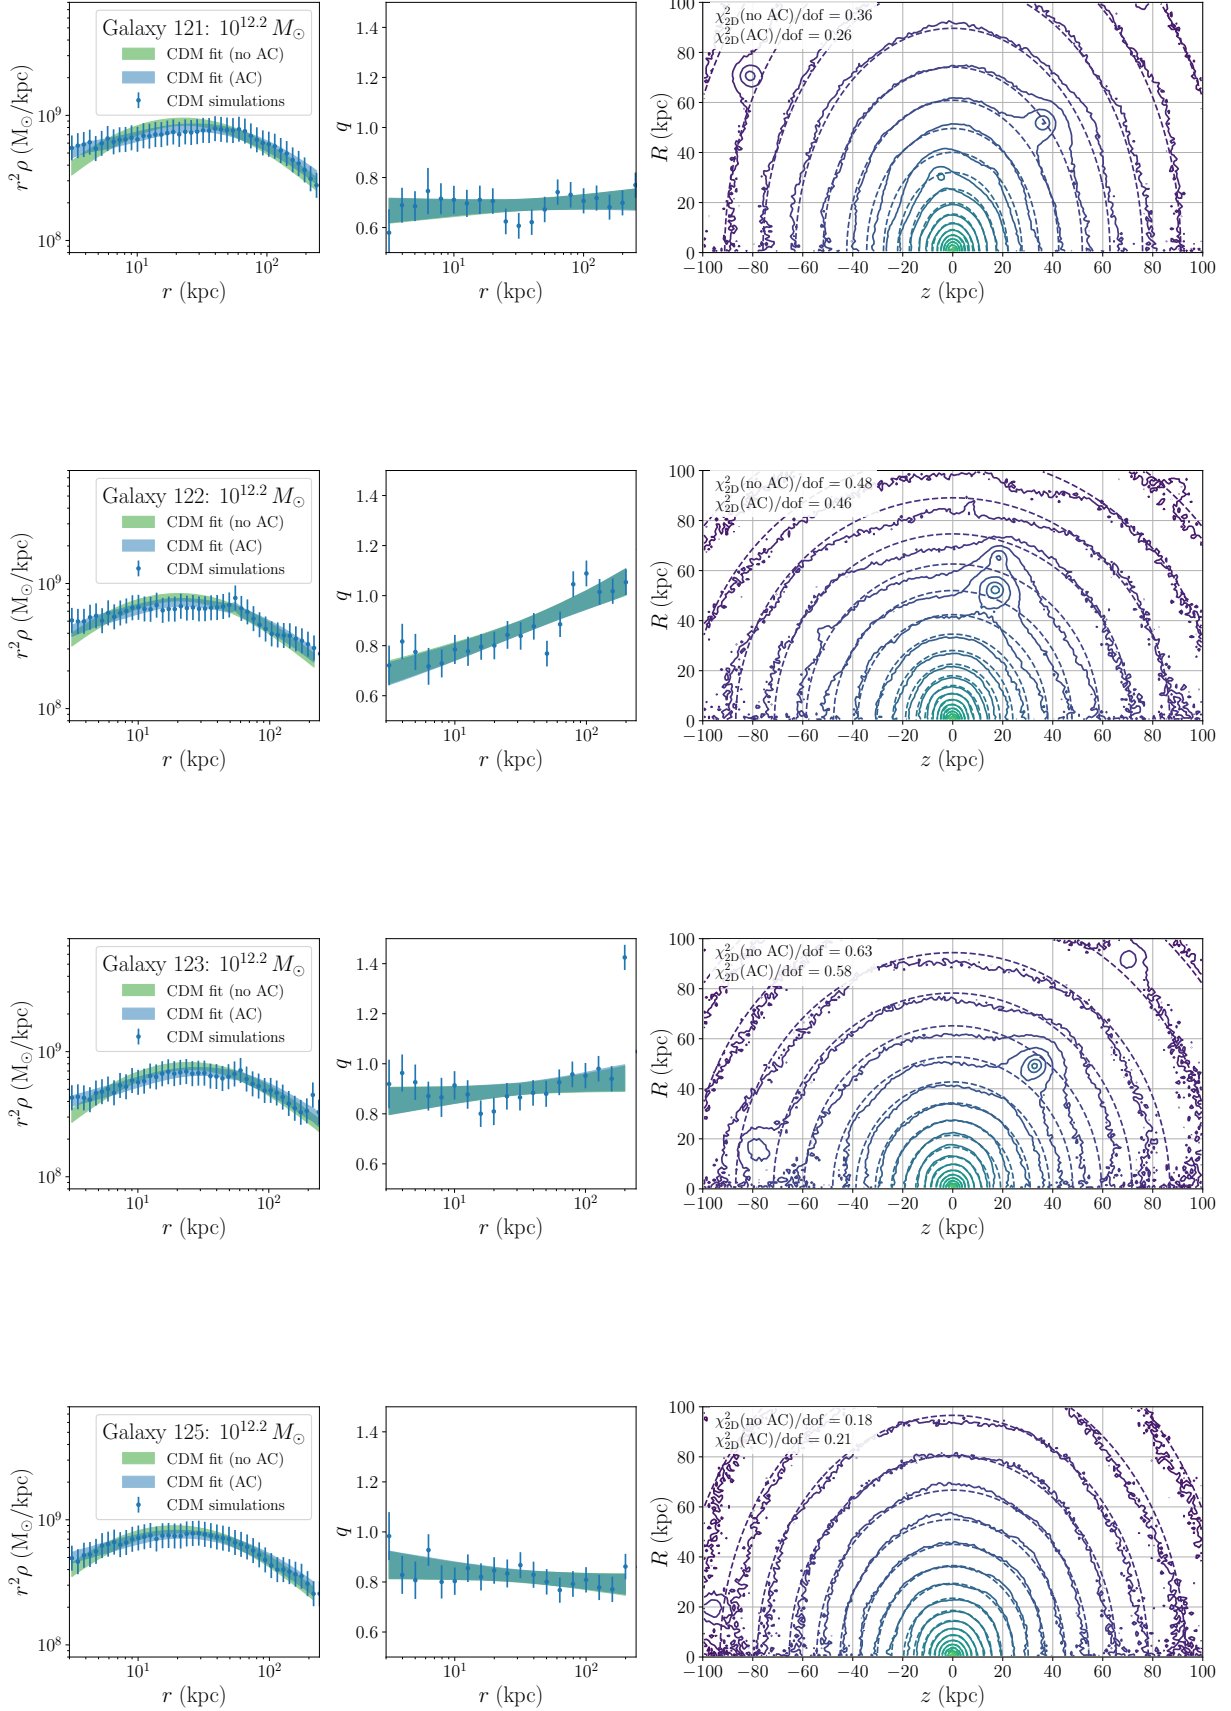

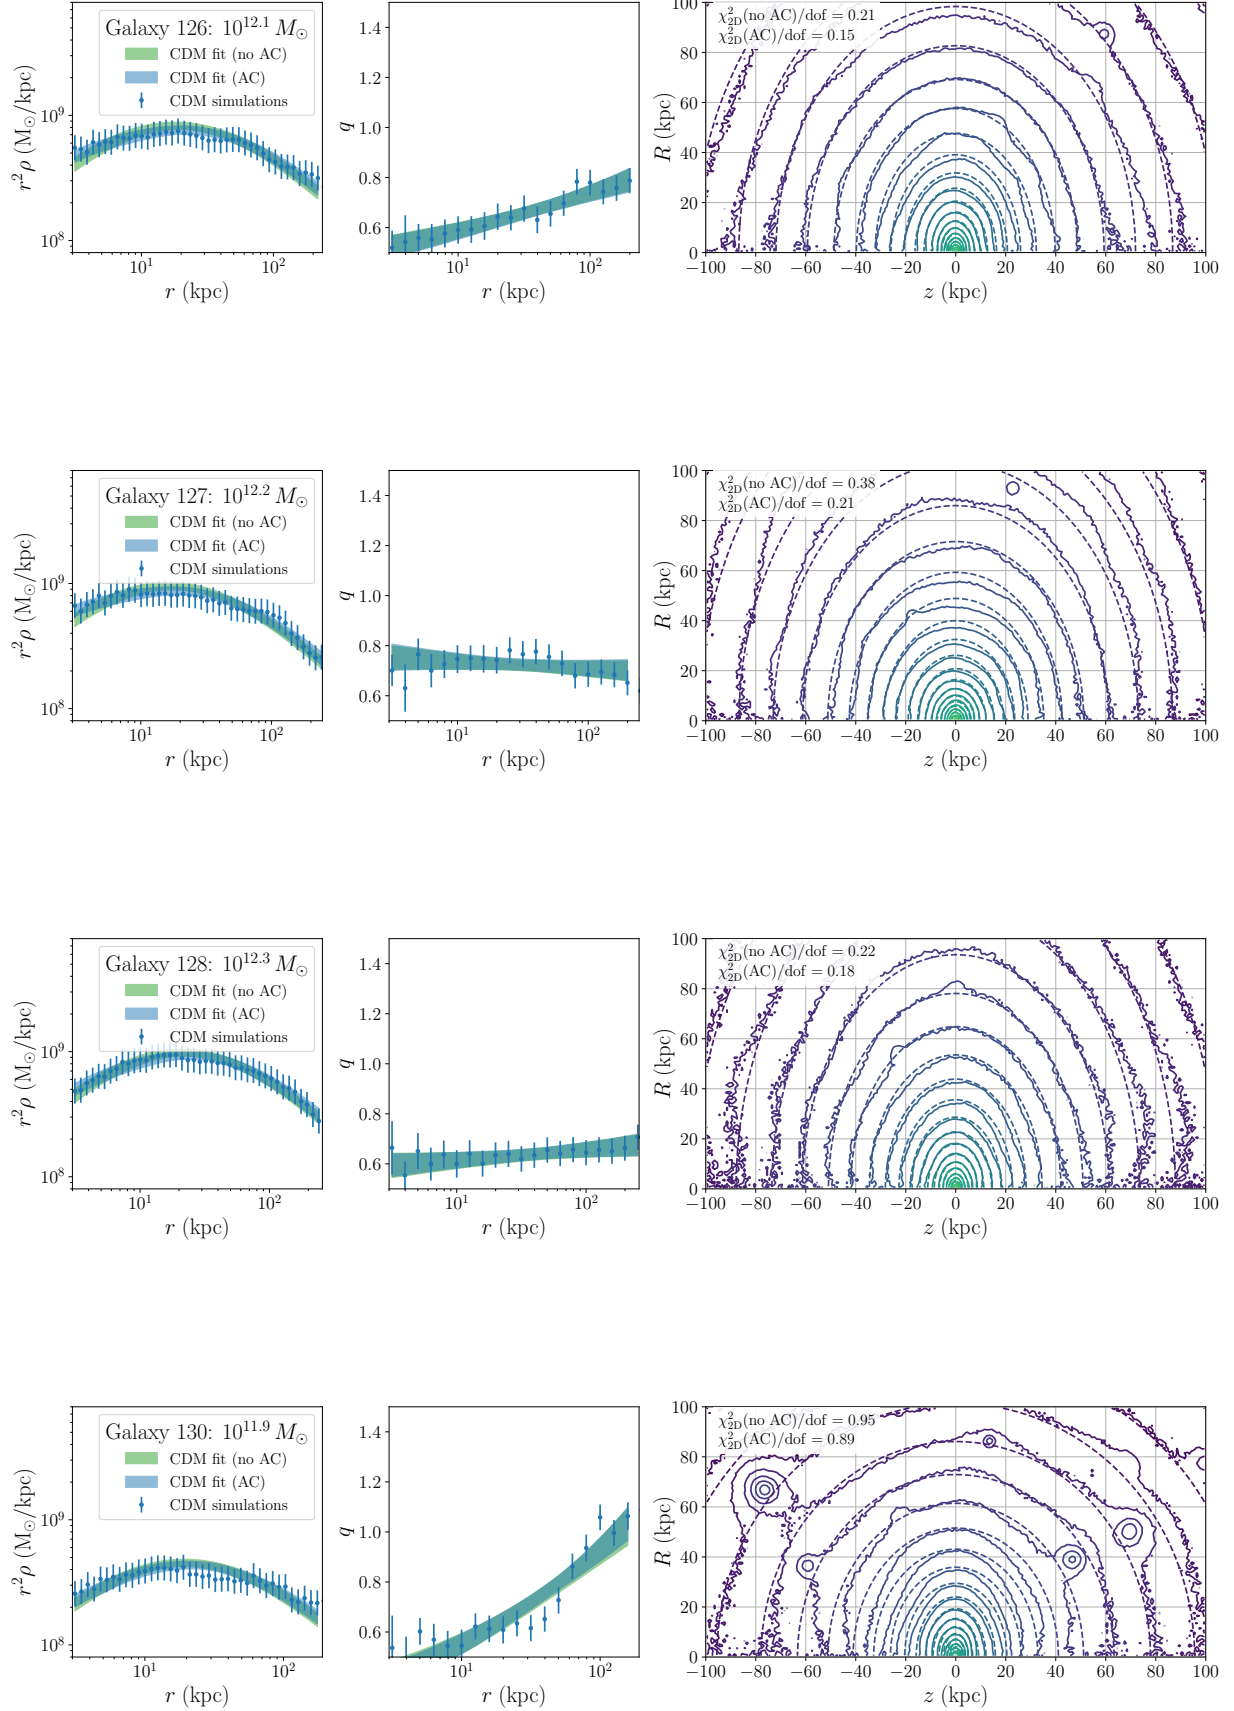



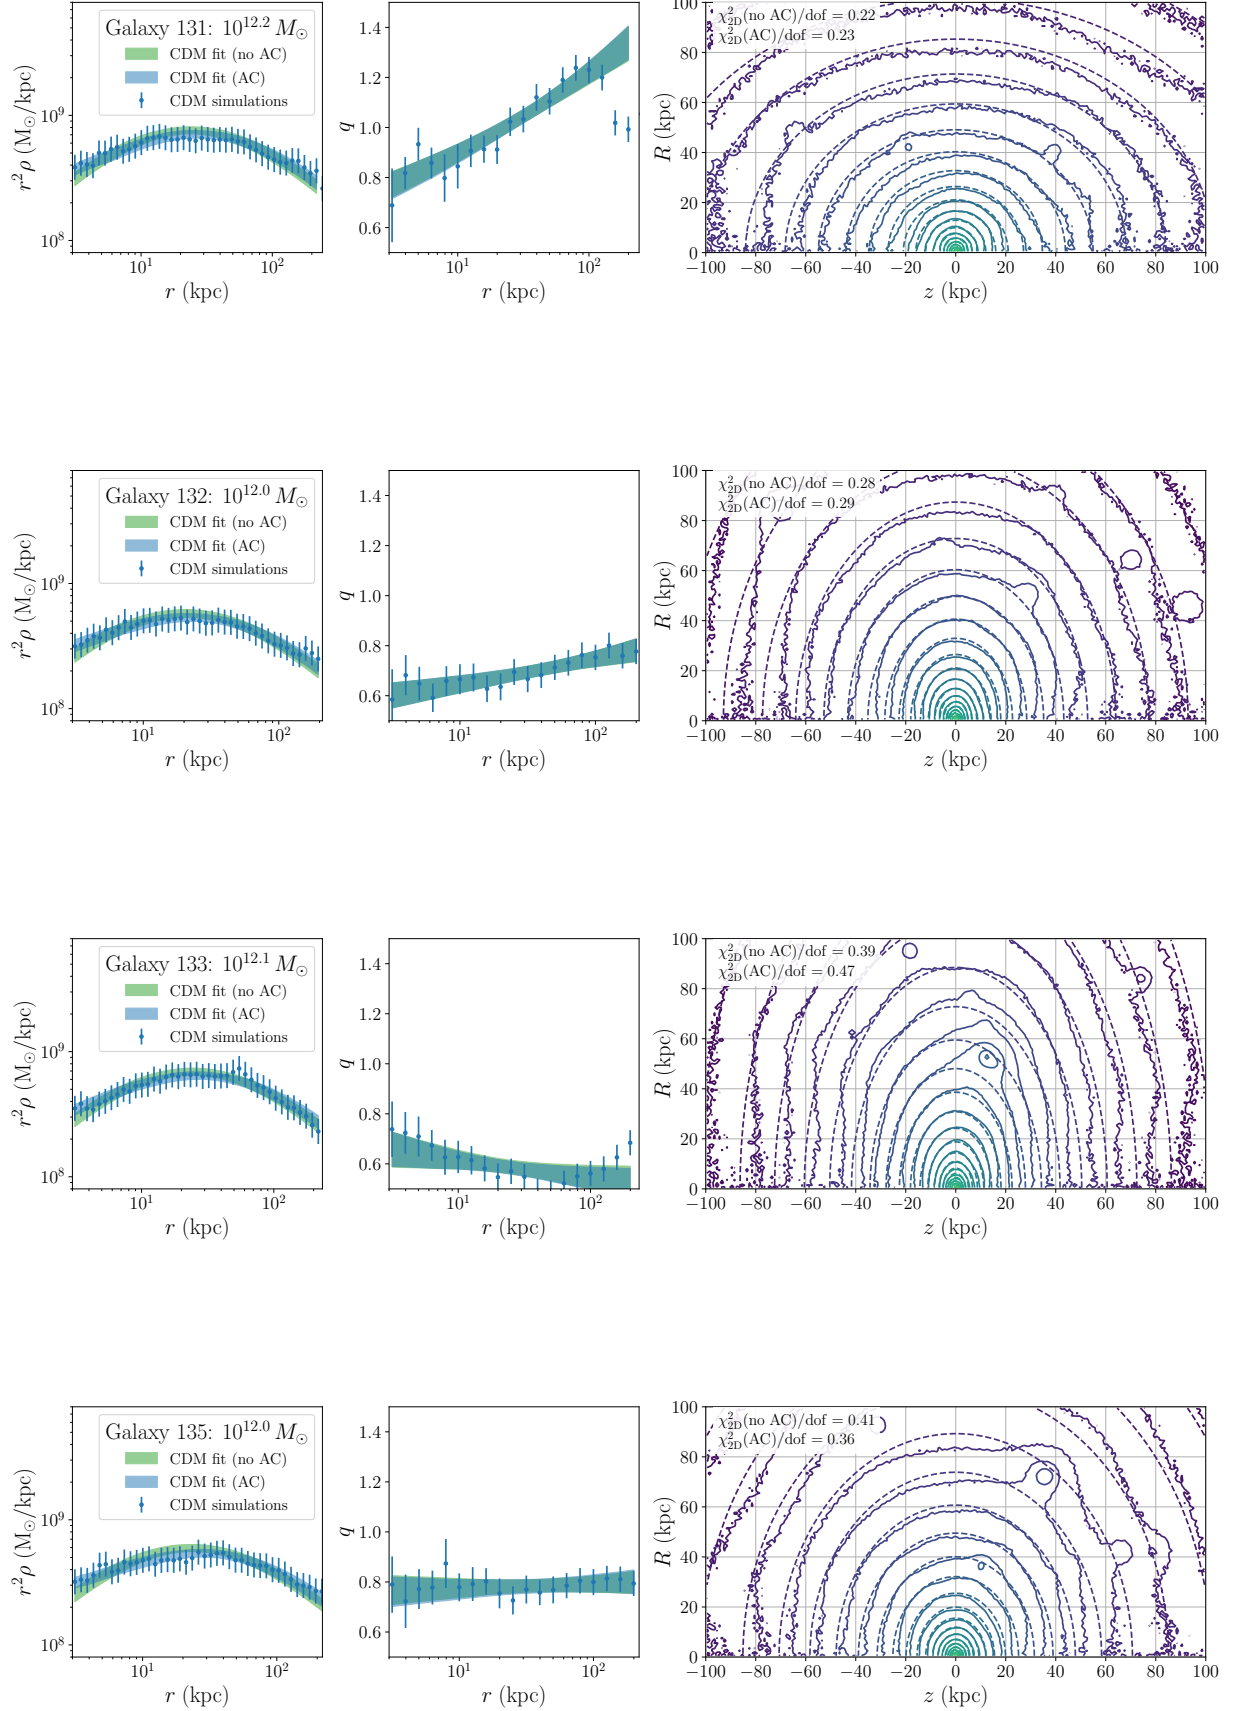



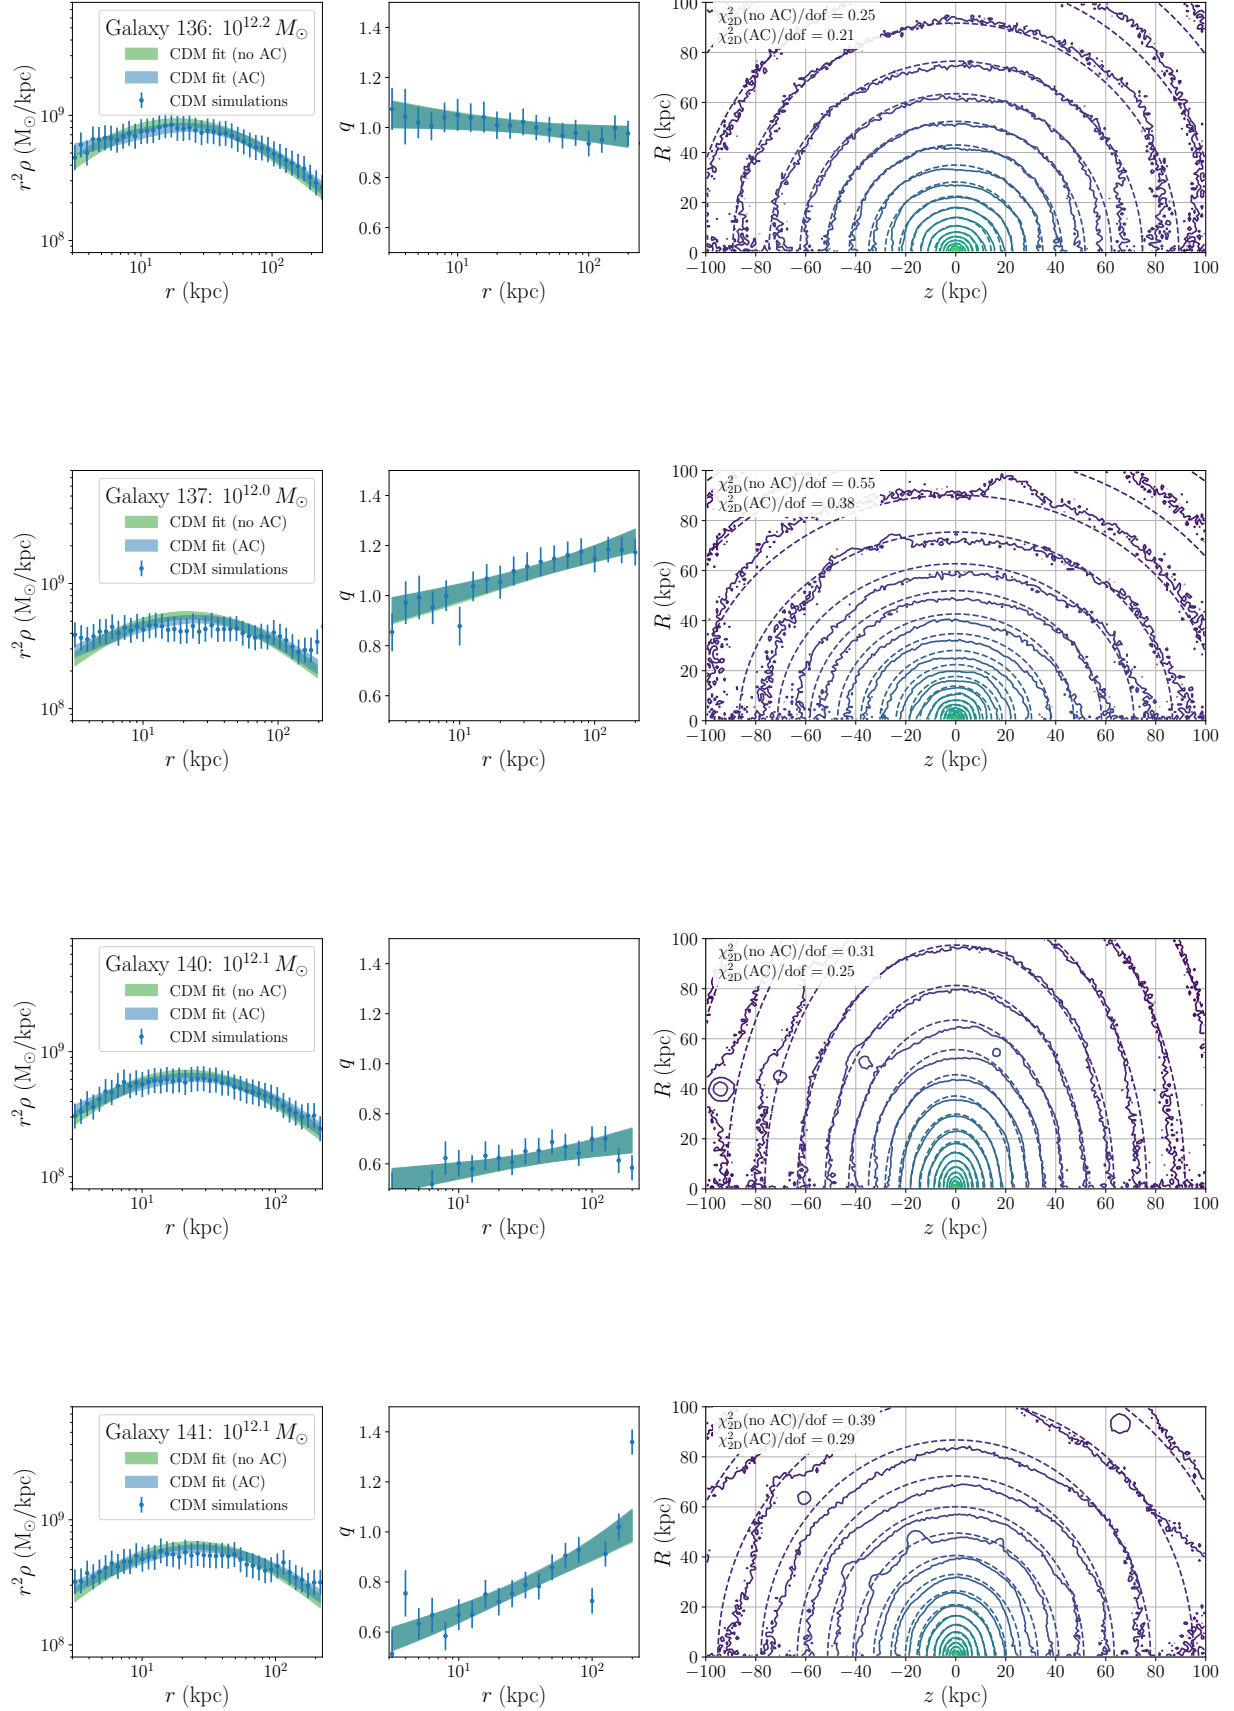

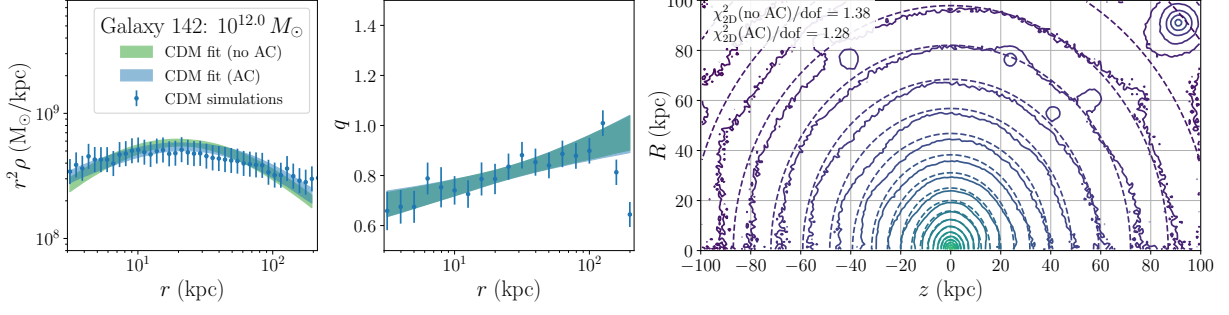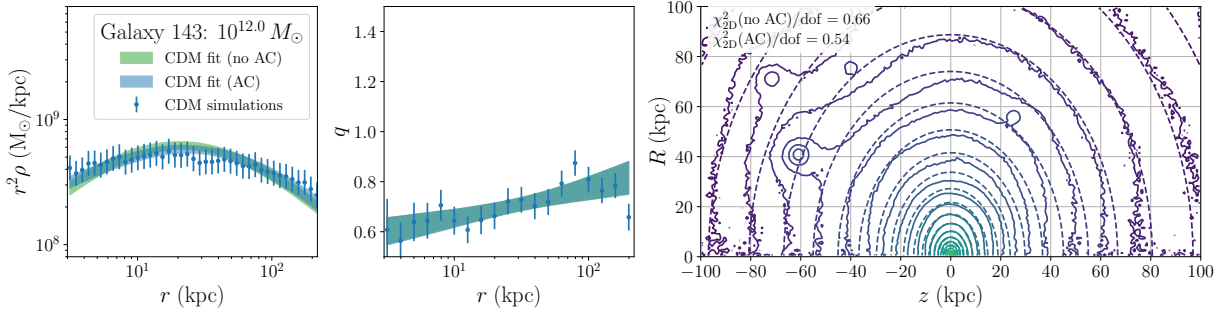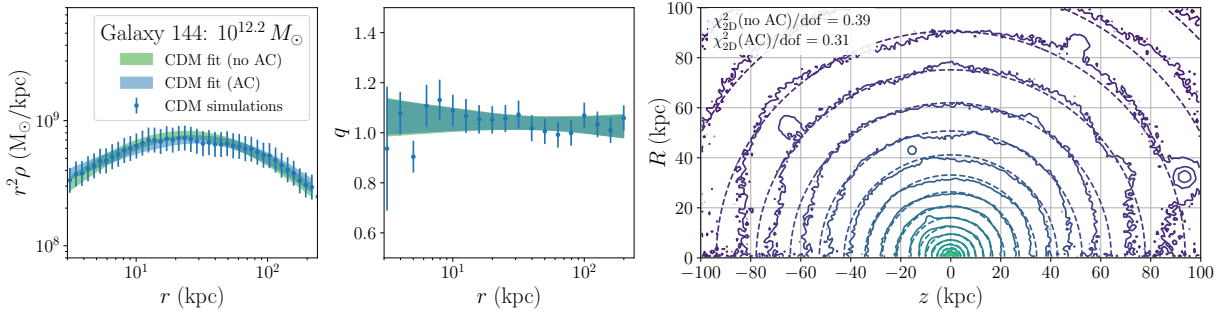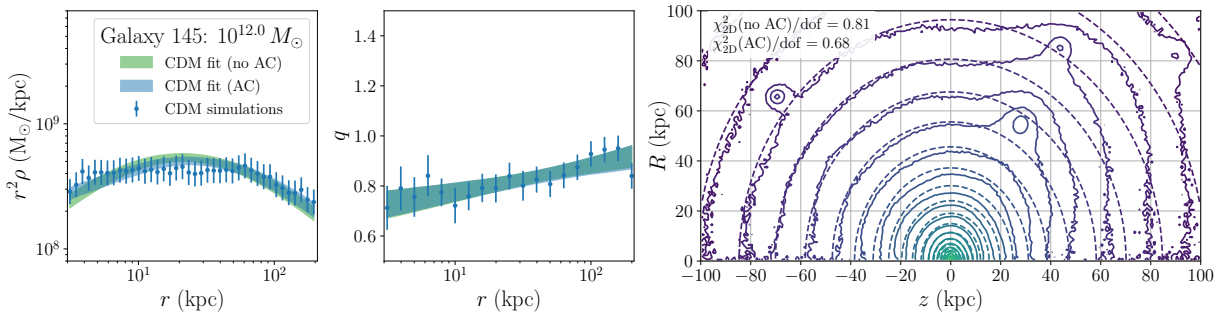

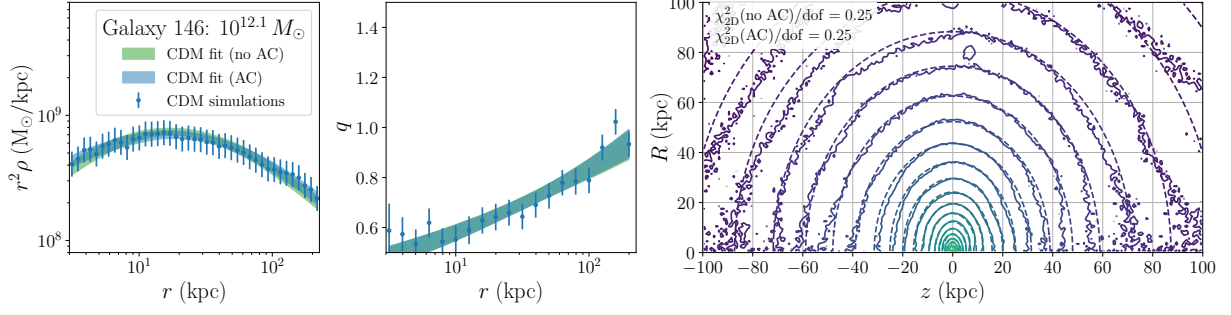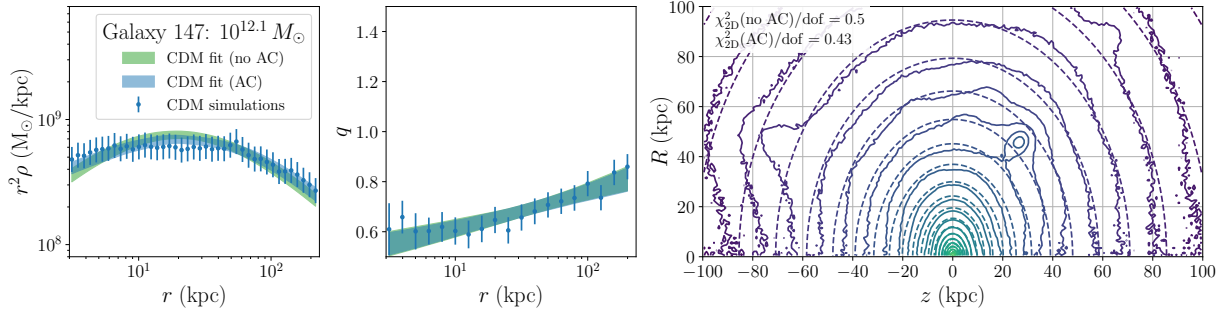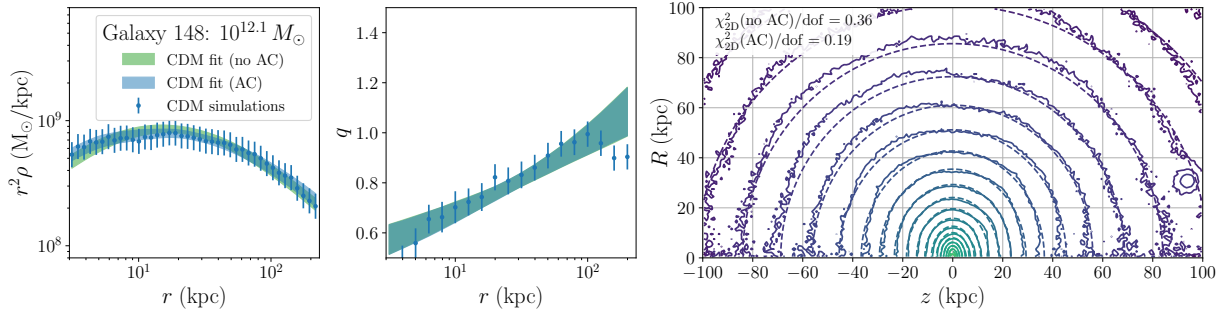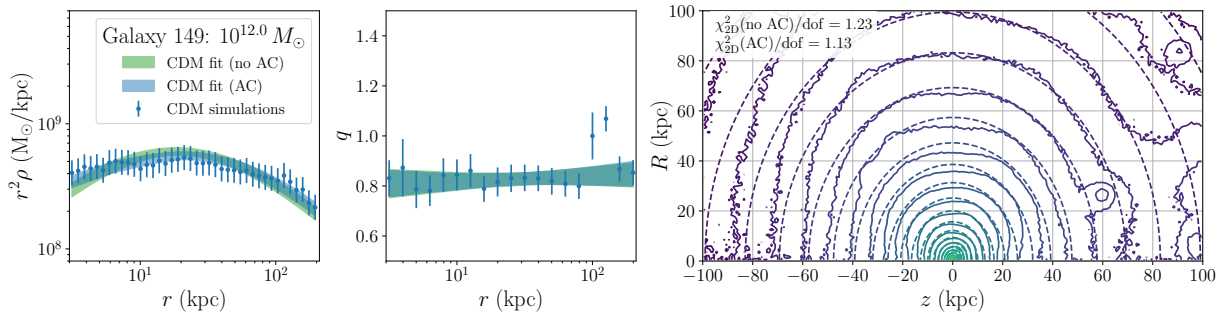

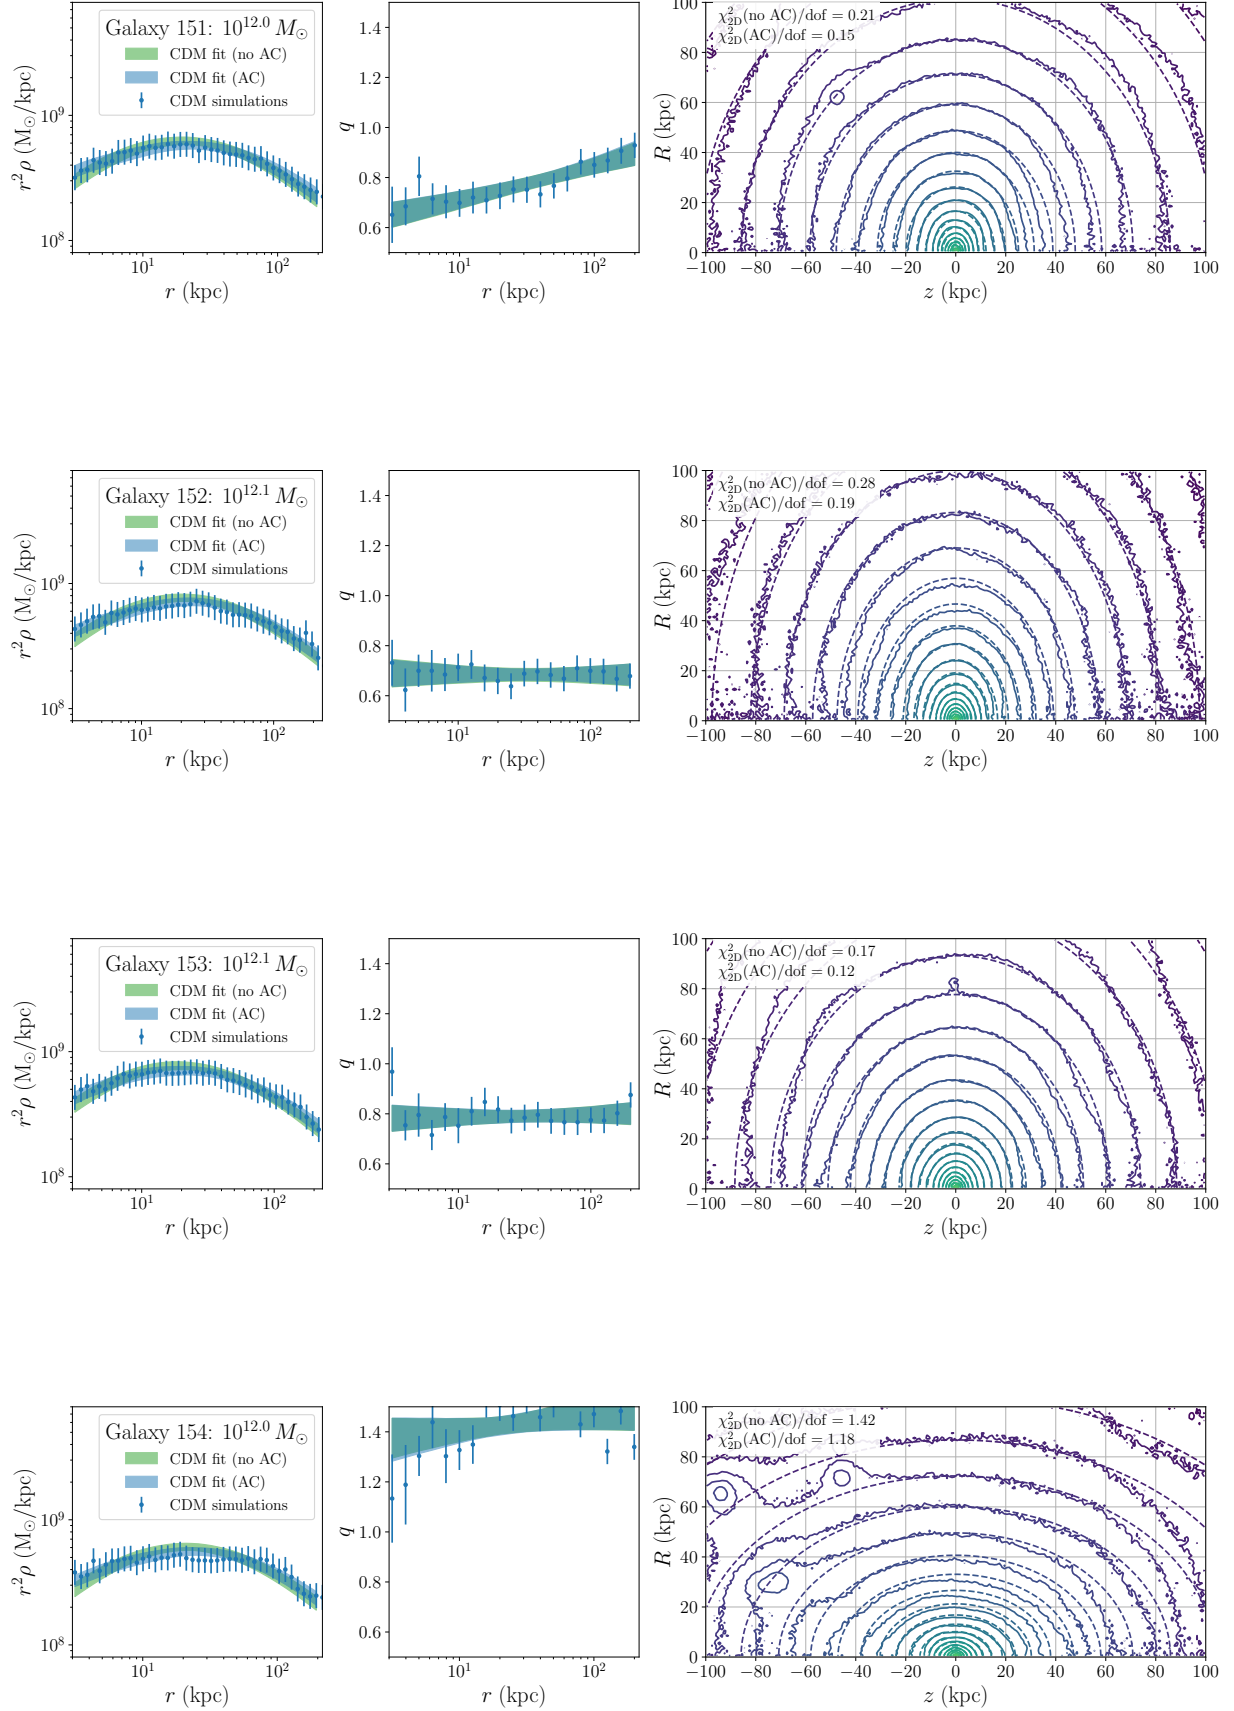

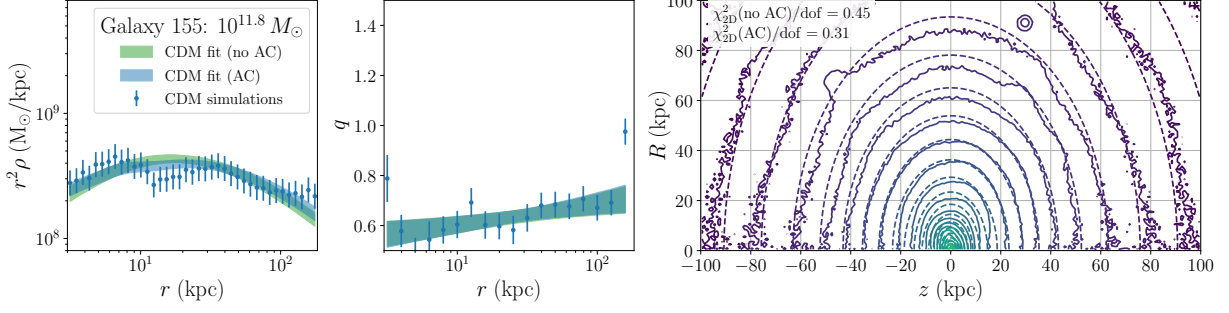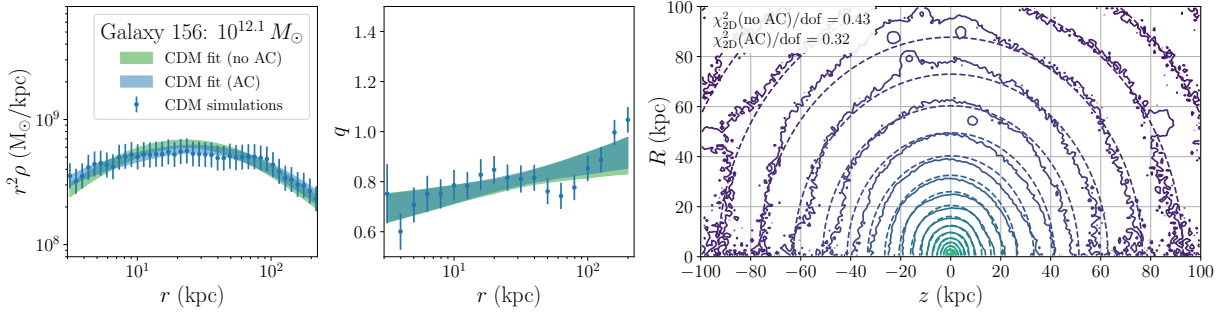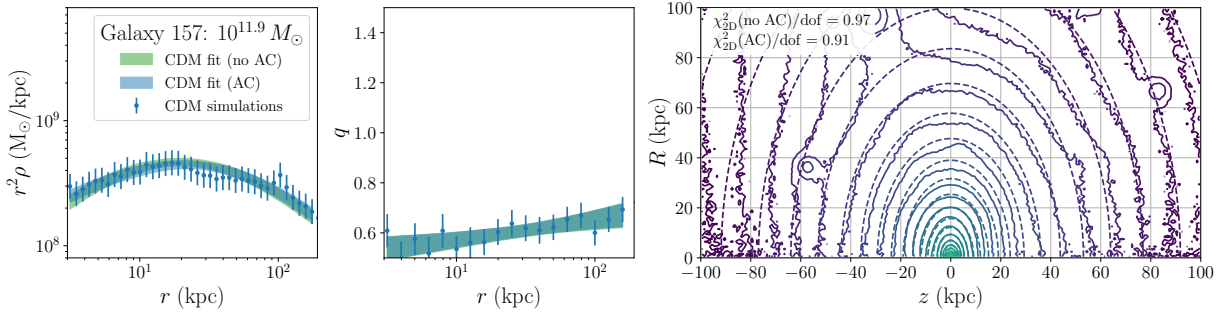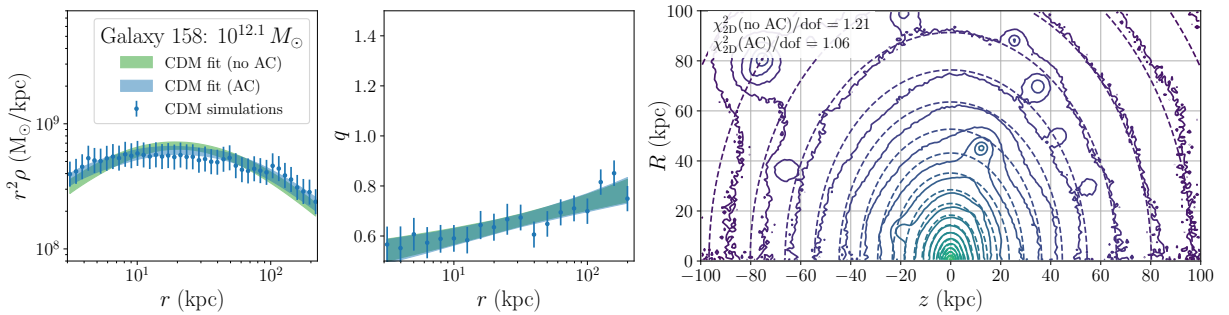

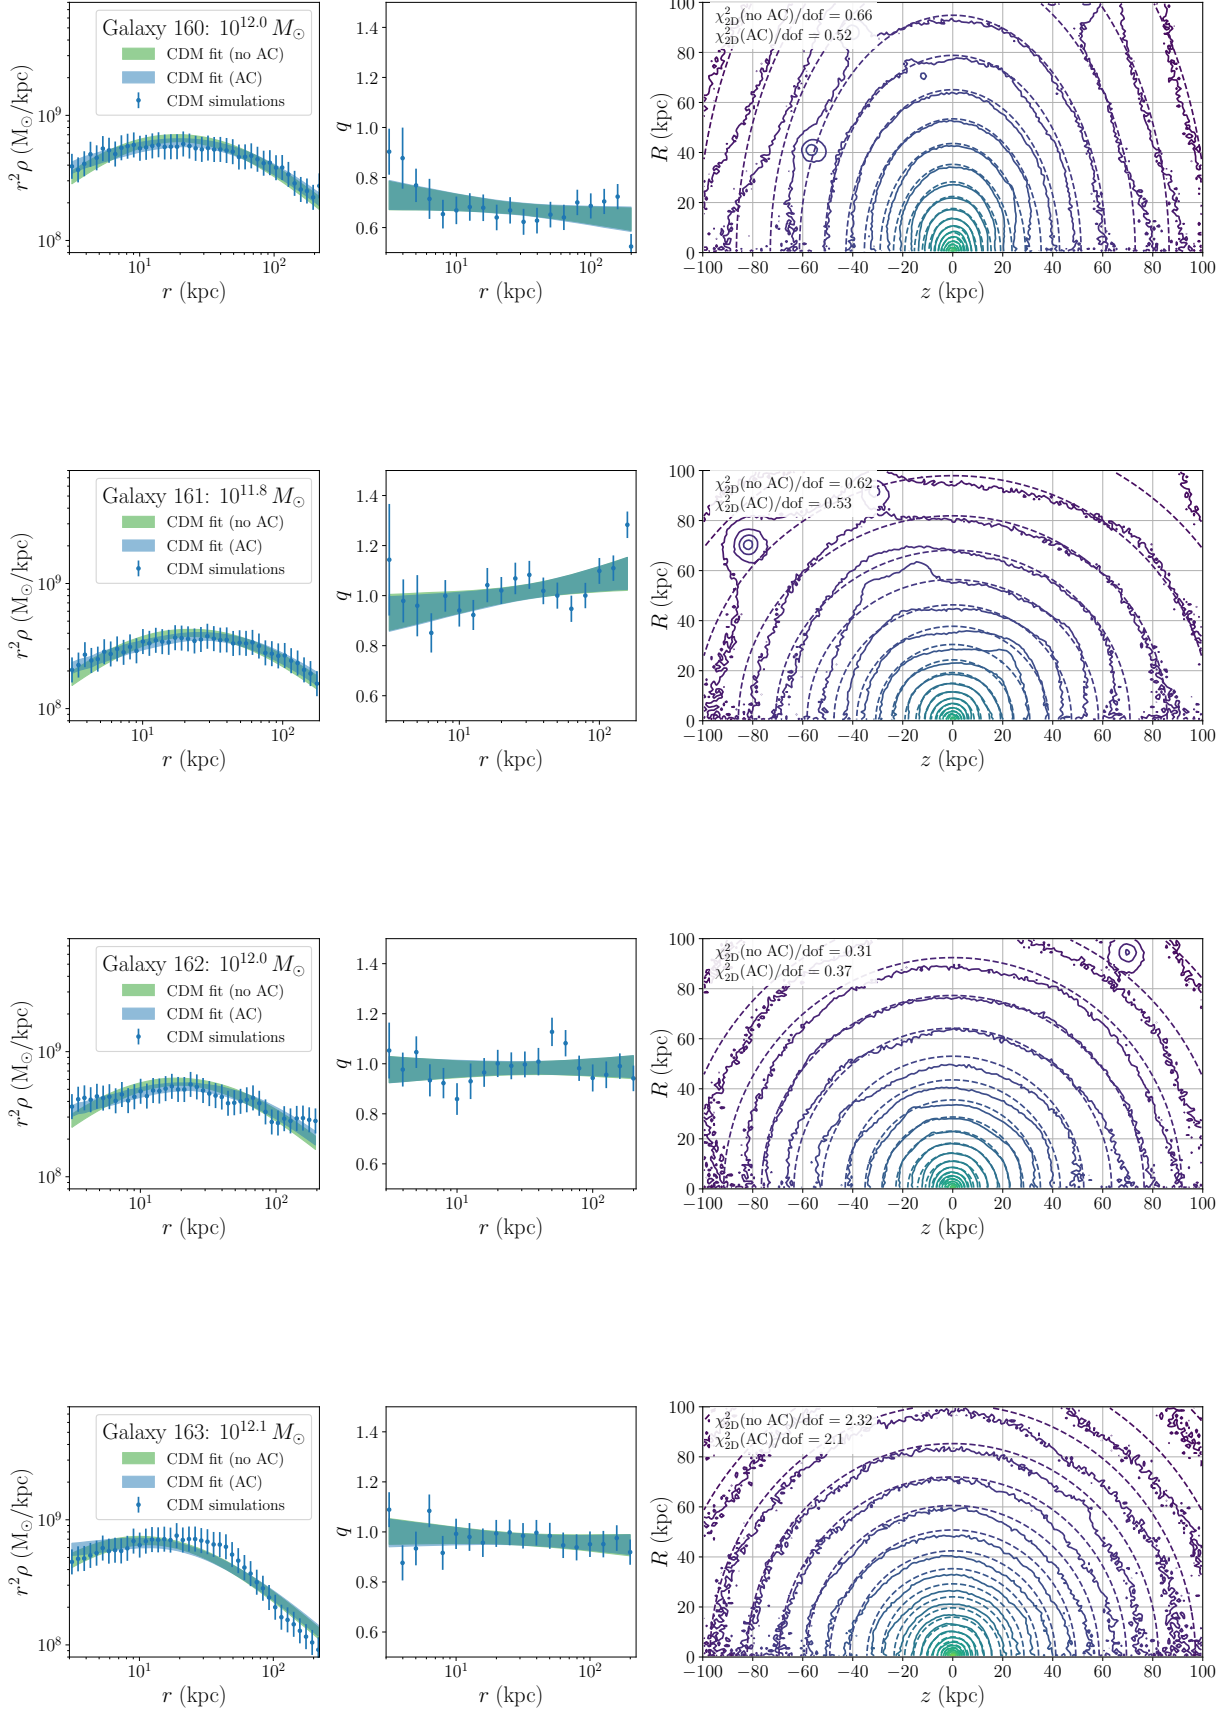



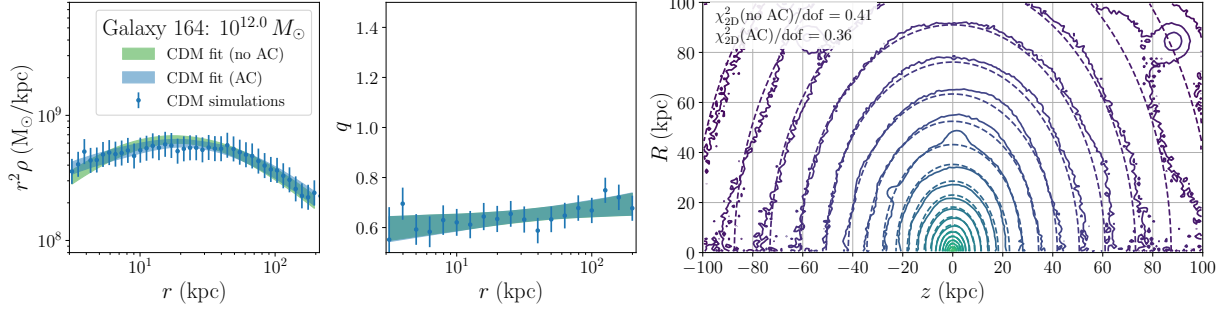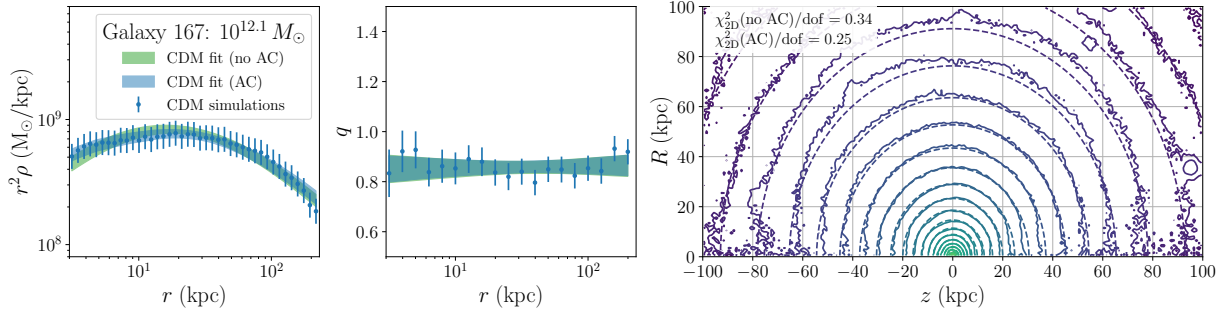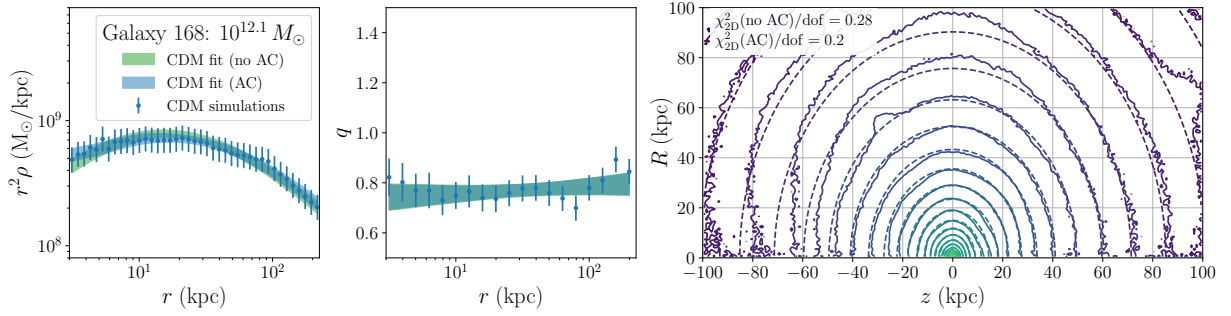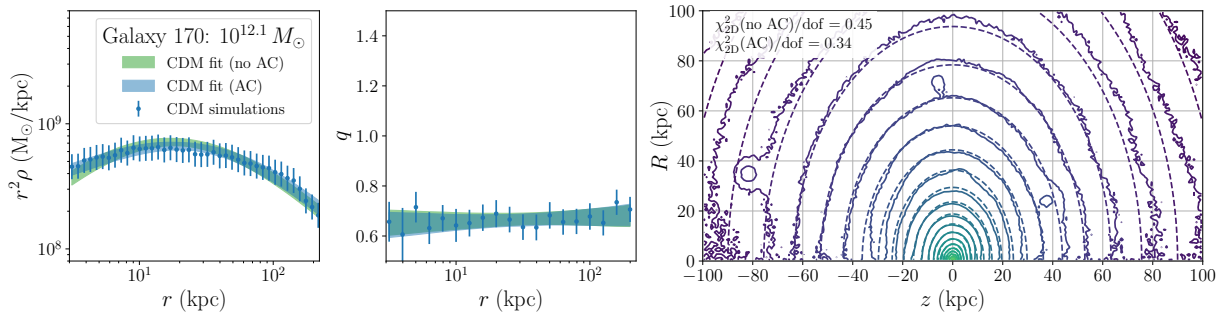



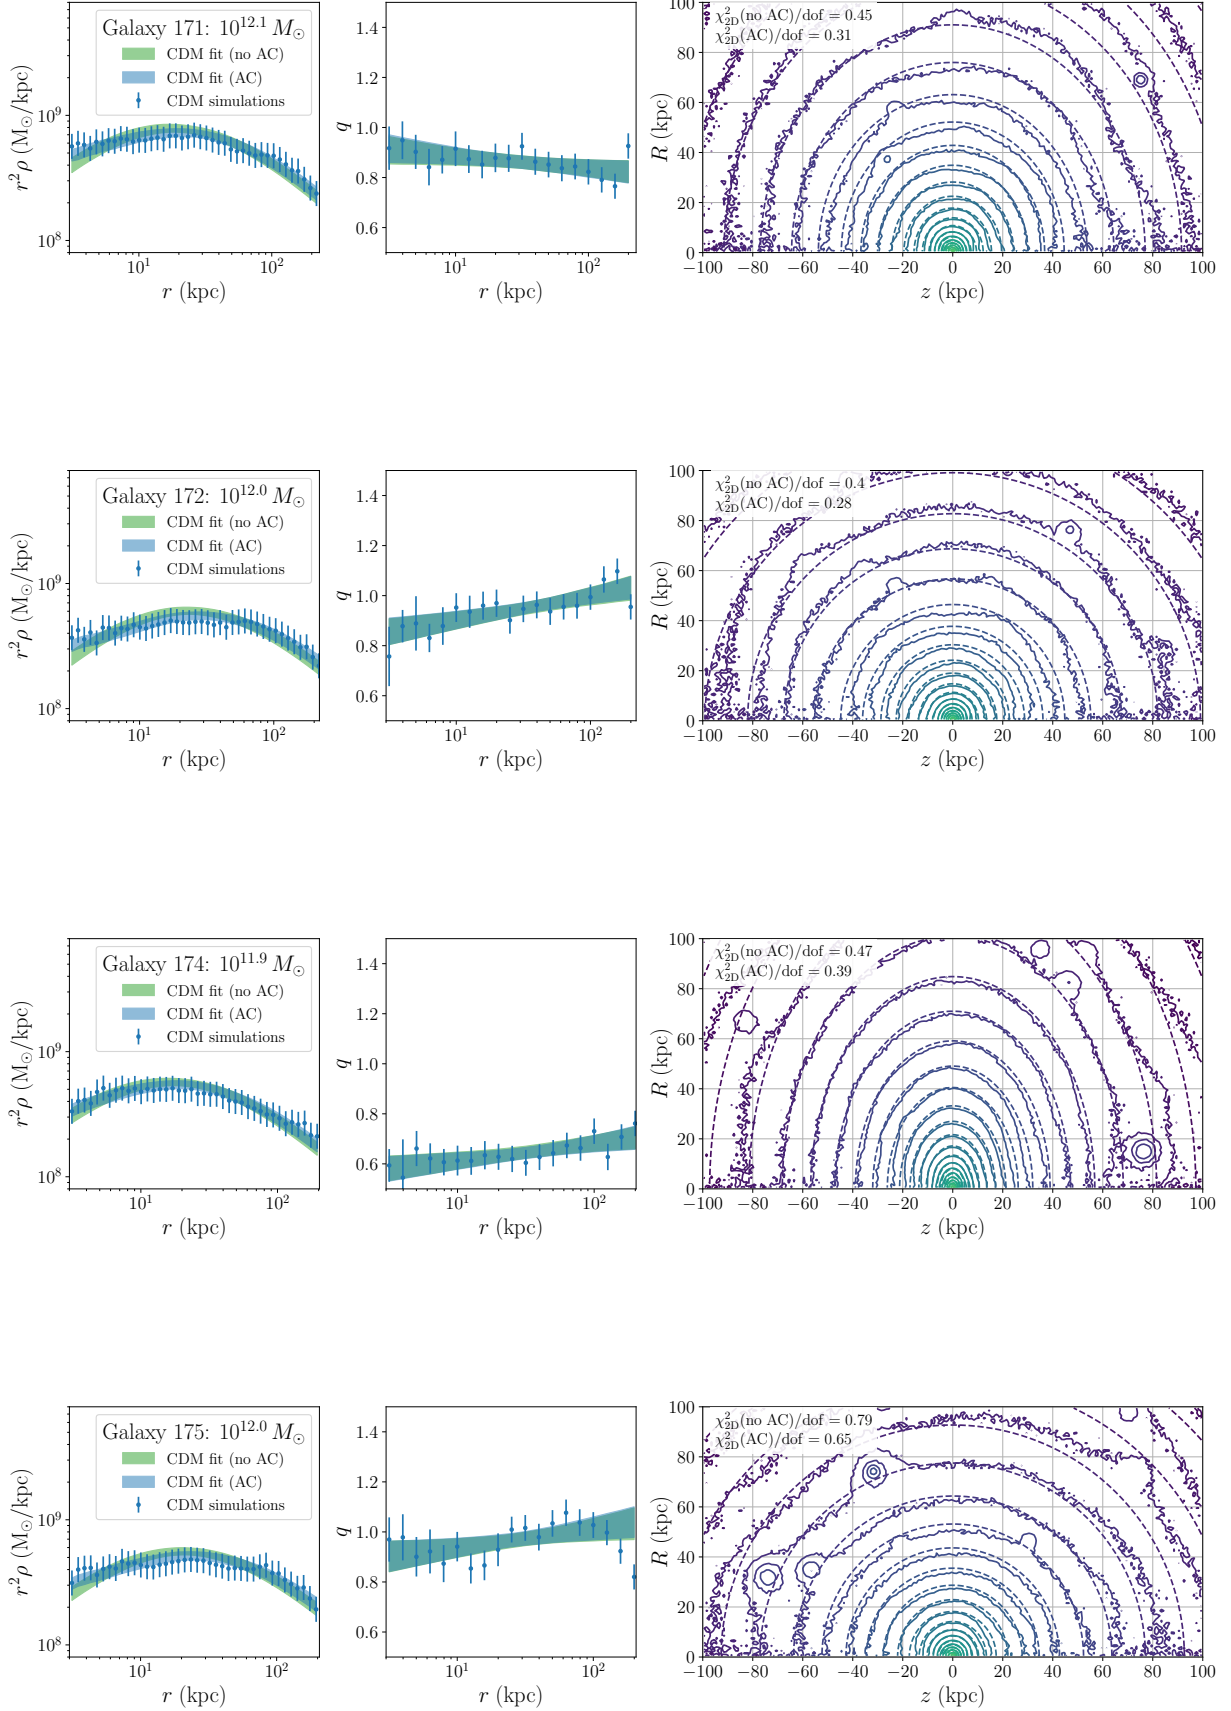

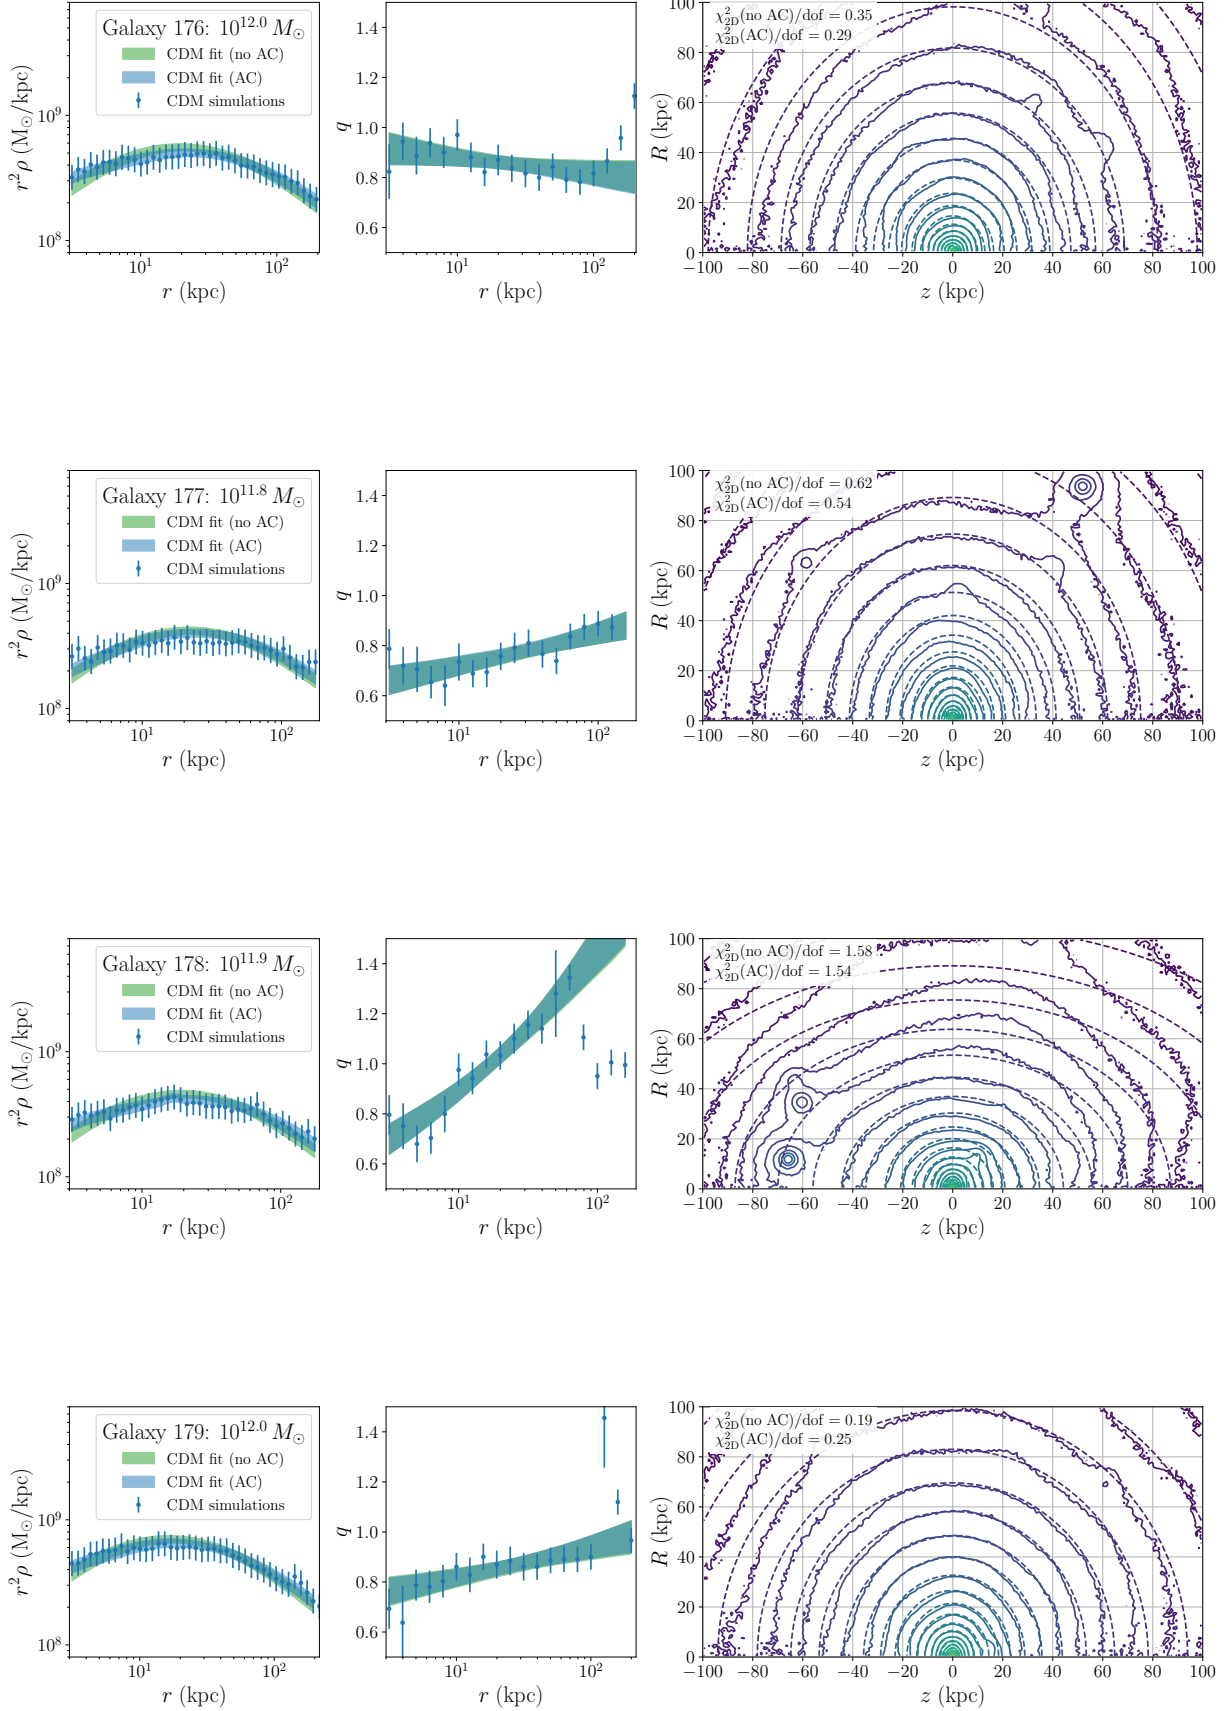

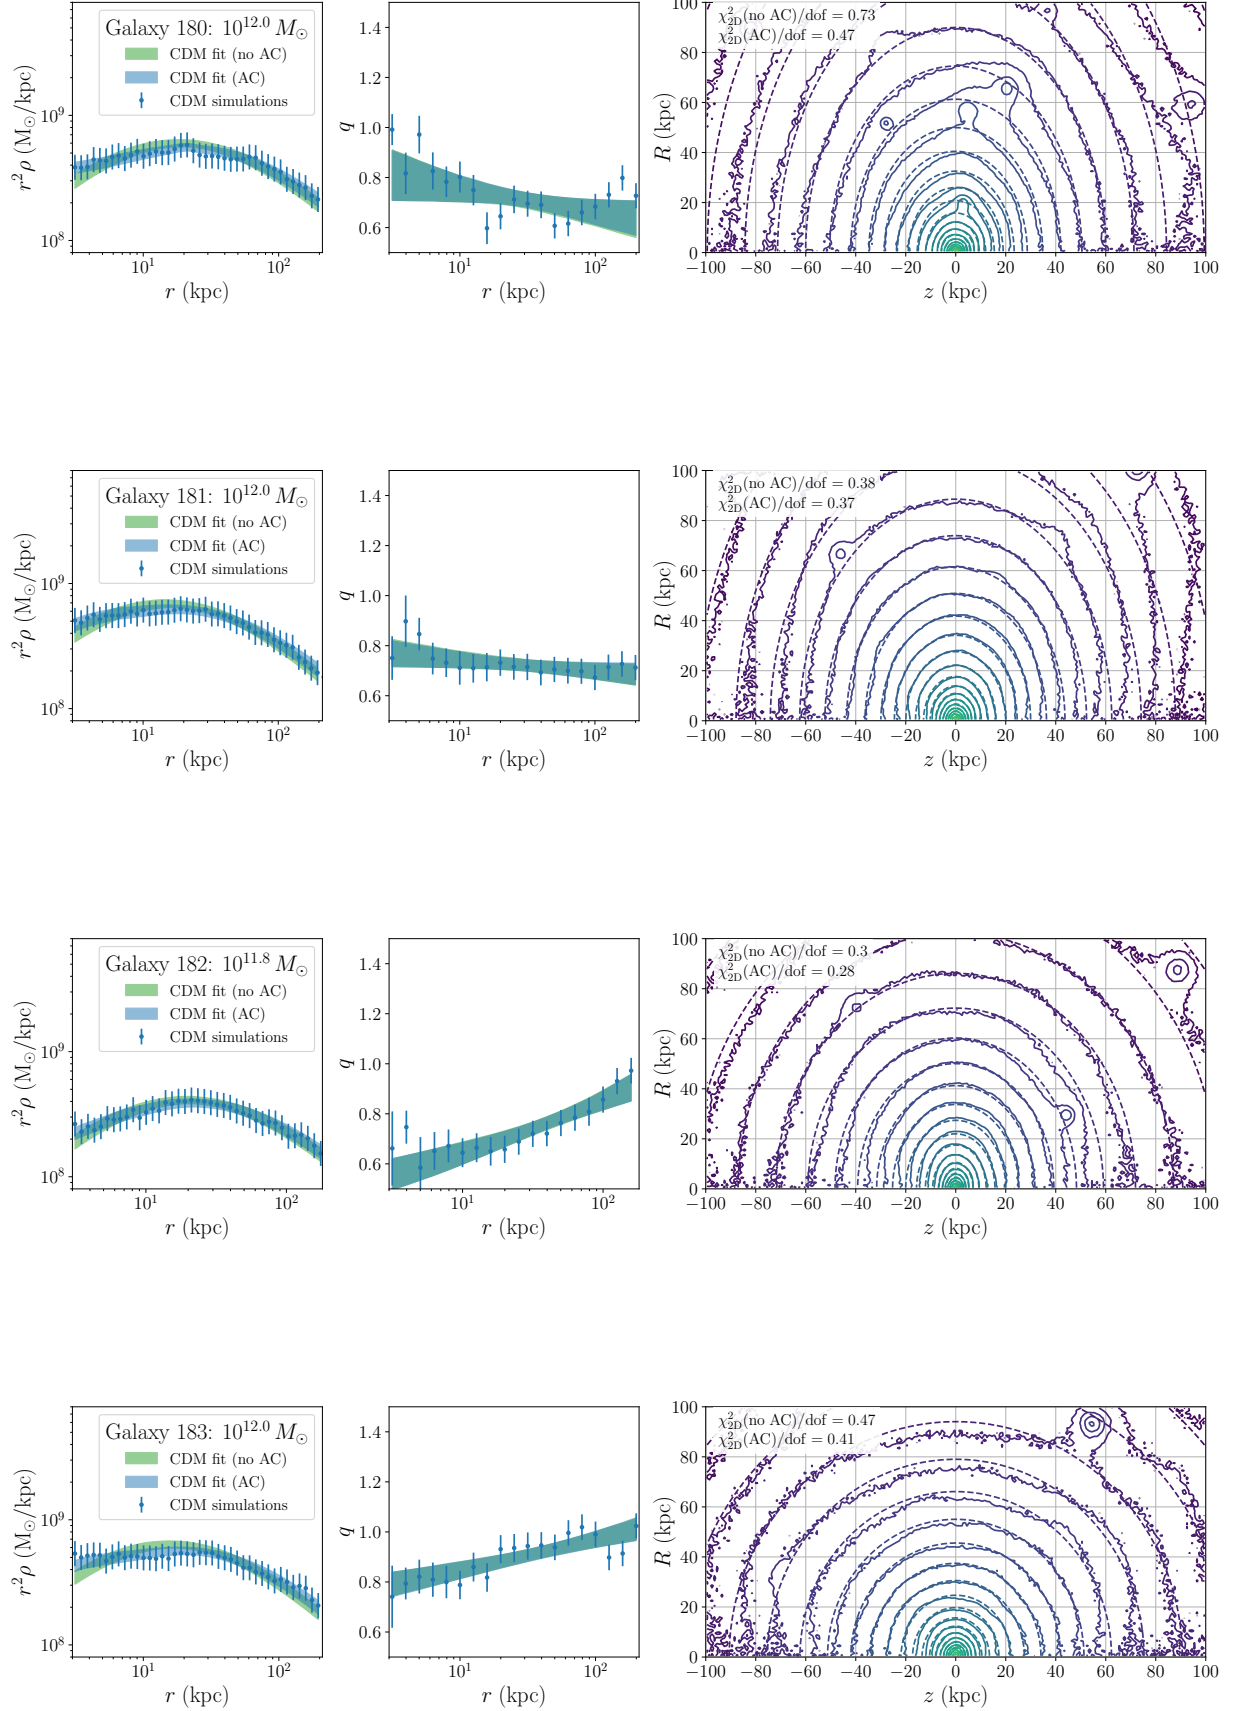

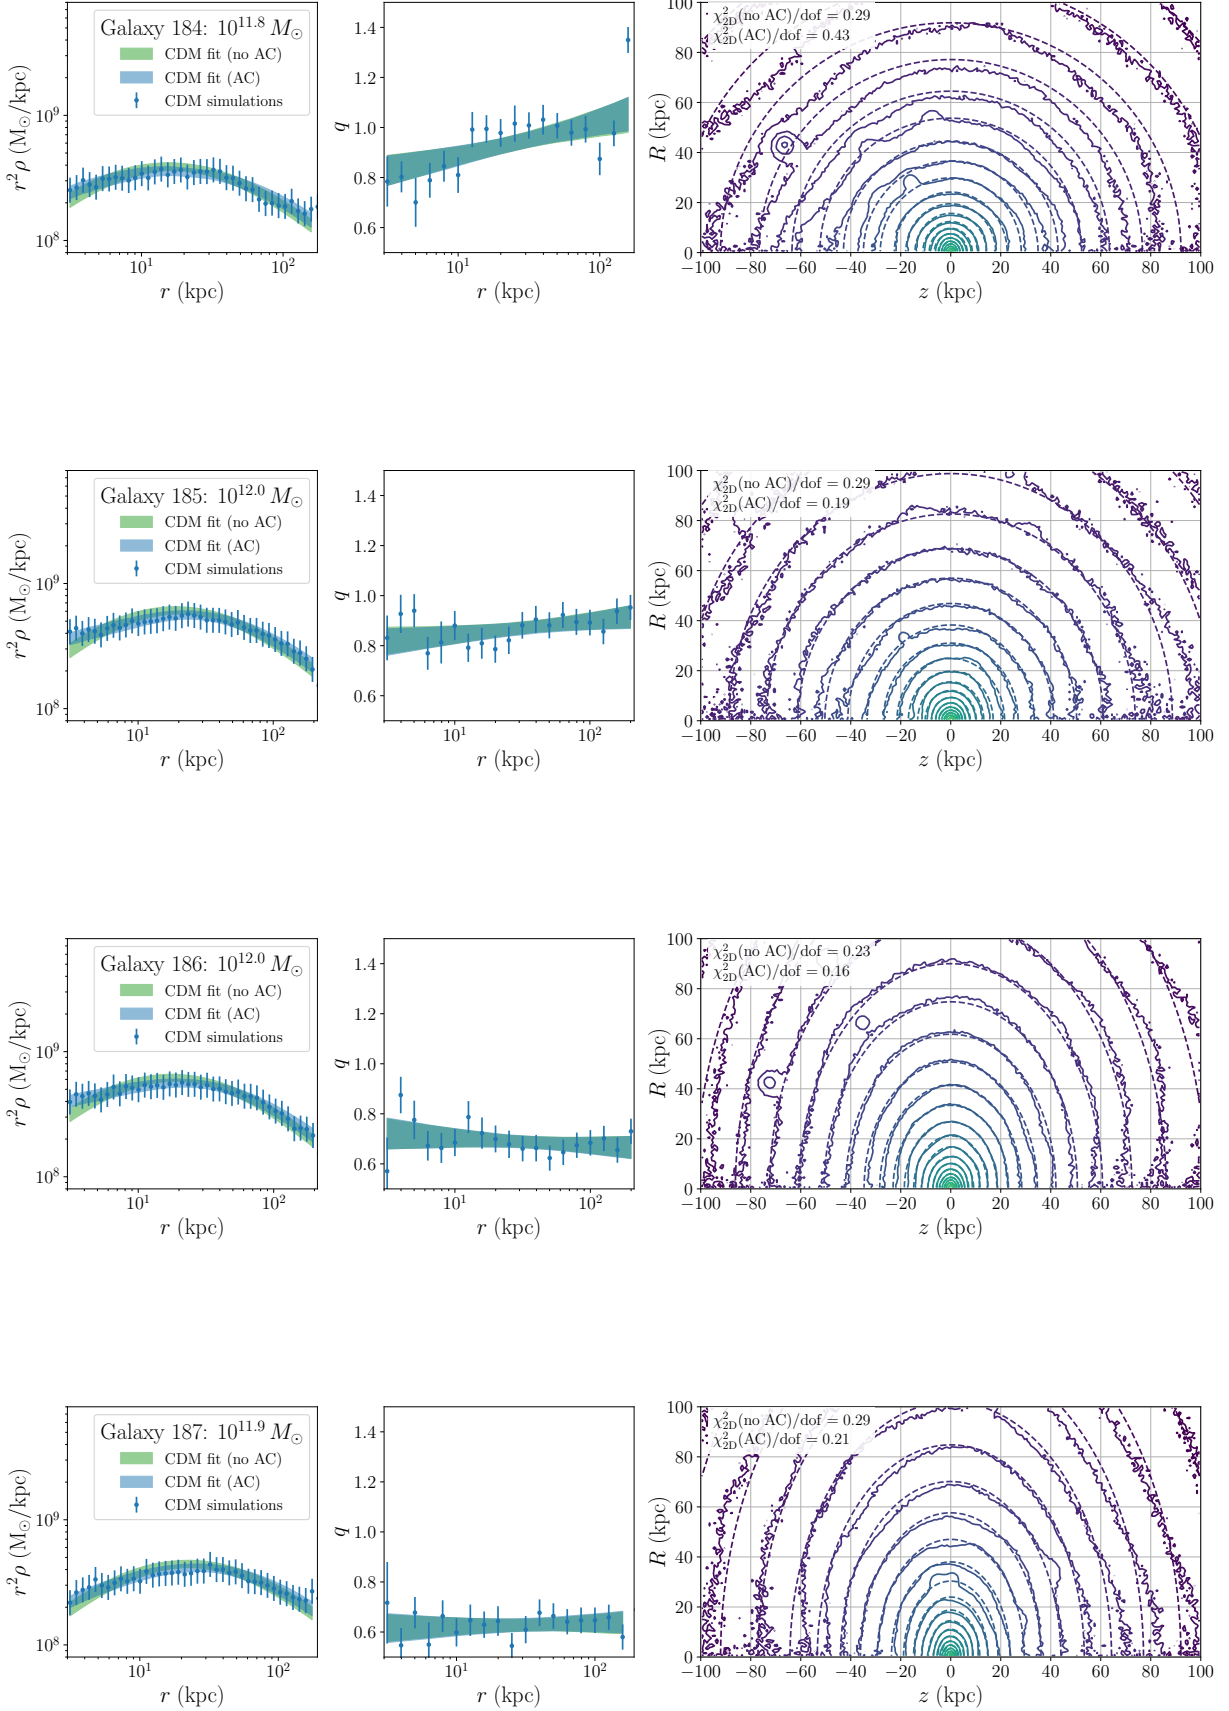

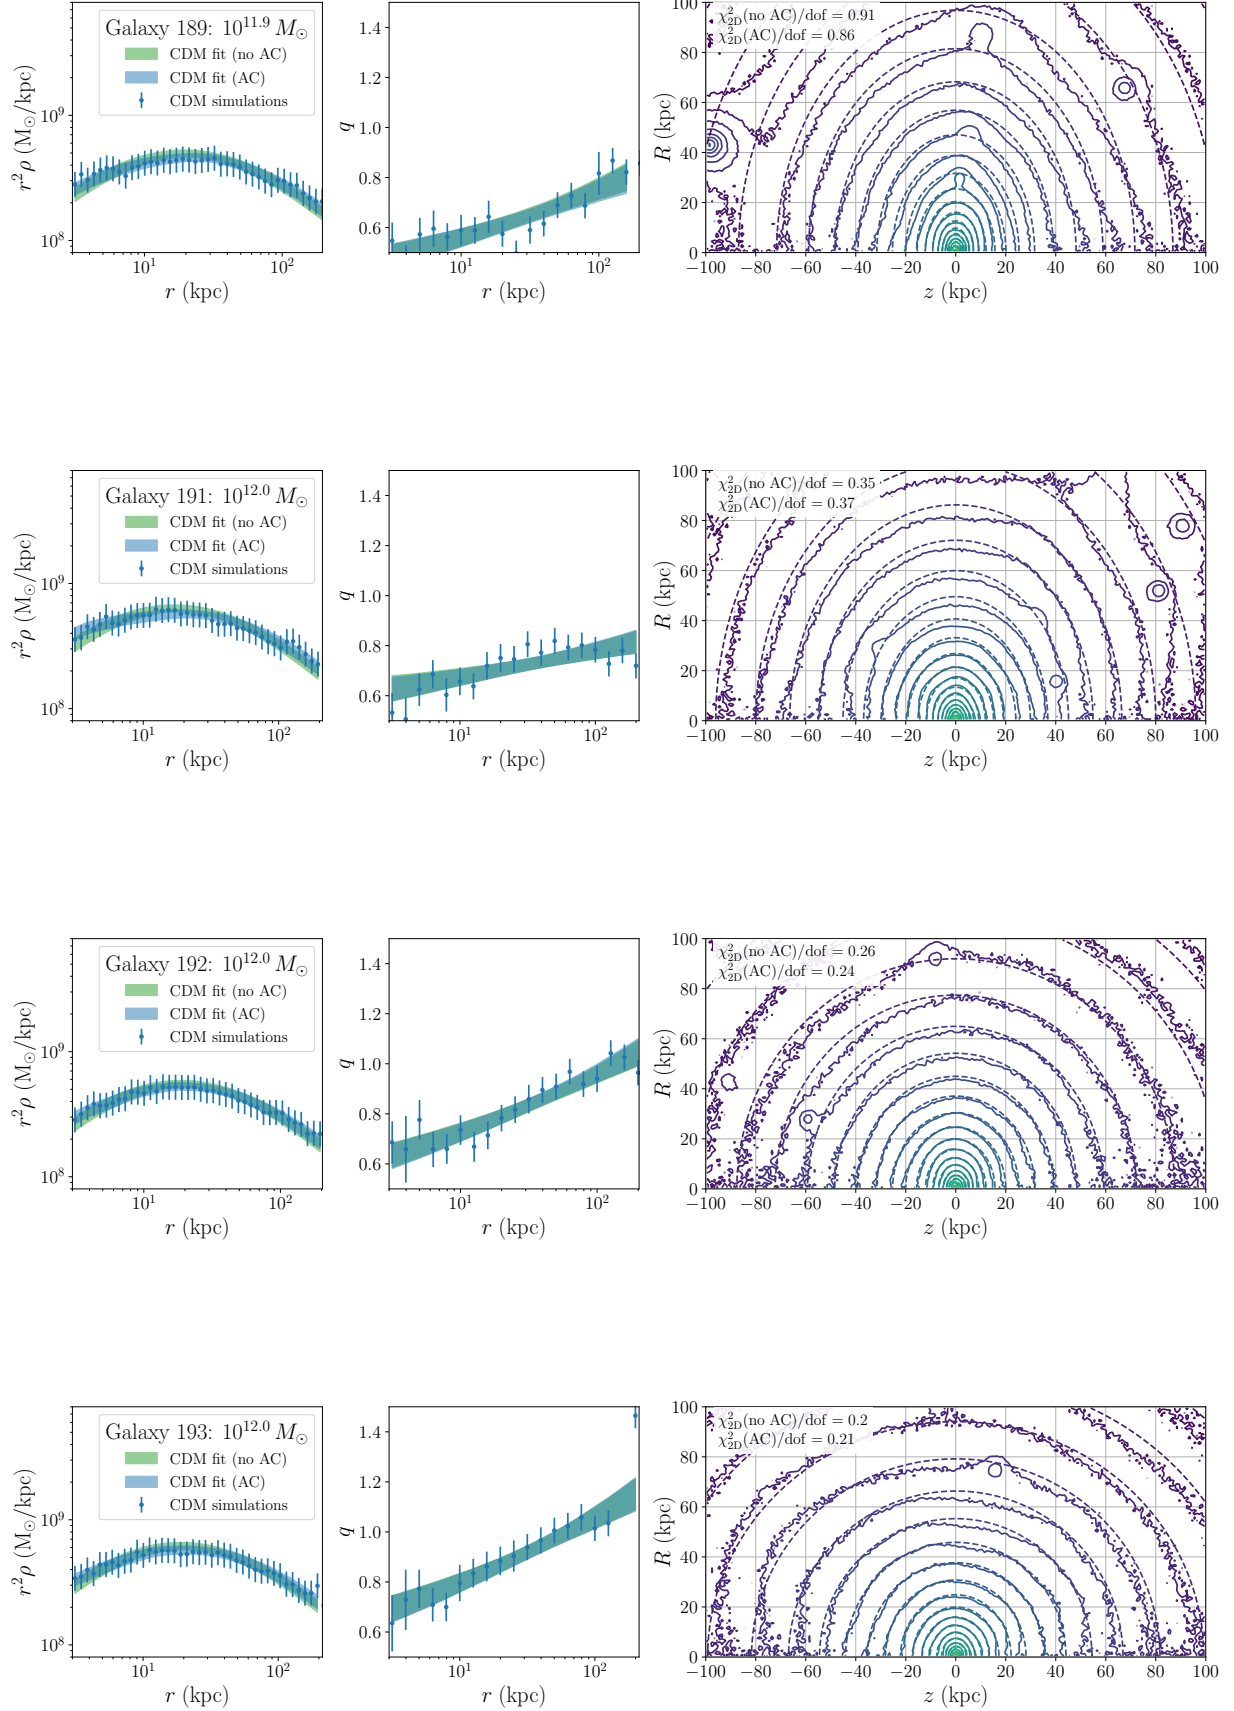

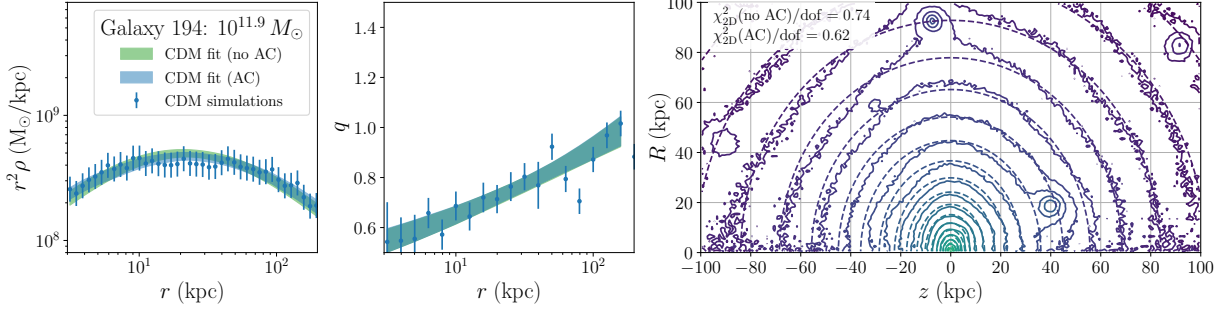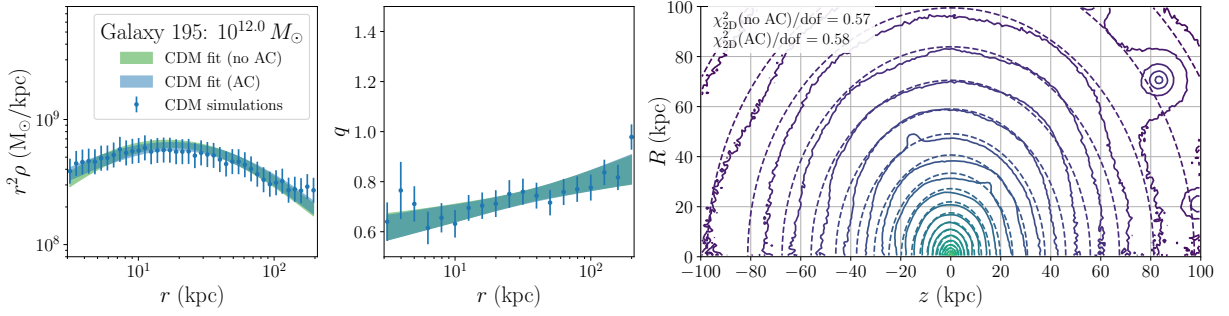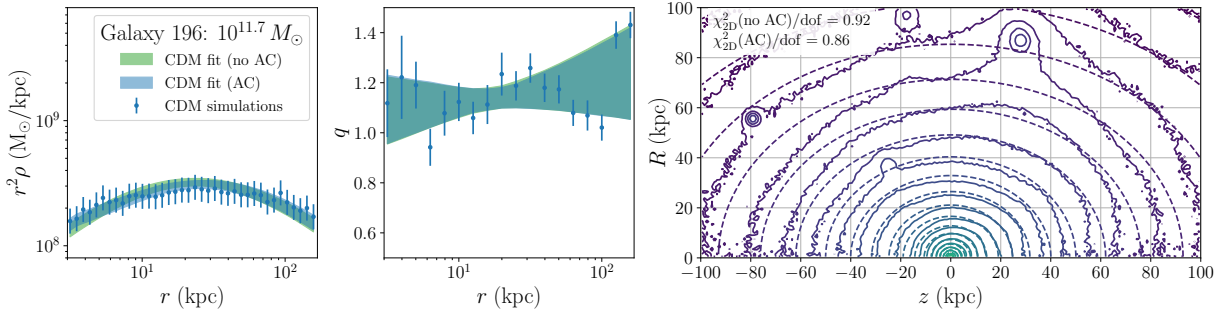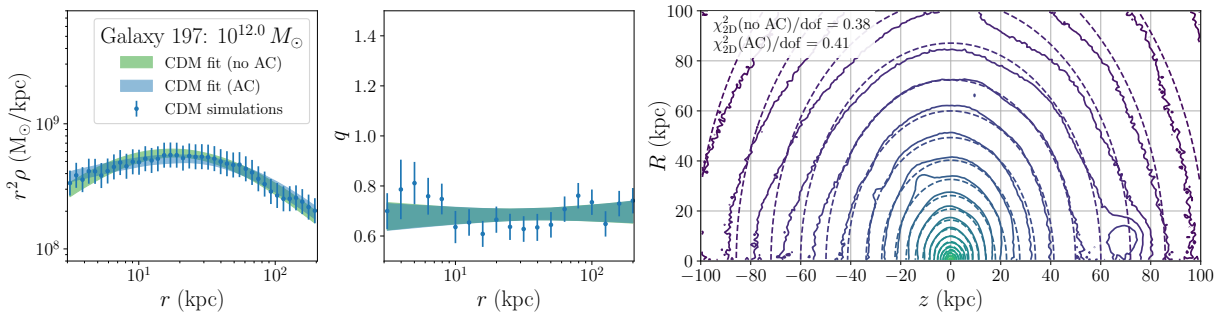



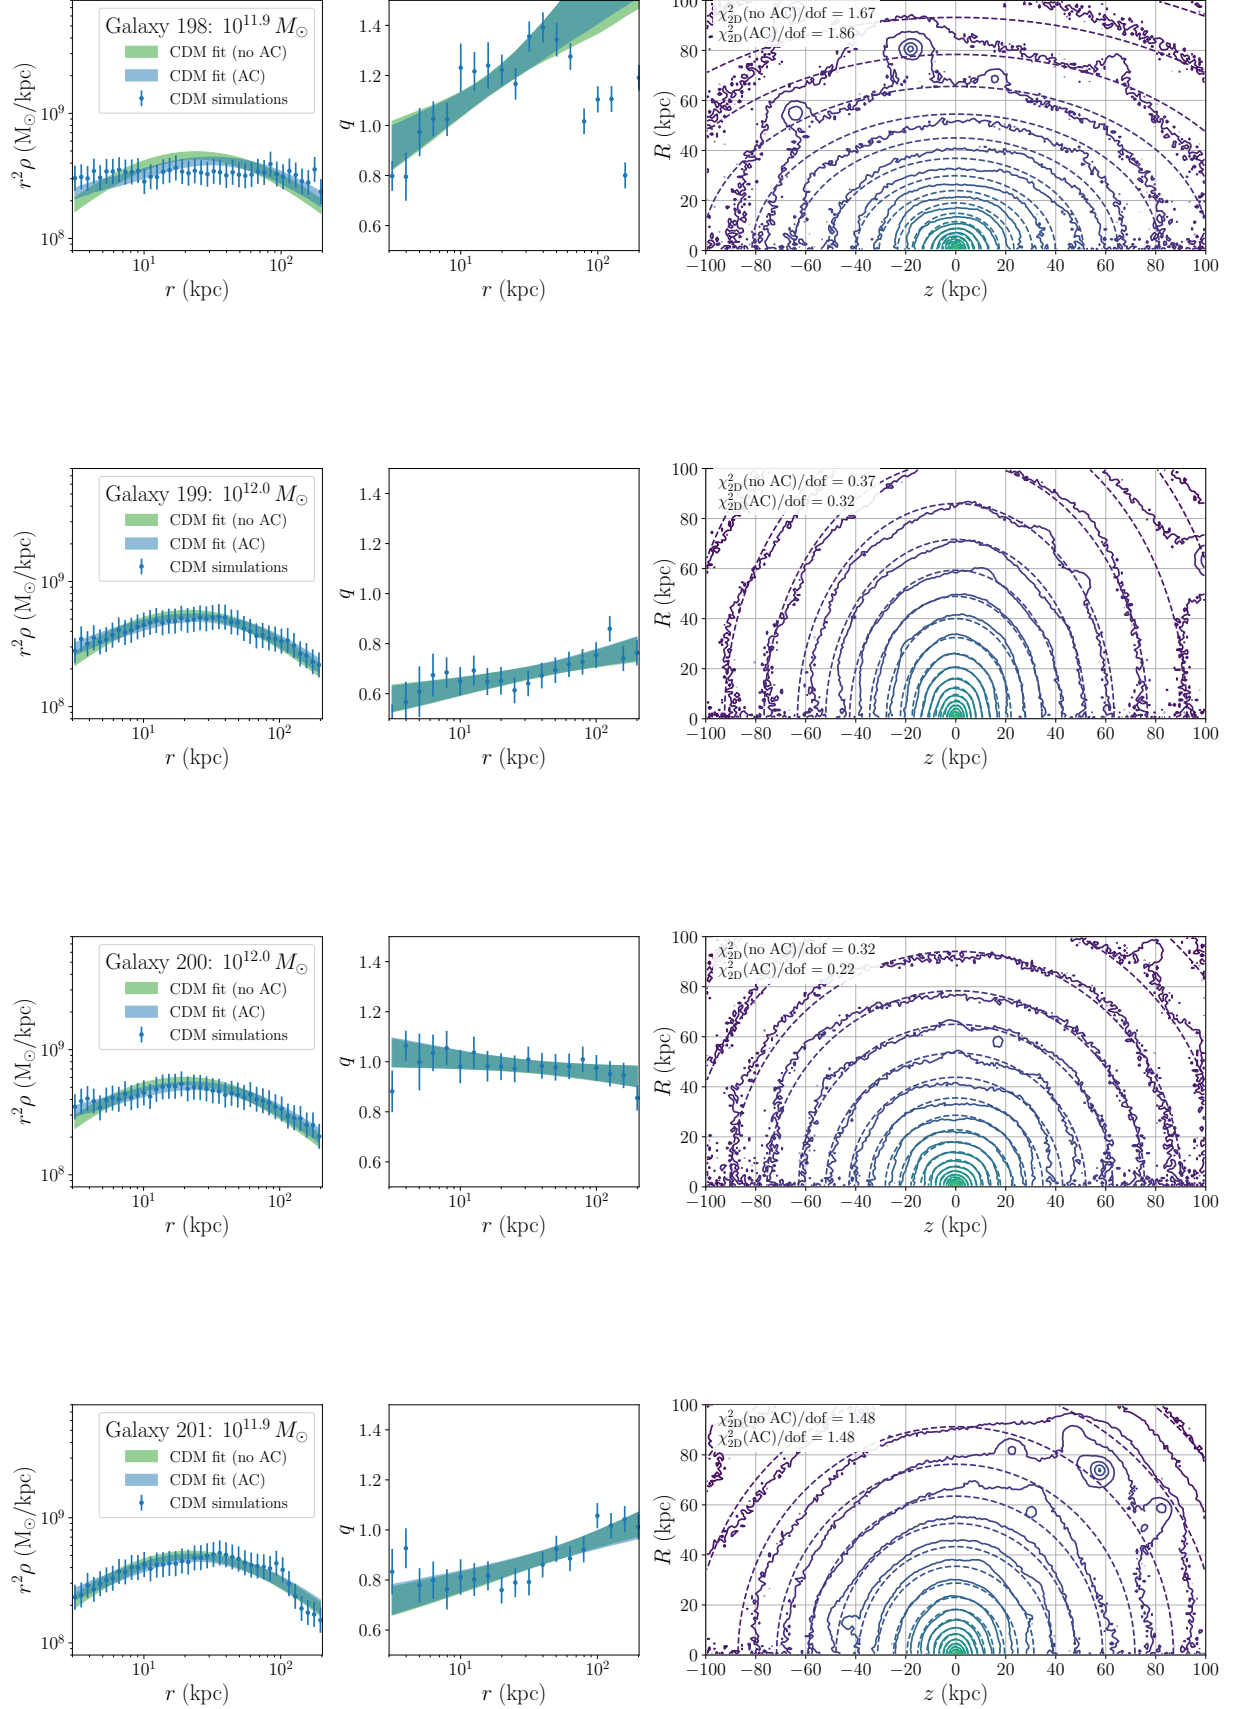

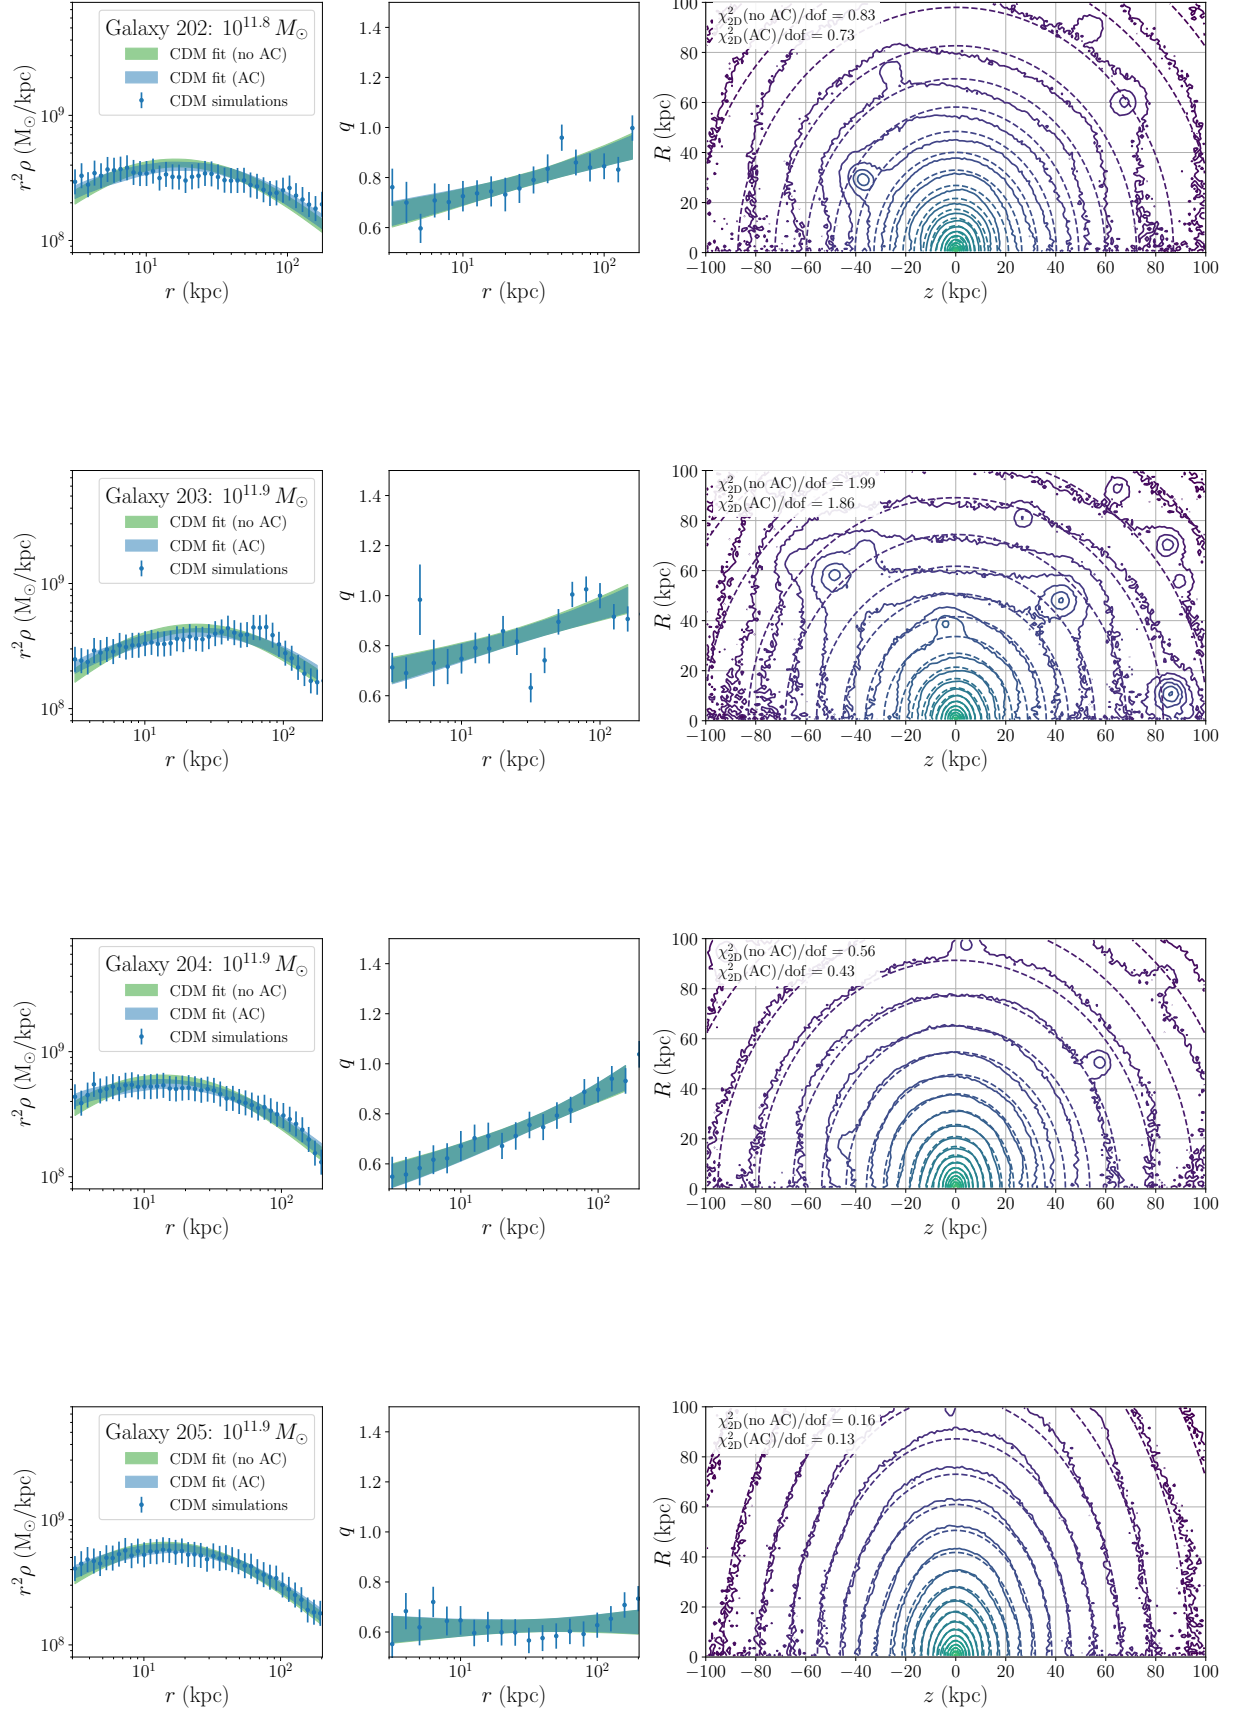

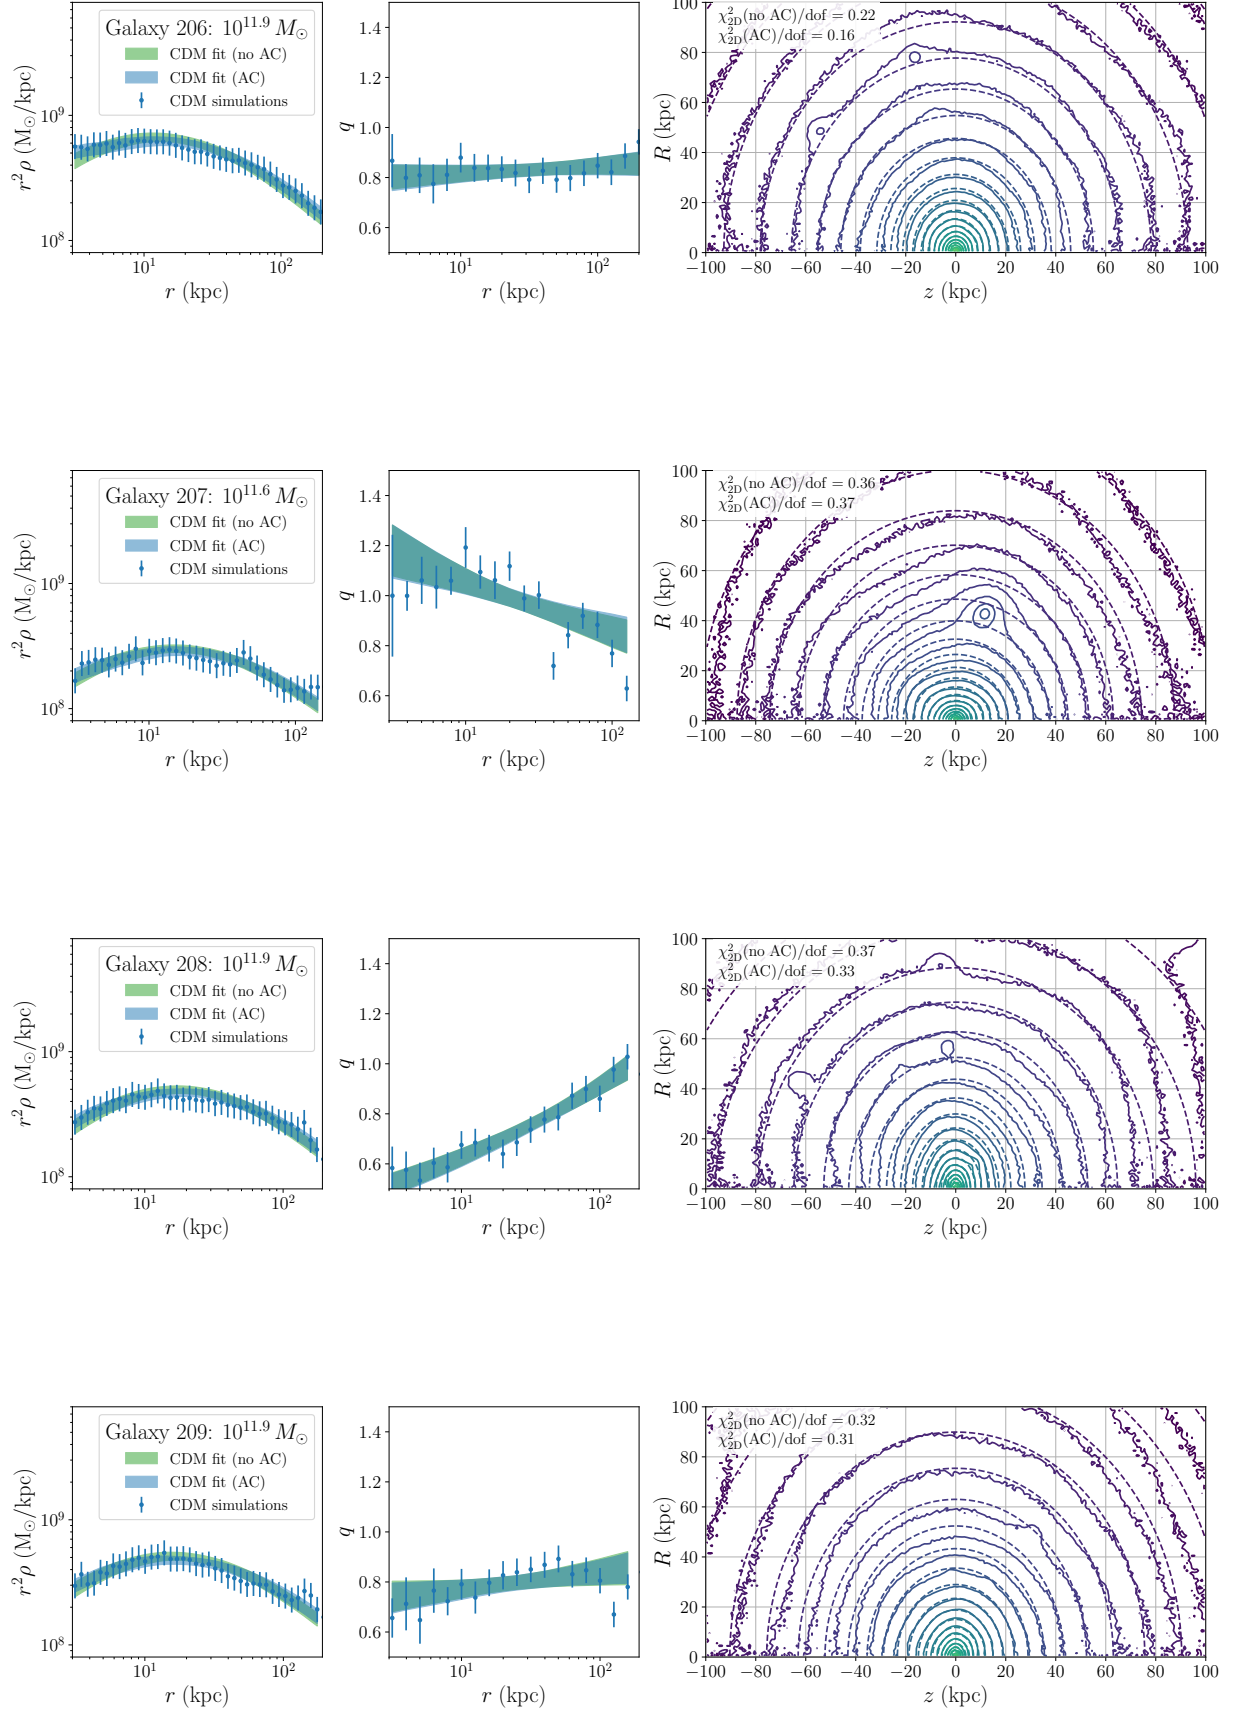

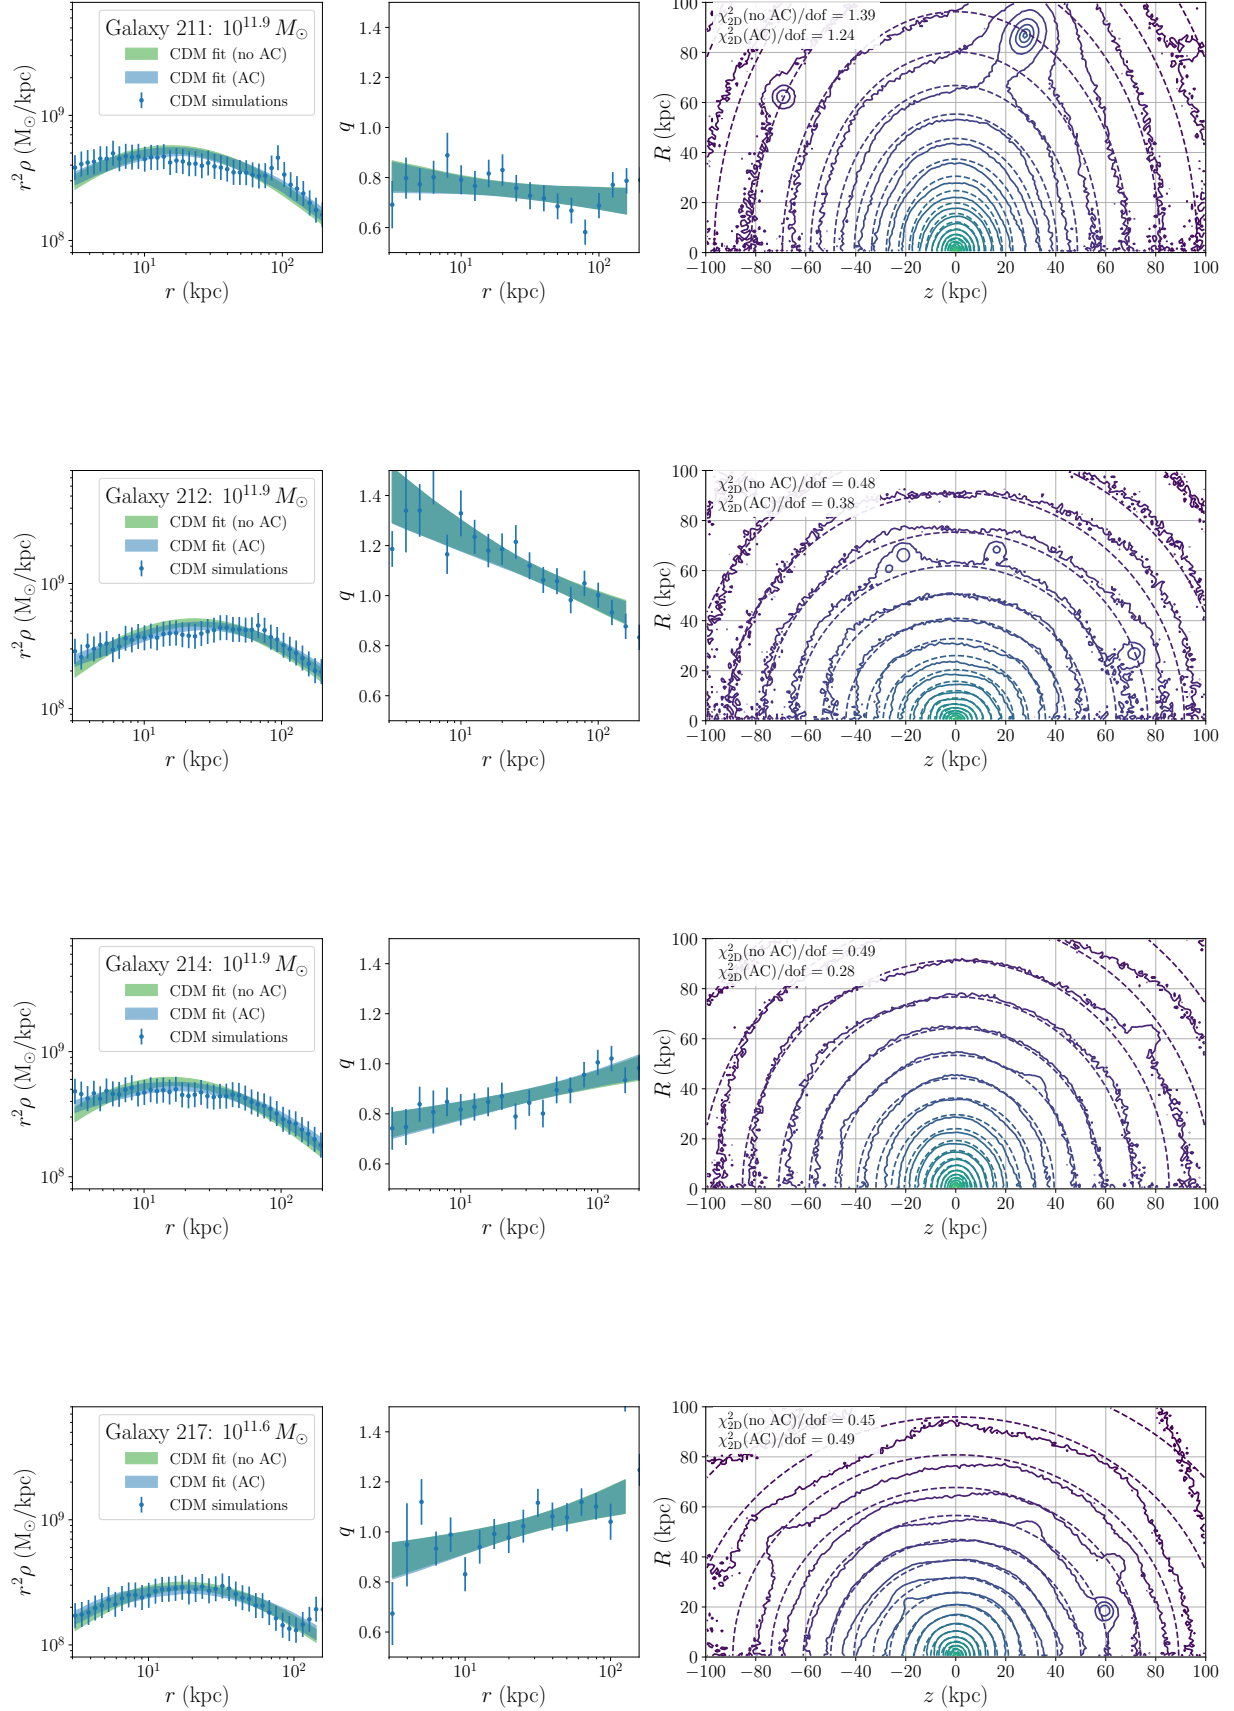

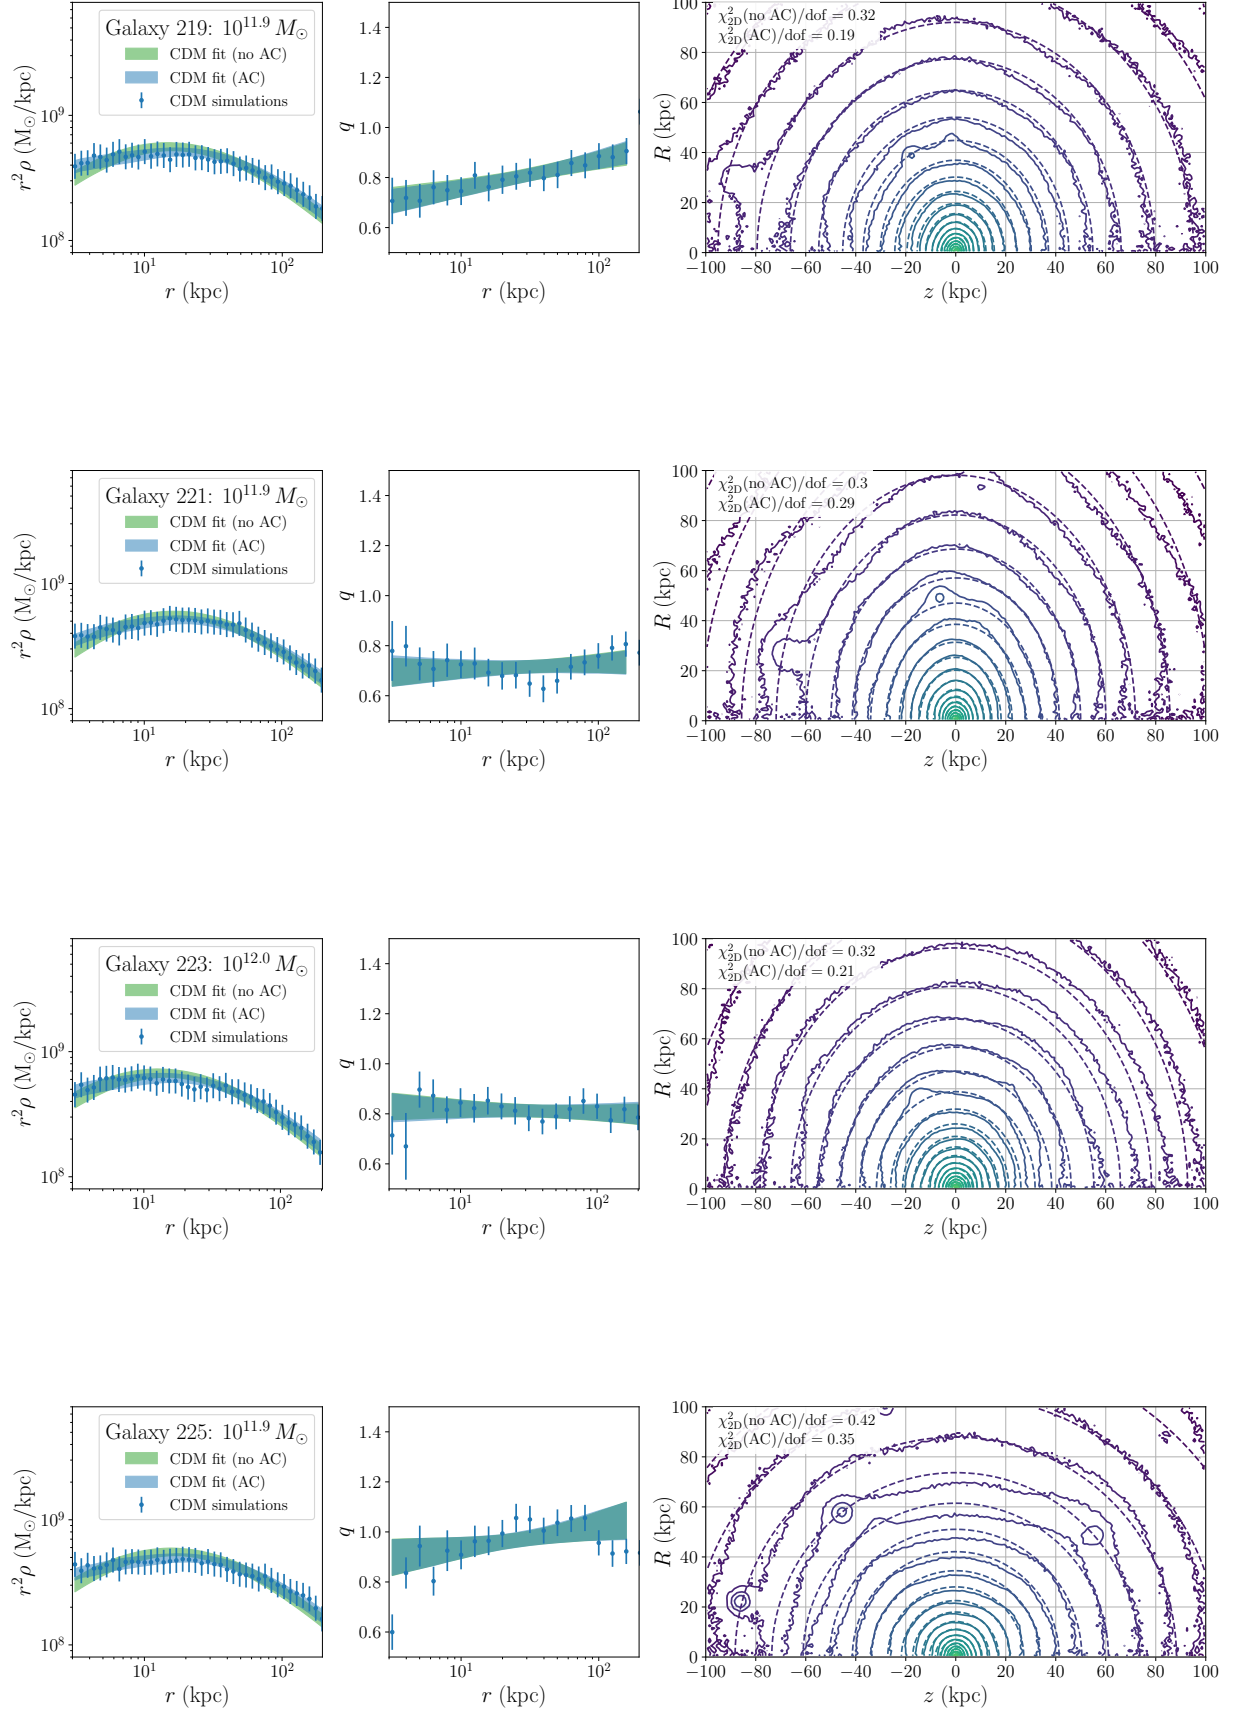

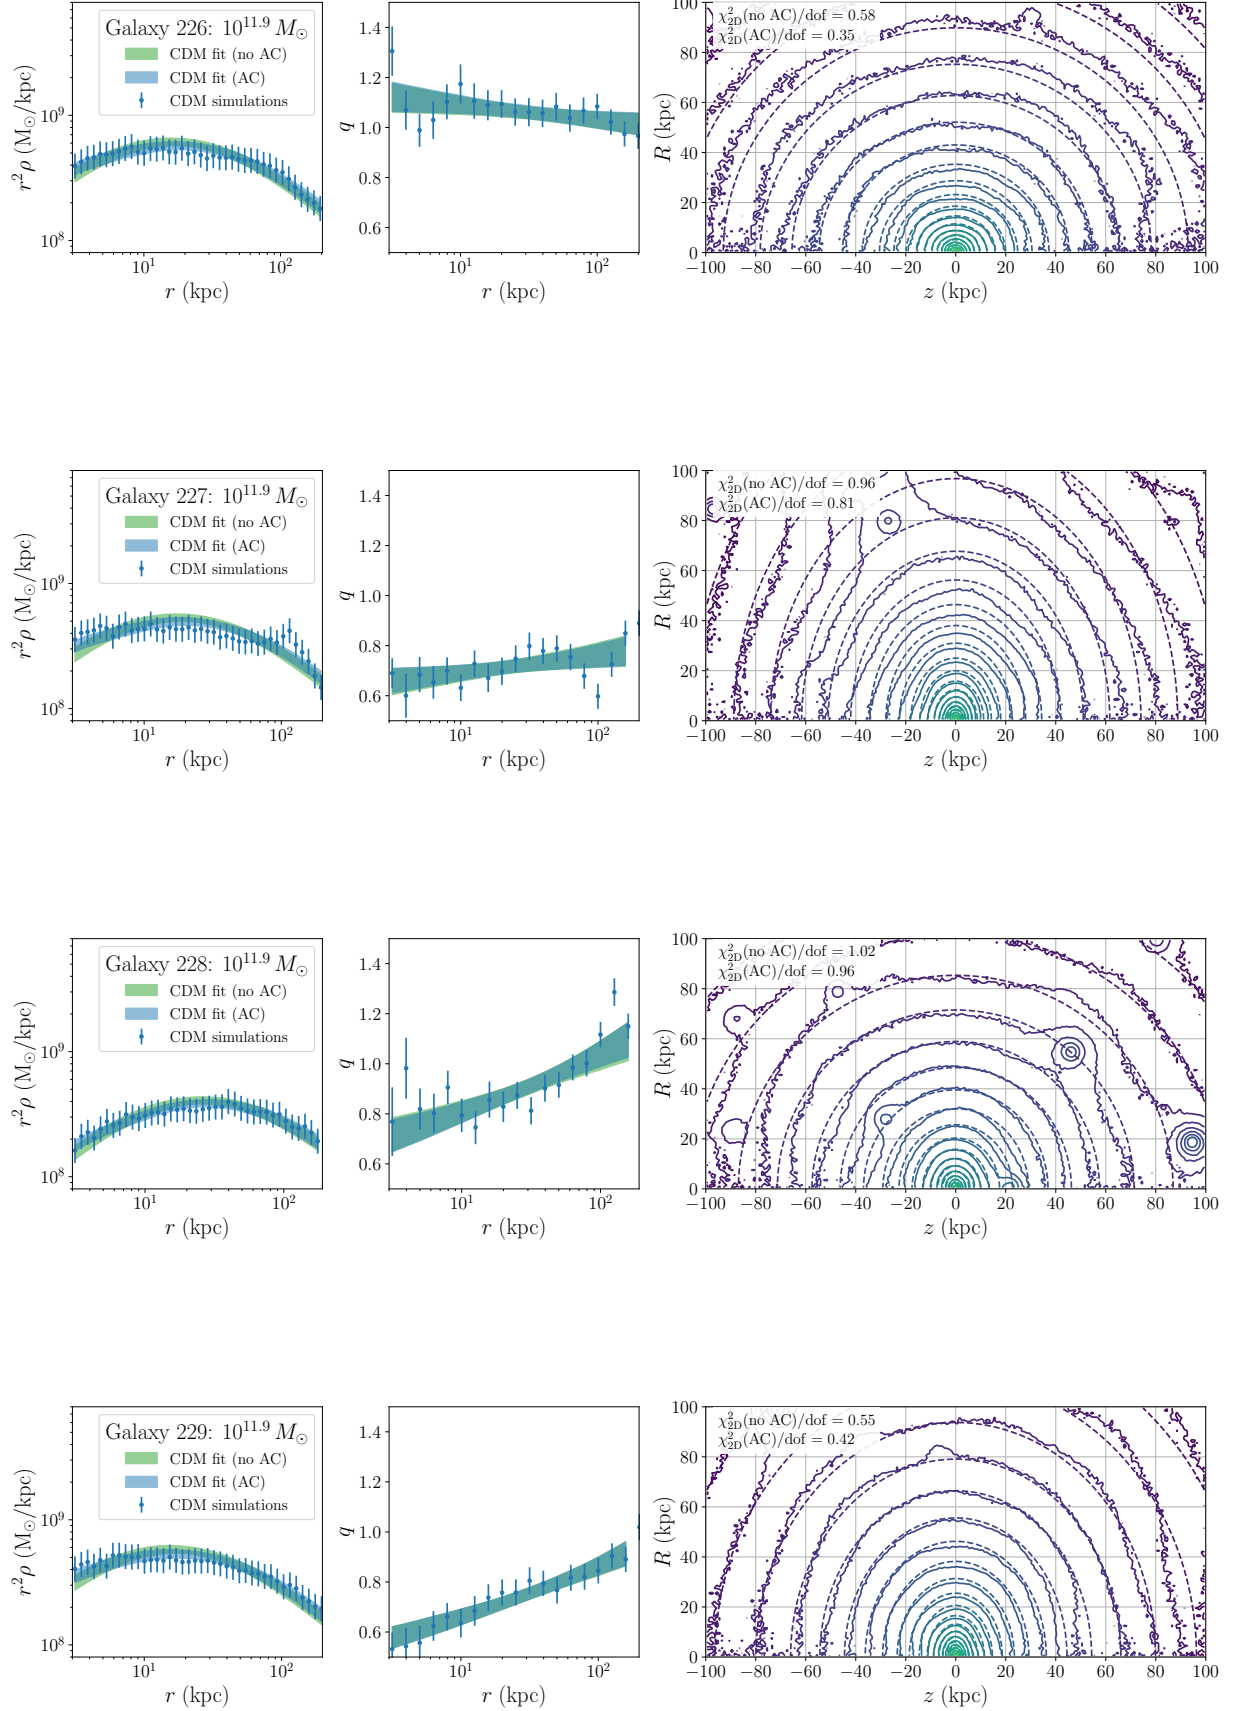



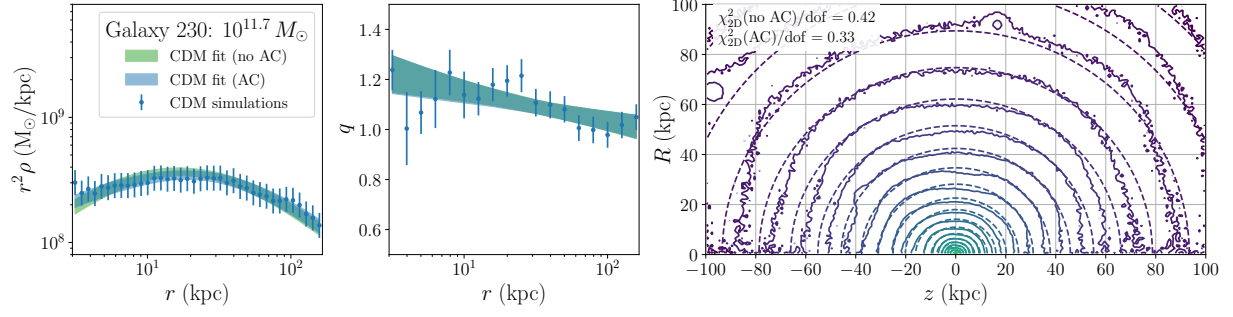

- 
- [1] A. Robertson et al., Mon. Not. Roy. Astron. Soc. 501 (2021) 4610, 2009.07844.
