# Supplementary material for: Jeans Model for the Shapes of Self-interacting Dark Matter Halos
Source: arXiv:2511.10765 ancillary file (2025-11-13)
Supplement: Supplementary file 4 [file Ancillary4.pdf]

# **Ancillary material 4: Squashed Jeans model fits for CDM halos in the Eagle-50 simulations set. This material is associated to the submission, Jeans Model for the Shapes of Self-interacting Dark Matter Halo Shapes**

Yilber Fabian Bautista, Andrew Robertson, Laura Sagunski, Adam Smith-Orlik, and Sean Tulin

Comparison of CDM halos from the EAGLE-50 simulations set presented in Ref. [1] to squashed and spherical Jeans fits. Panels (left-to-right) show (a) spherically-averaged density and (b) halo shape profiles, where blue (green) bands denote 80% confidence region from our nonspherical (spherical) fits; (c) azimuthally-averaged 2D iso-density contours for CDM simulations (solid) and our best-fit squashed Jeans model profile (dashed), and (d) blue (green) posterior distribution for  $\sigma/m$  (in  $\text{cm}^2/\text{g}$ ) for squashed (spherical) model. Further details are provided in Section V-A-2 of the main text.

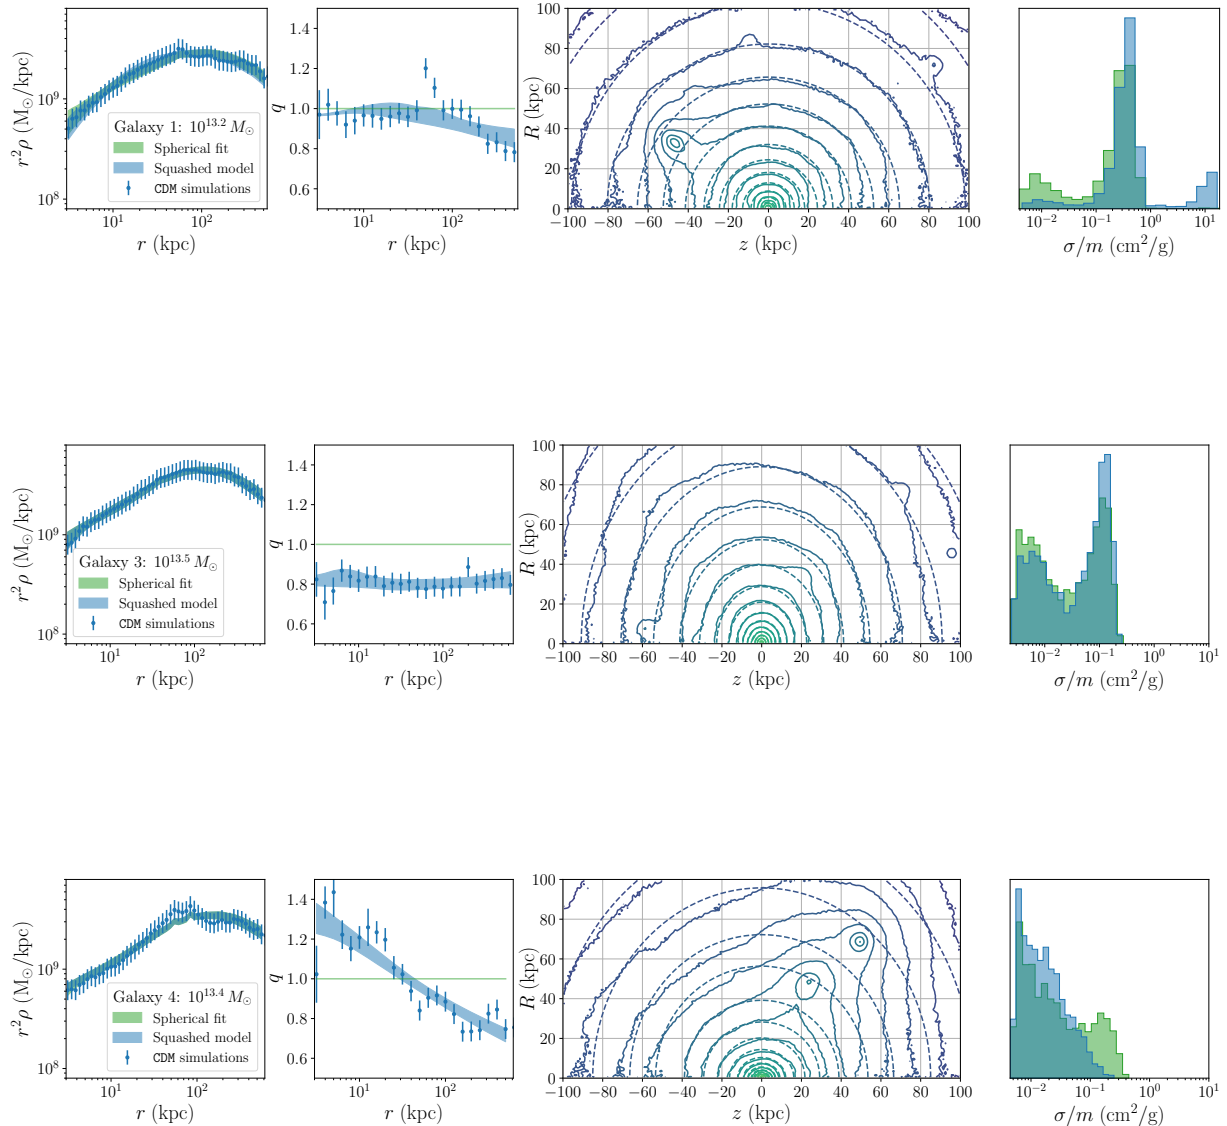

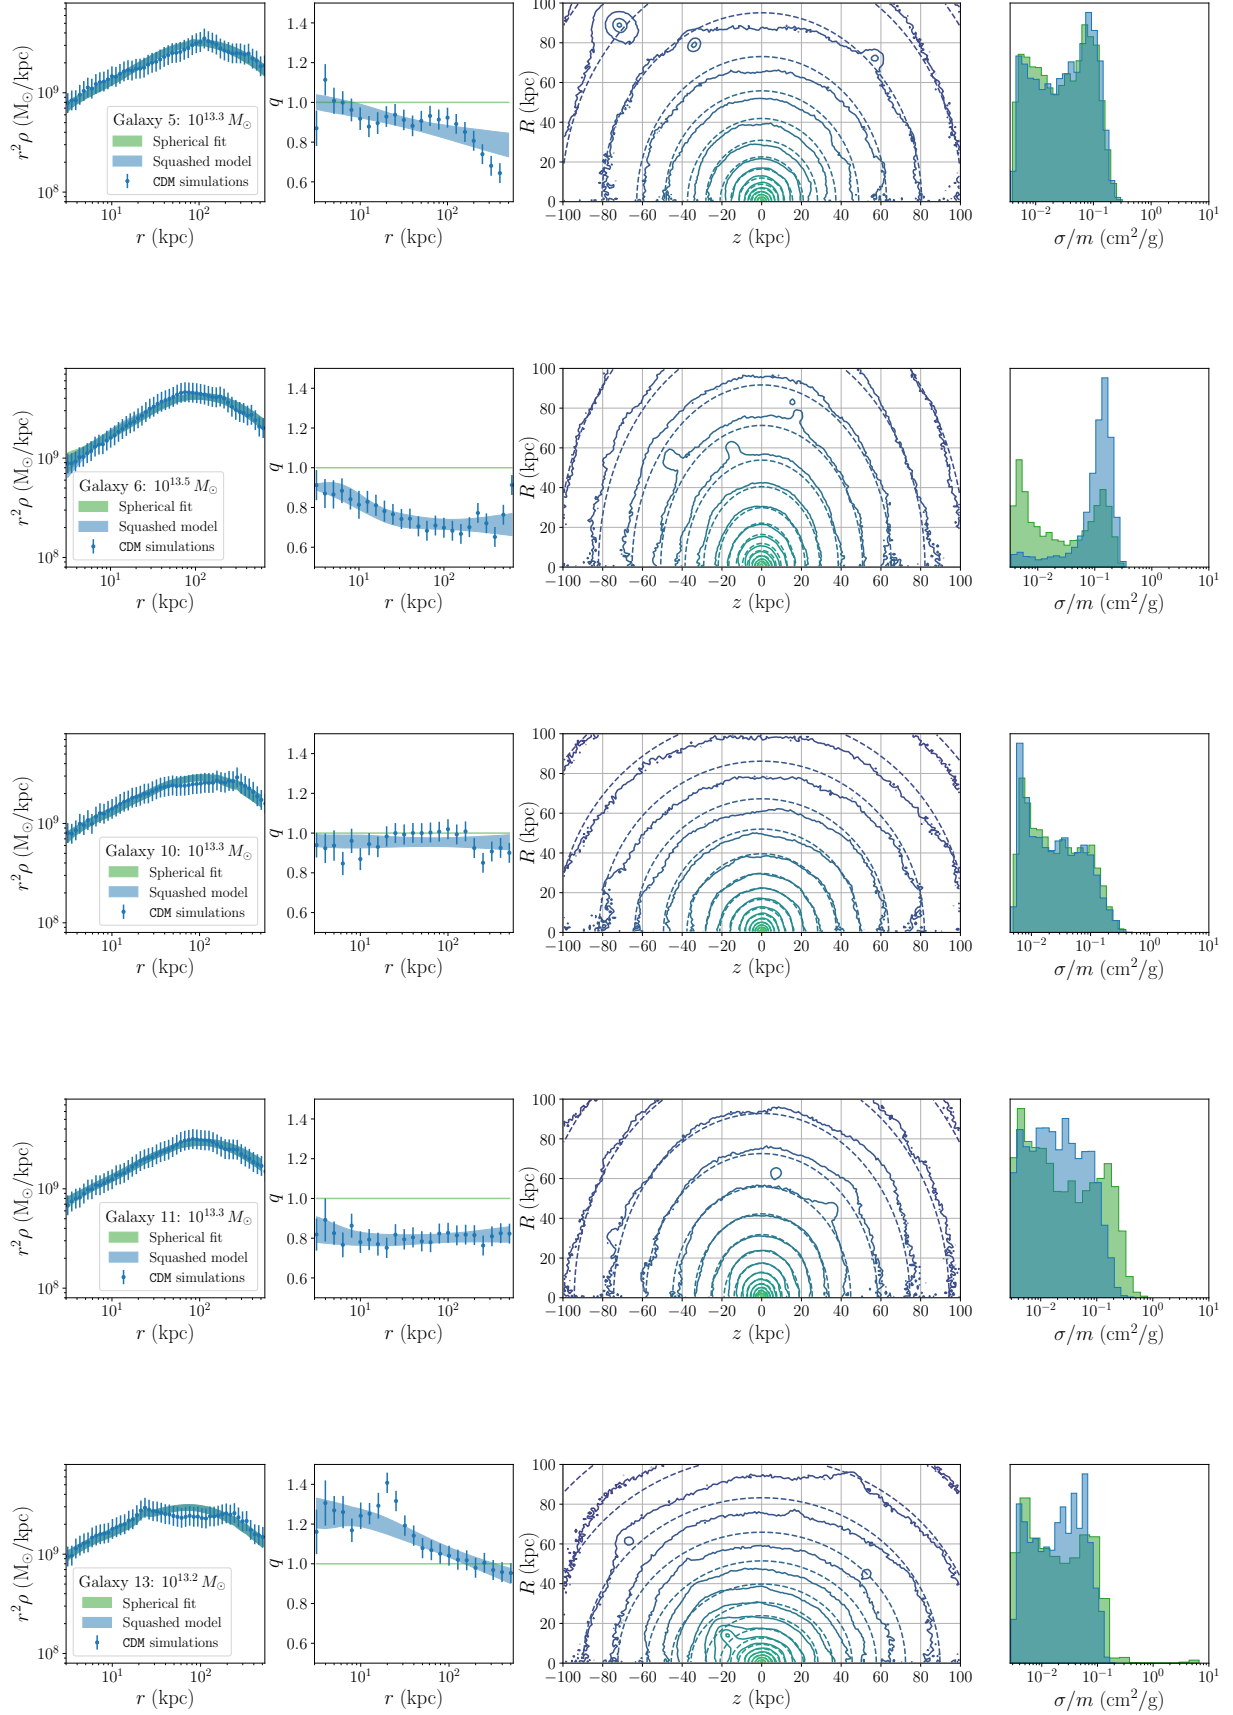

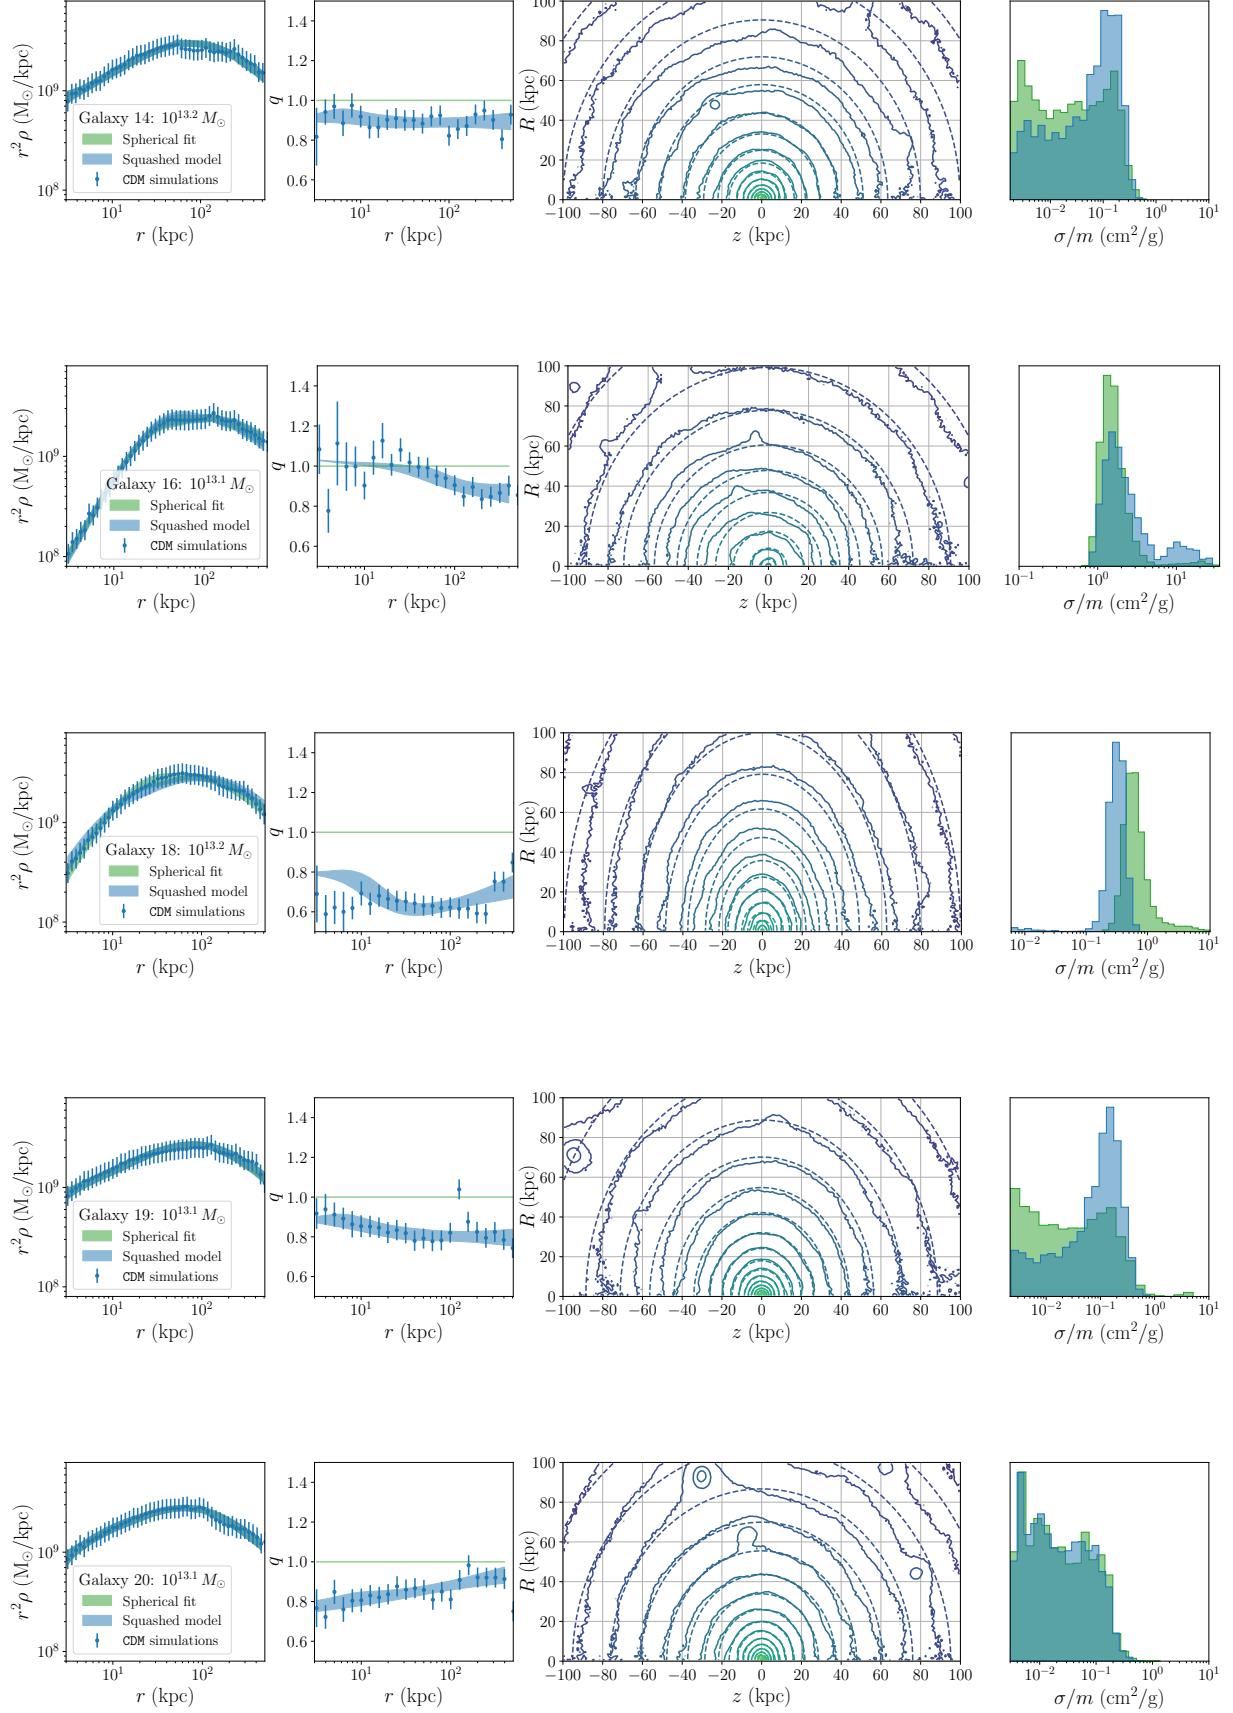

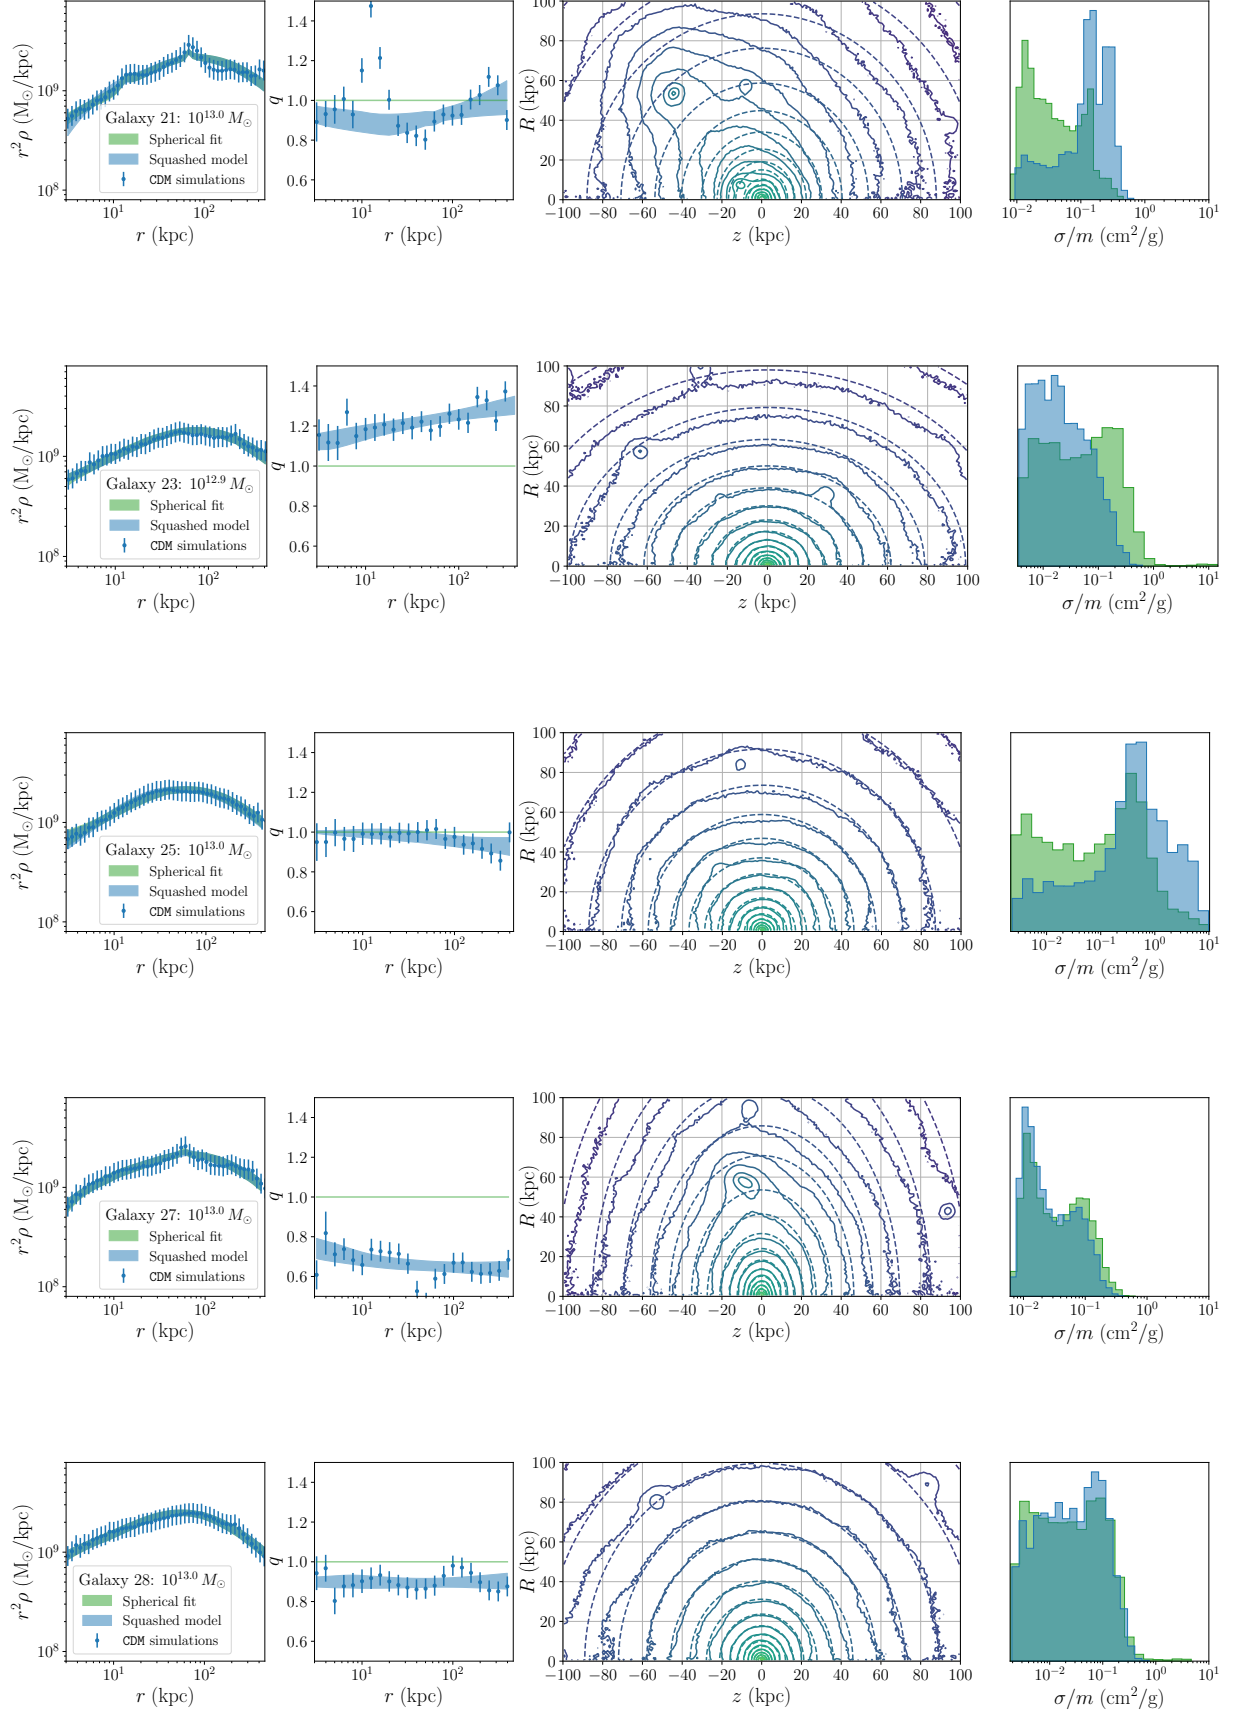



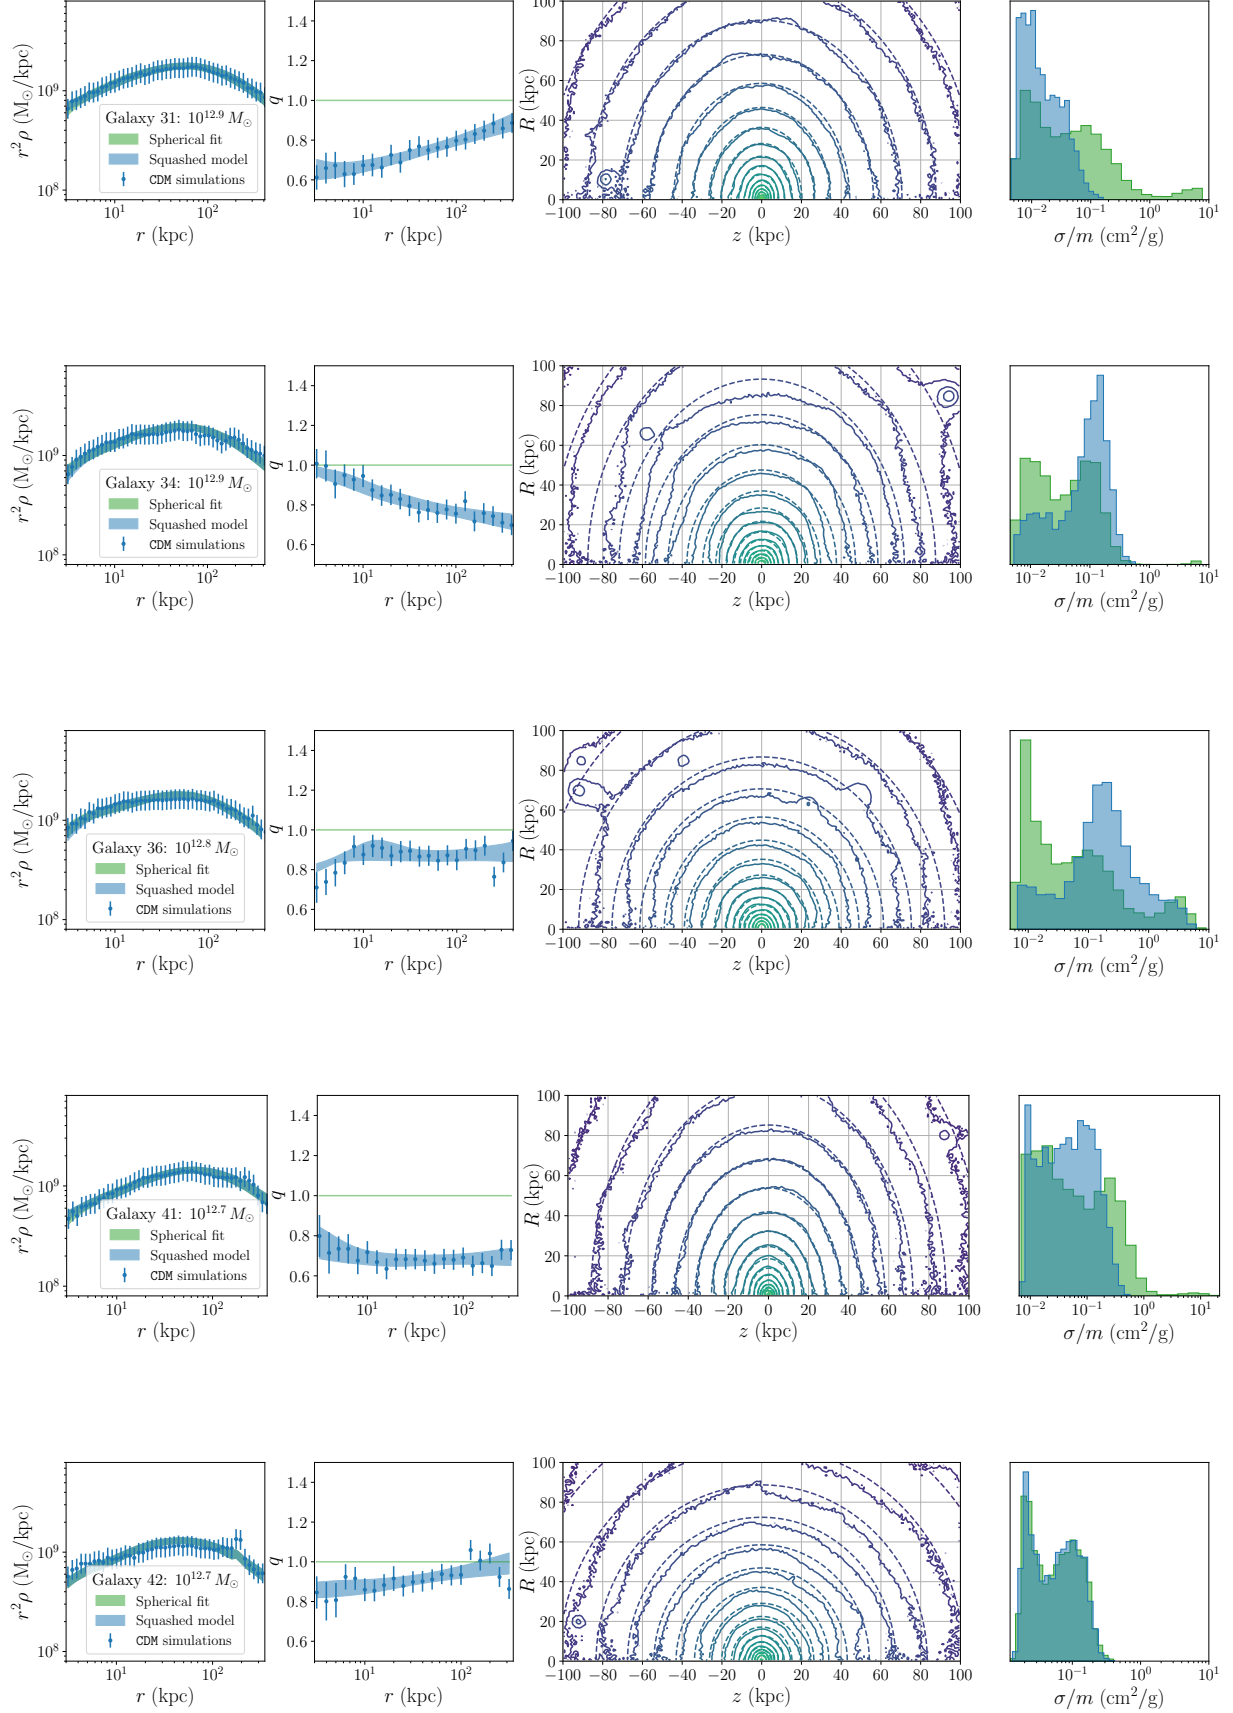

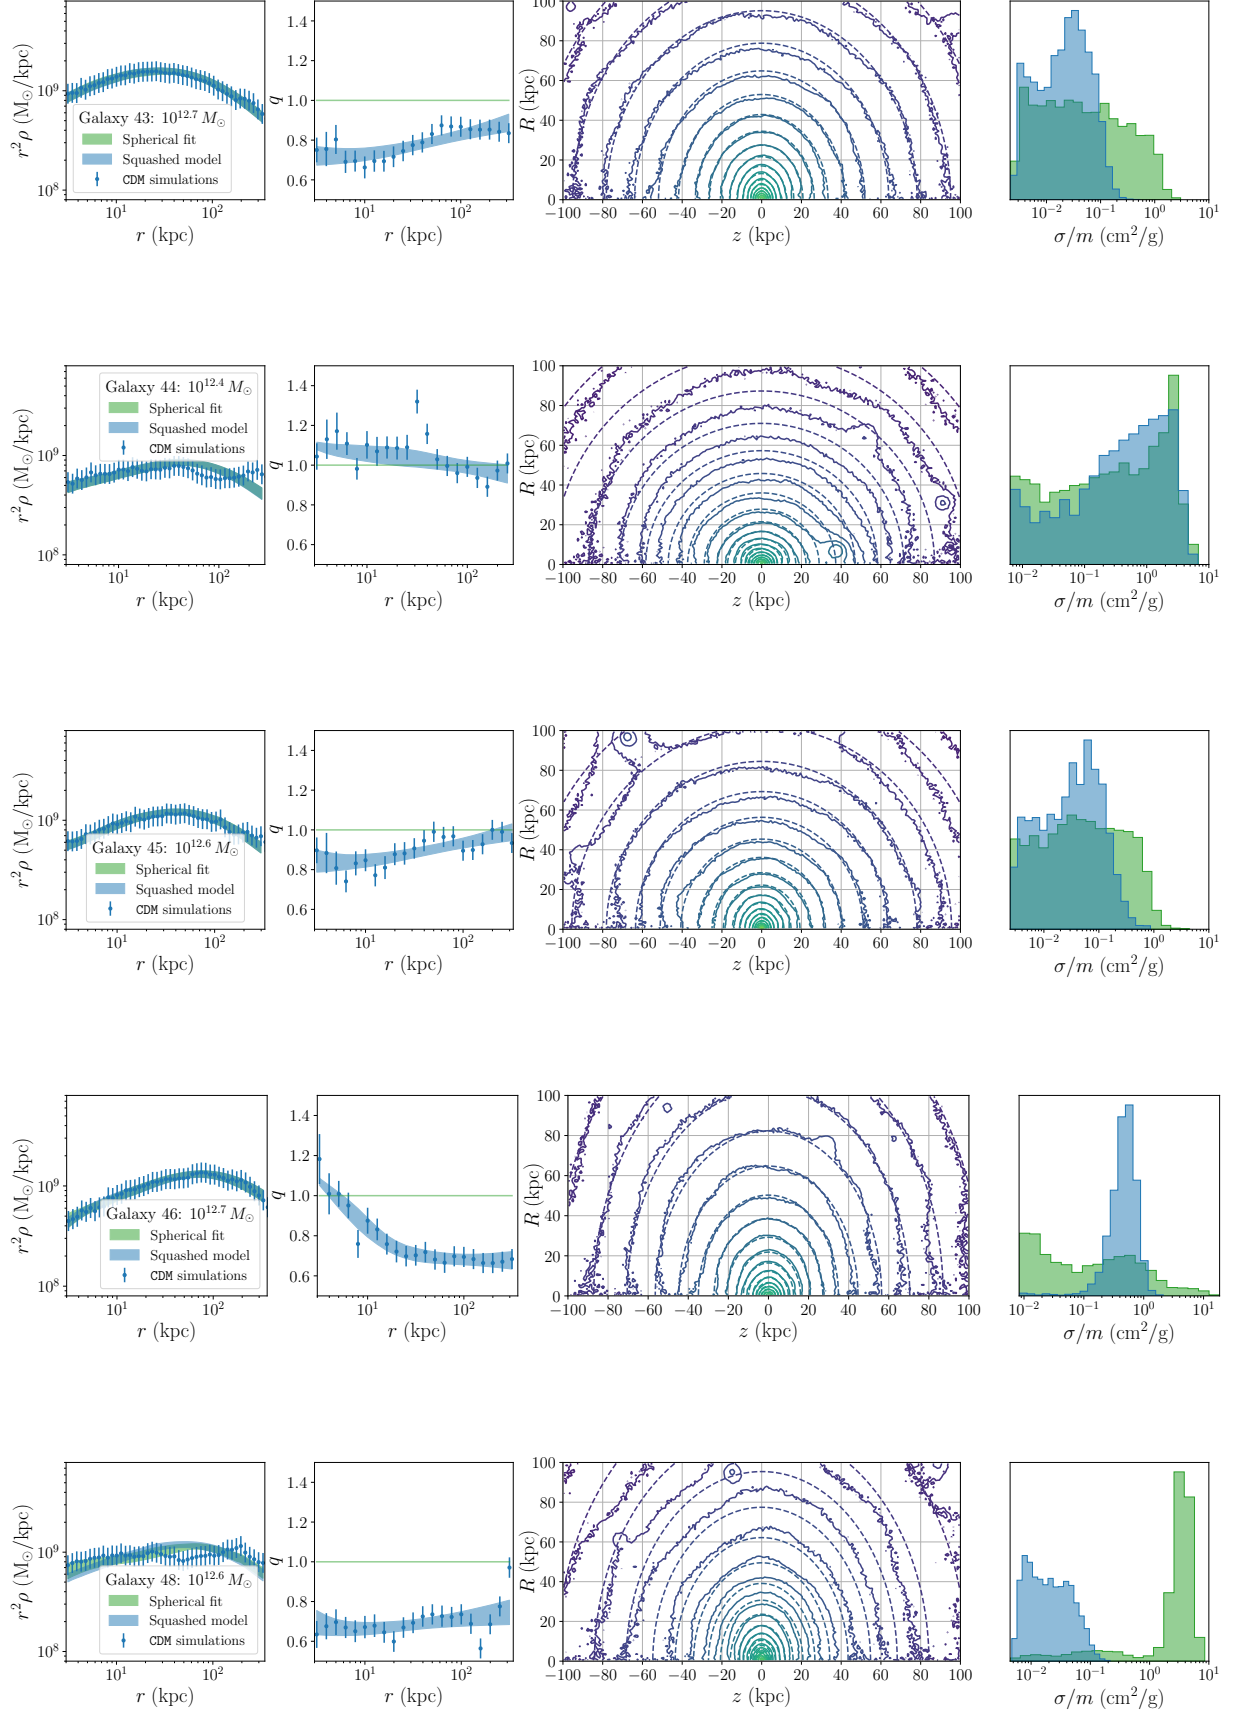

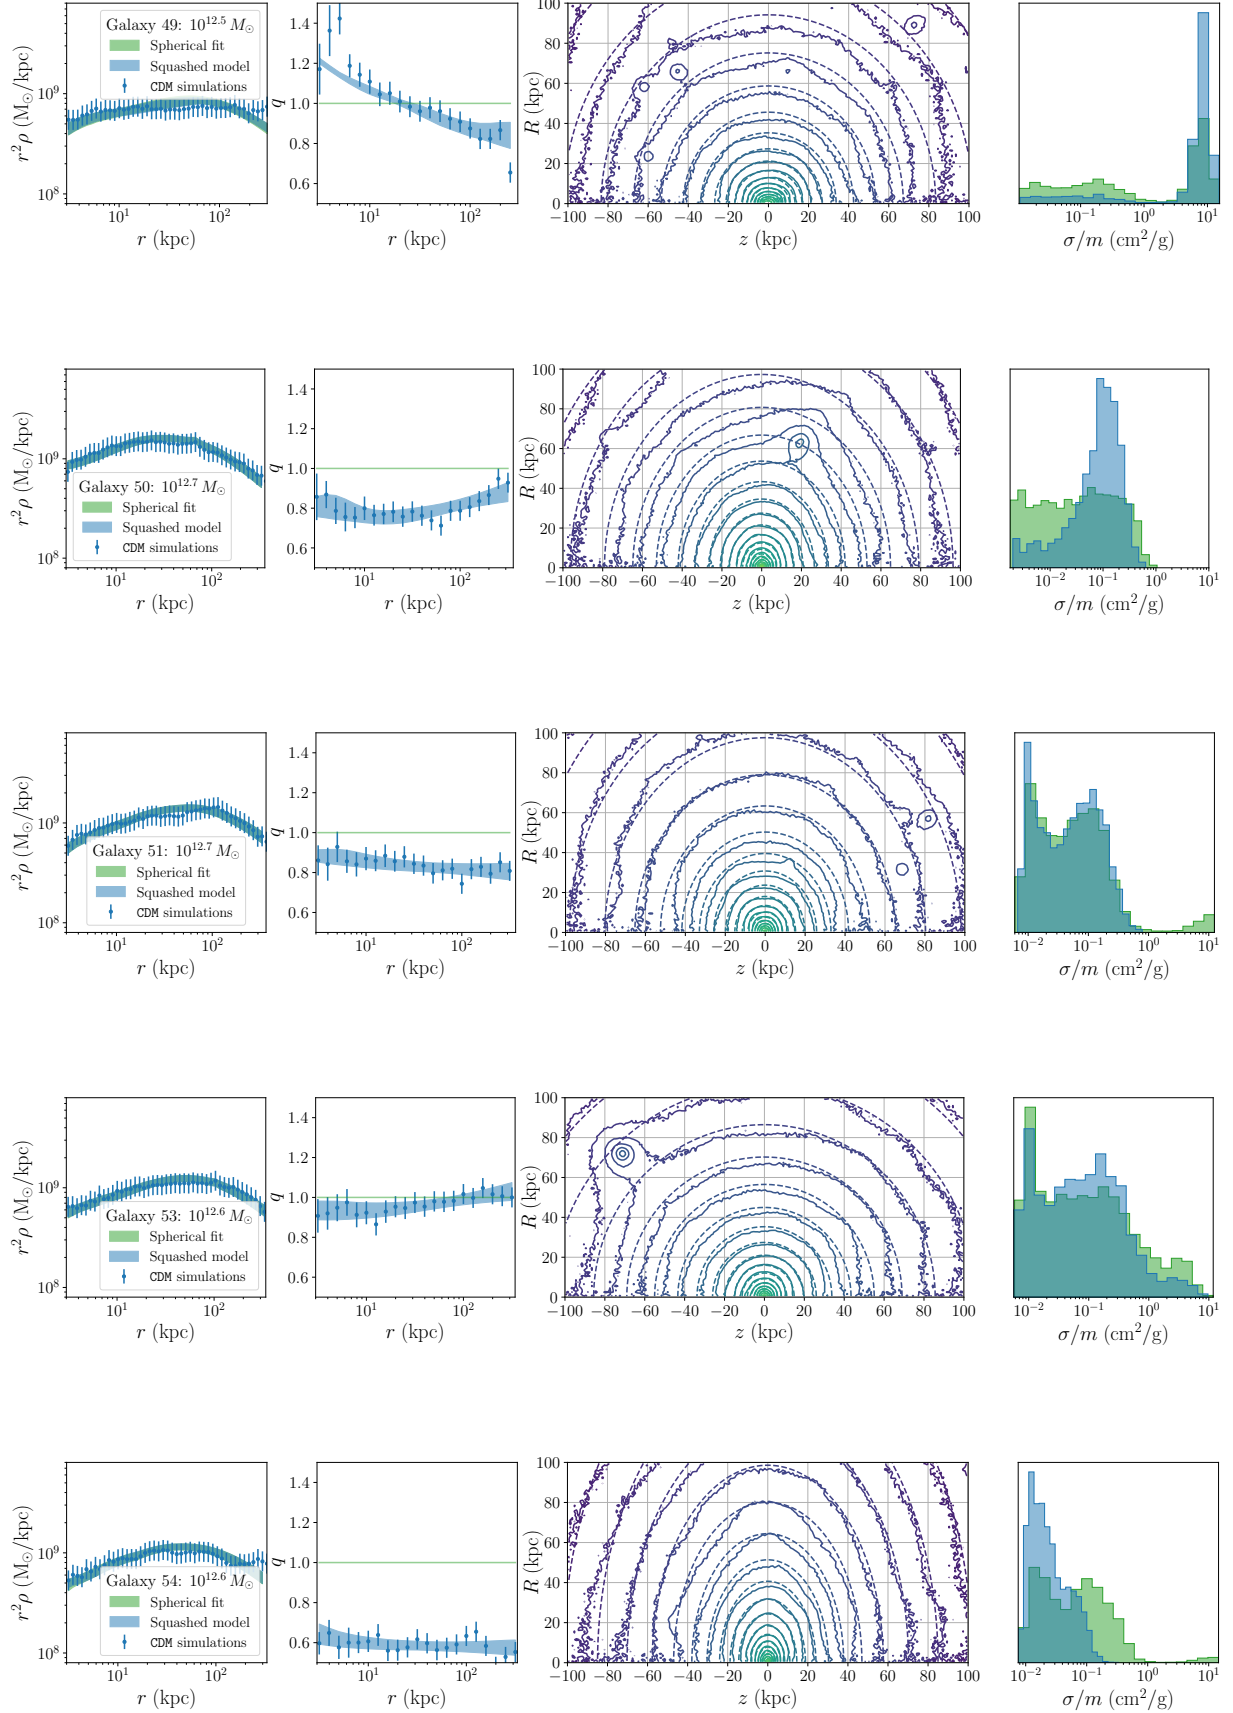

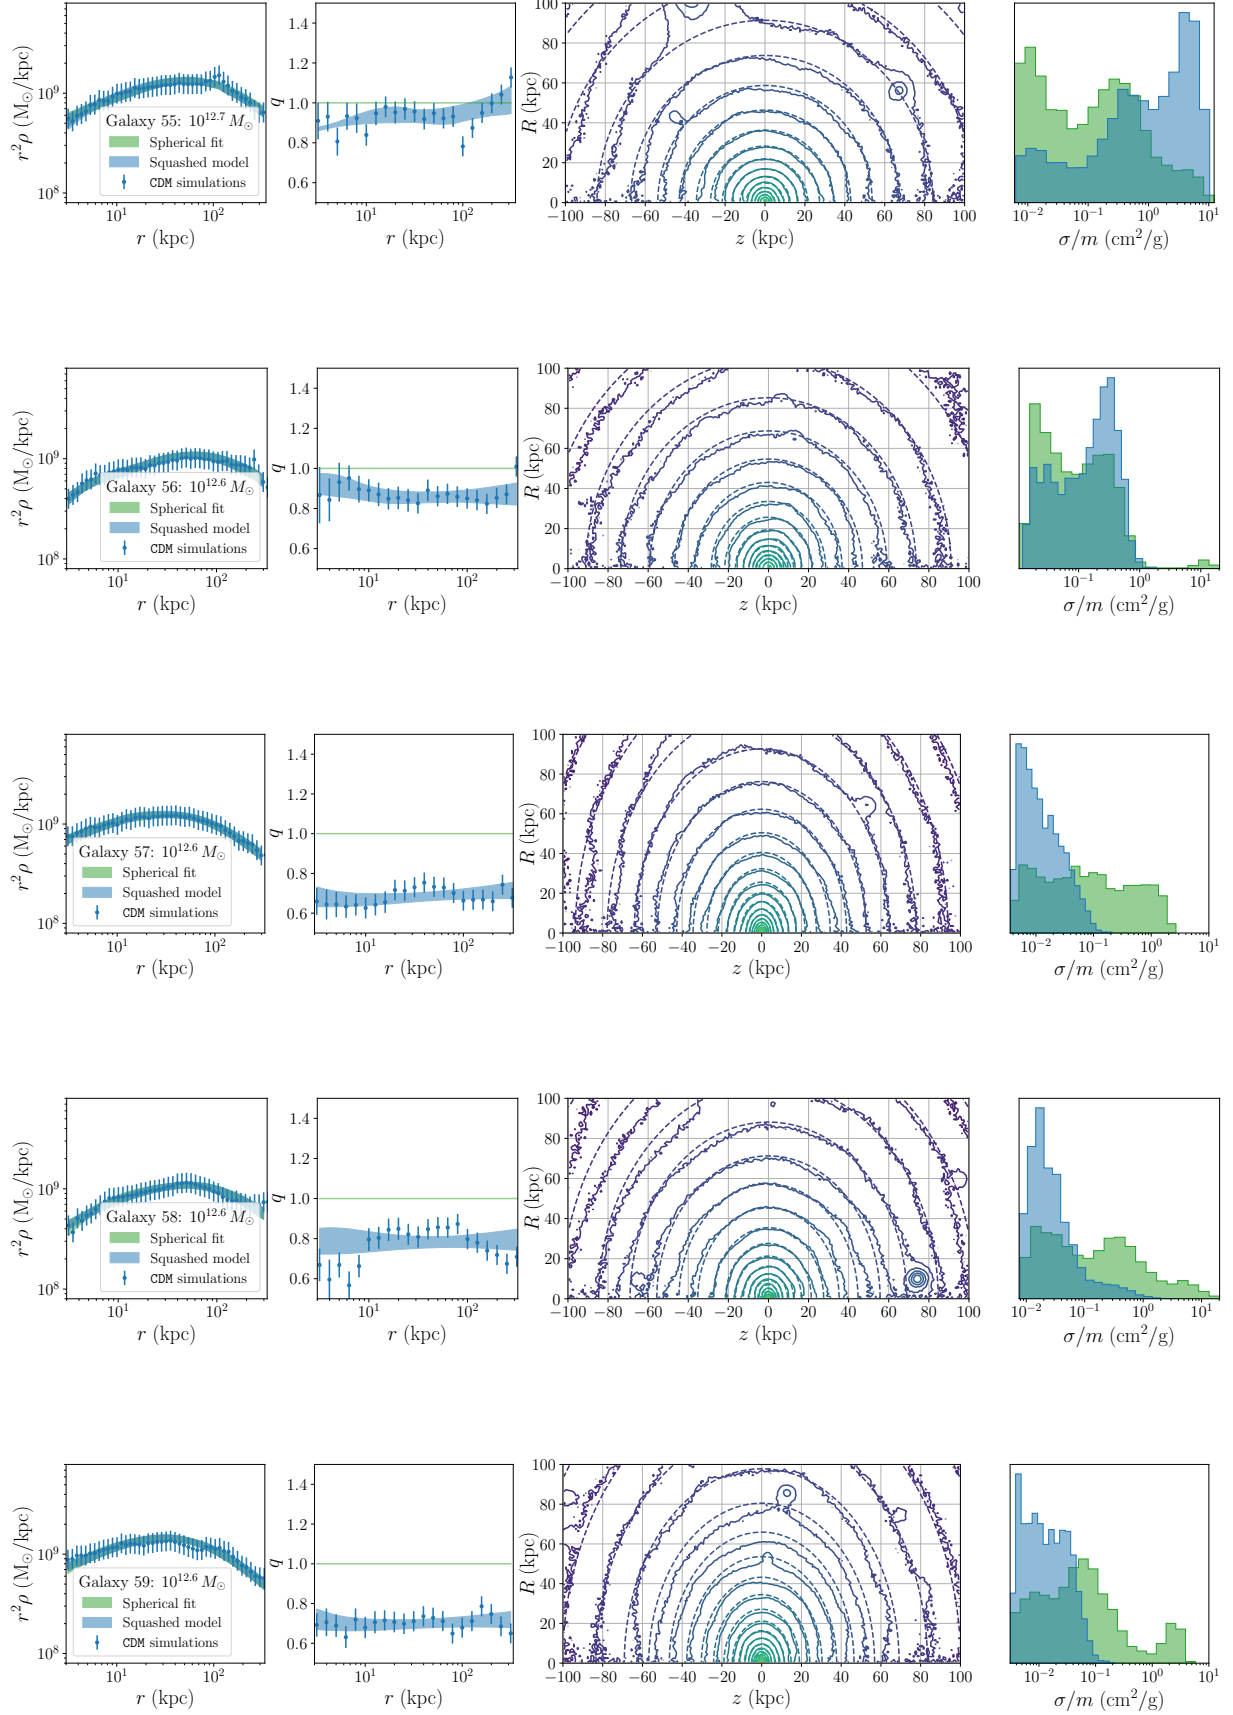

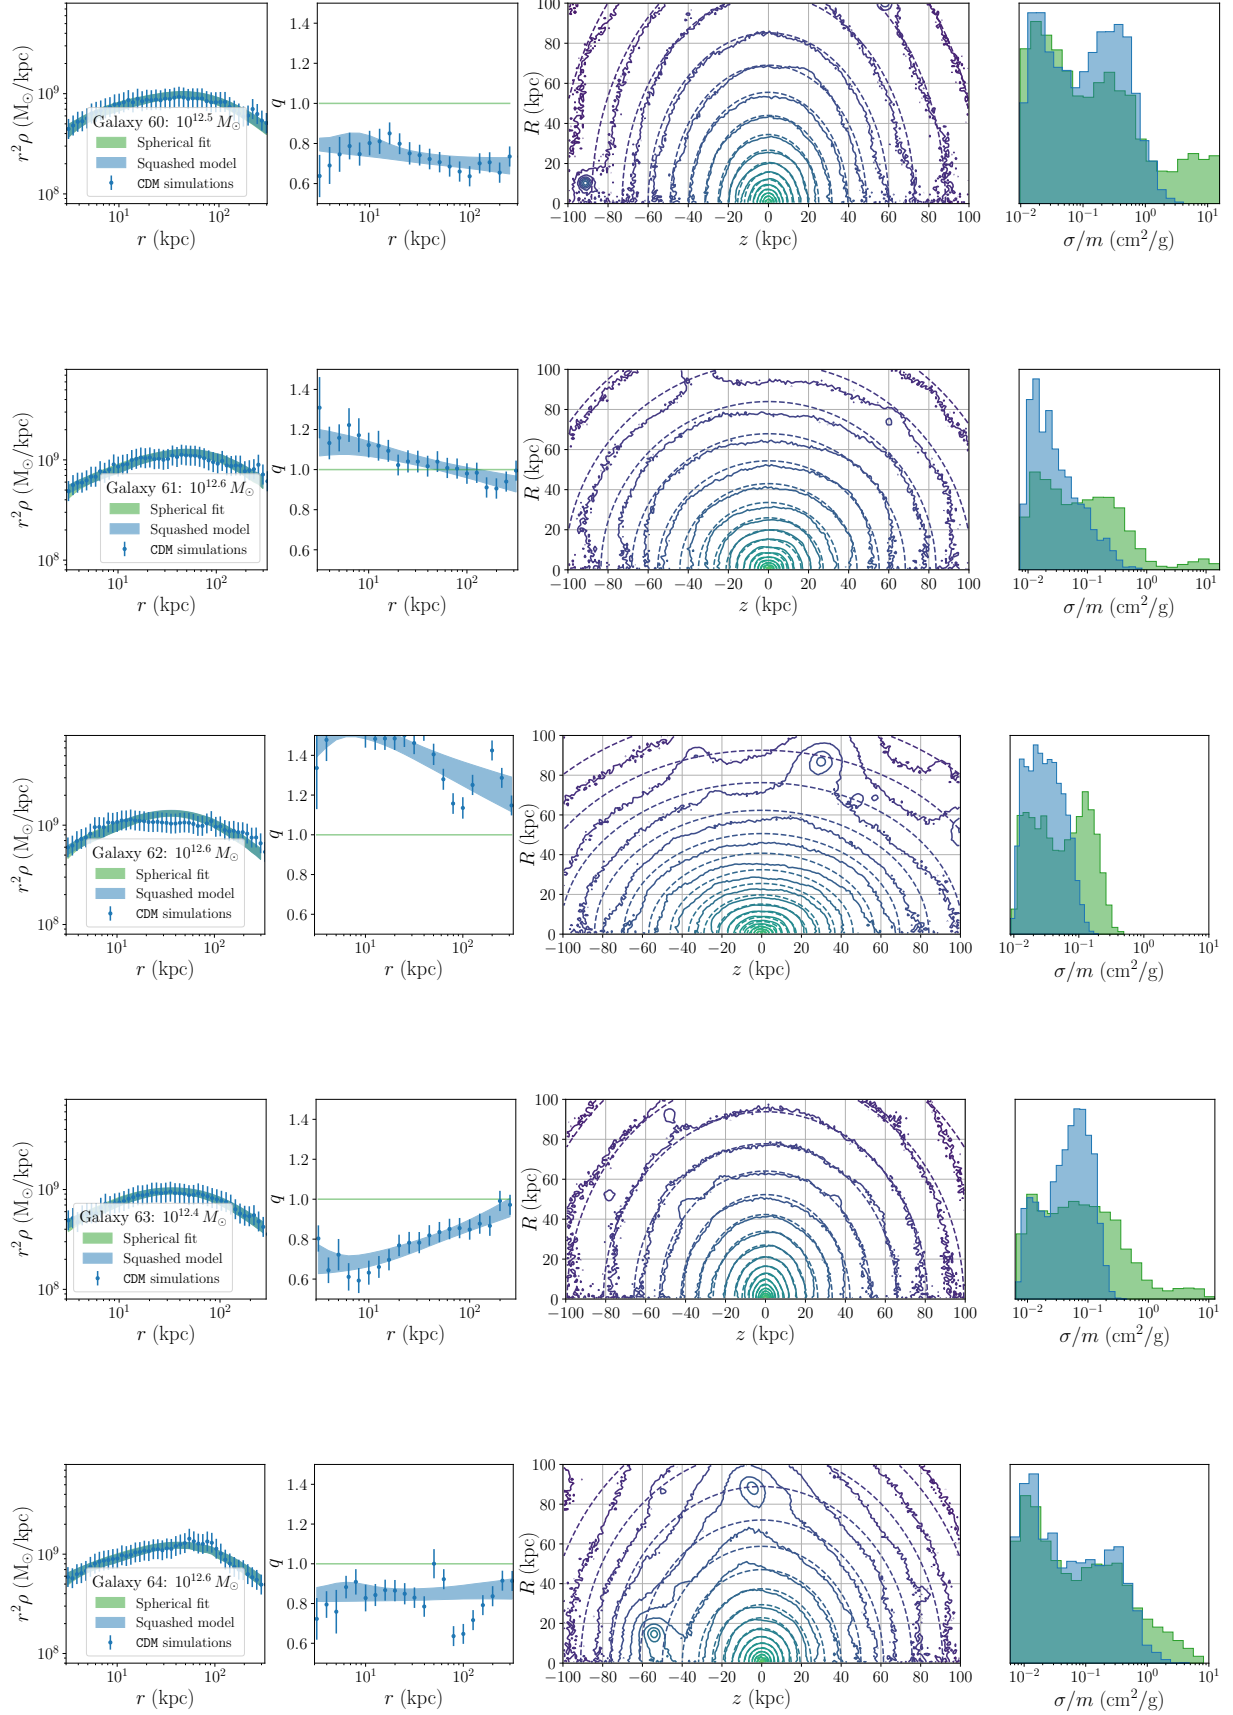

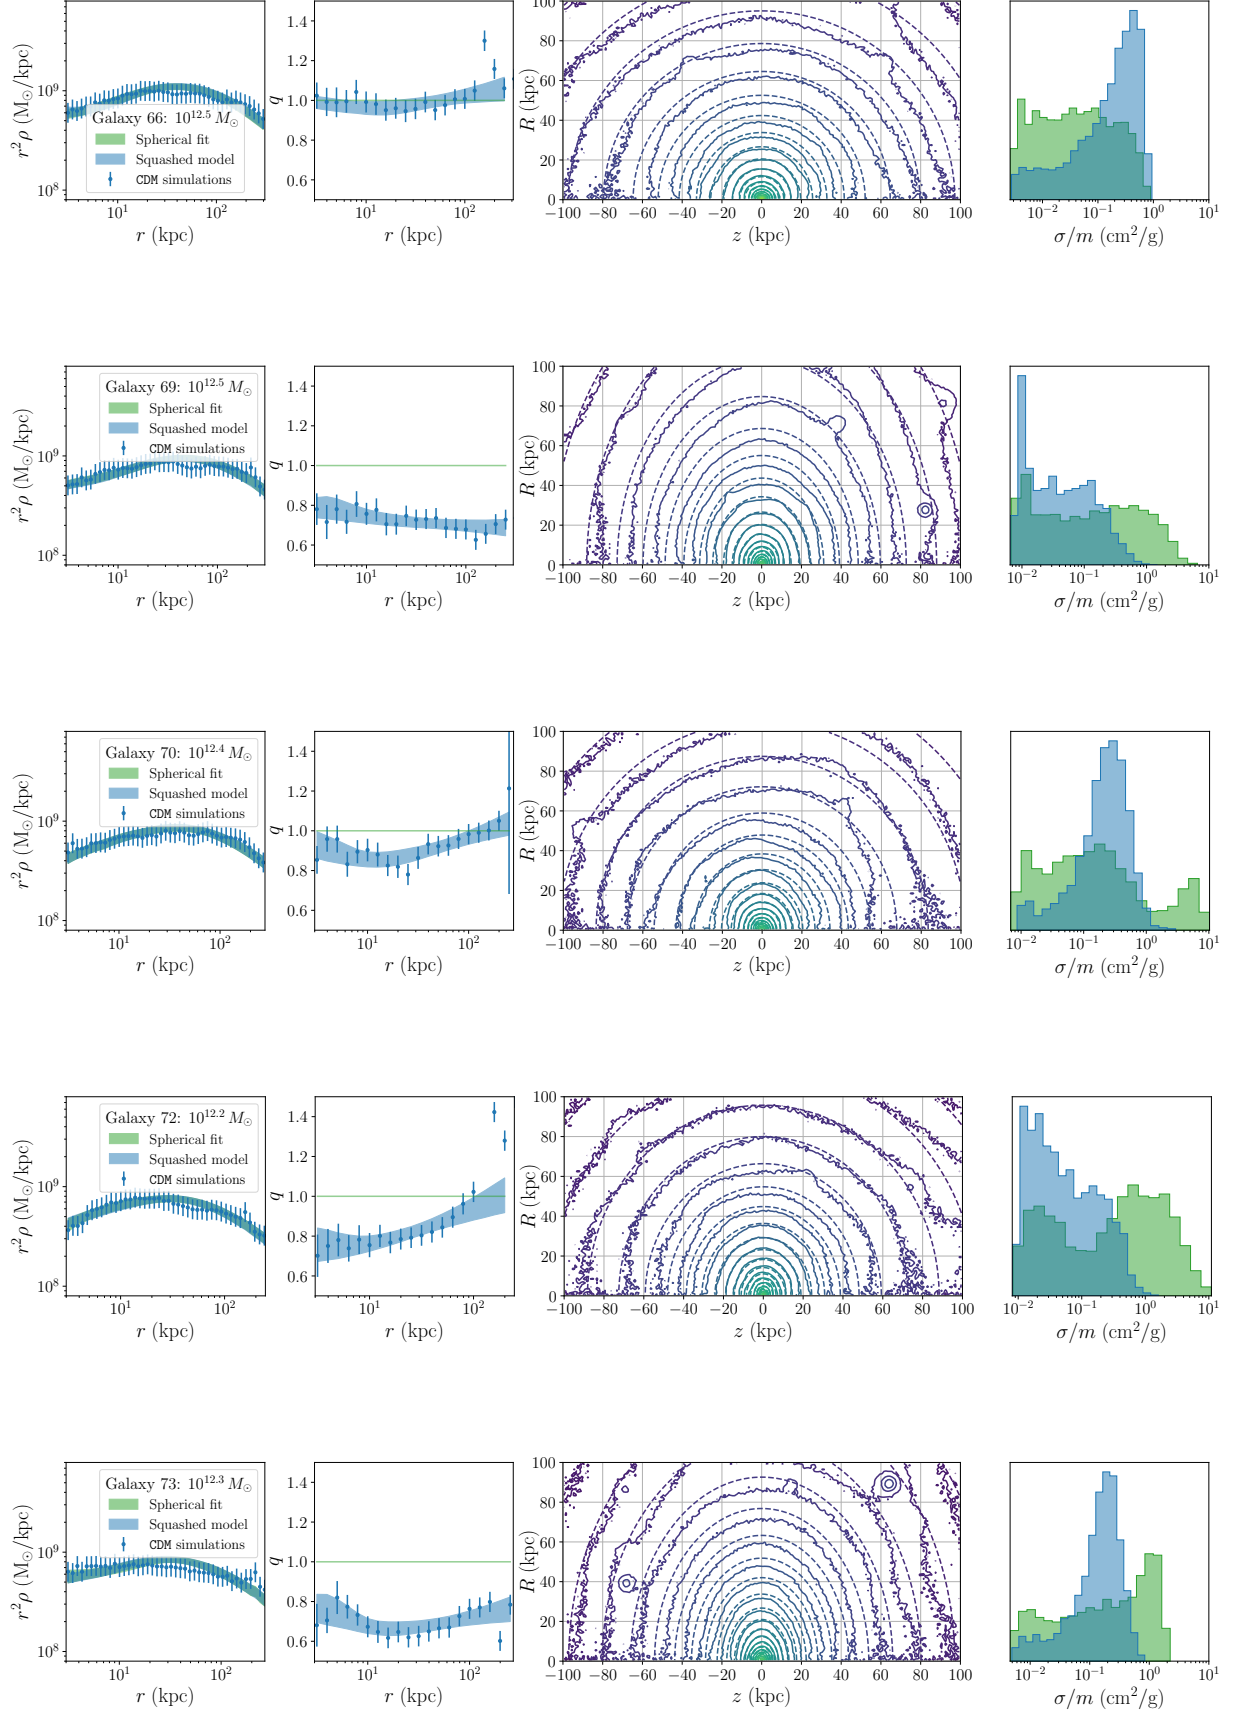



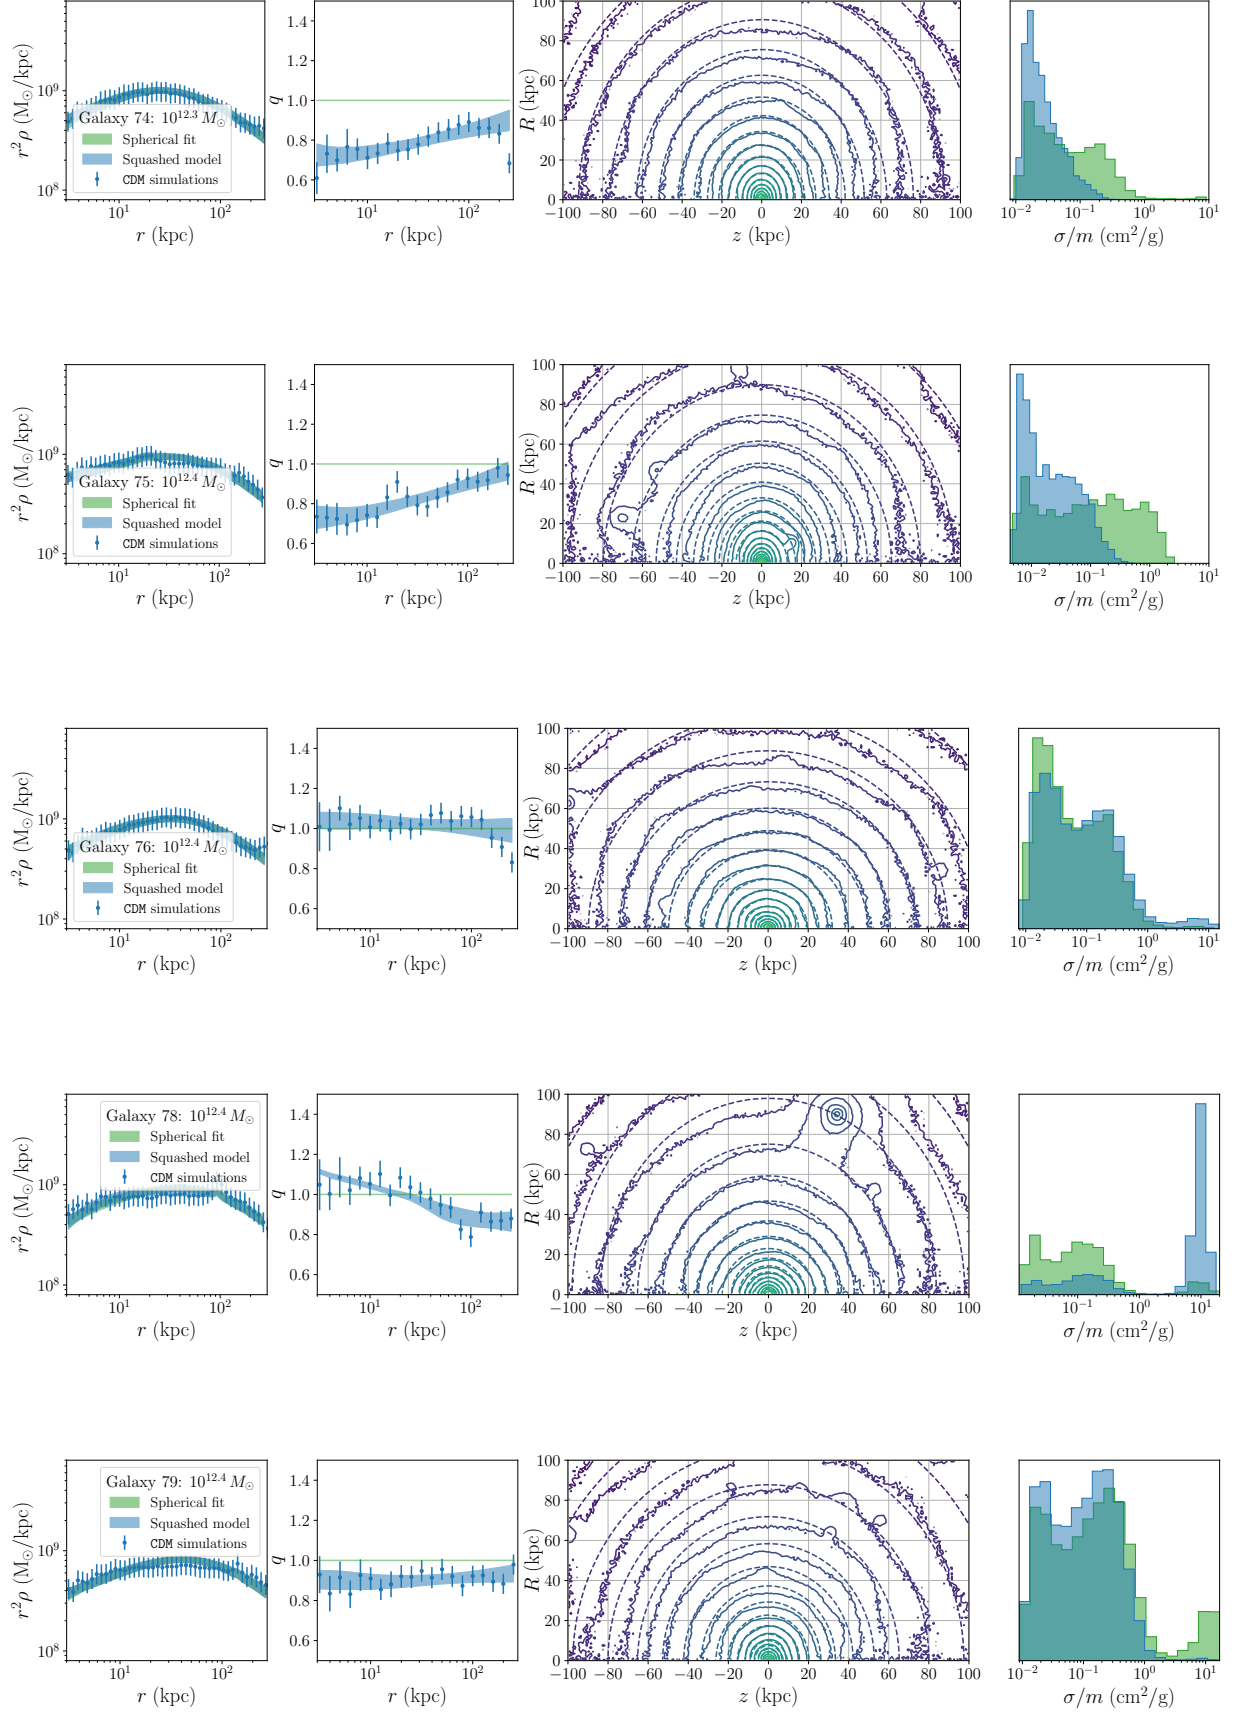



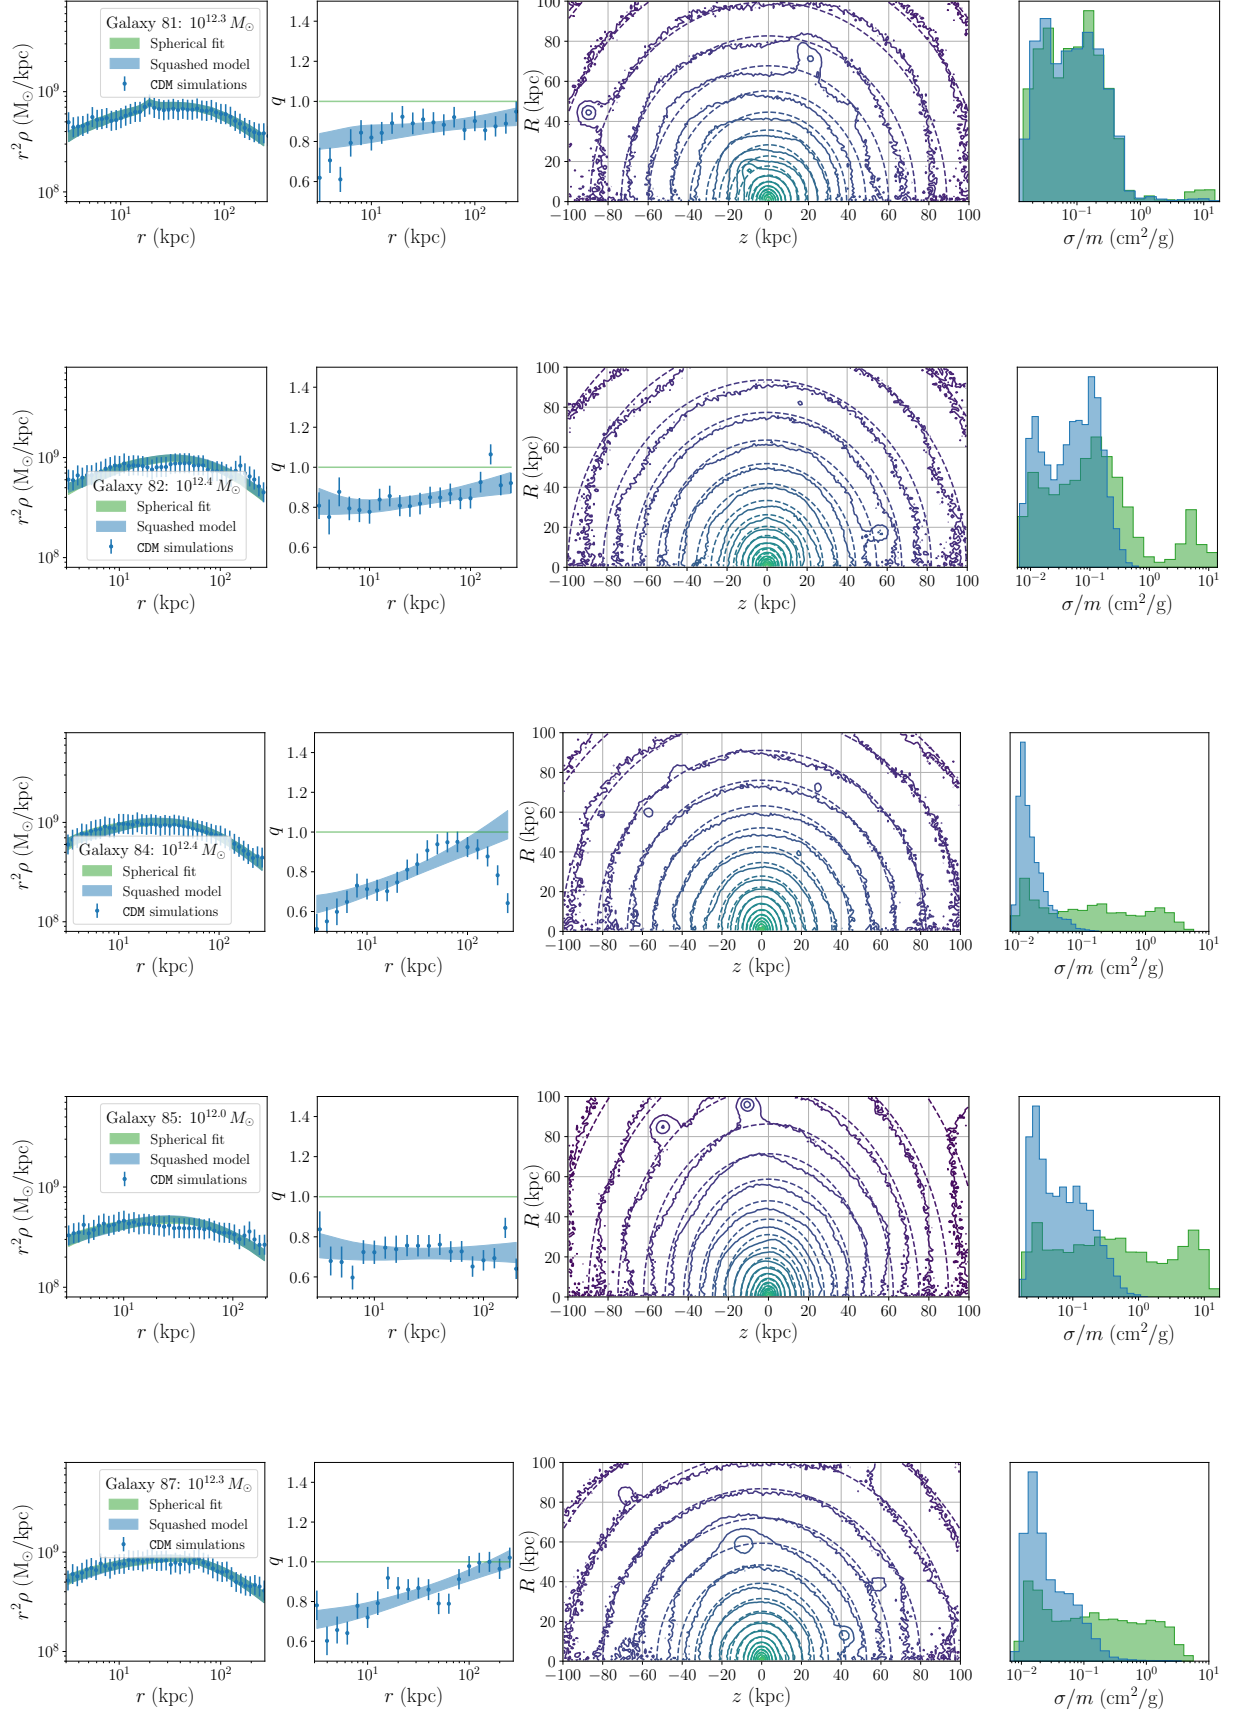

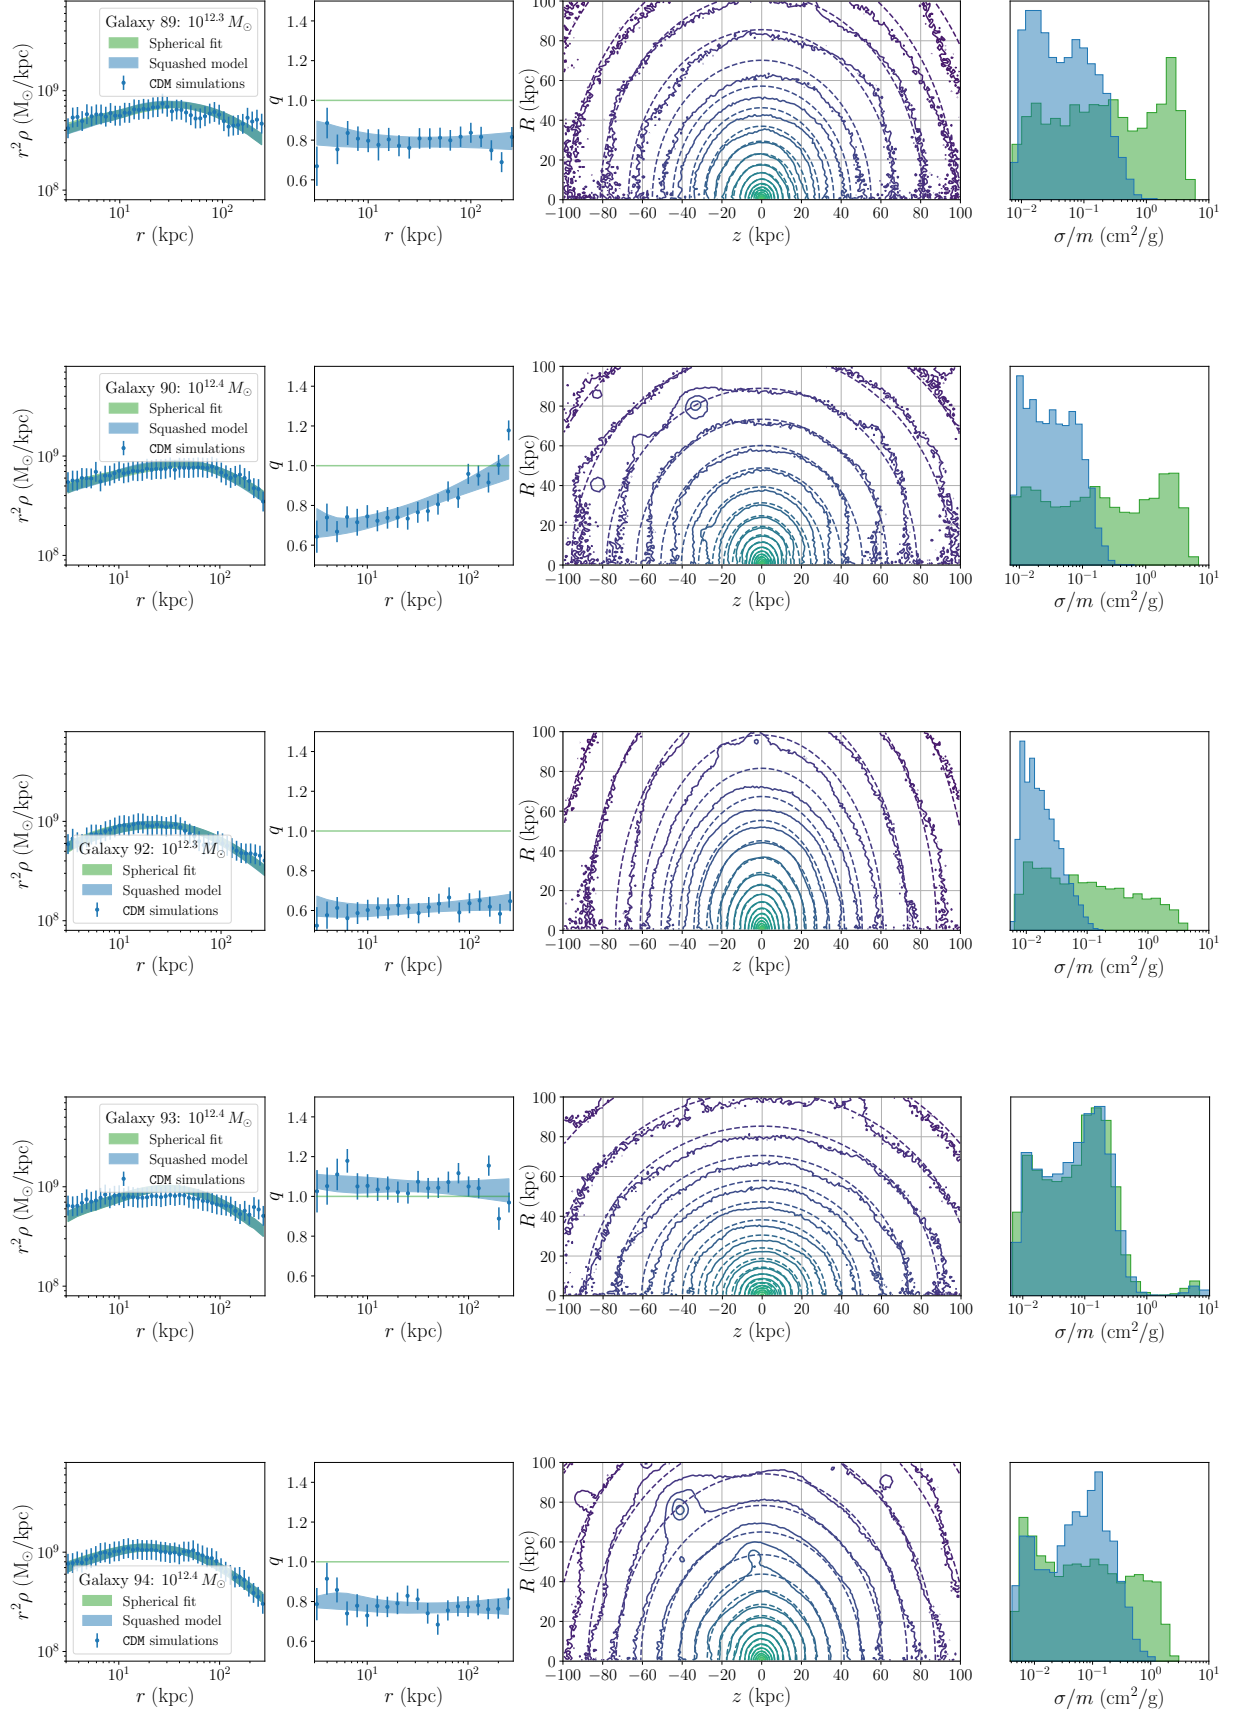

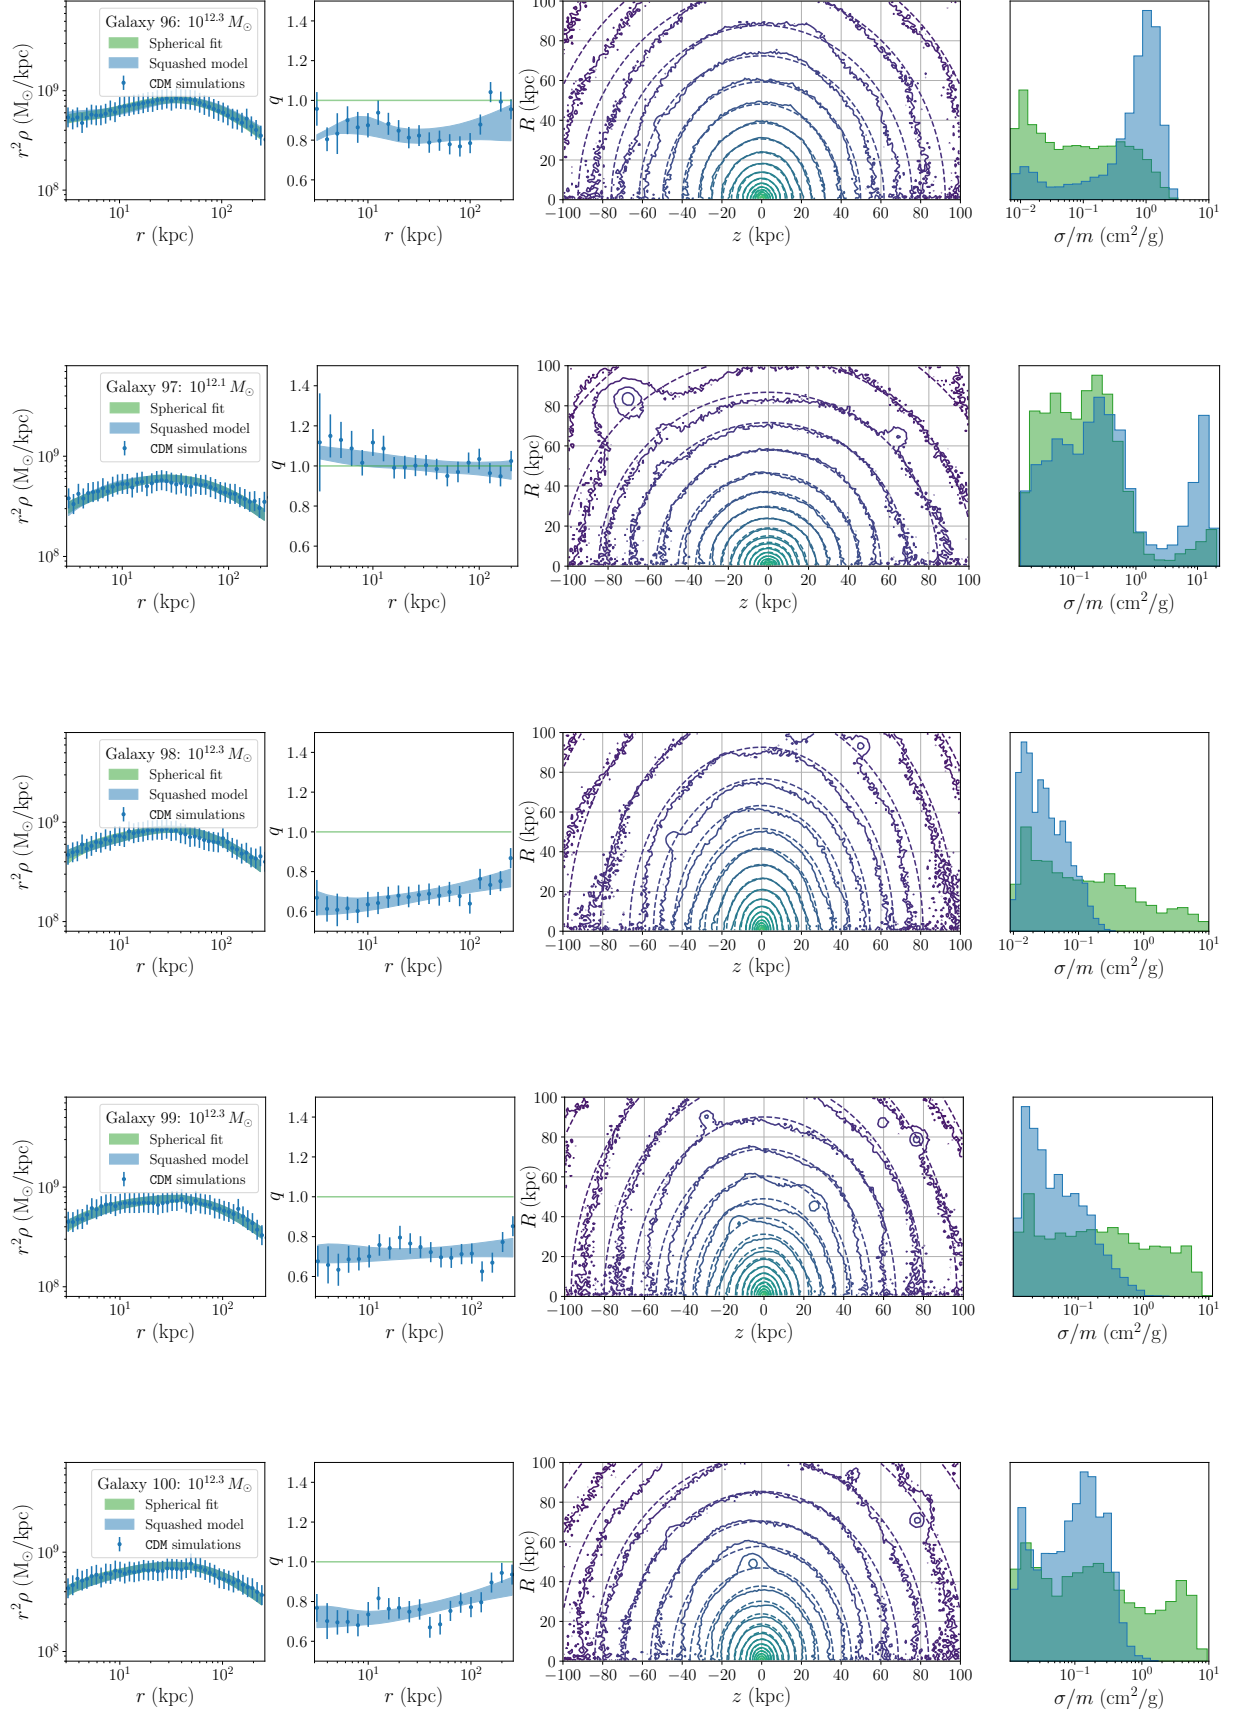

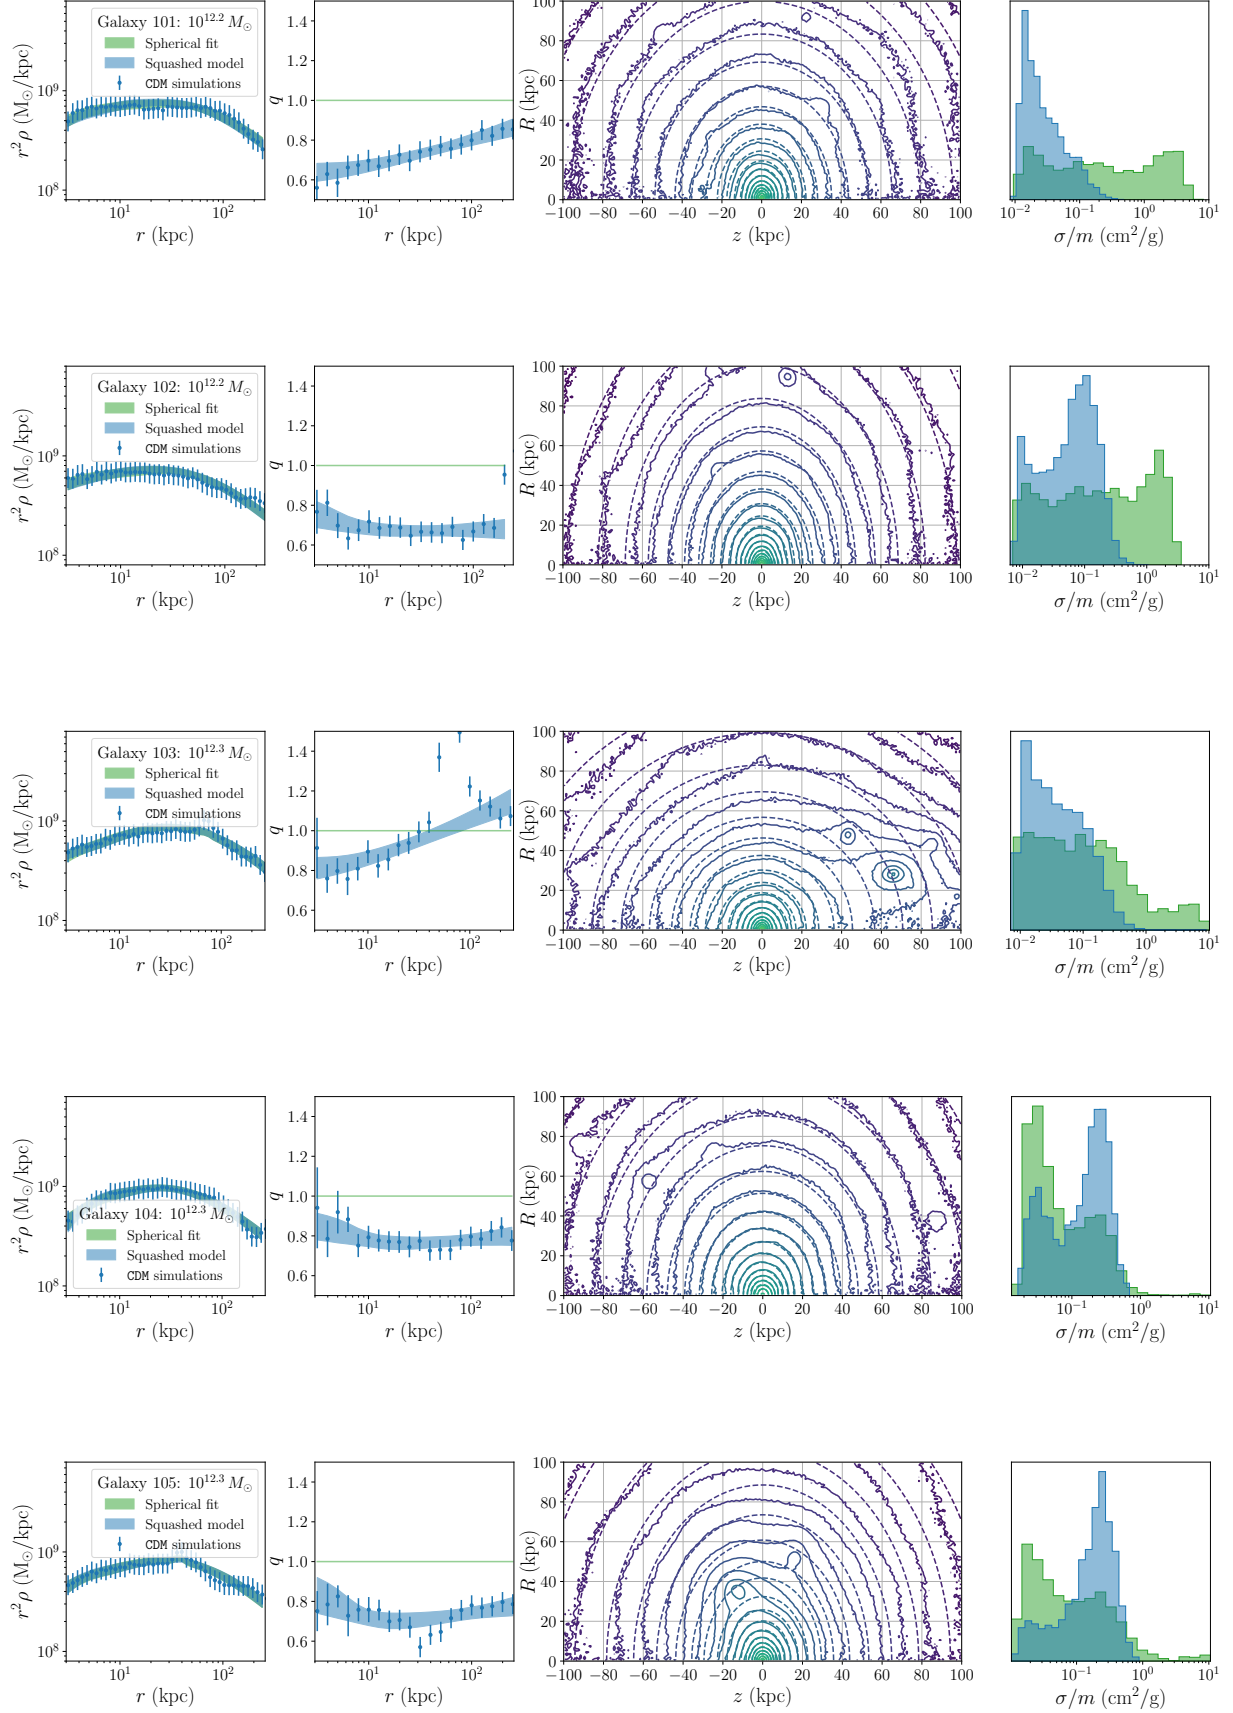

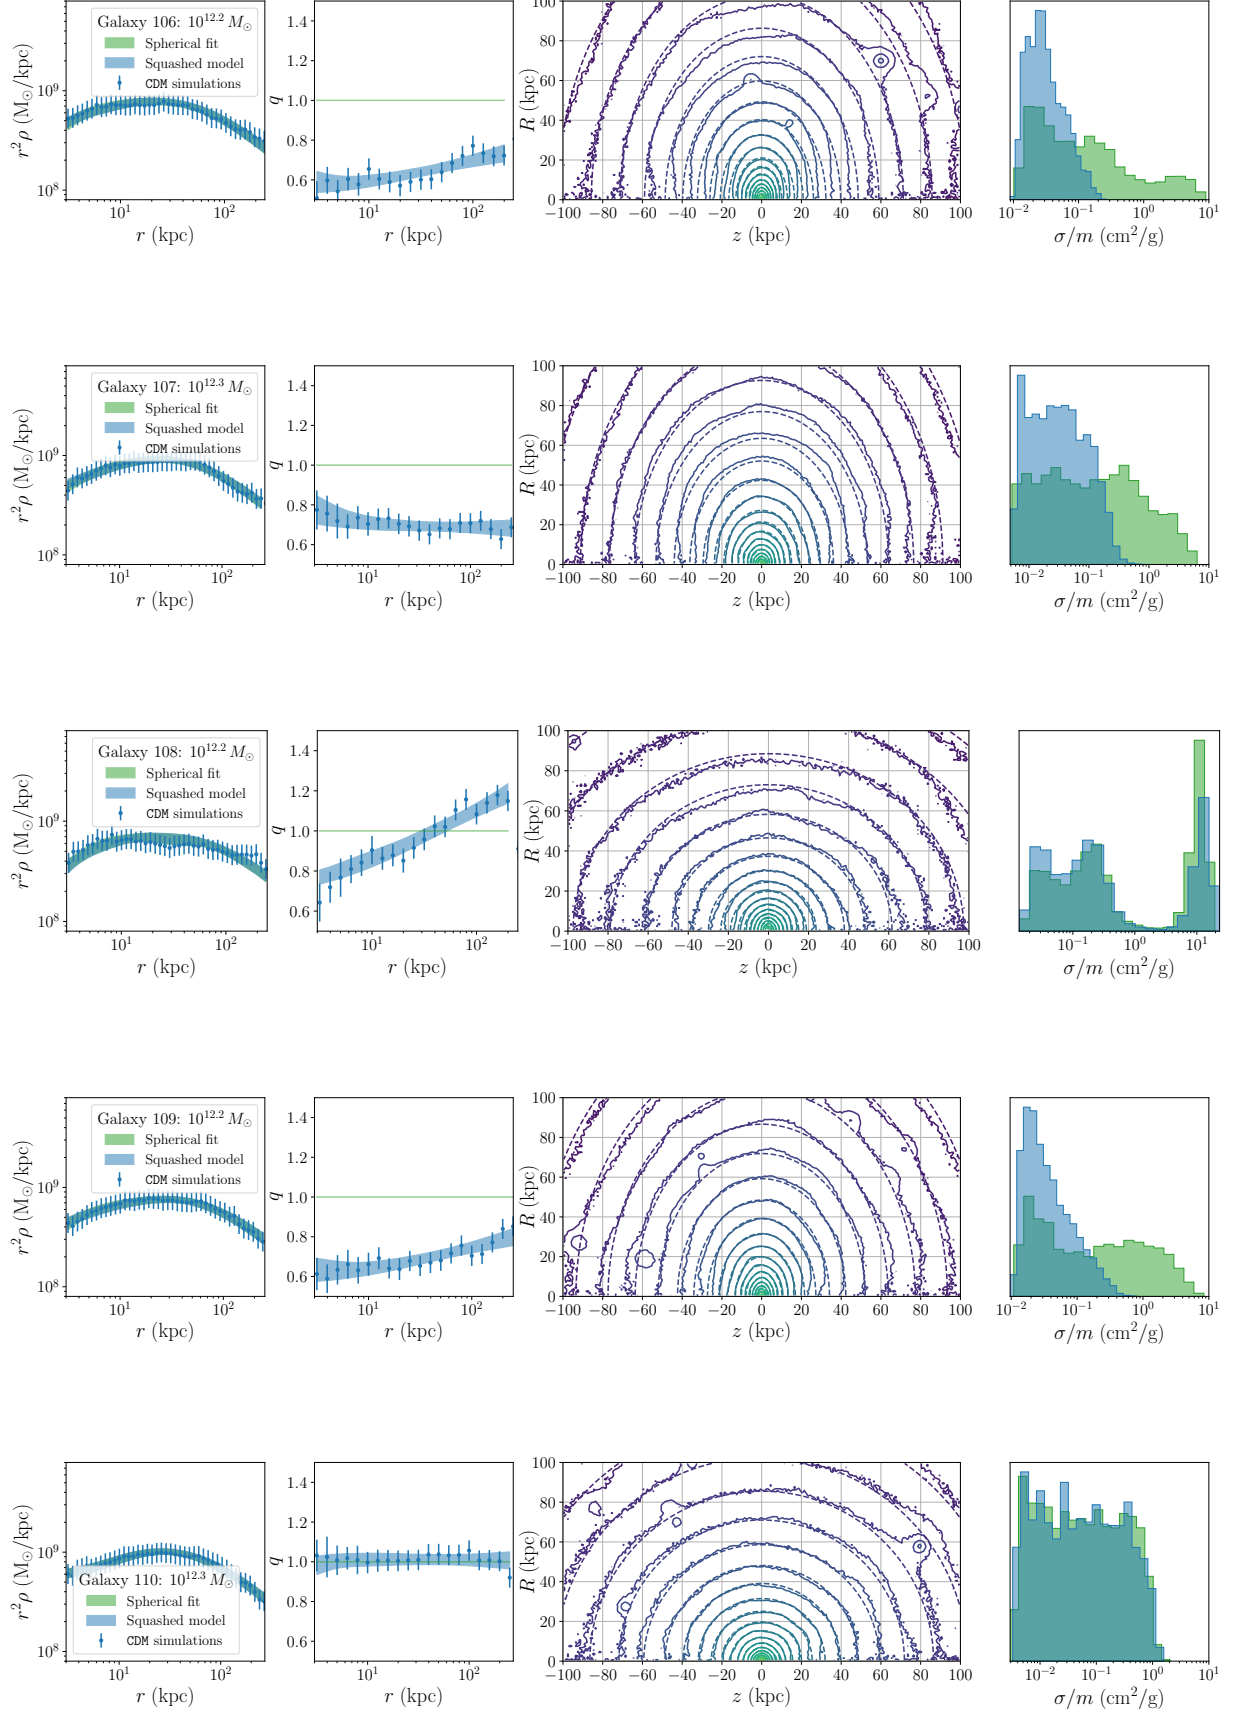

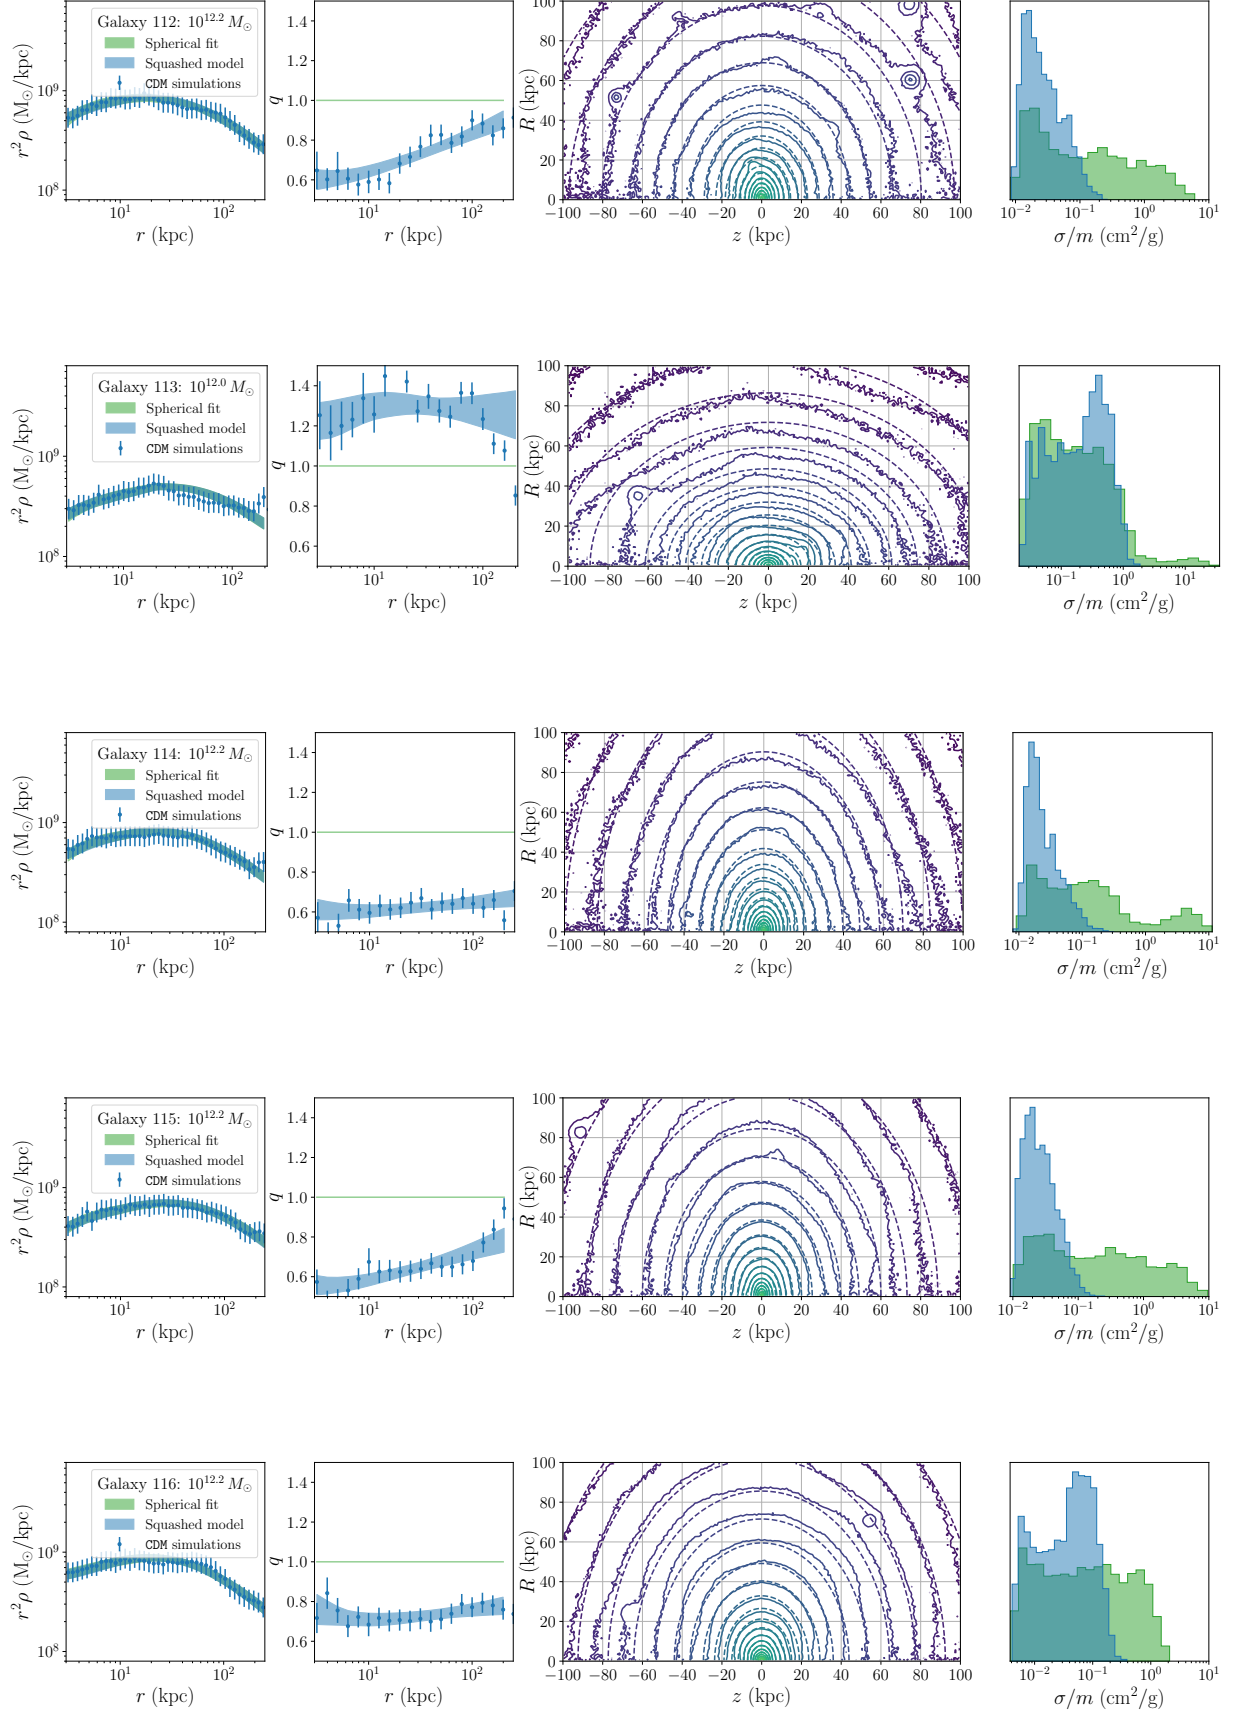



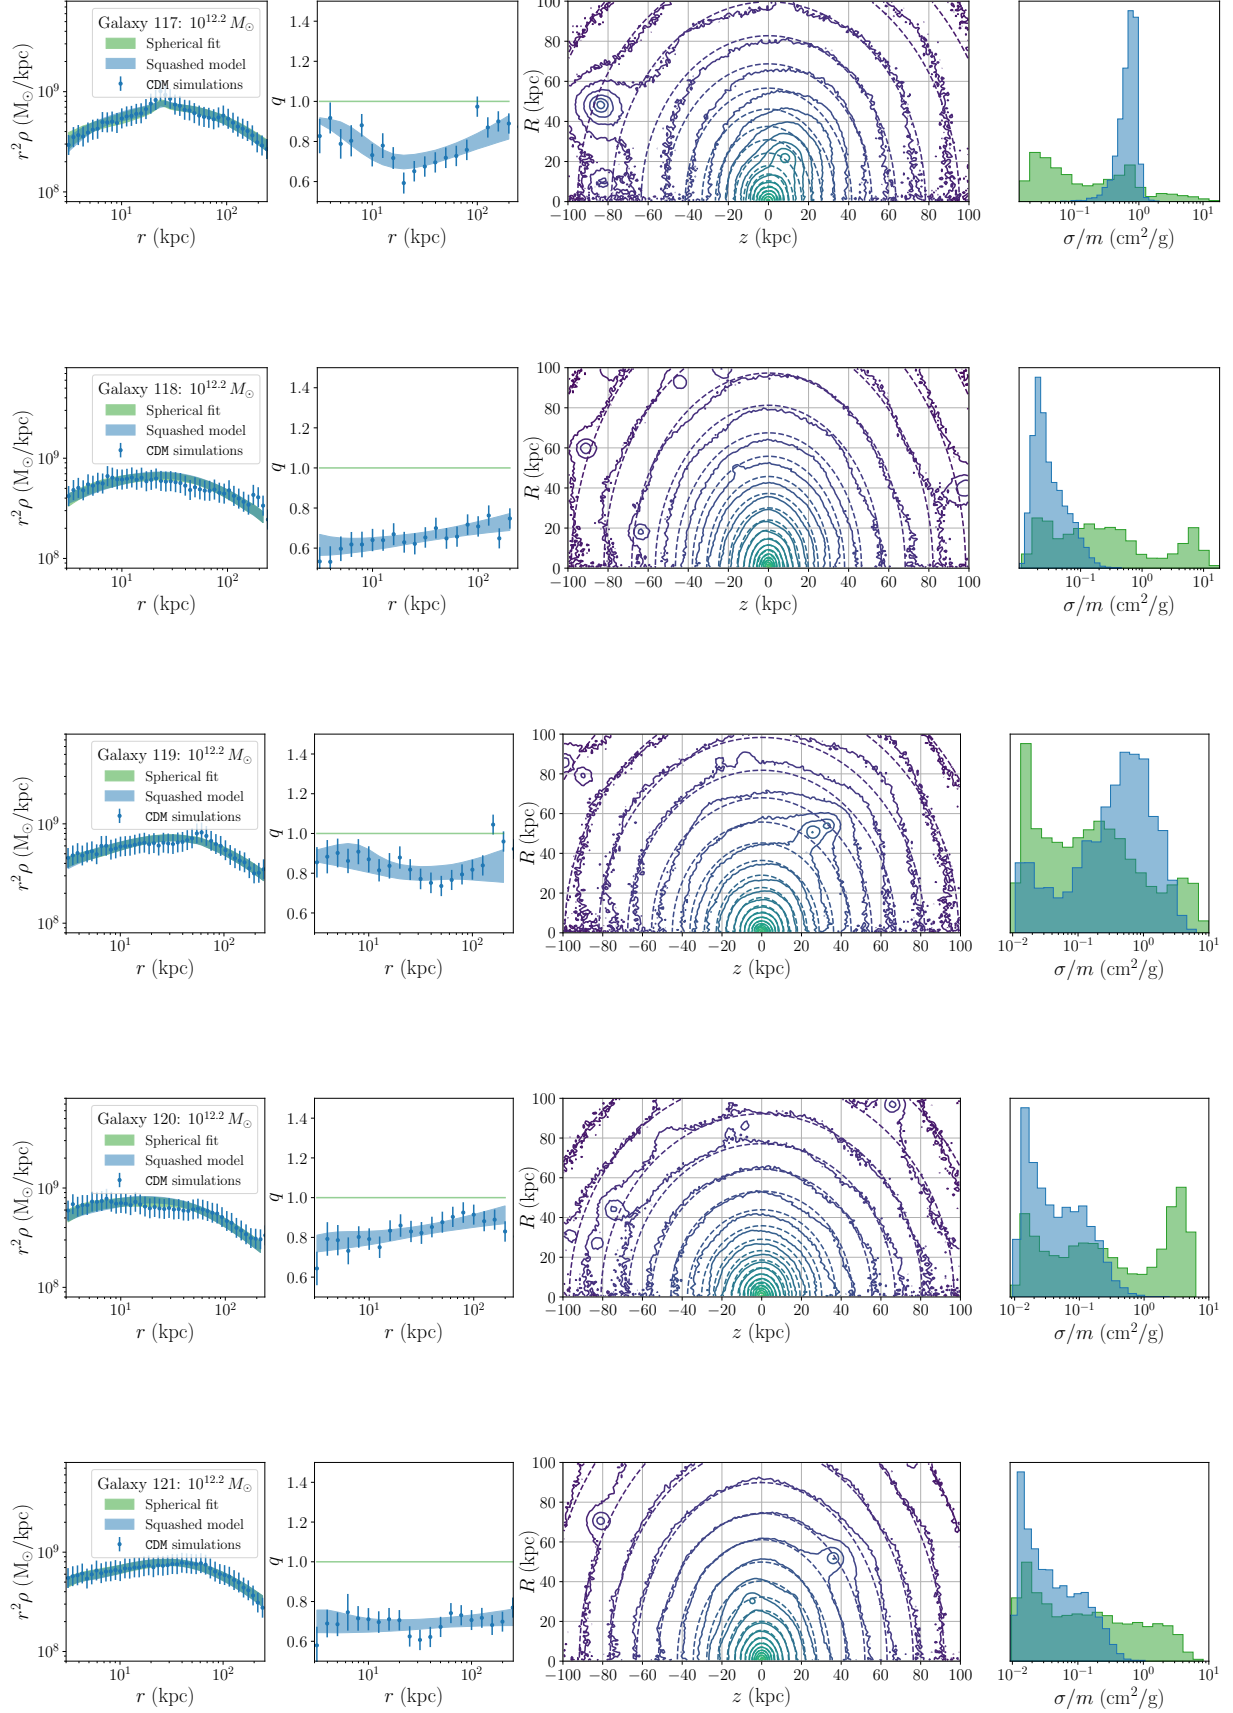



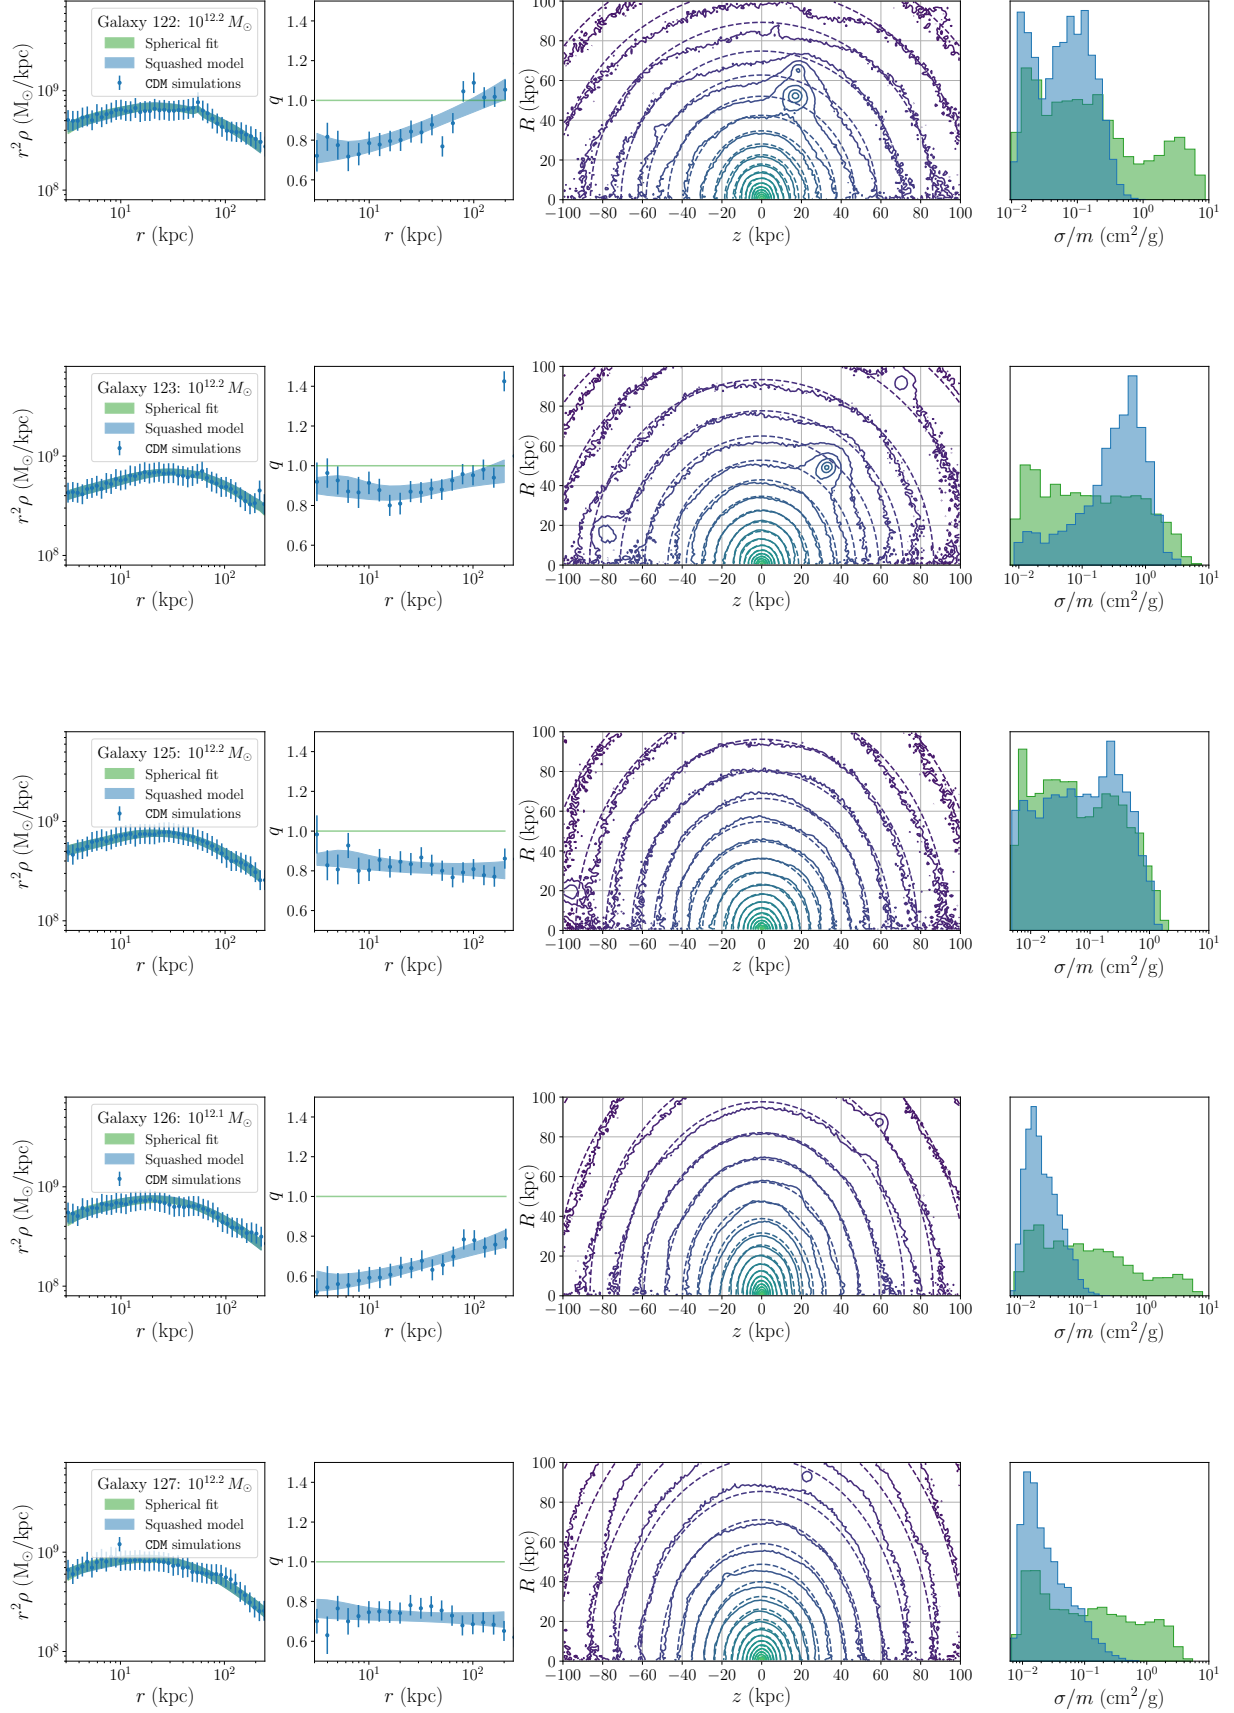

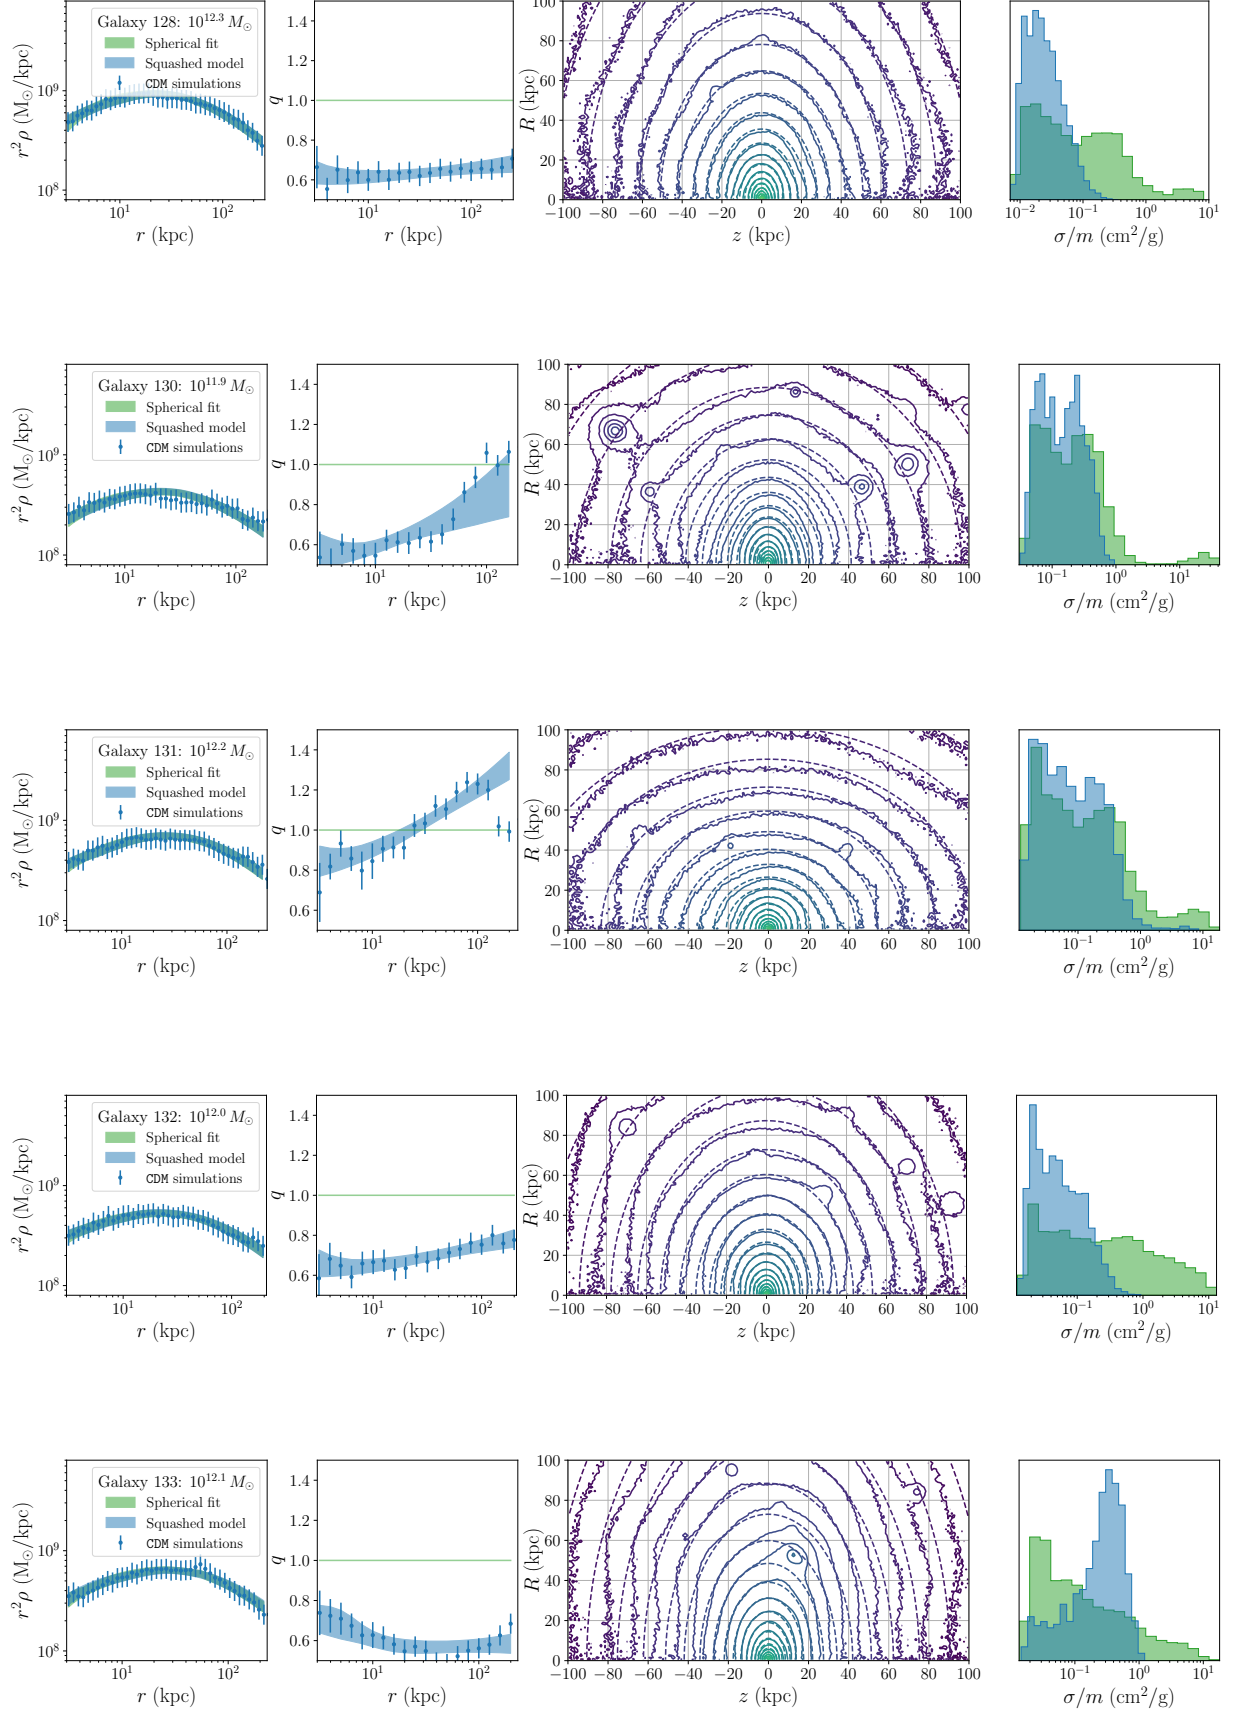

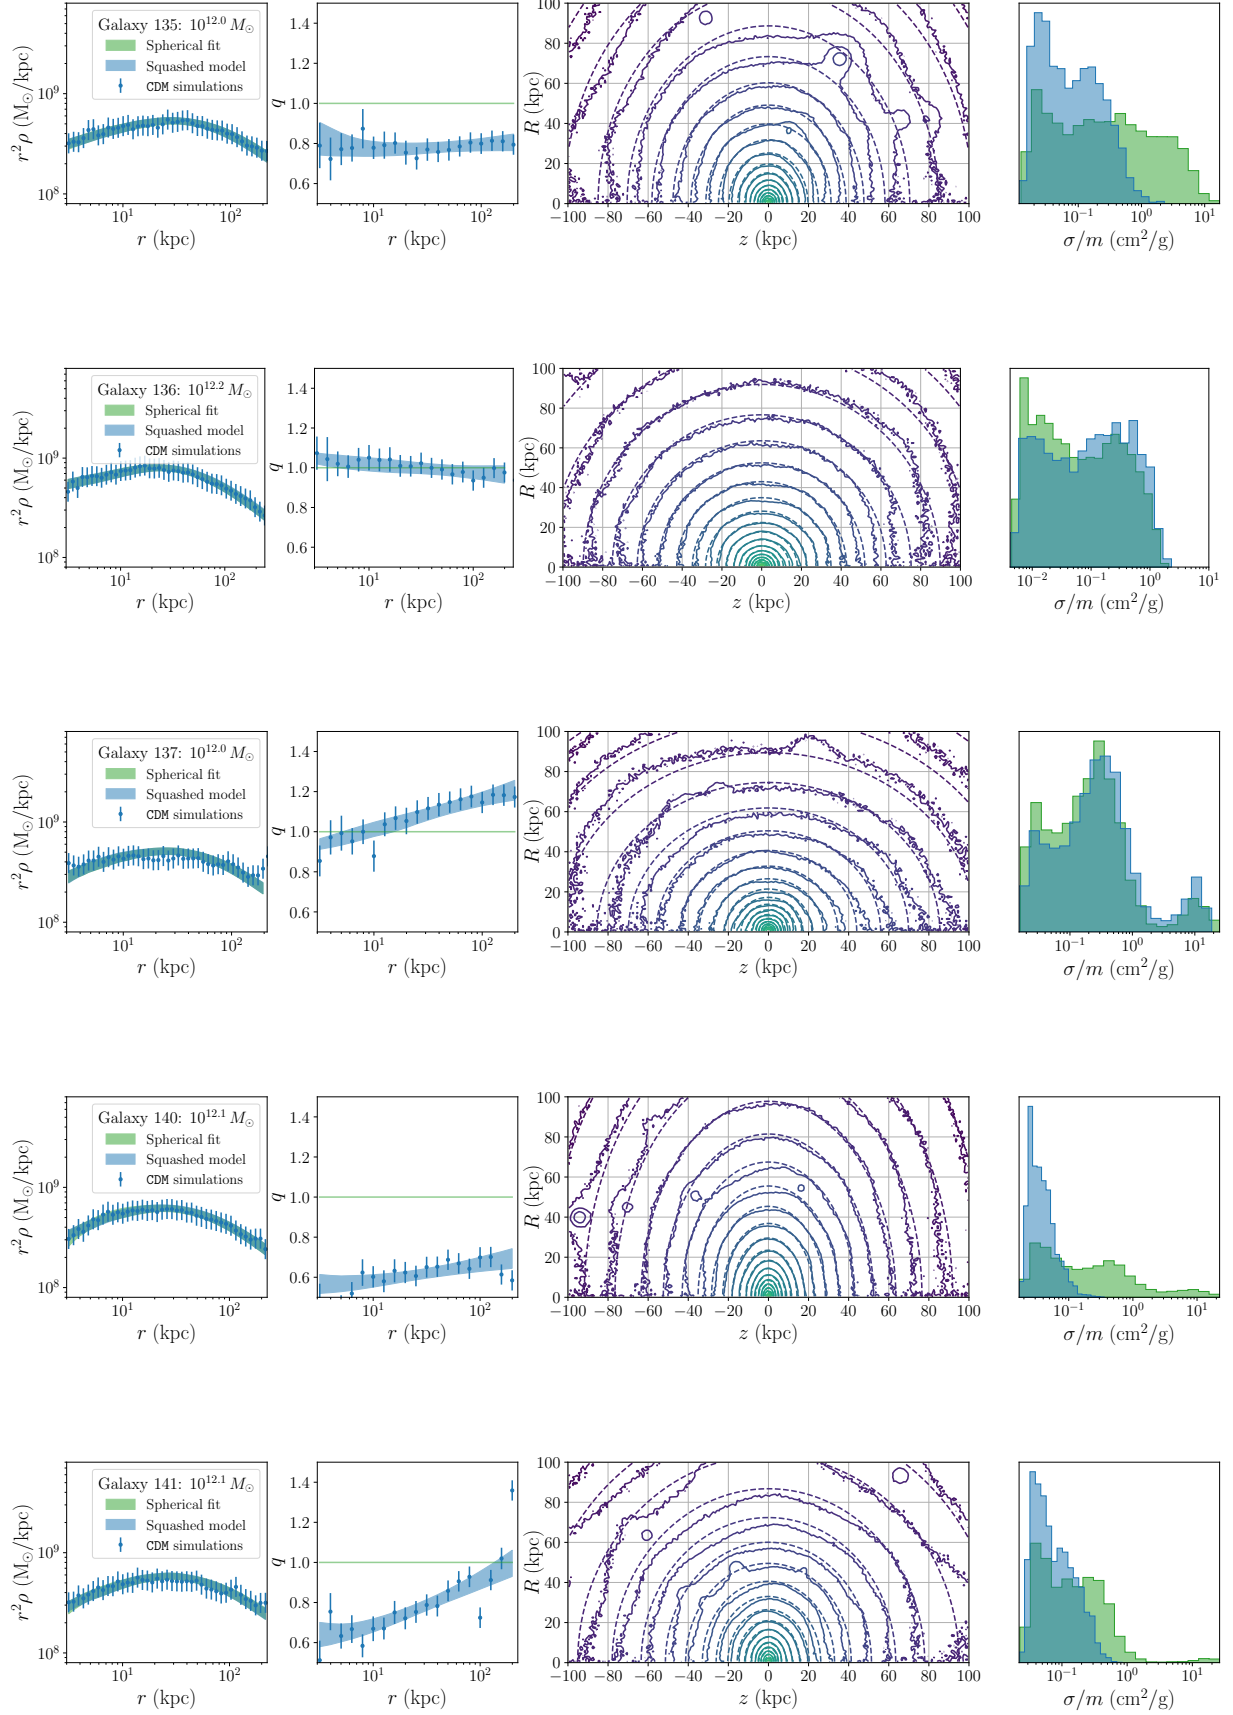

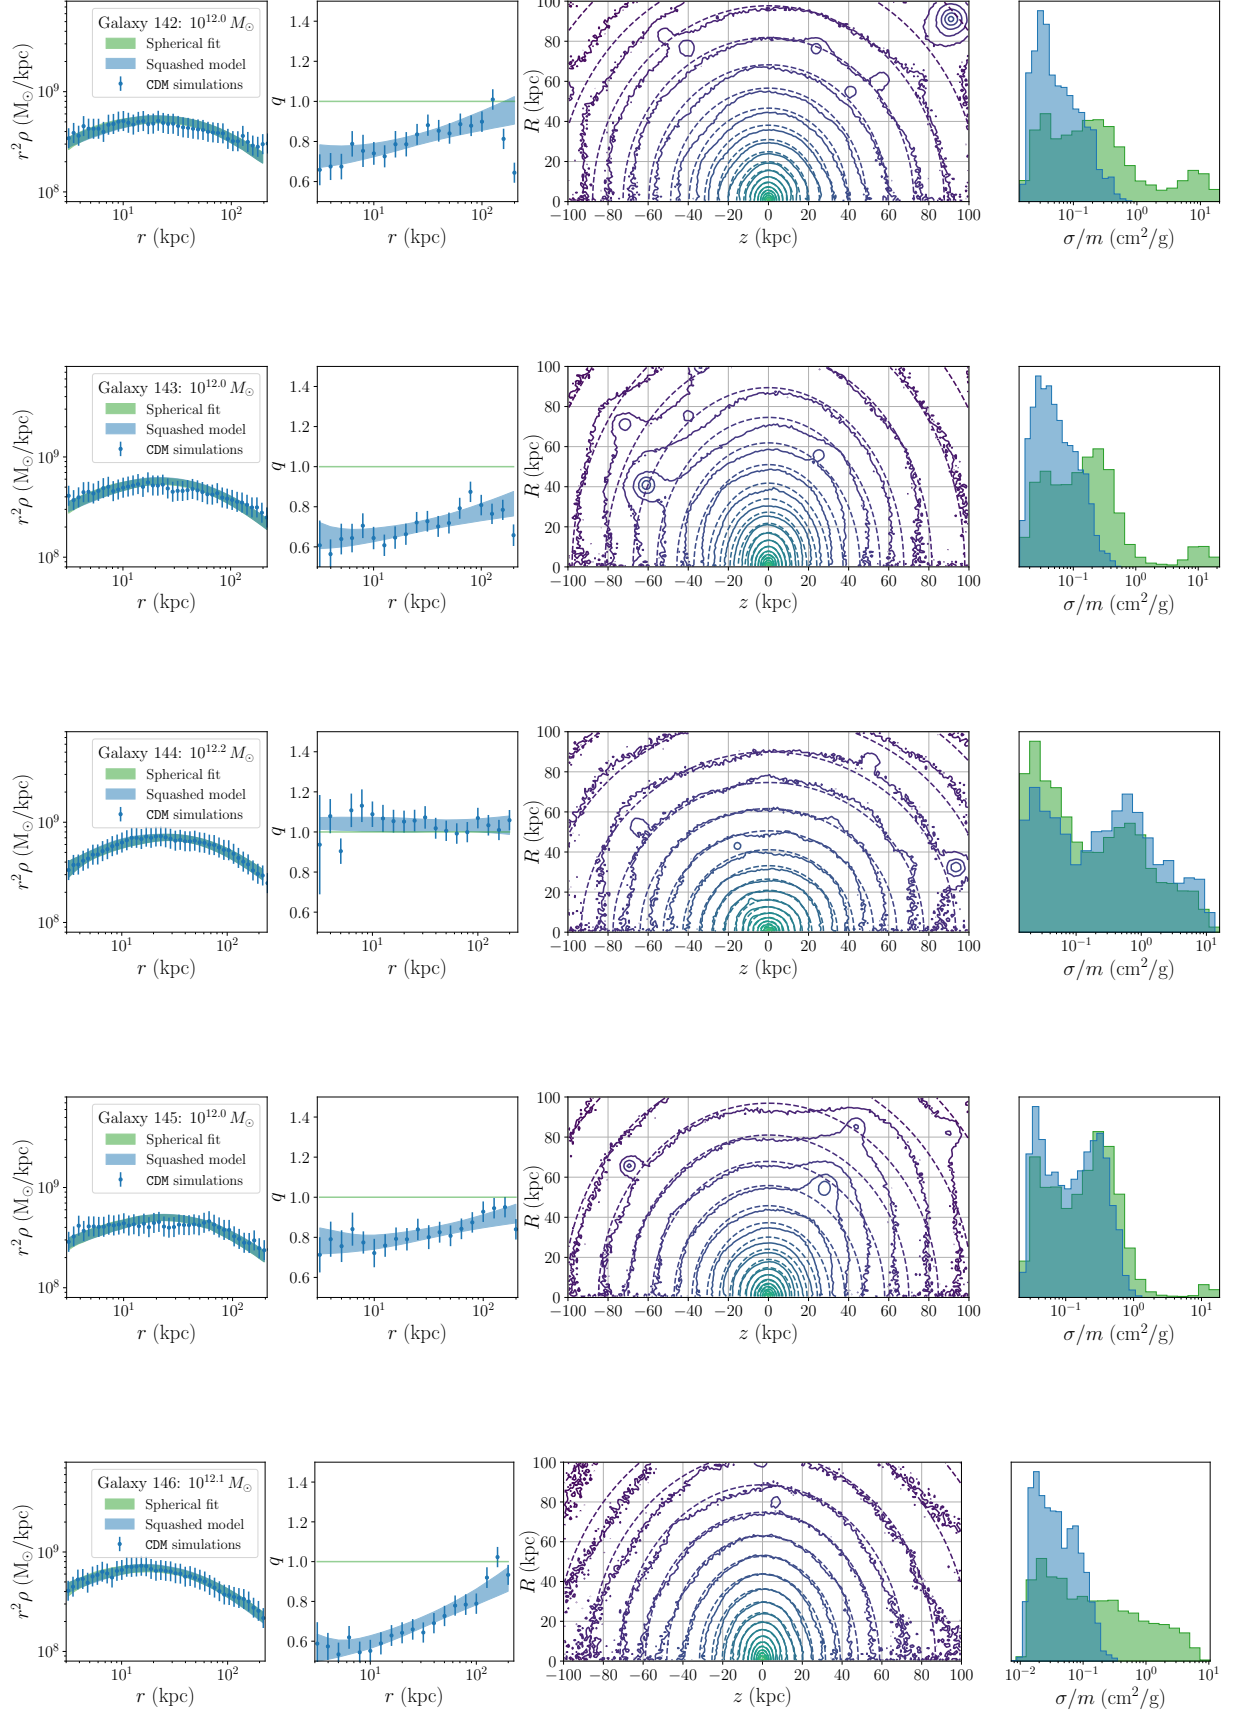

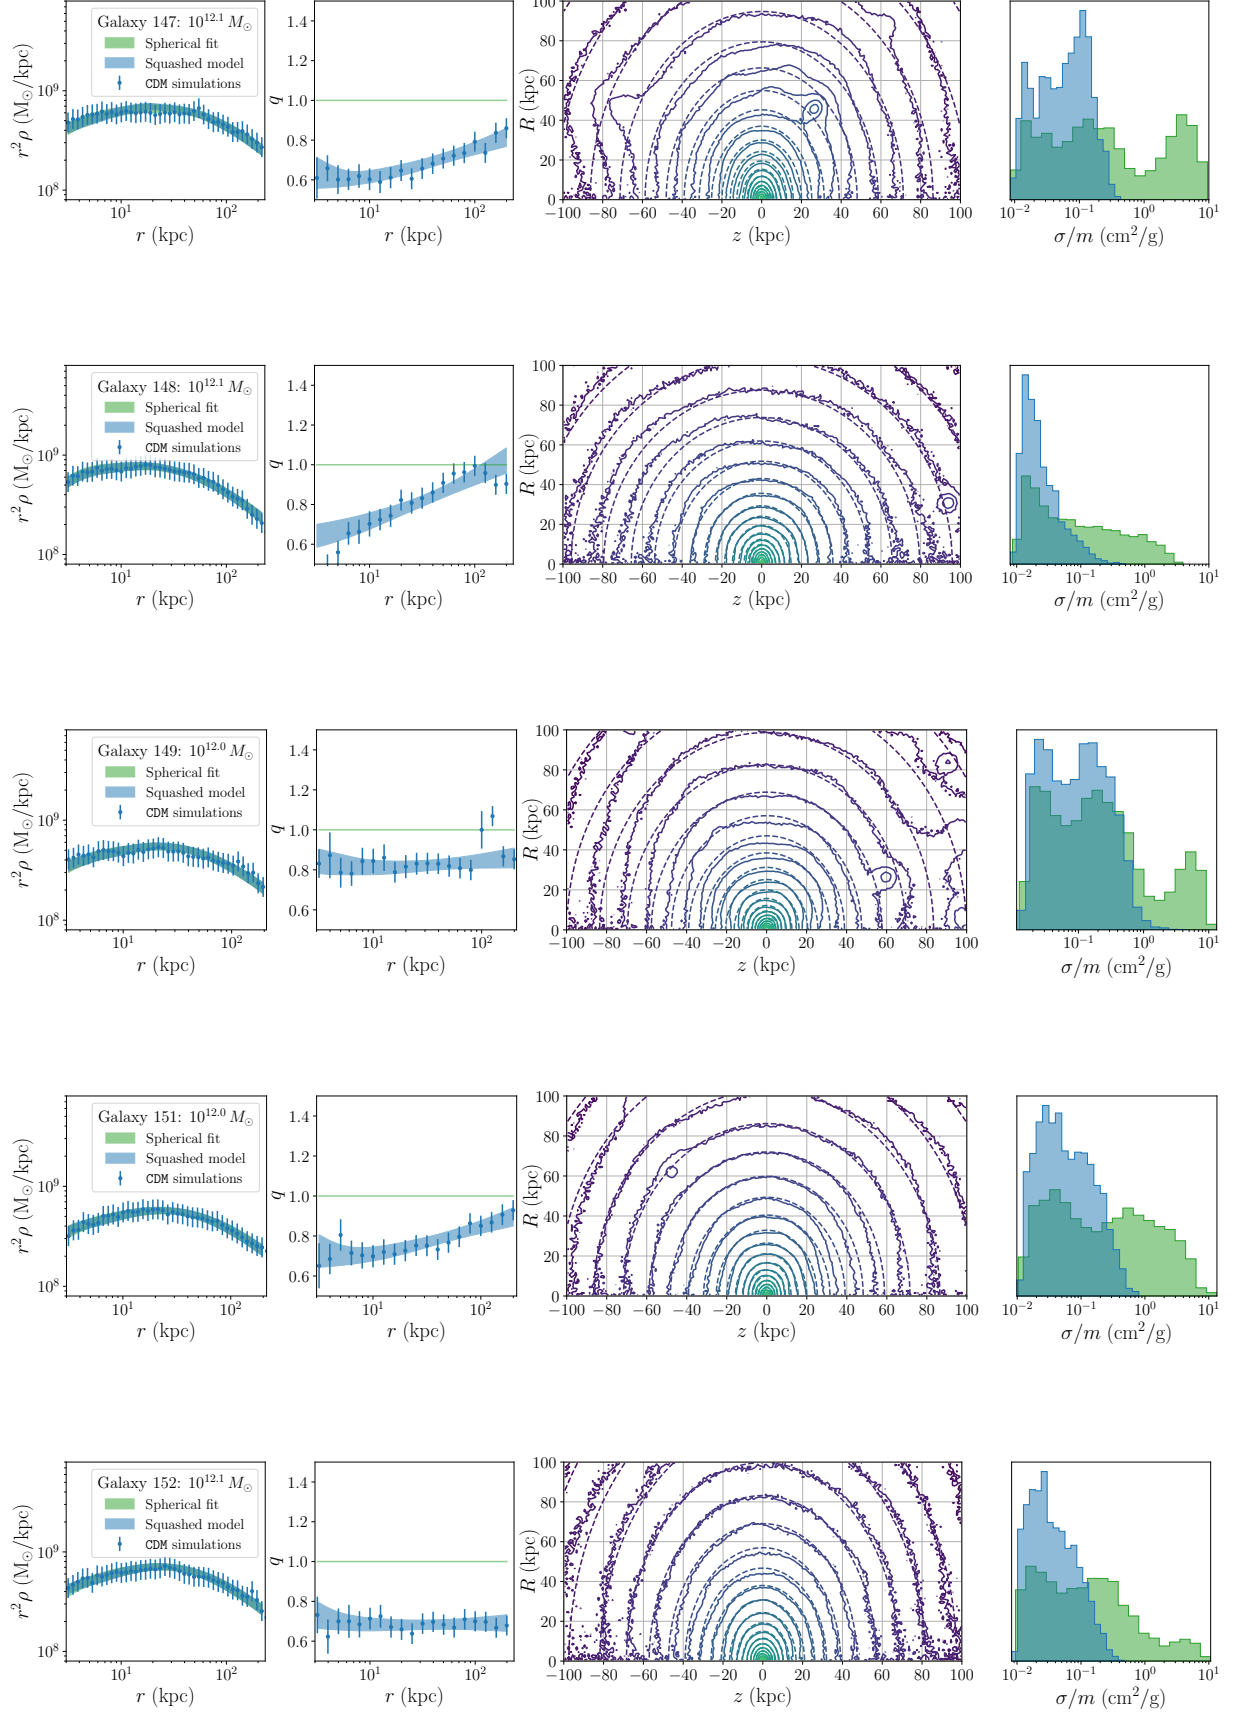

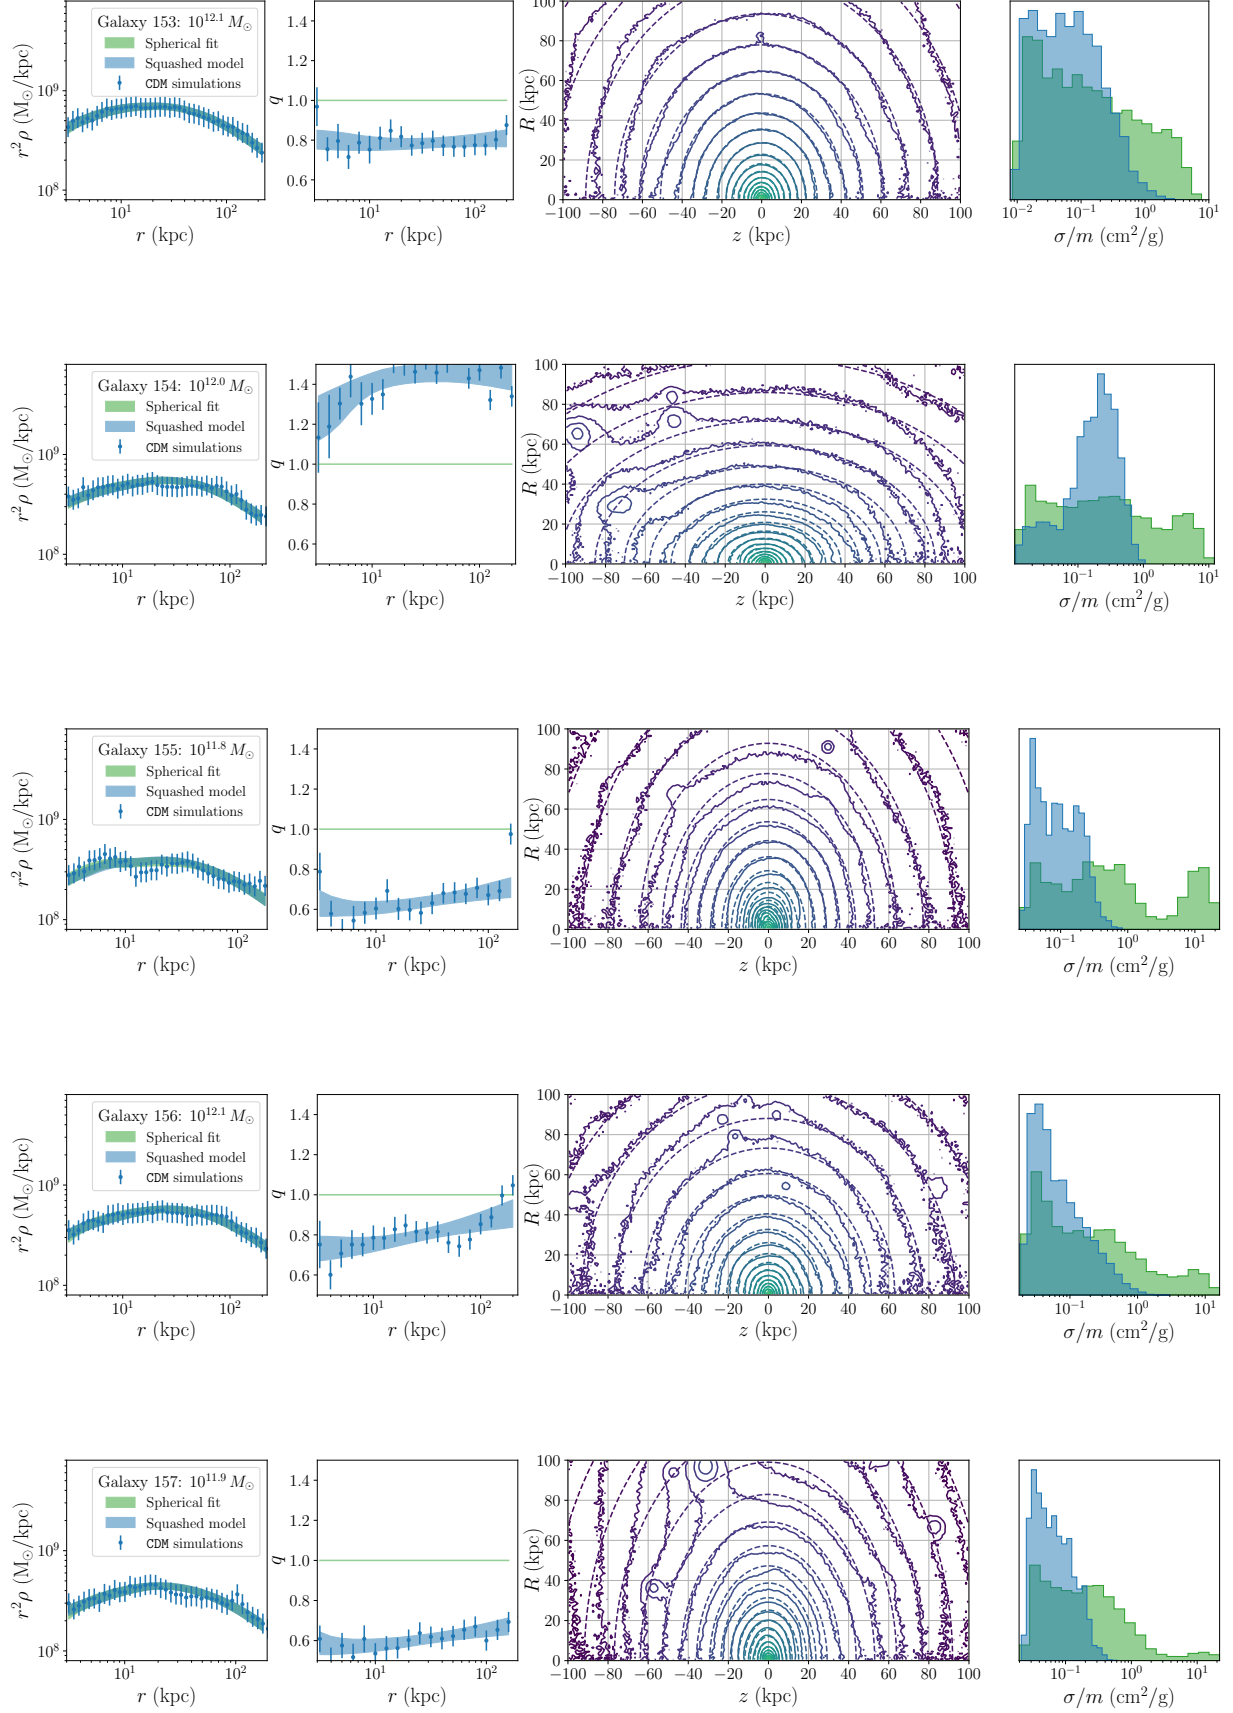



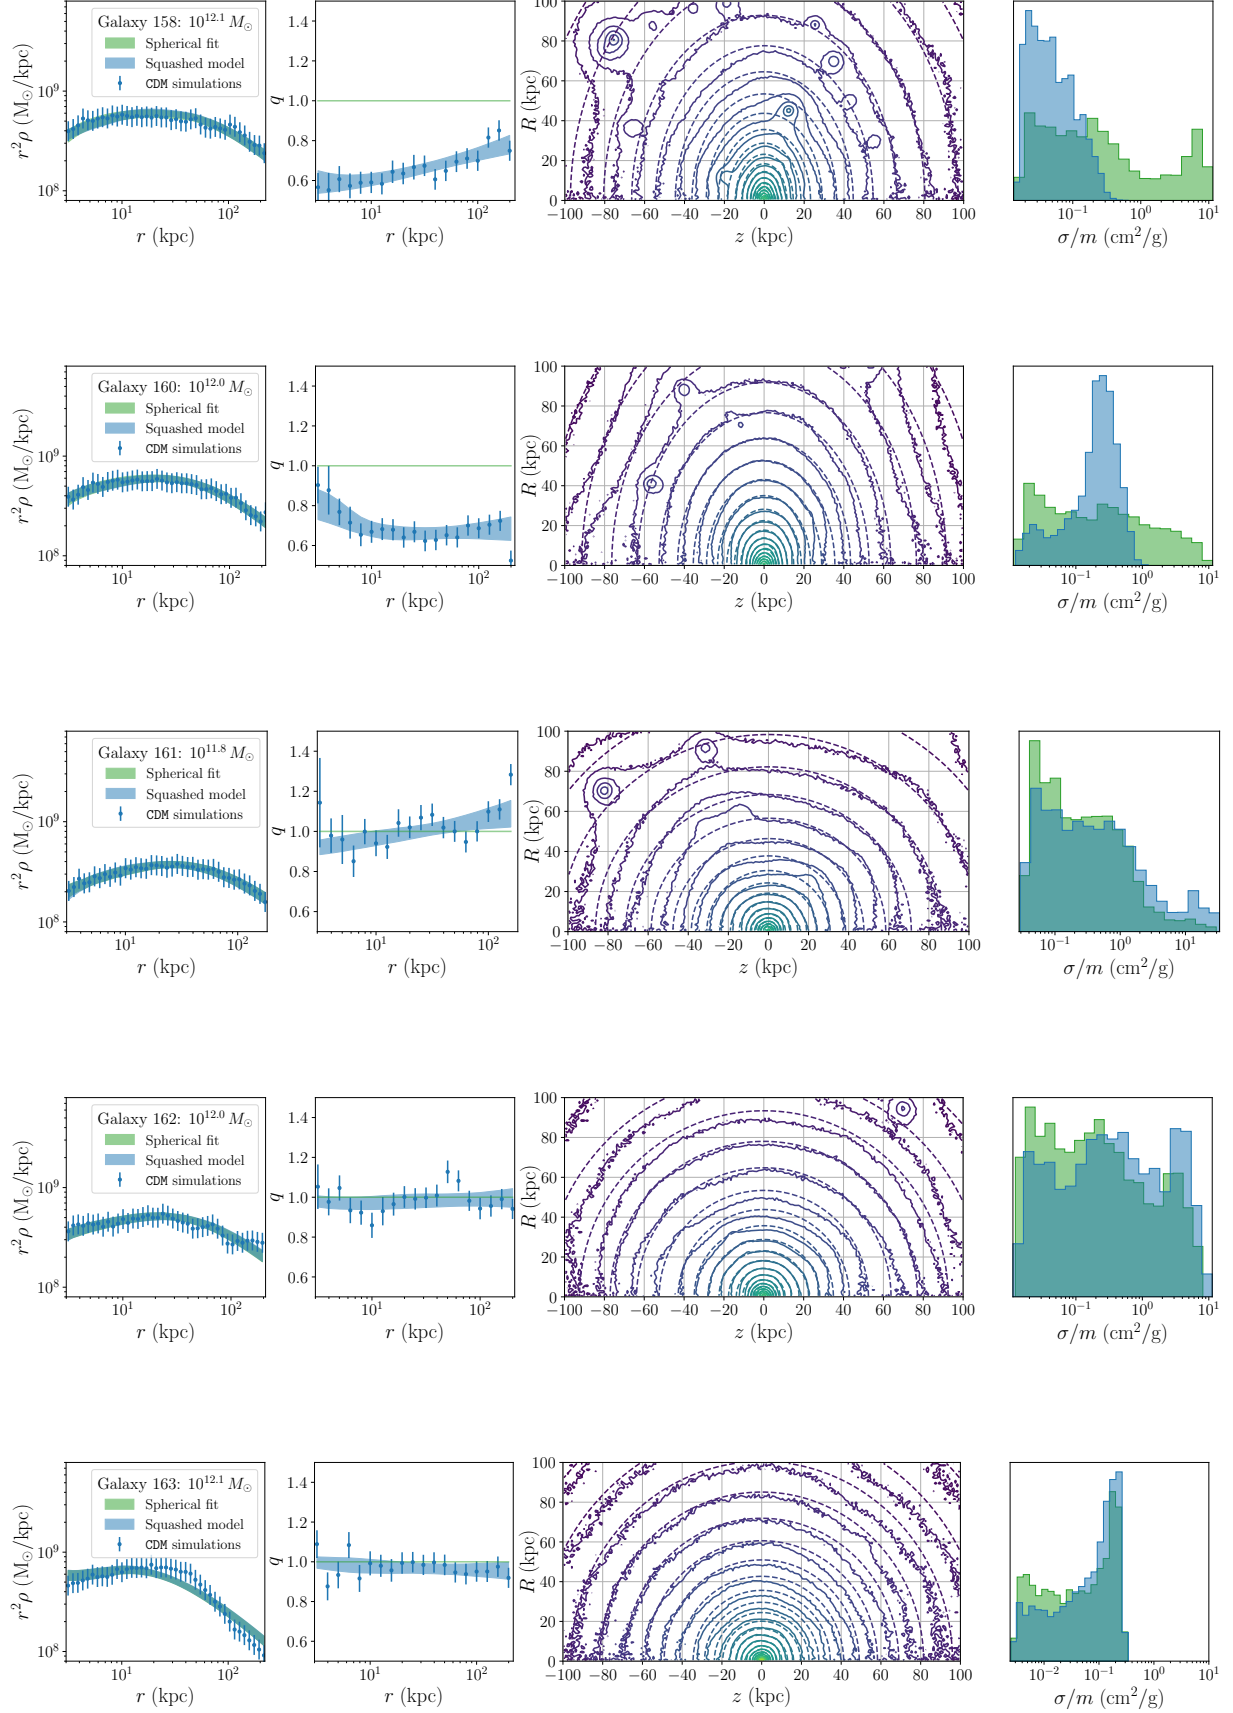



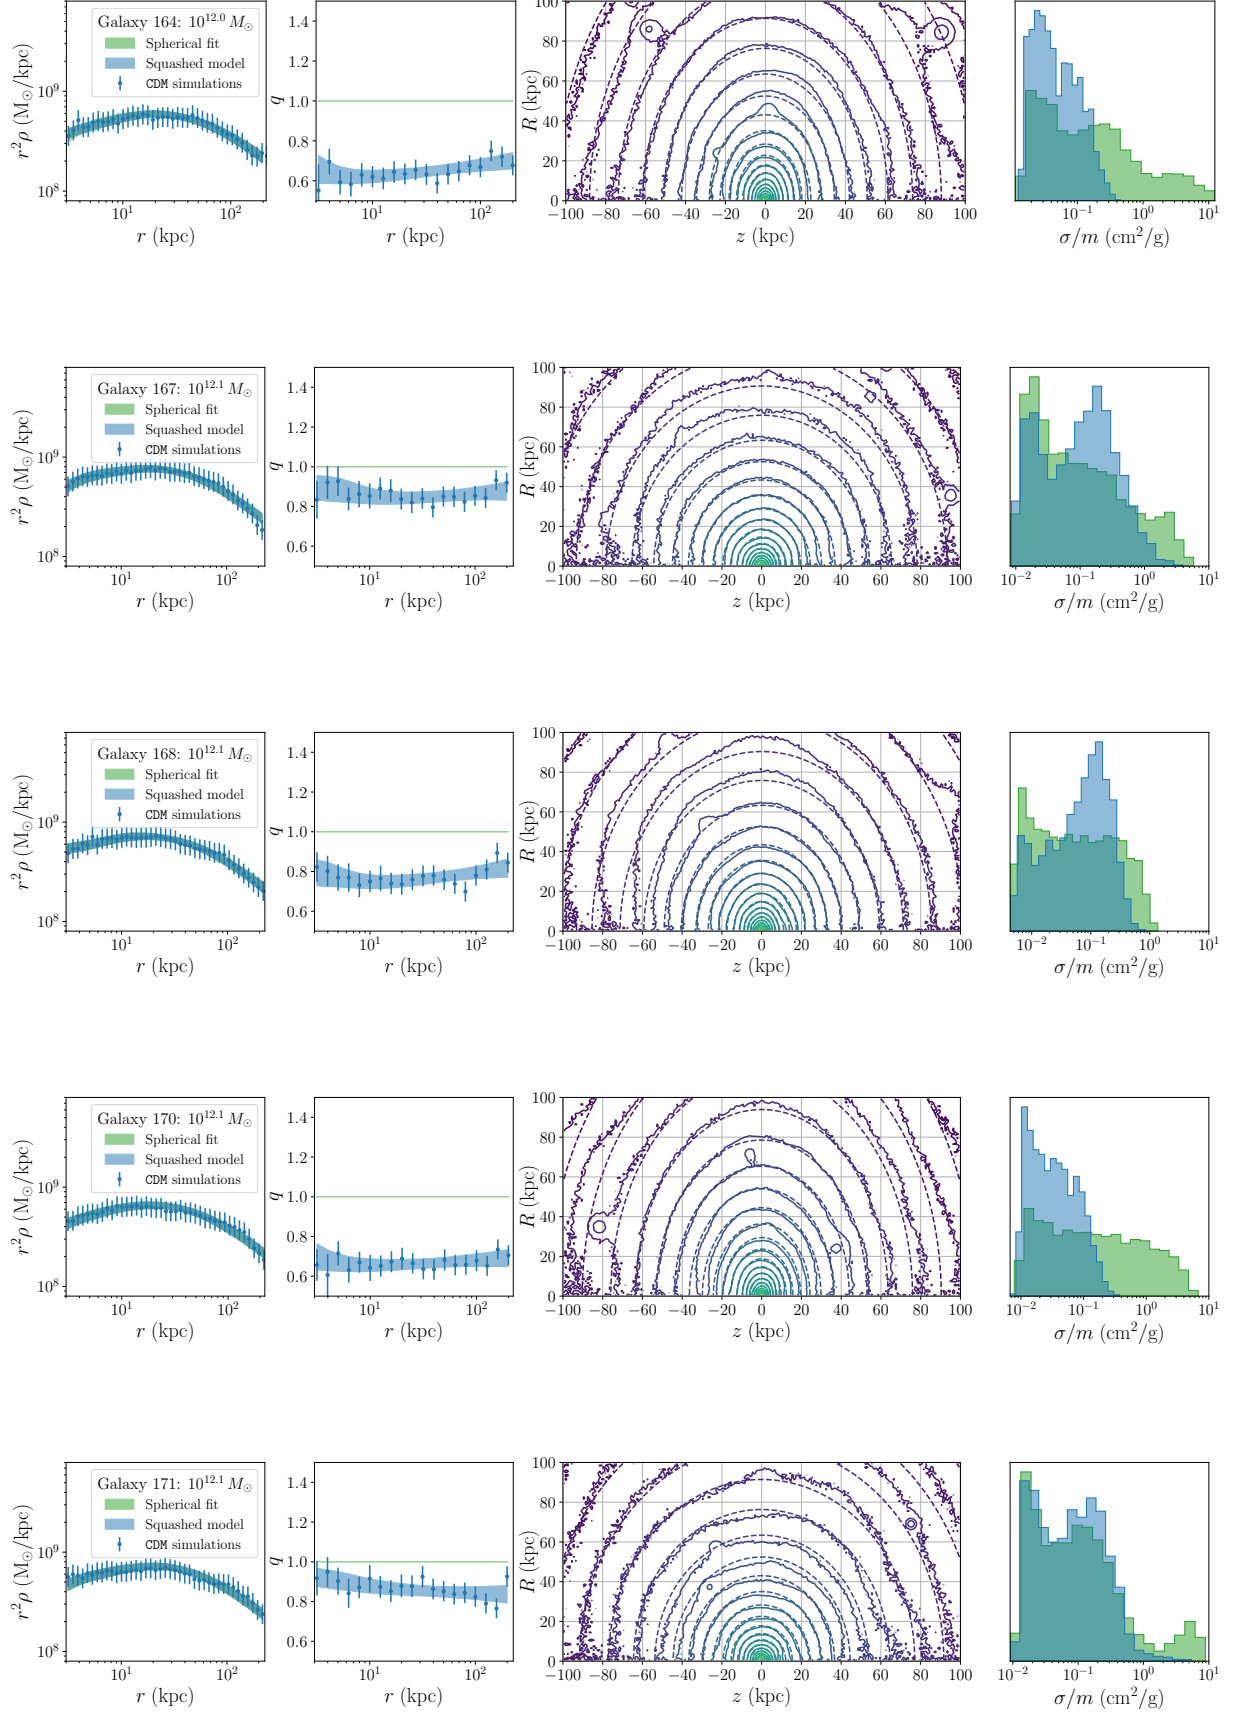

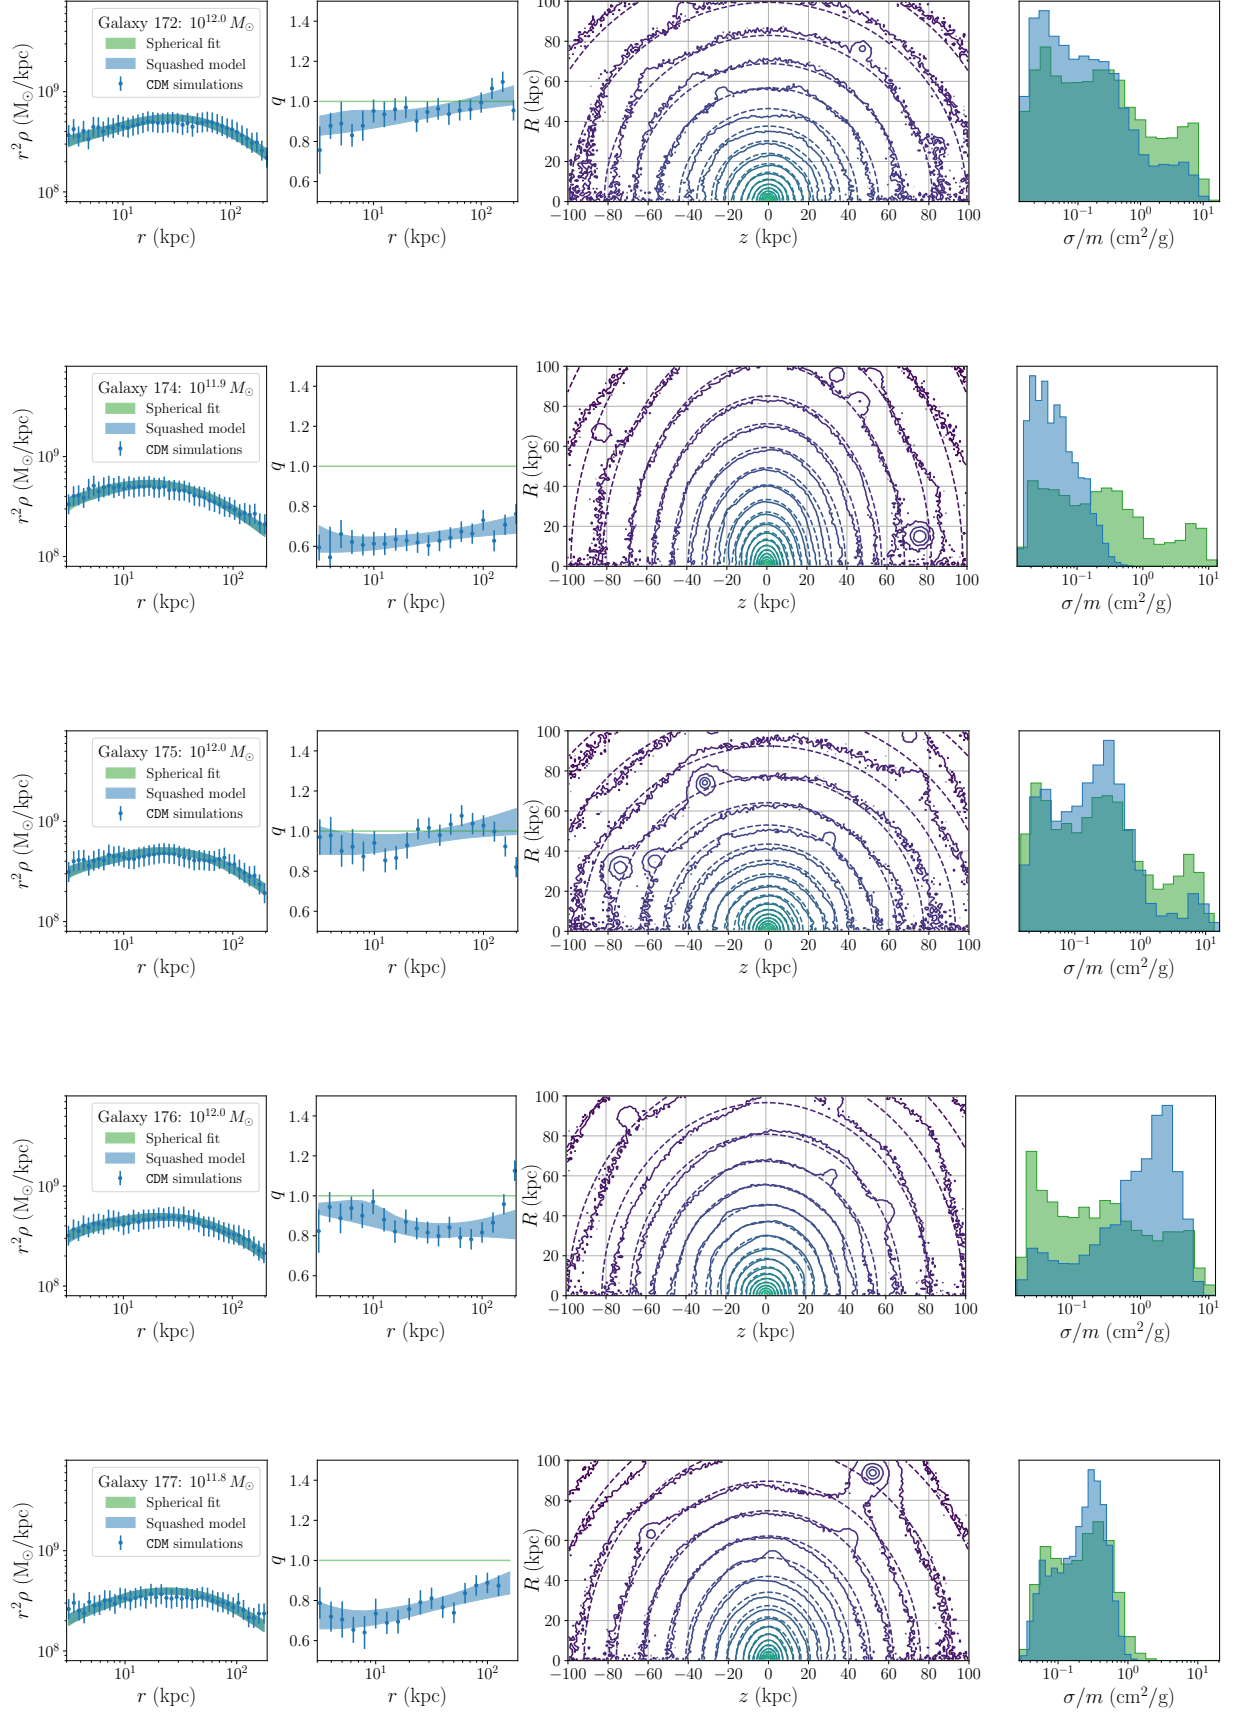

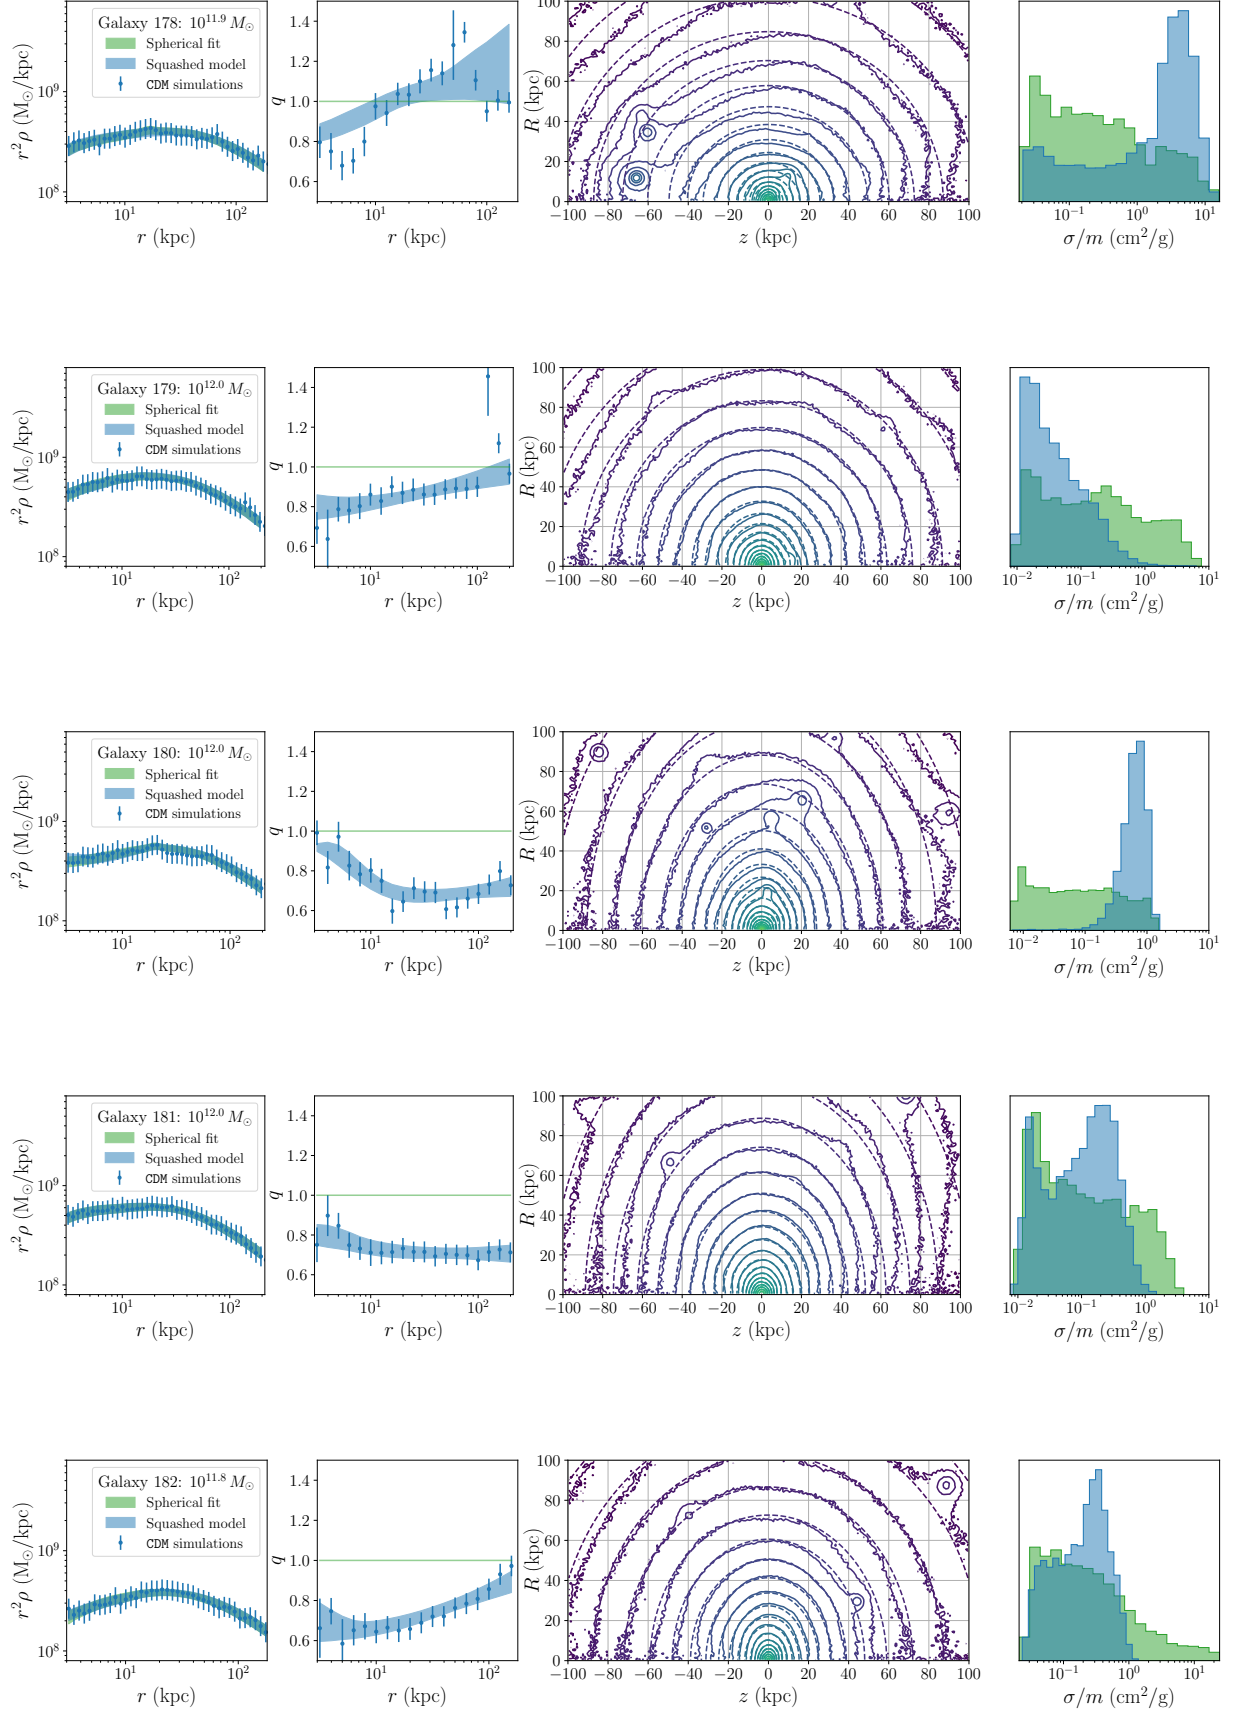

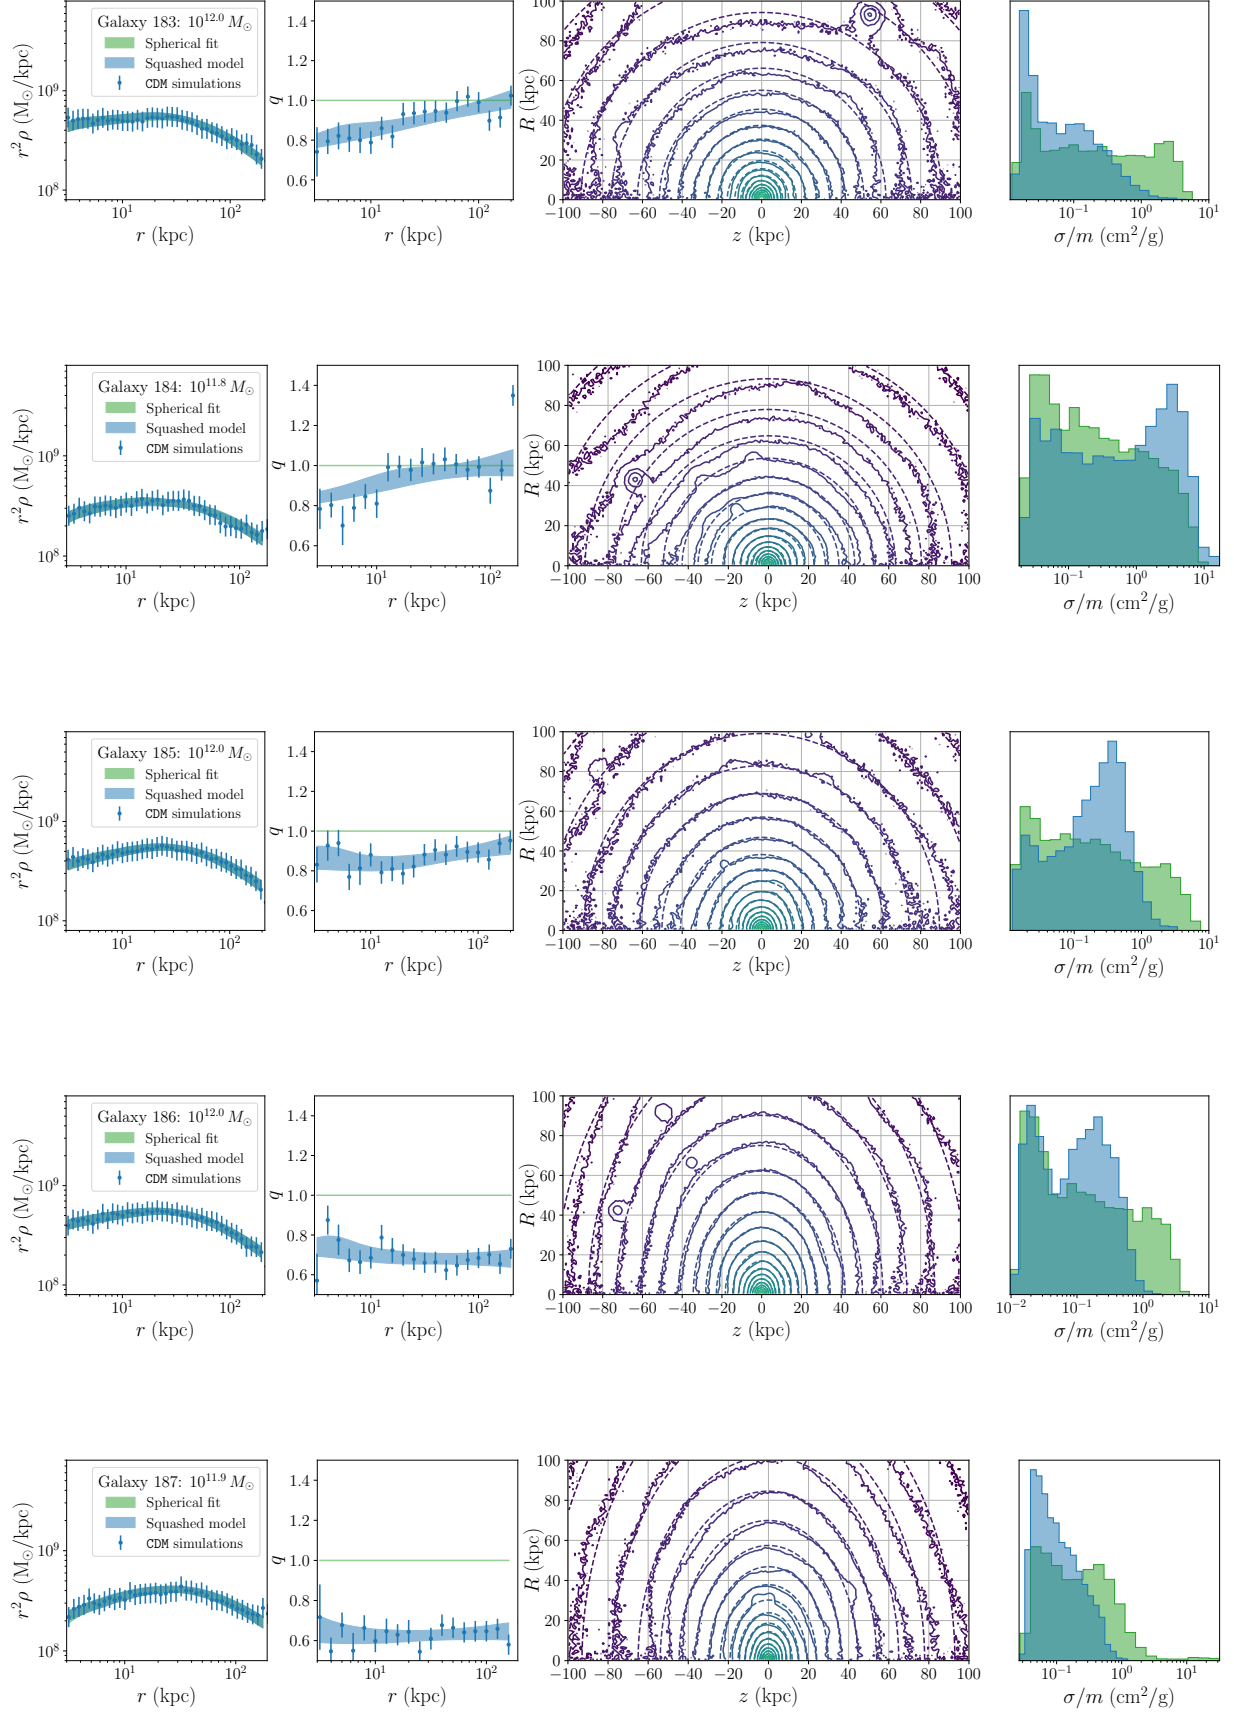

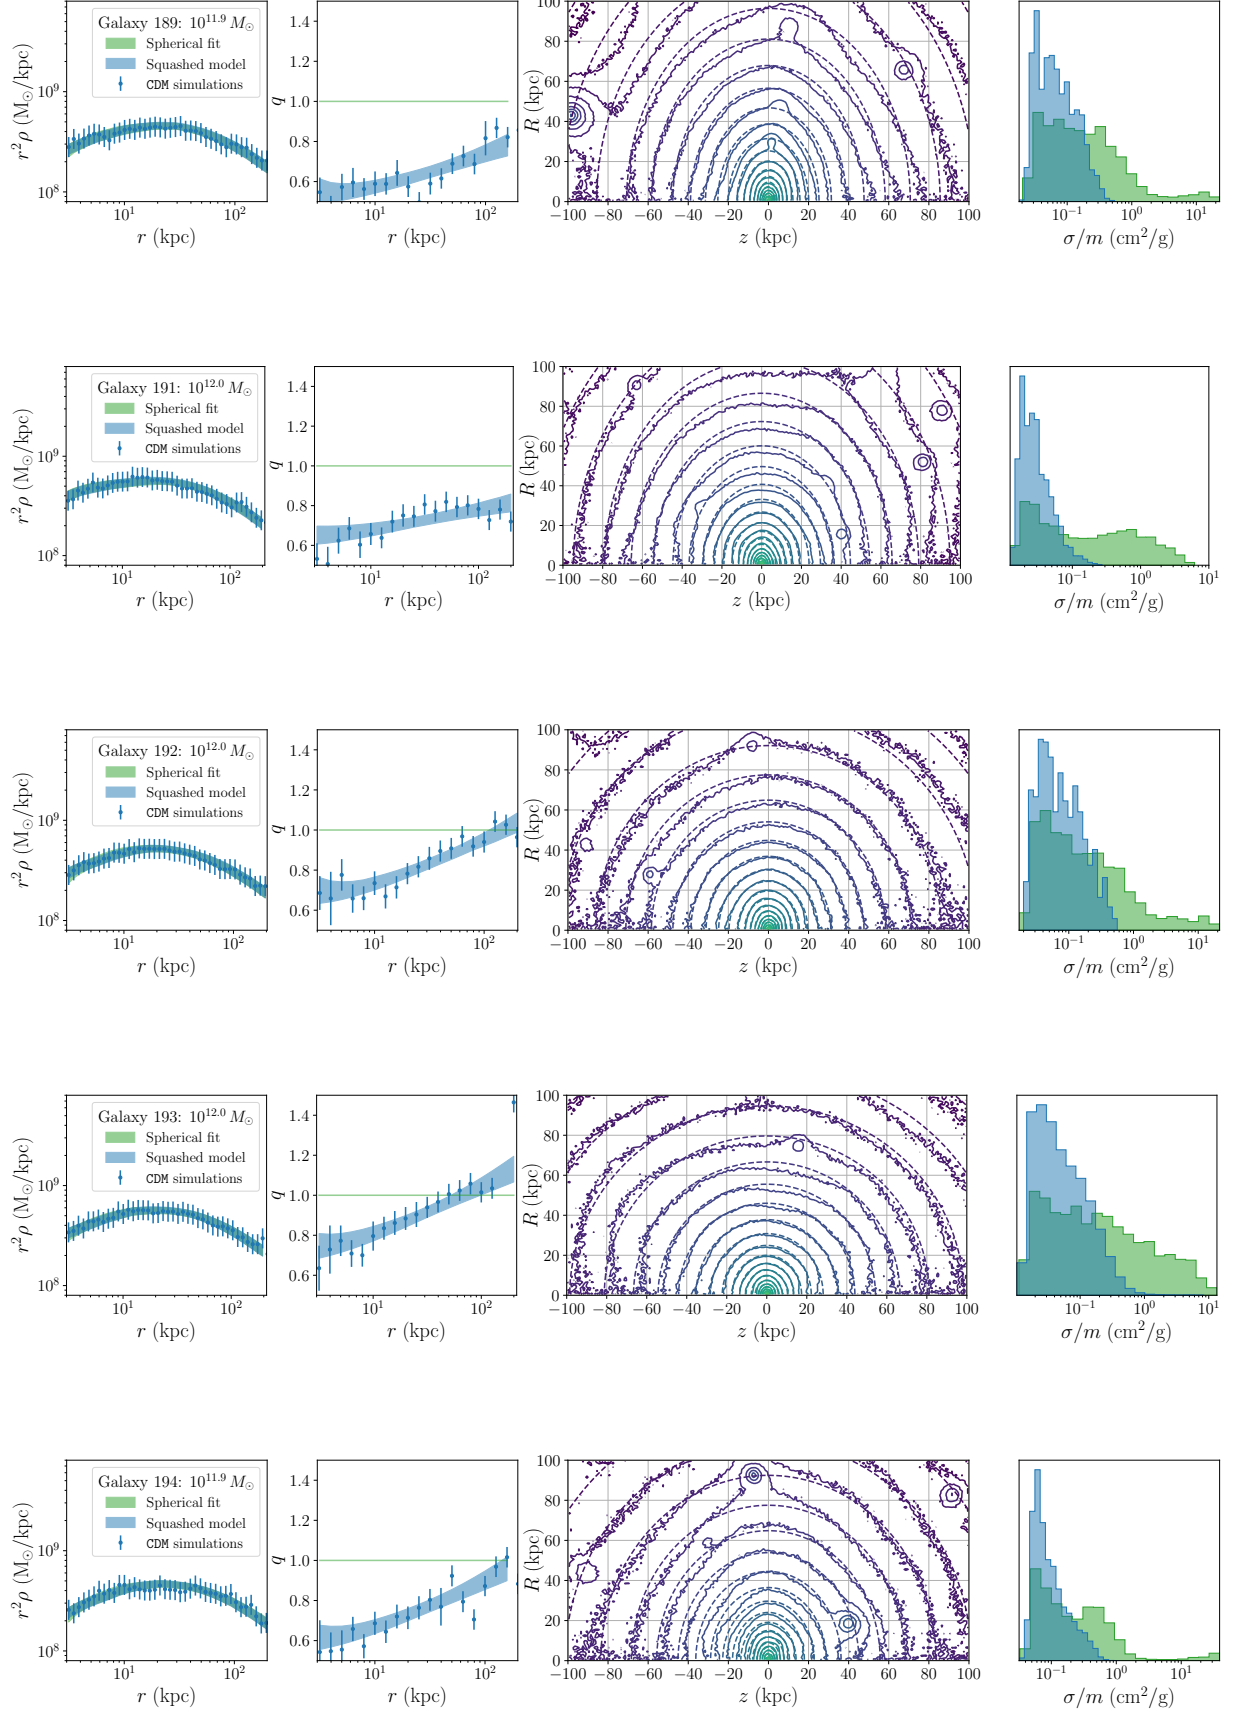

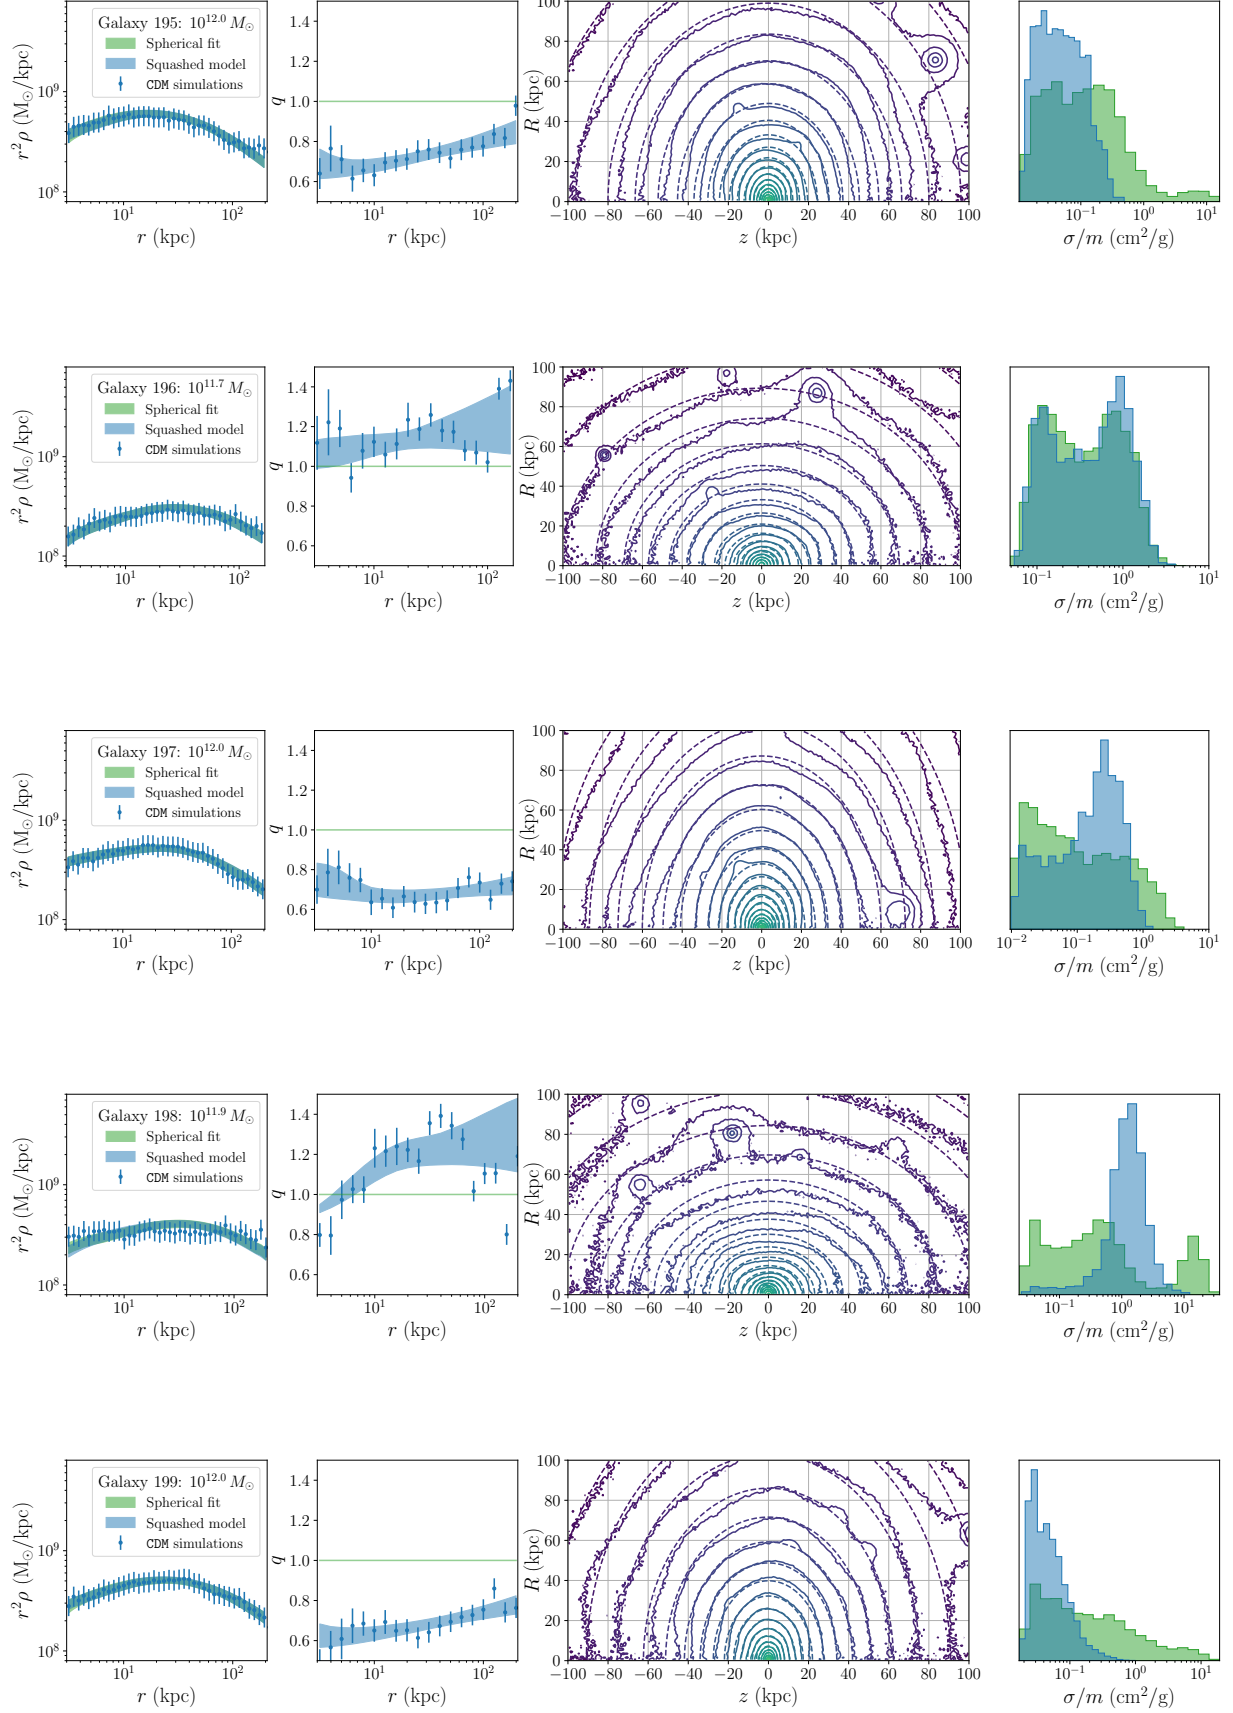



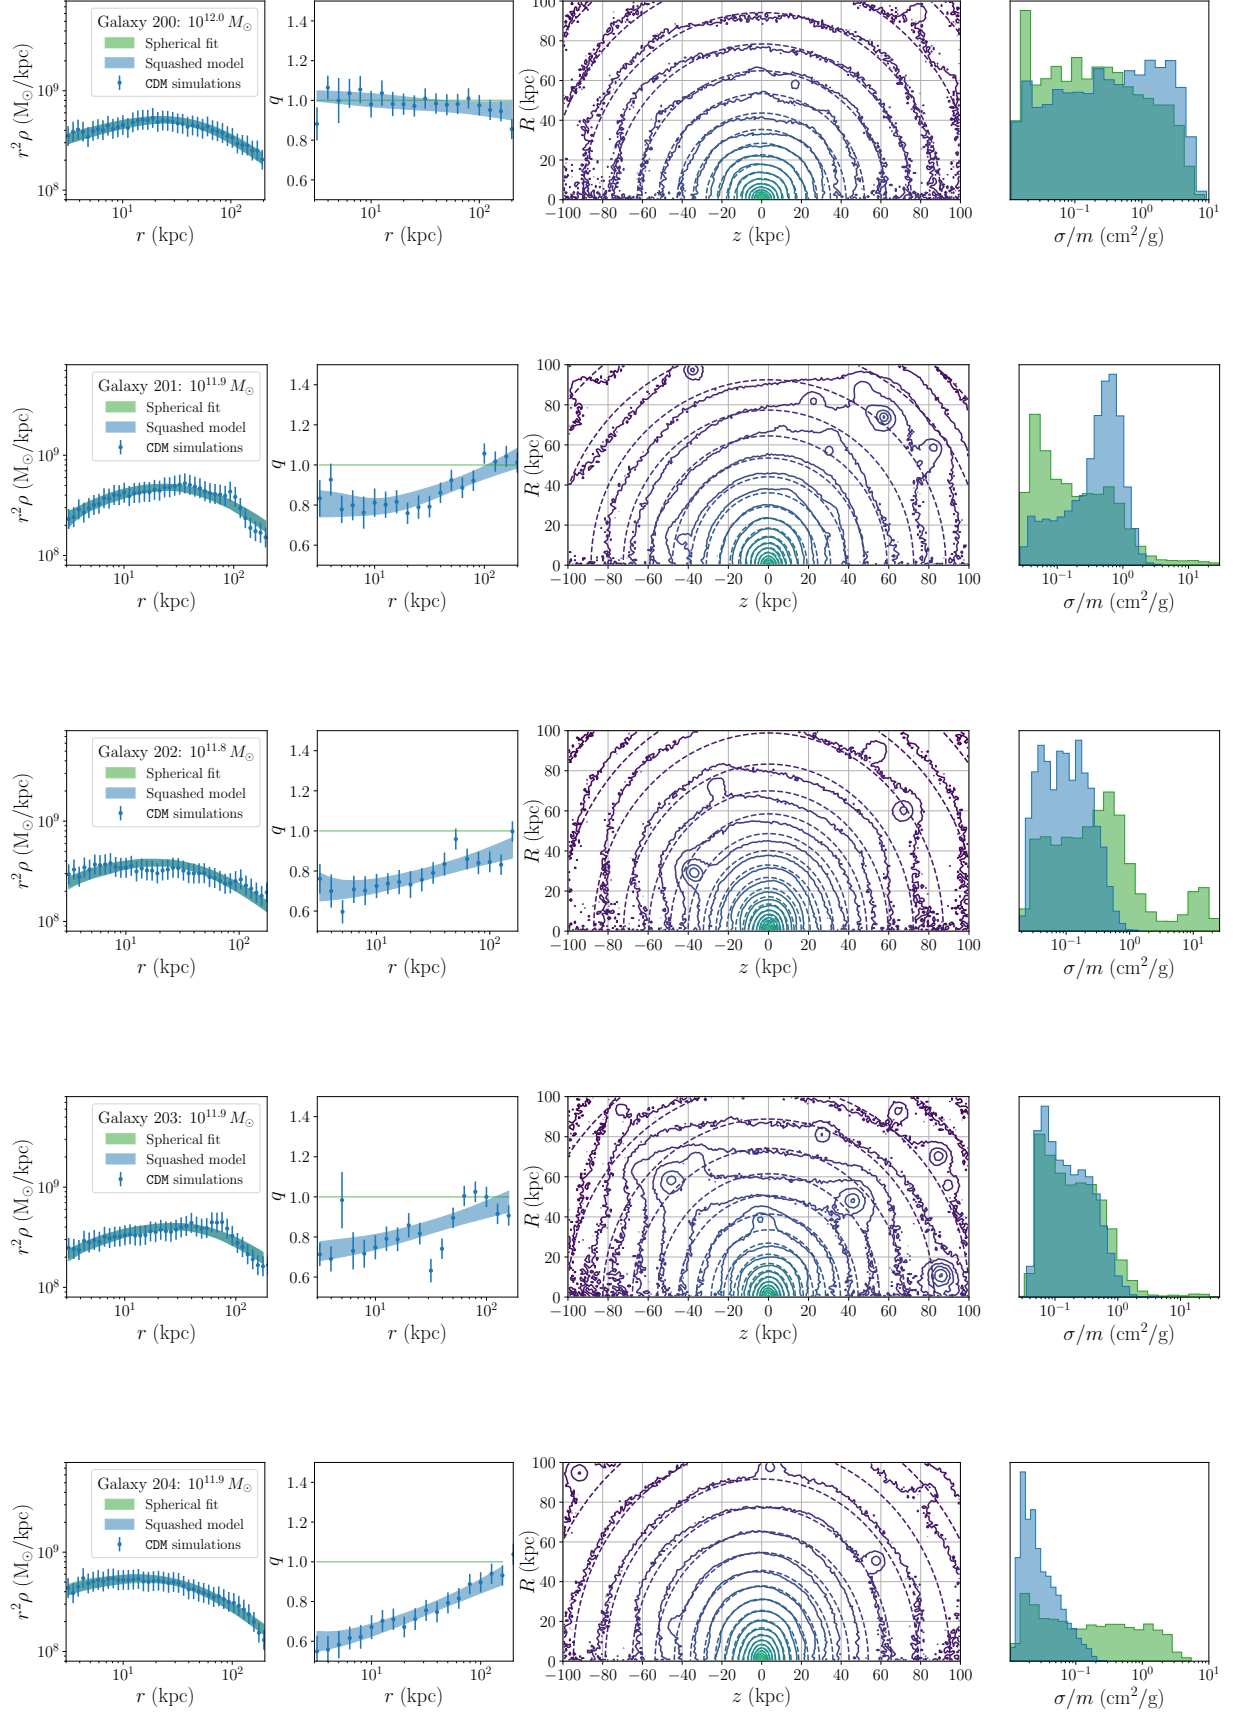



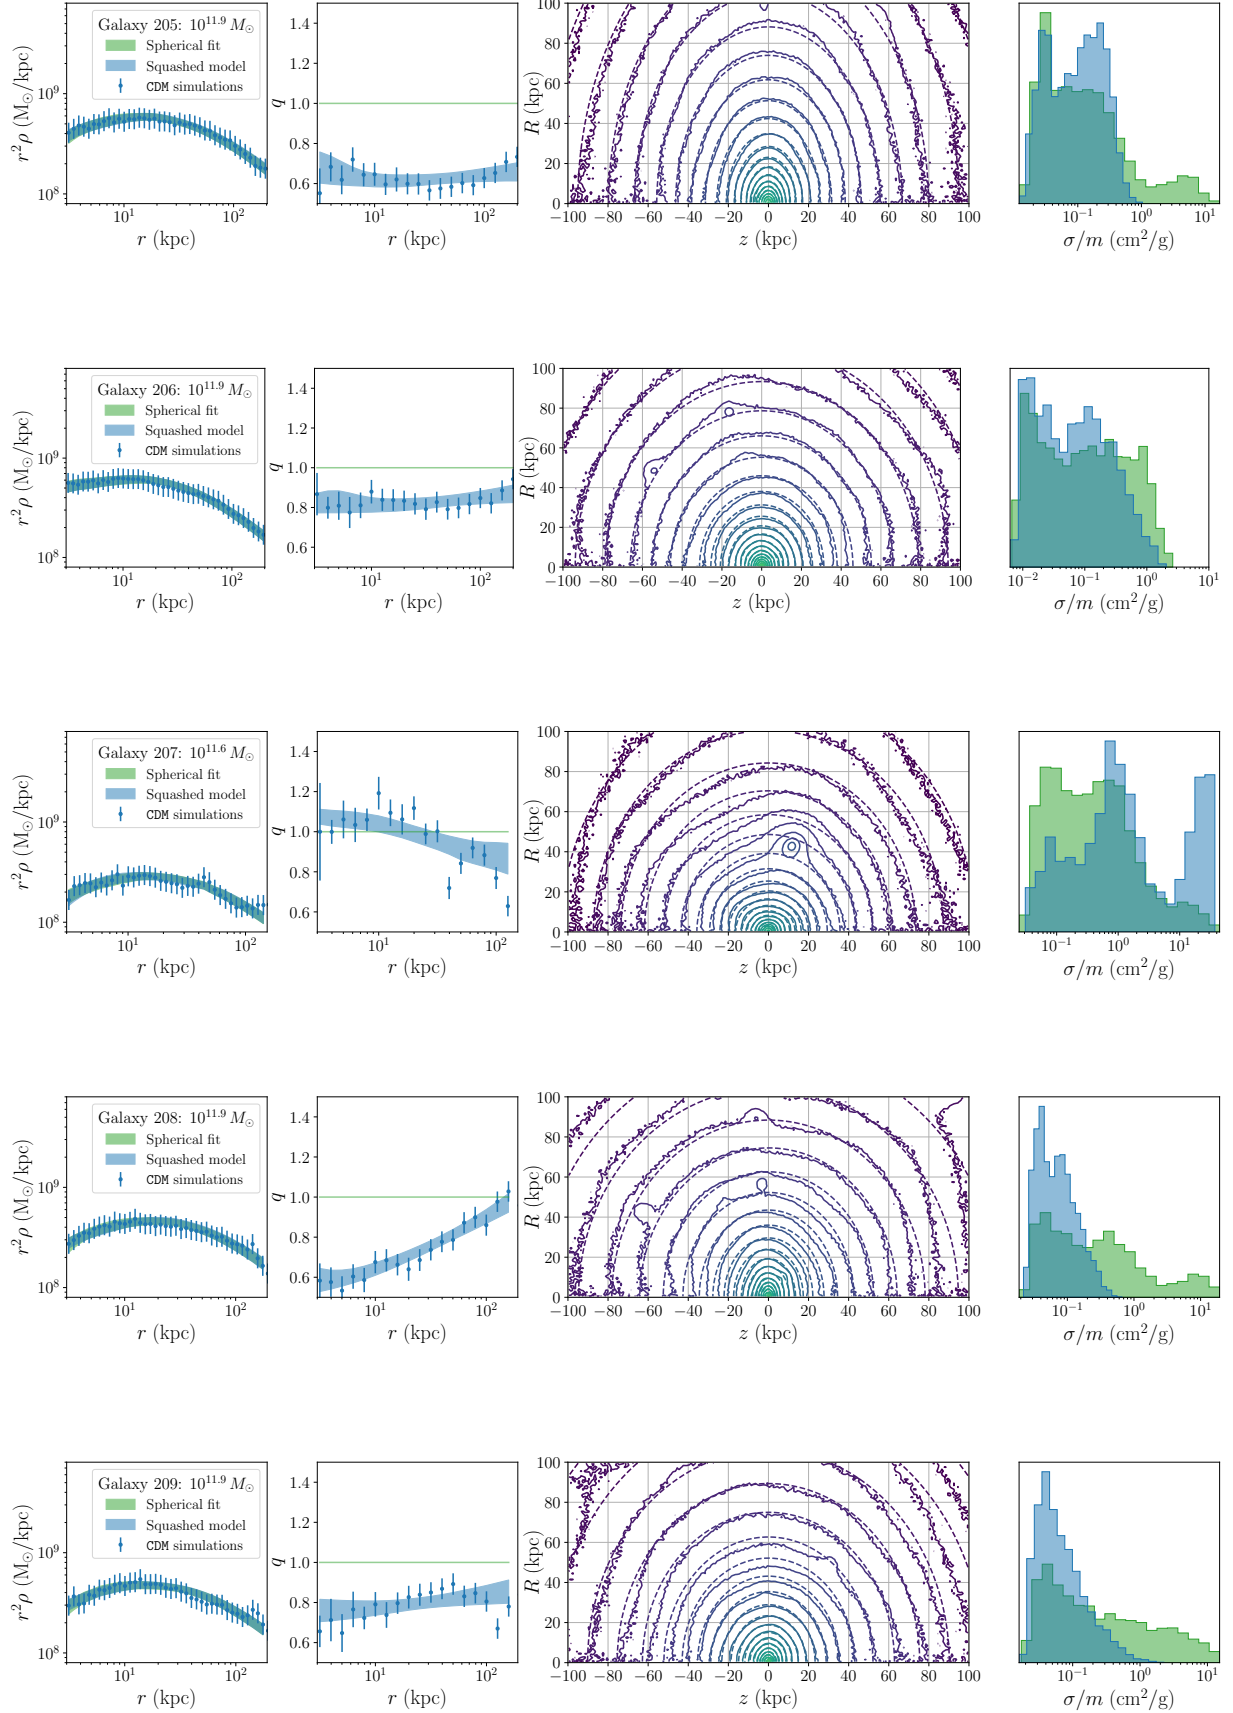

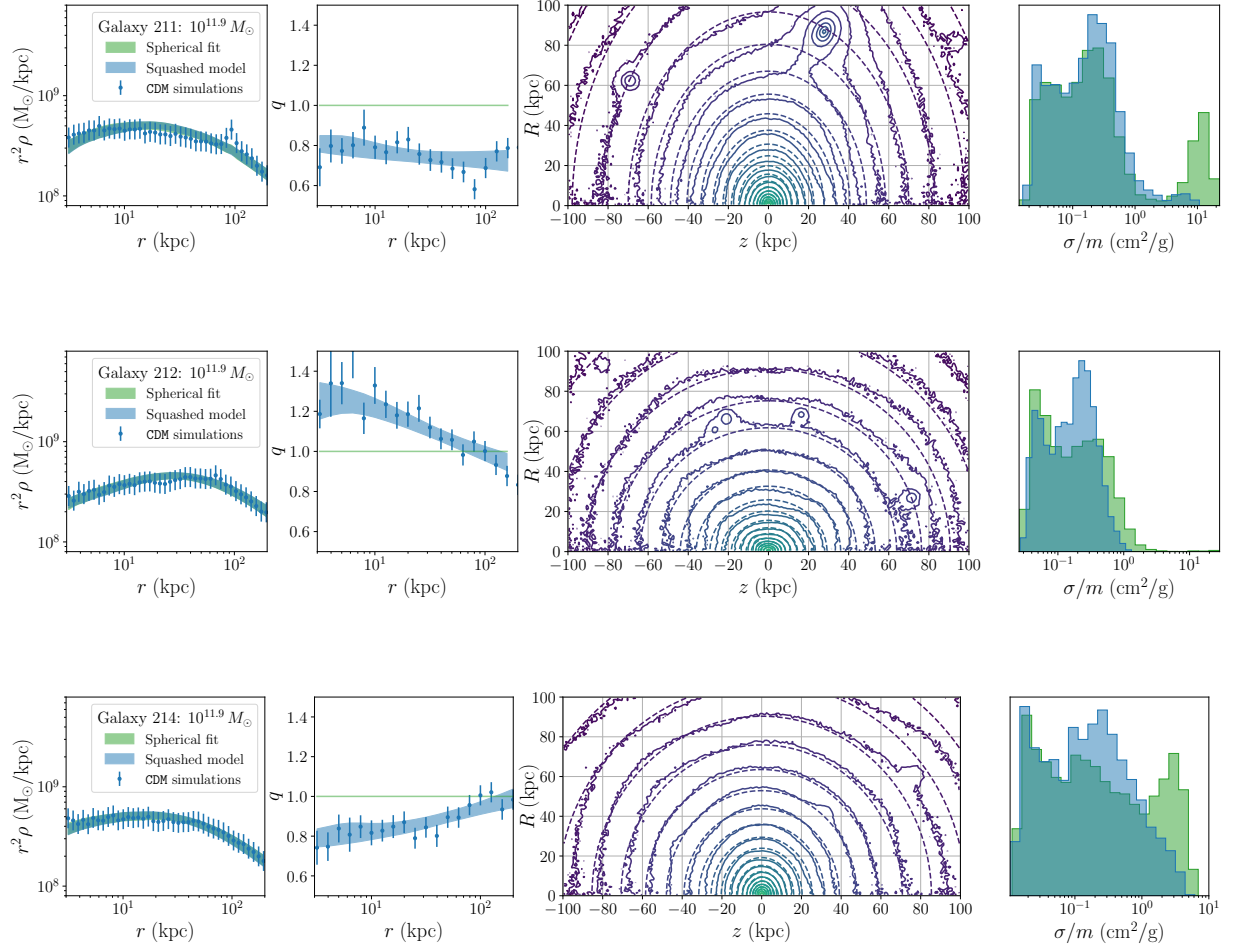

[1] A. Robertson et al., Mon. Not. Roy. Astron. Soc. 501 (2021) 4610, 2009.07844.
